# Supplementary material for: Background Matting
Source: arXiv:2002.04433 source file (2020-02-11)

| Image                                                                              | GT                                                                                  | AlphaGan-BG_M                                                                        | AlphaGan-BG_H                                                                         | AlphaGAN                                                                              |
|------------------------------------------------------------------------------------|-------------------------------------------------------------------------------------|--------------------------------------------------------------------------------------|---------------------------------------------------------------------------------------|---------------------------------------------------------------------------------------|
| 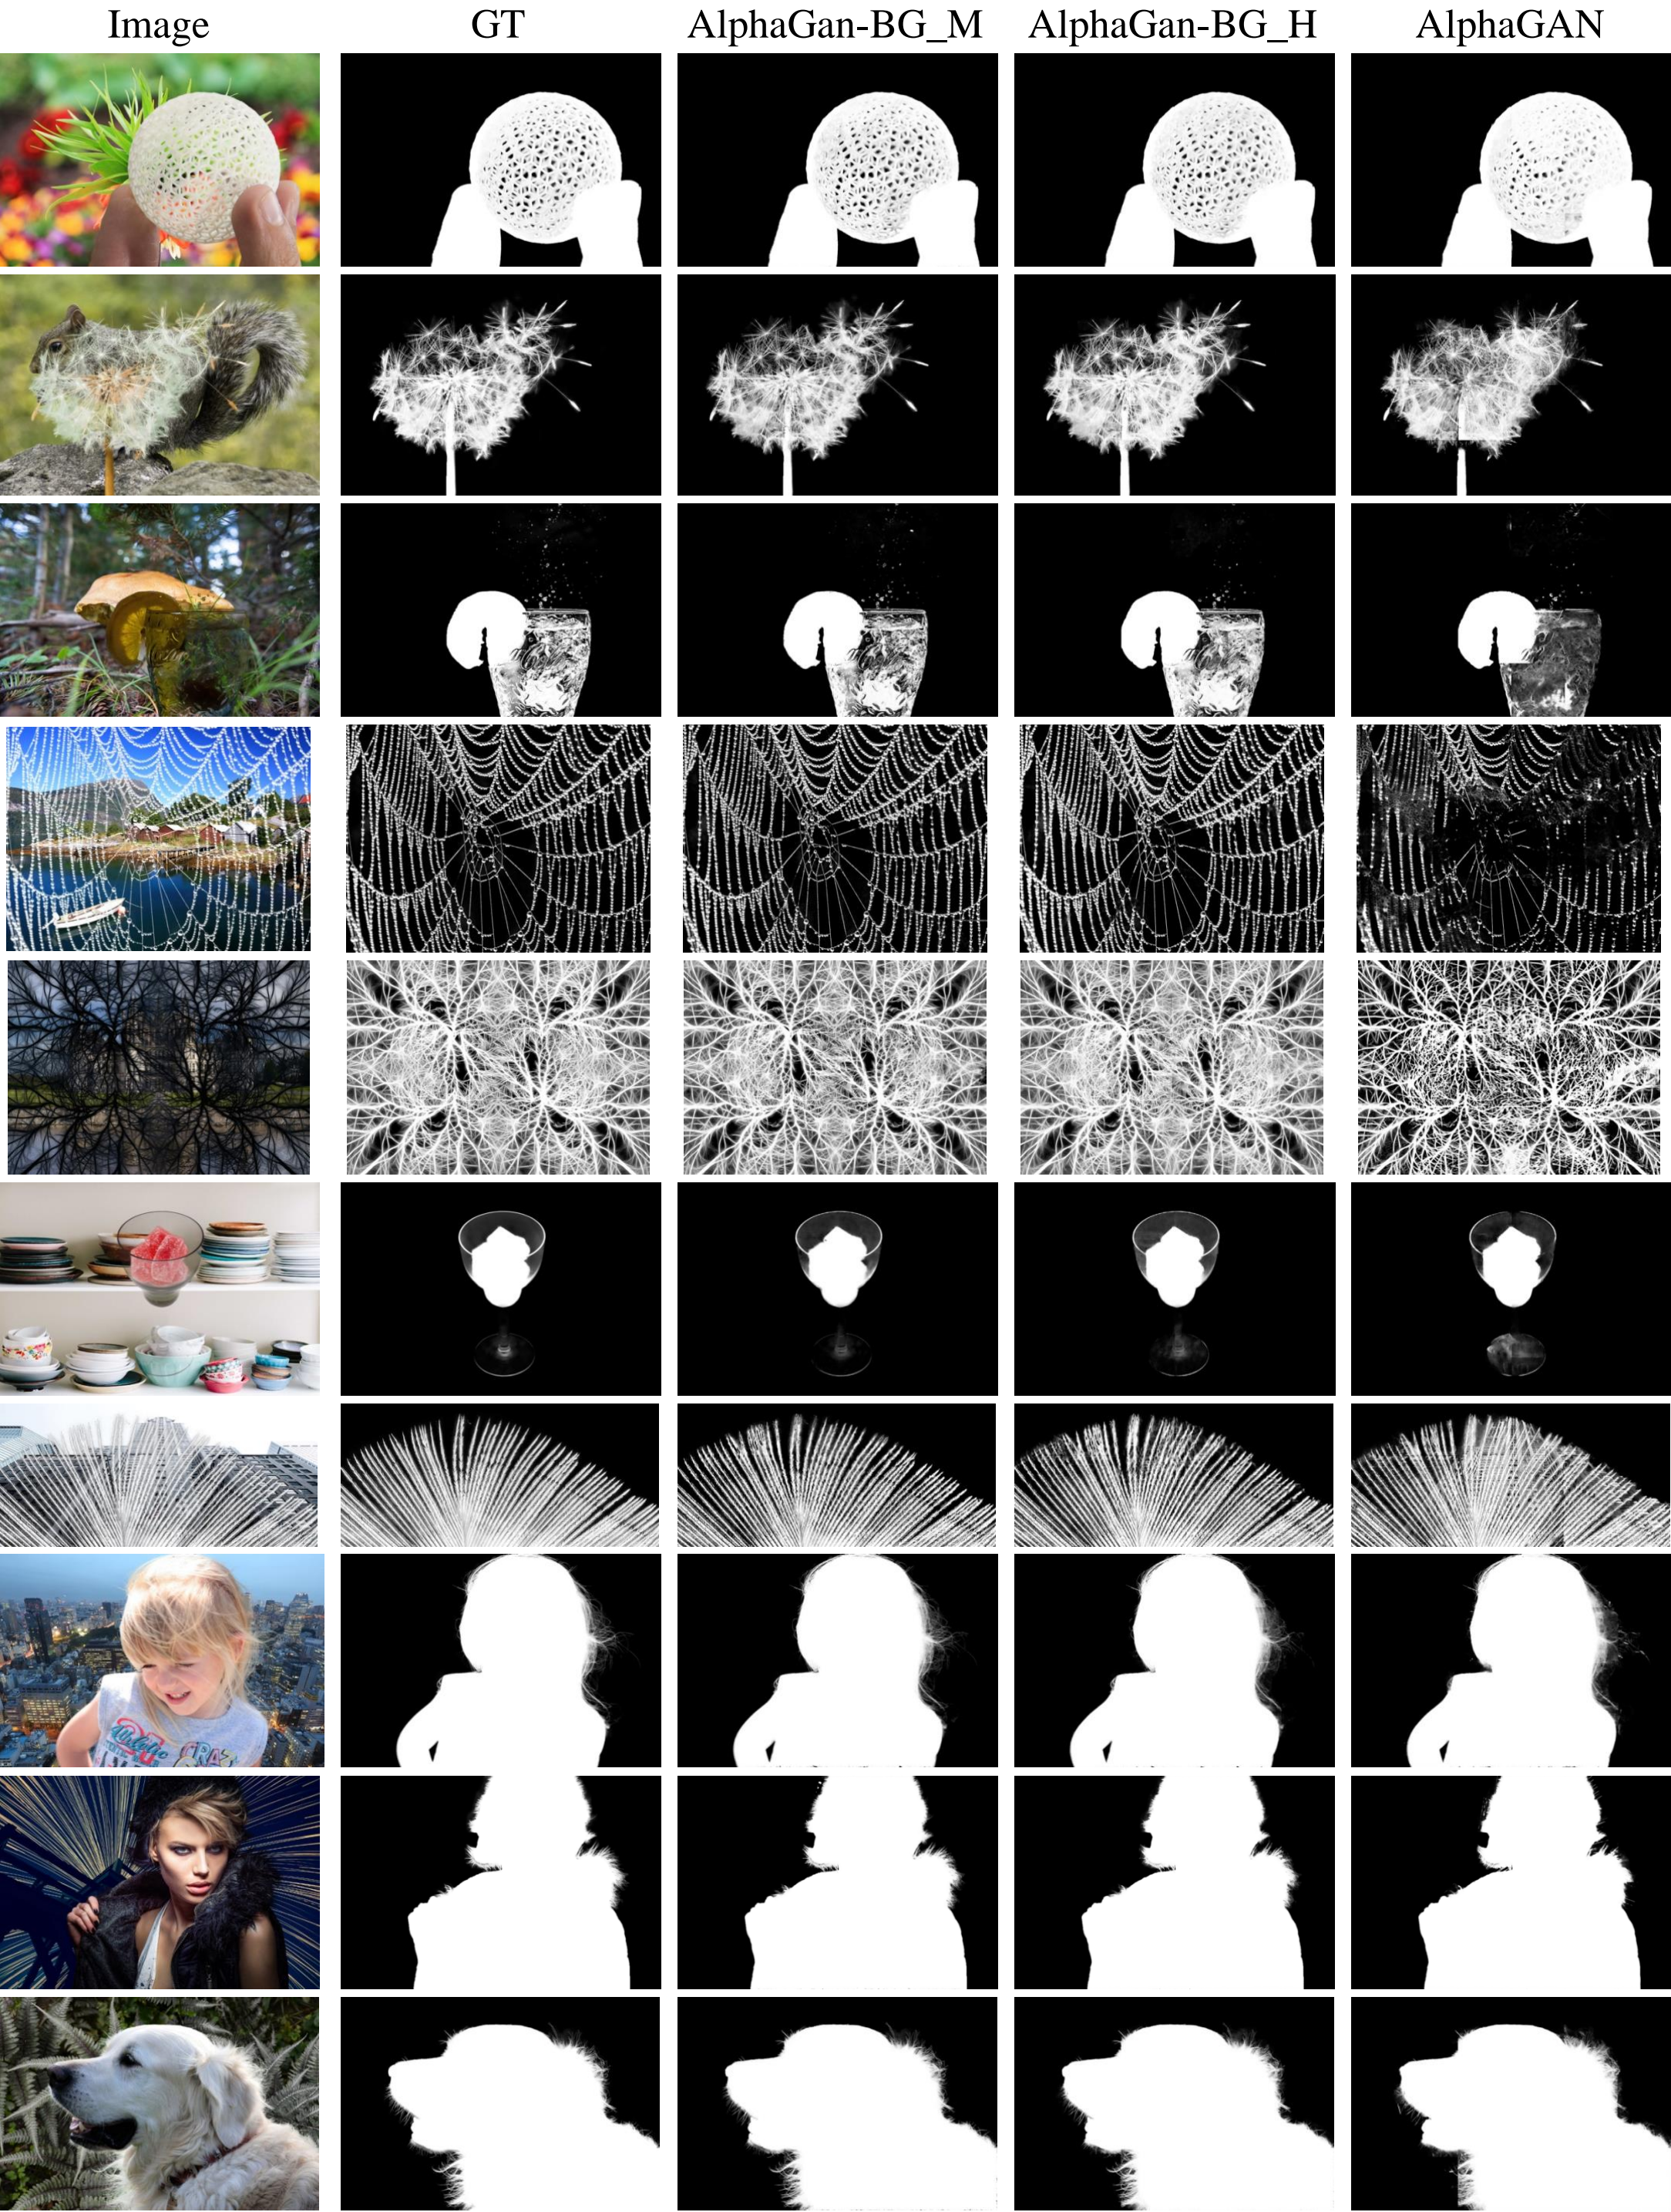   | 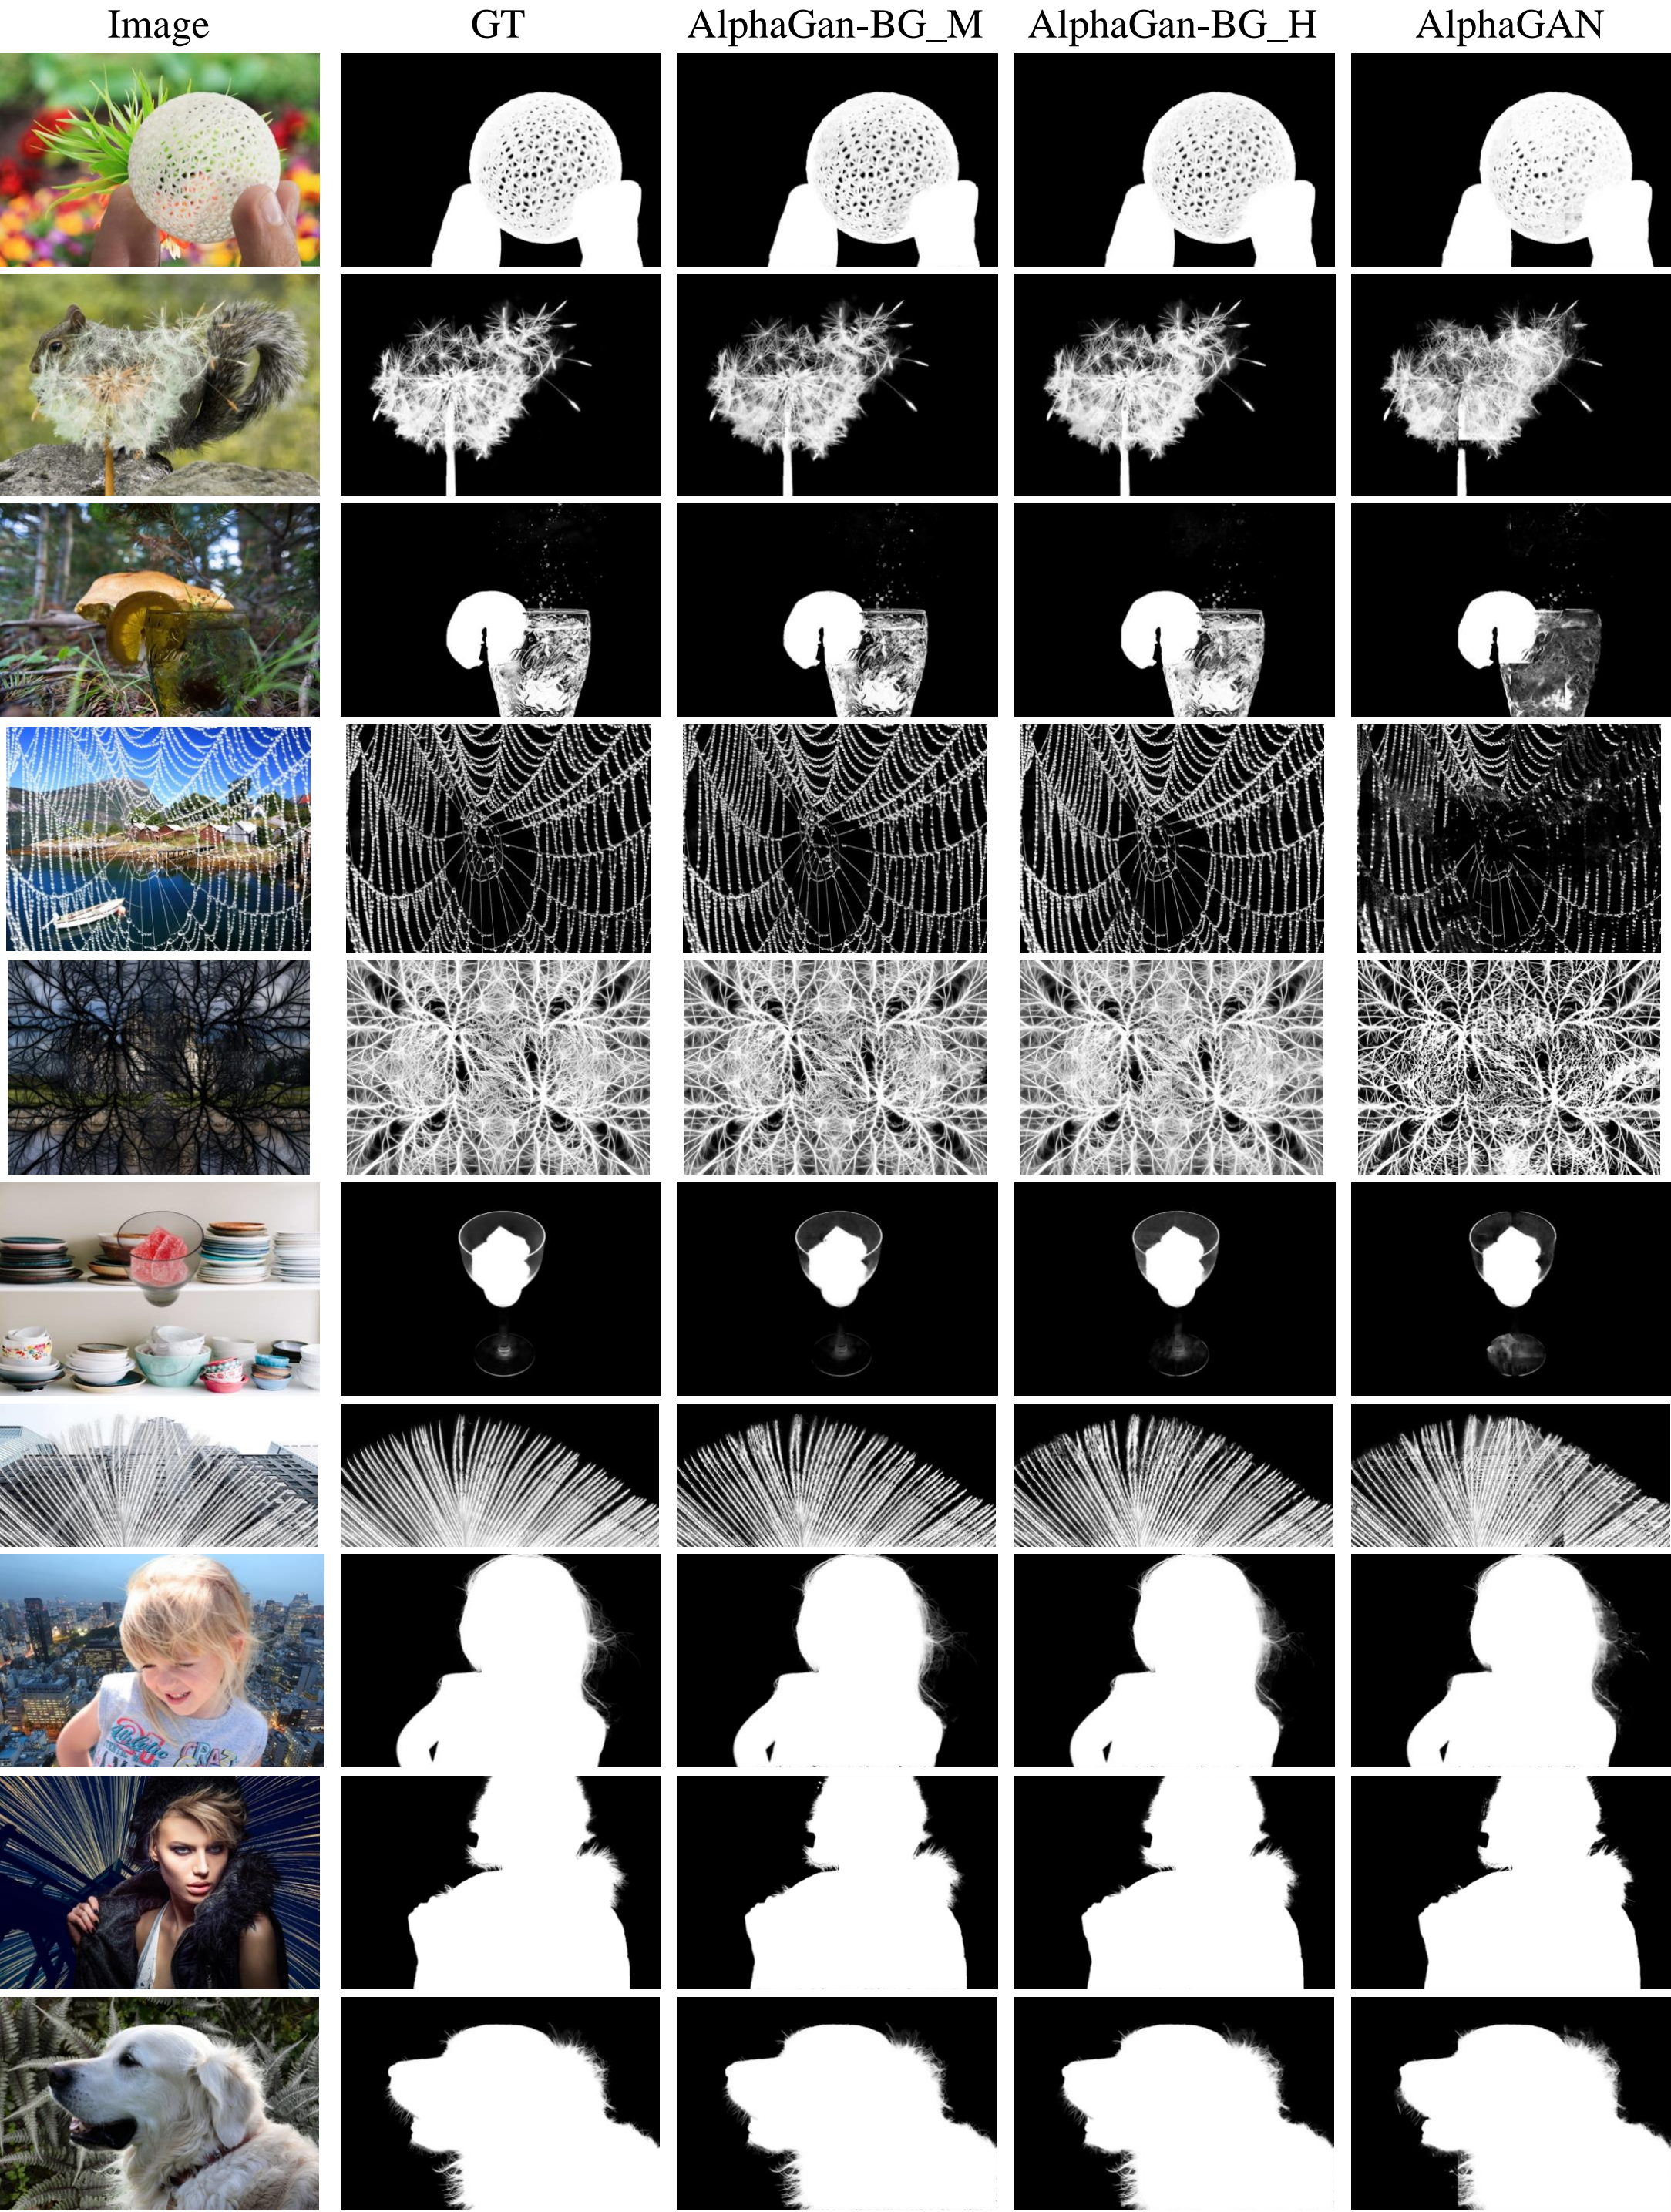   | 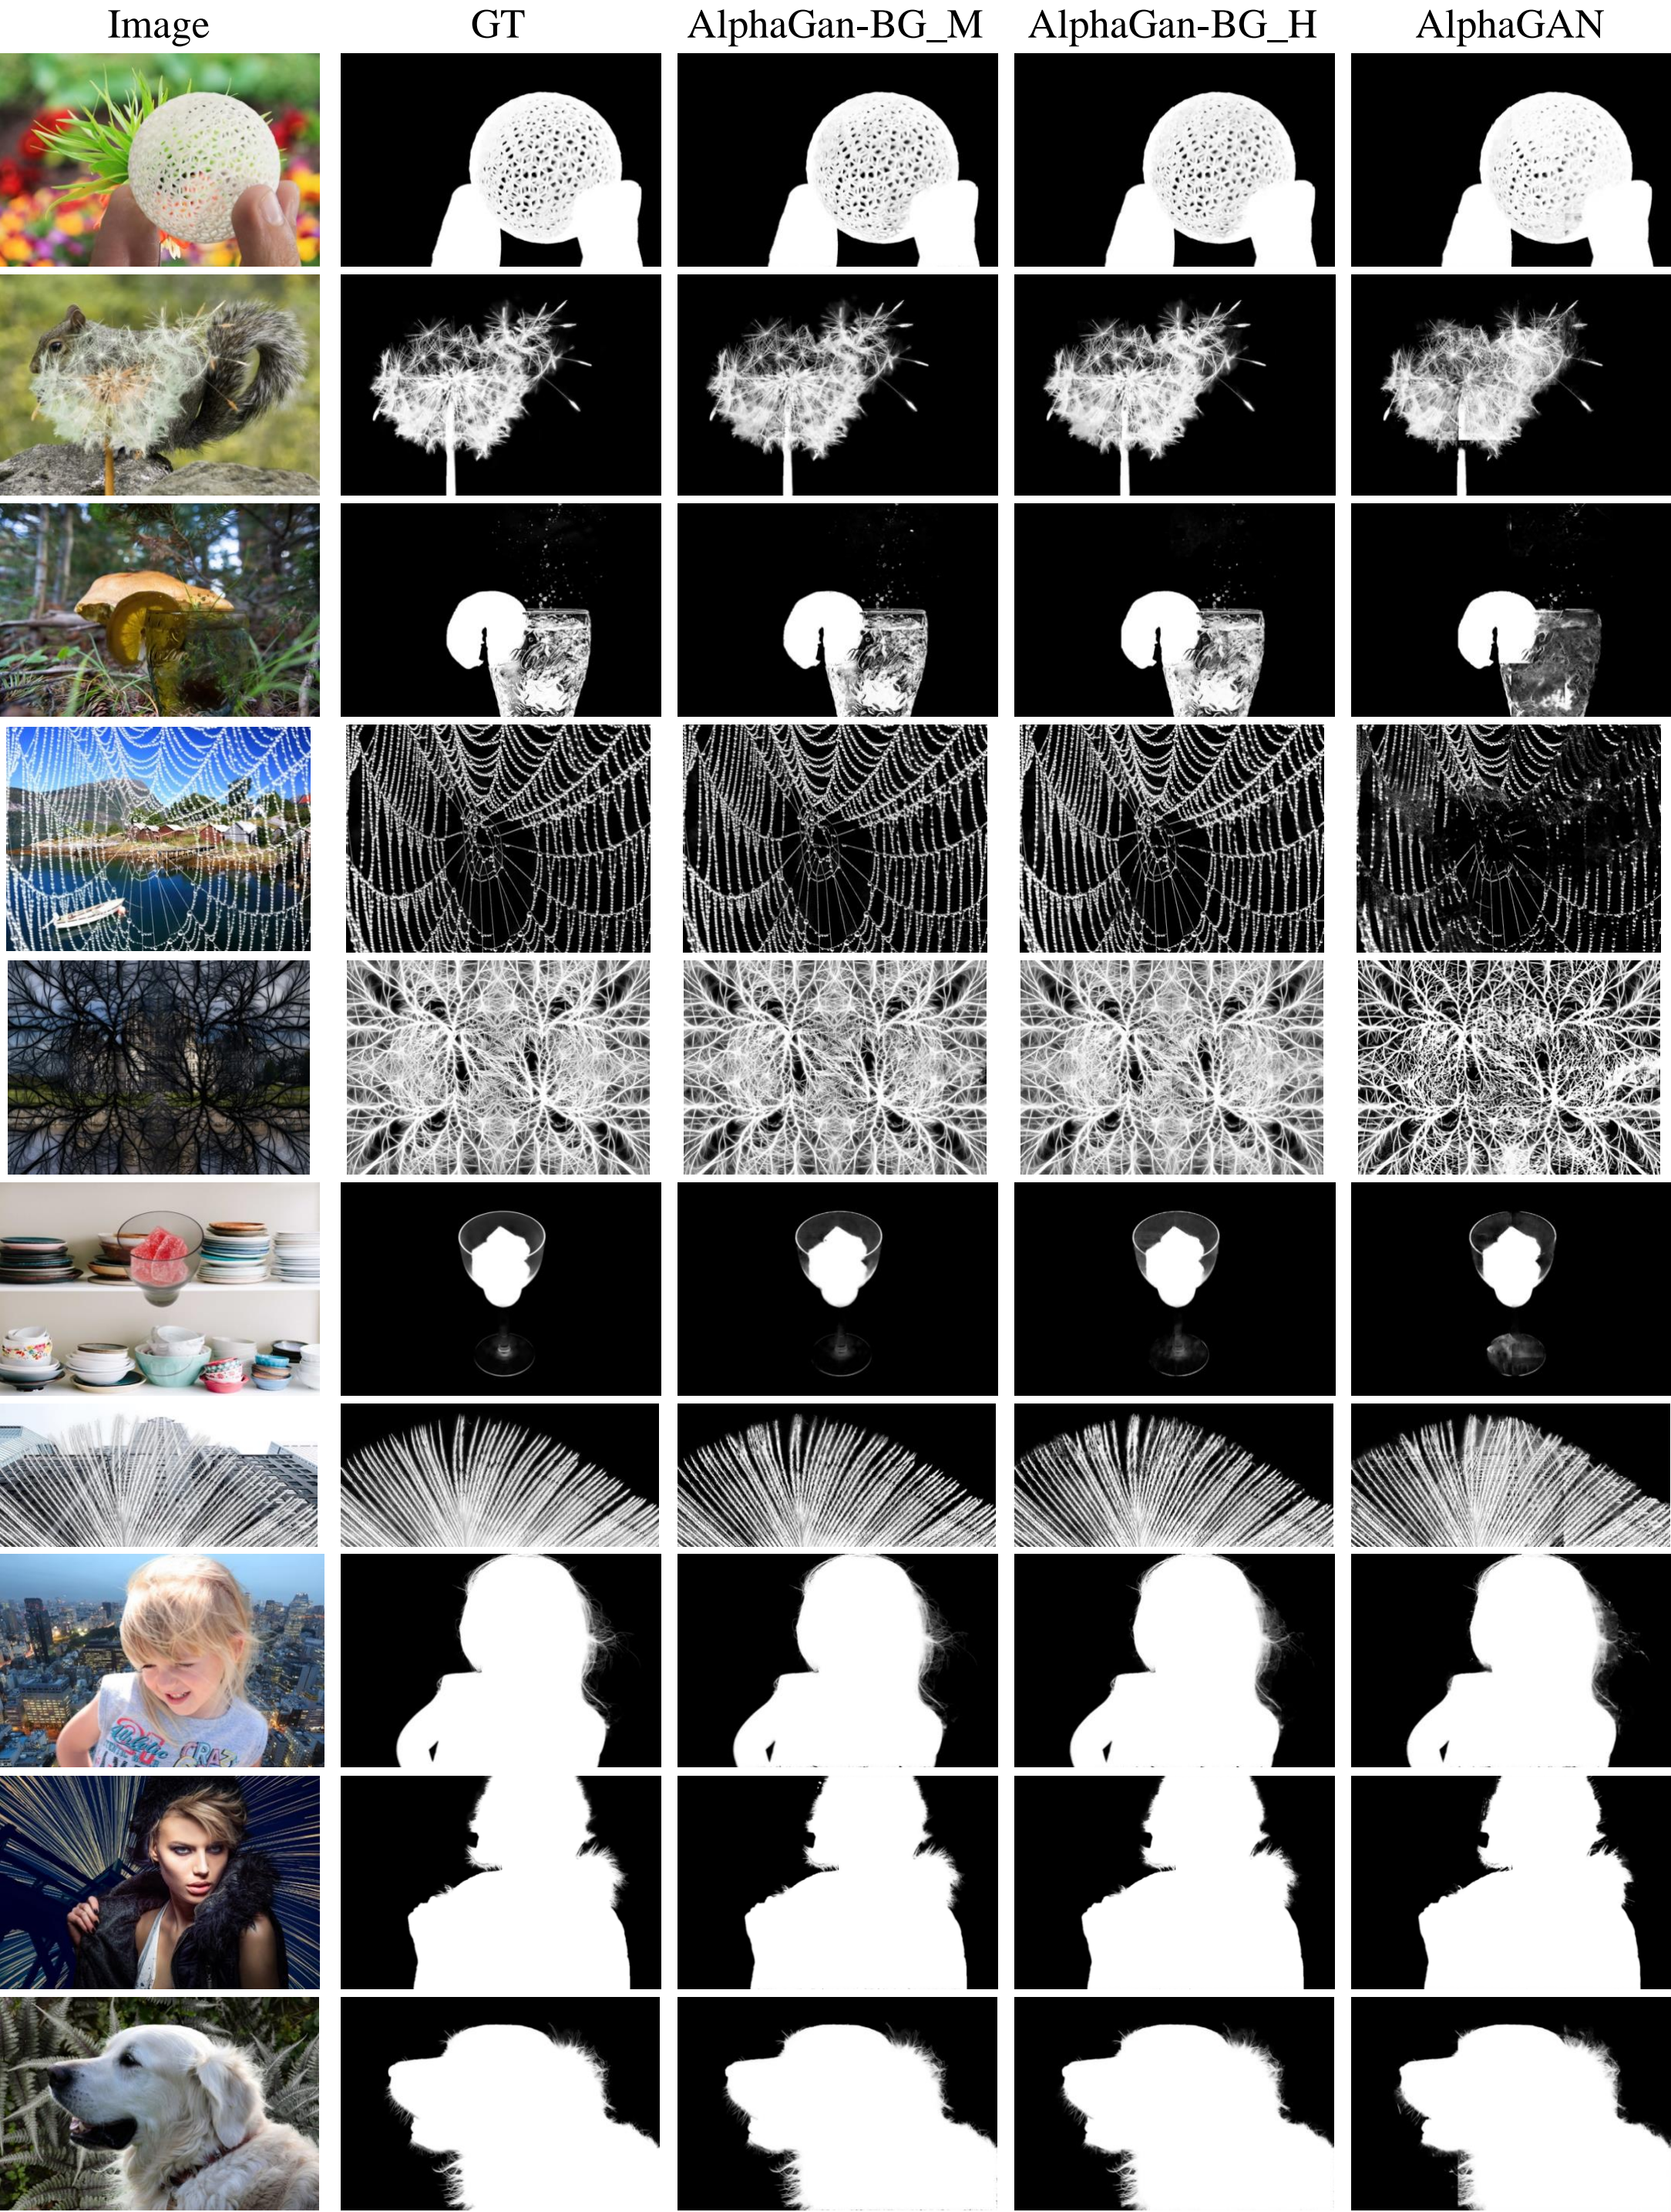   | 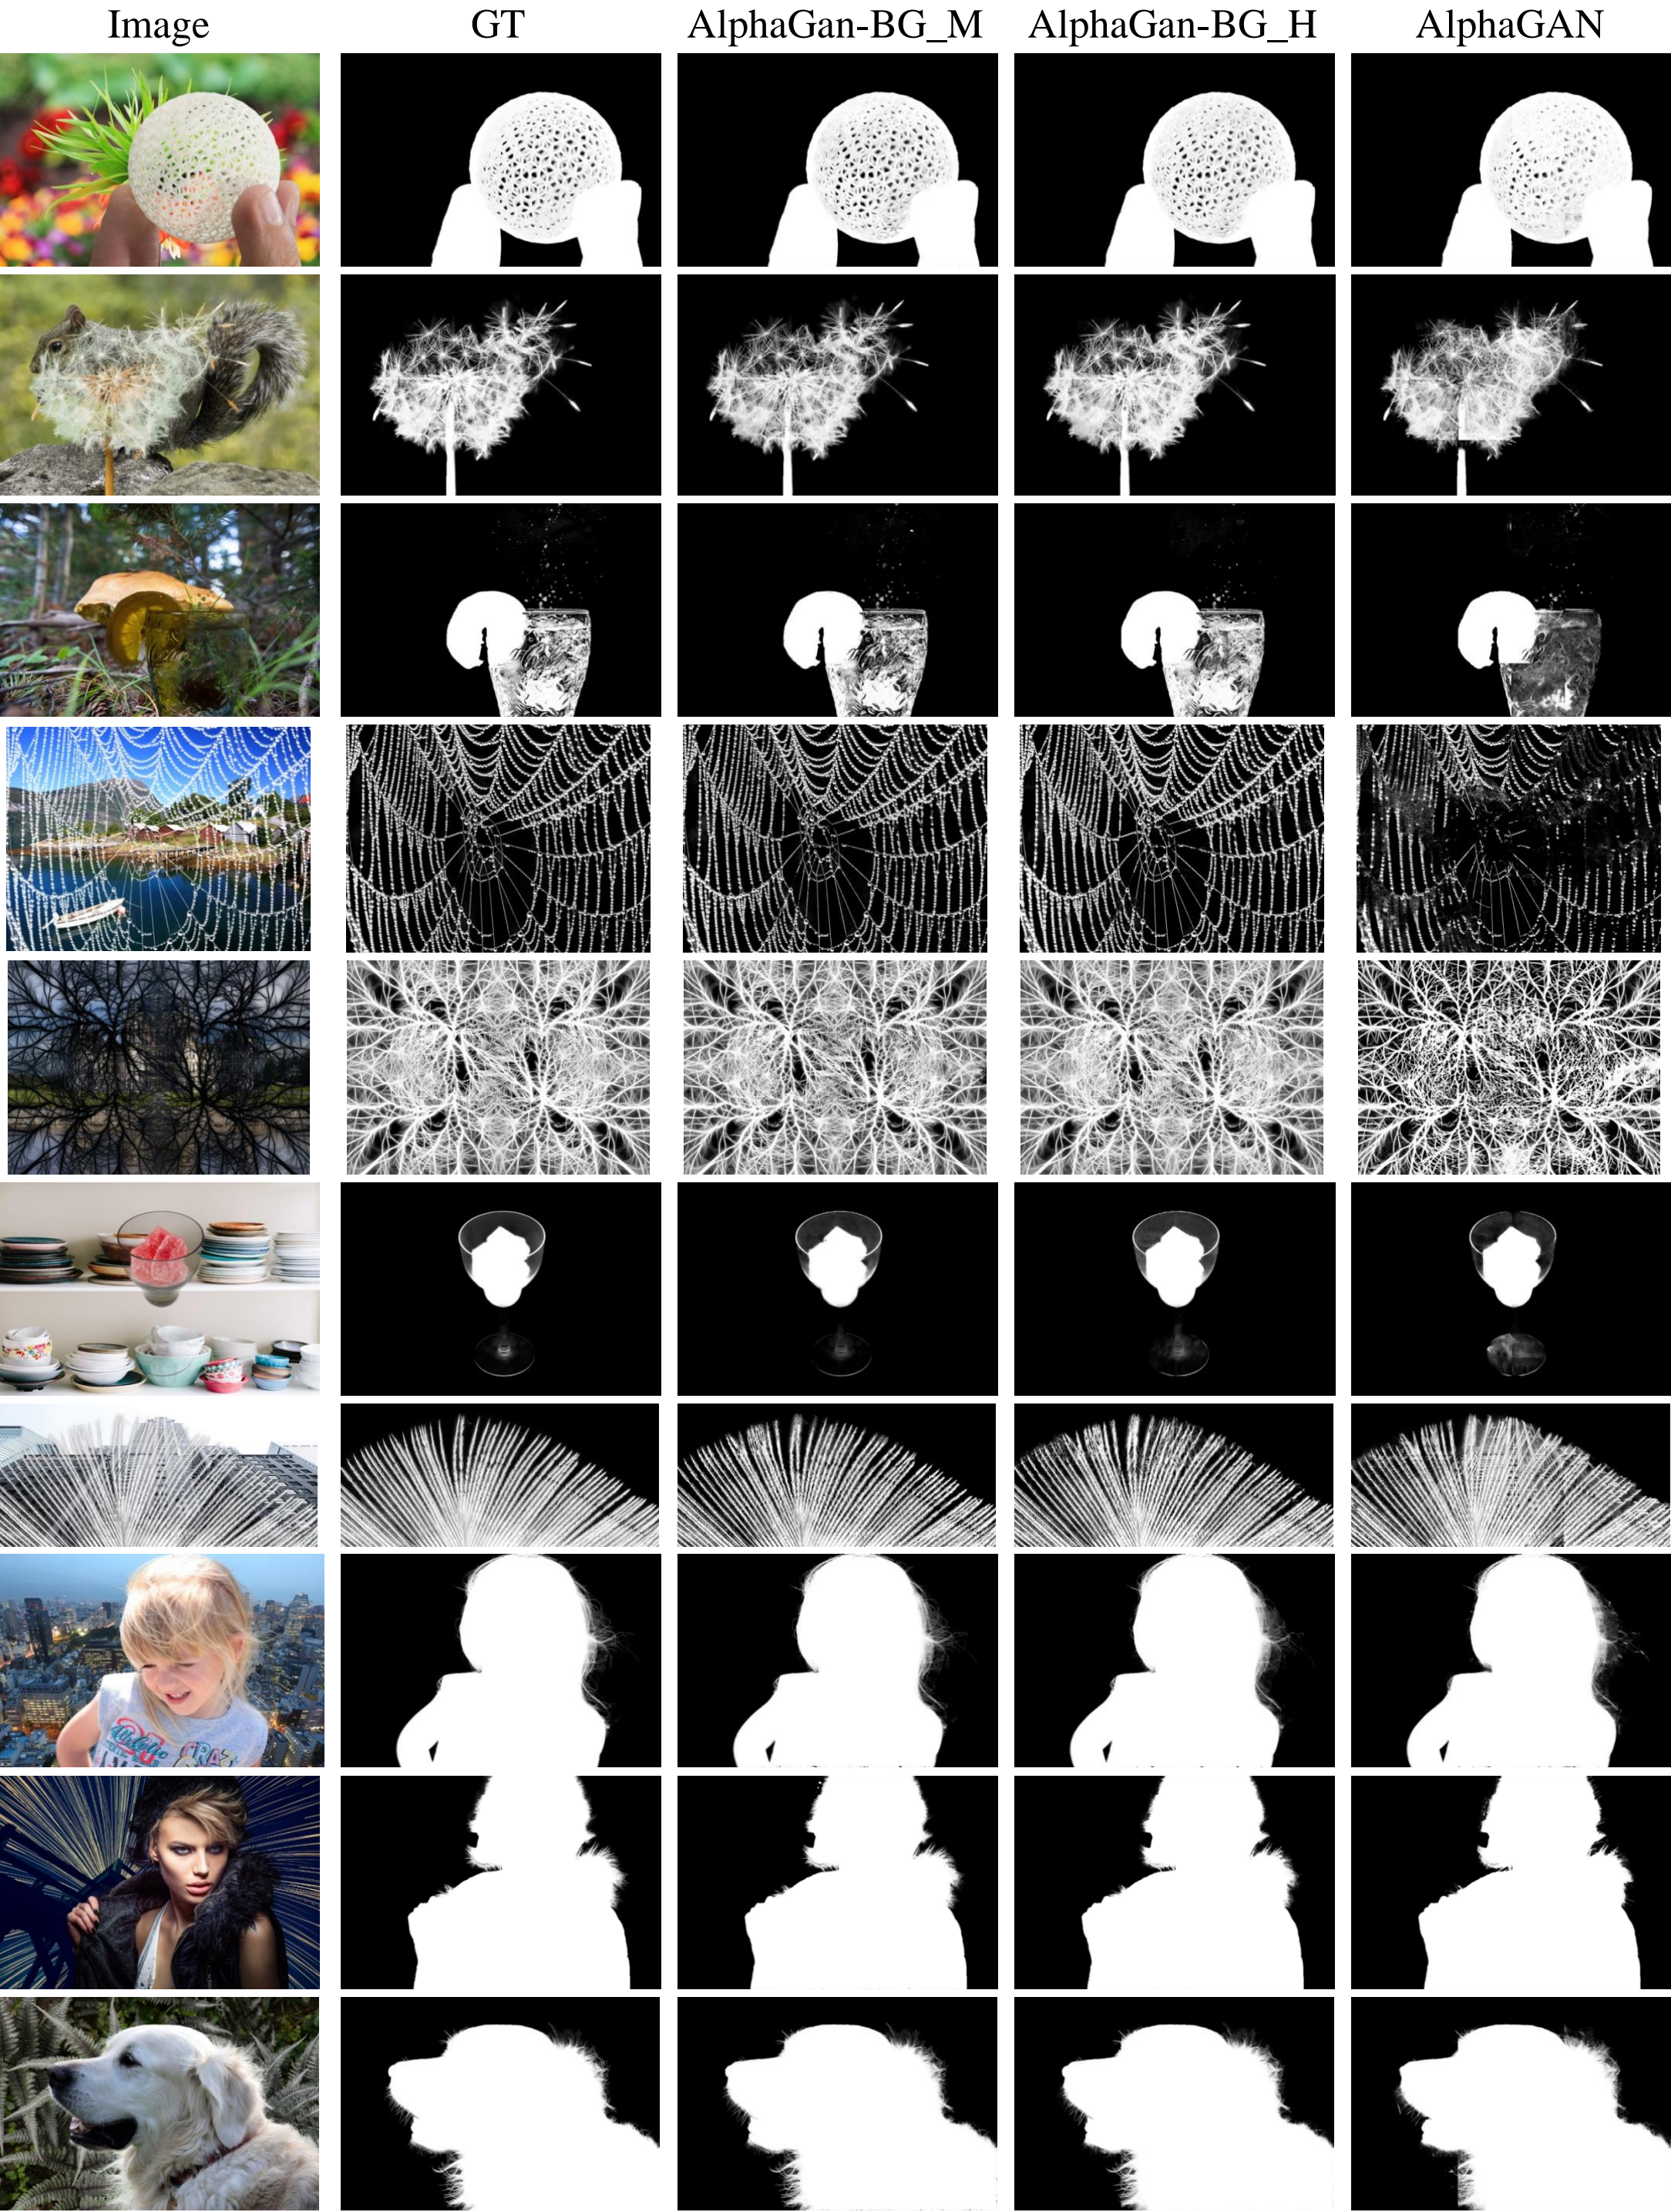   | 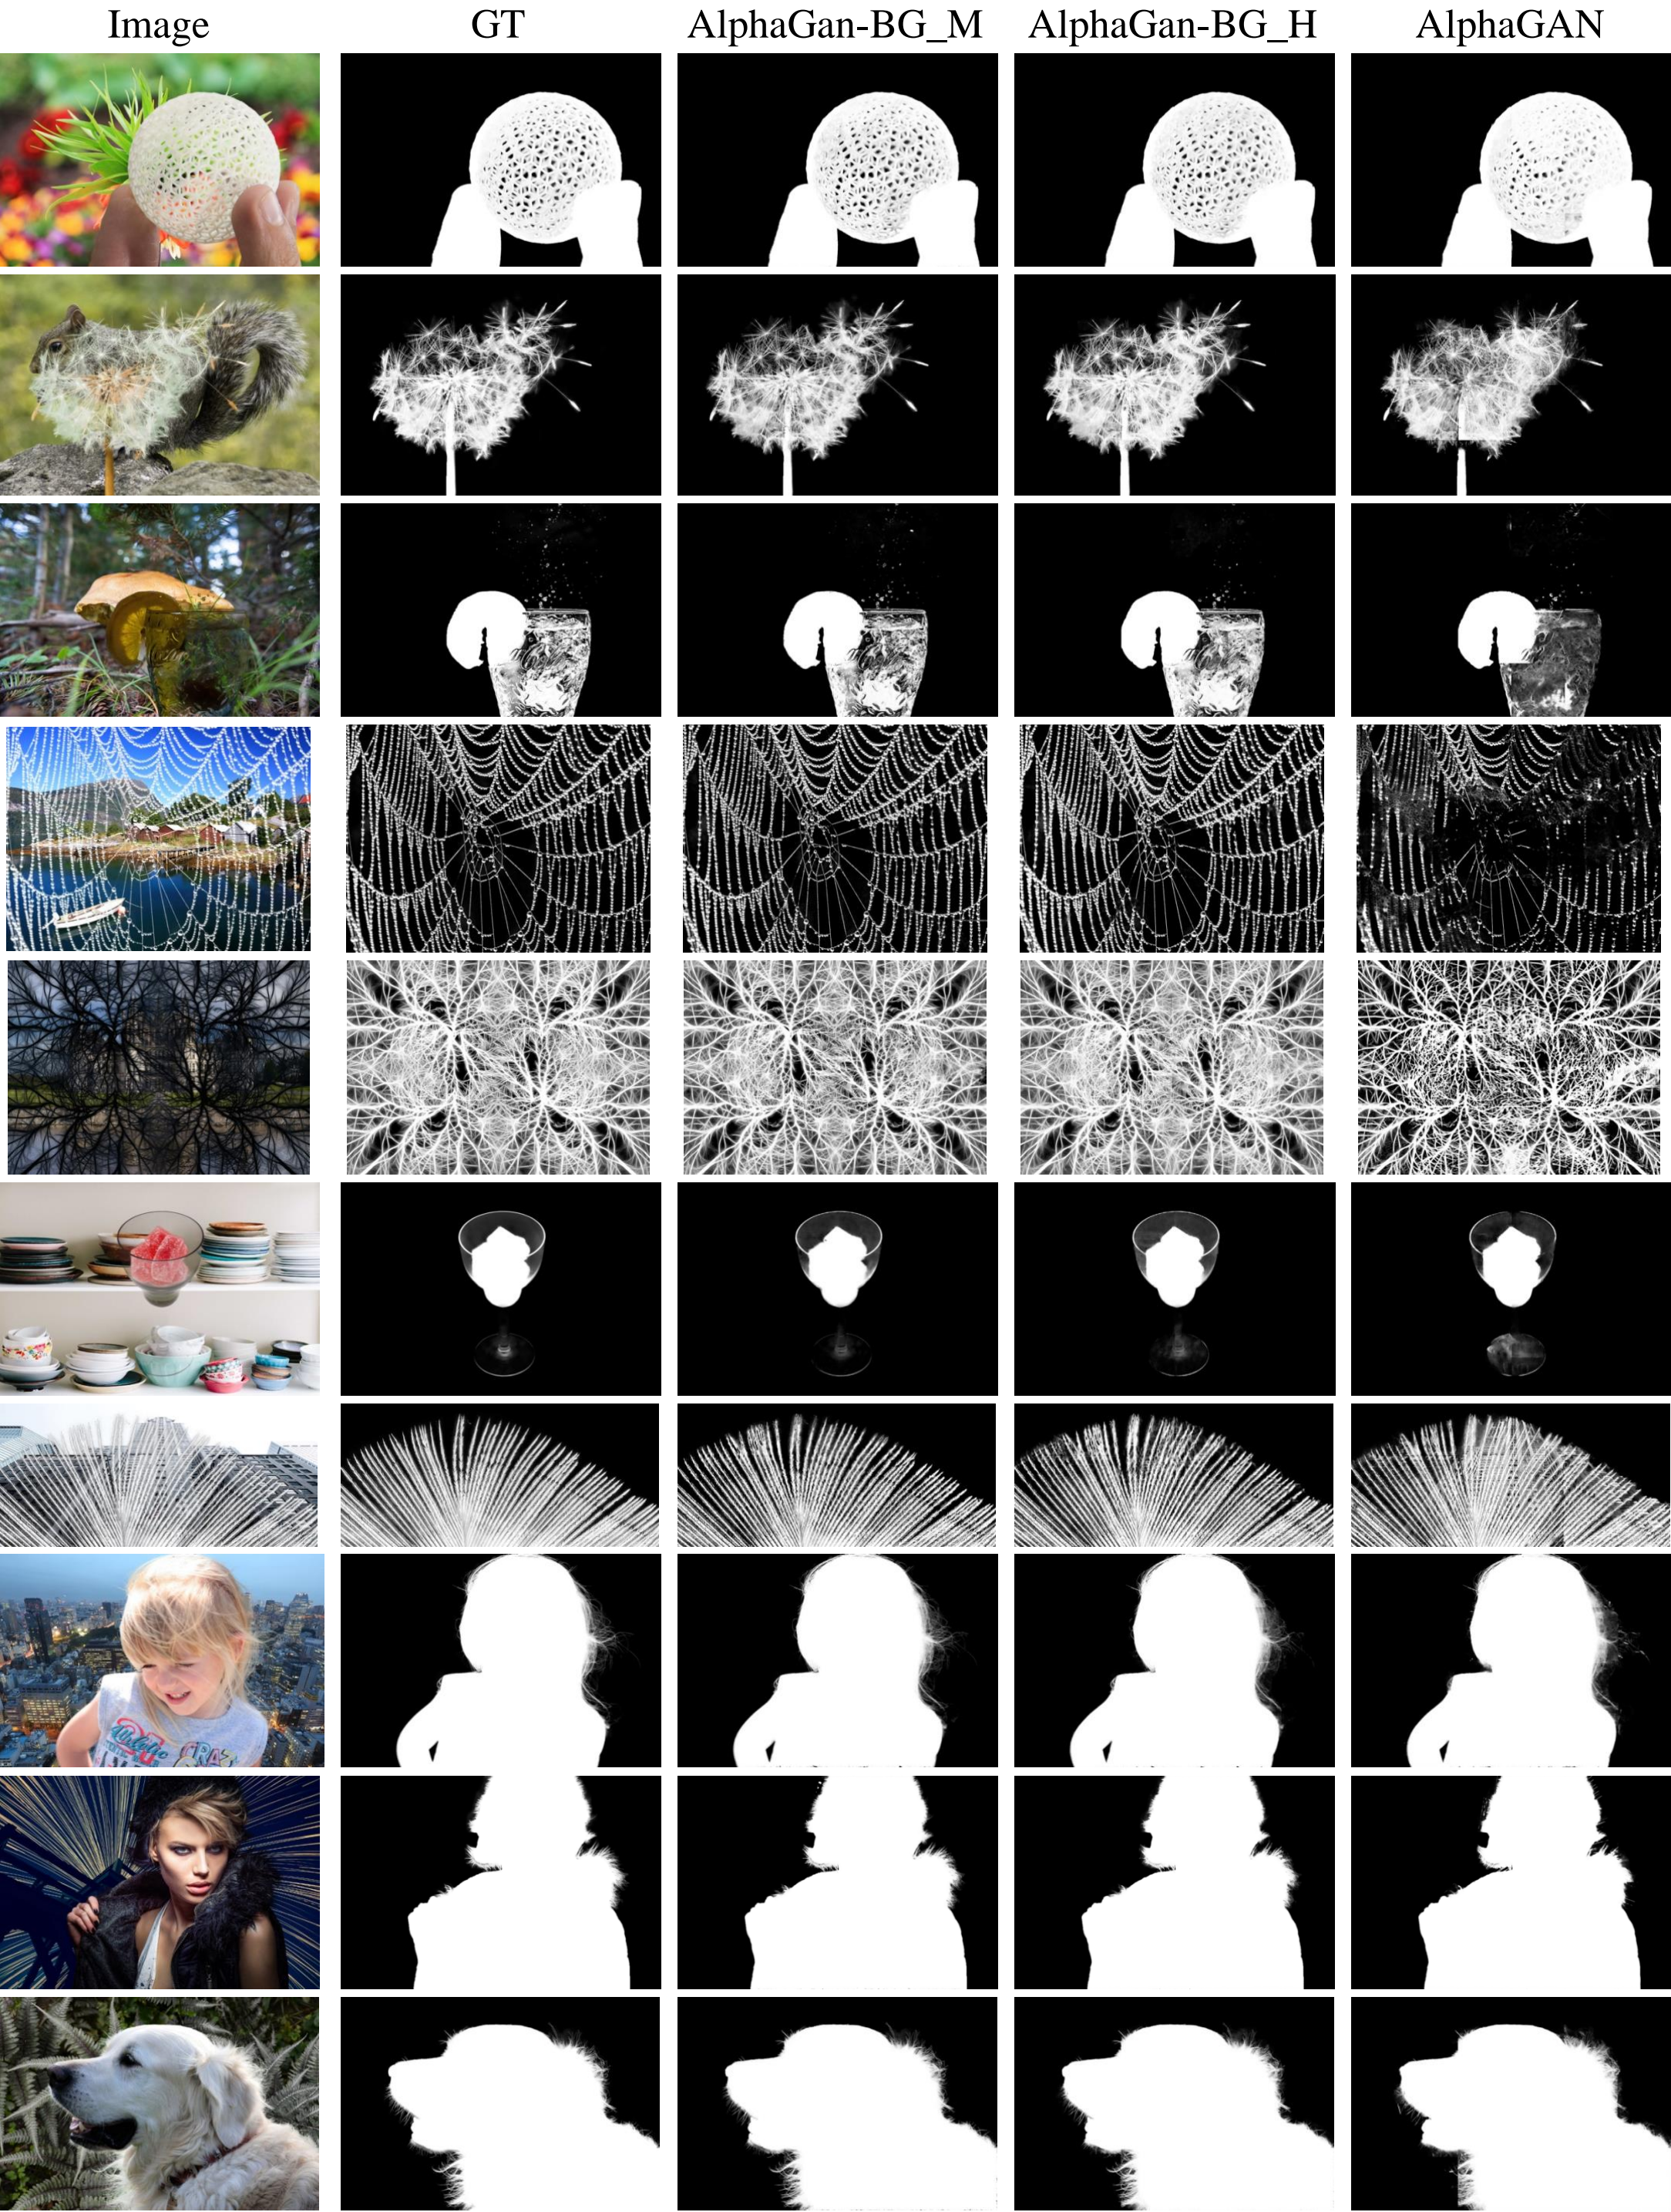   |
| 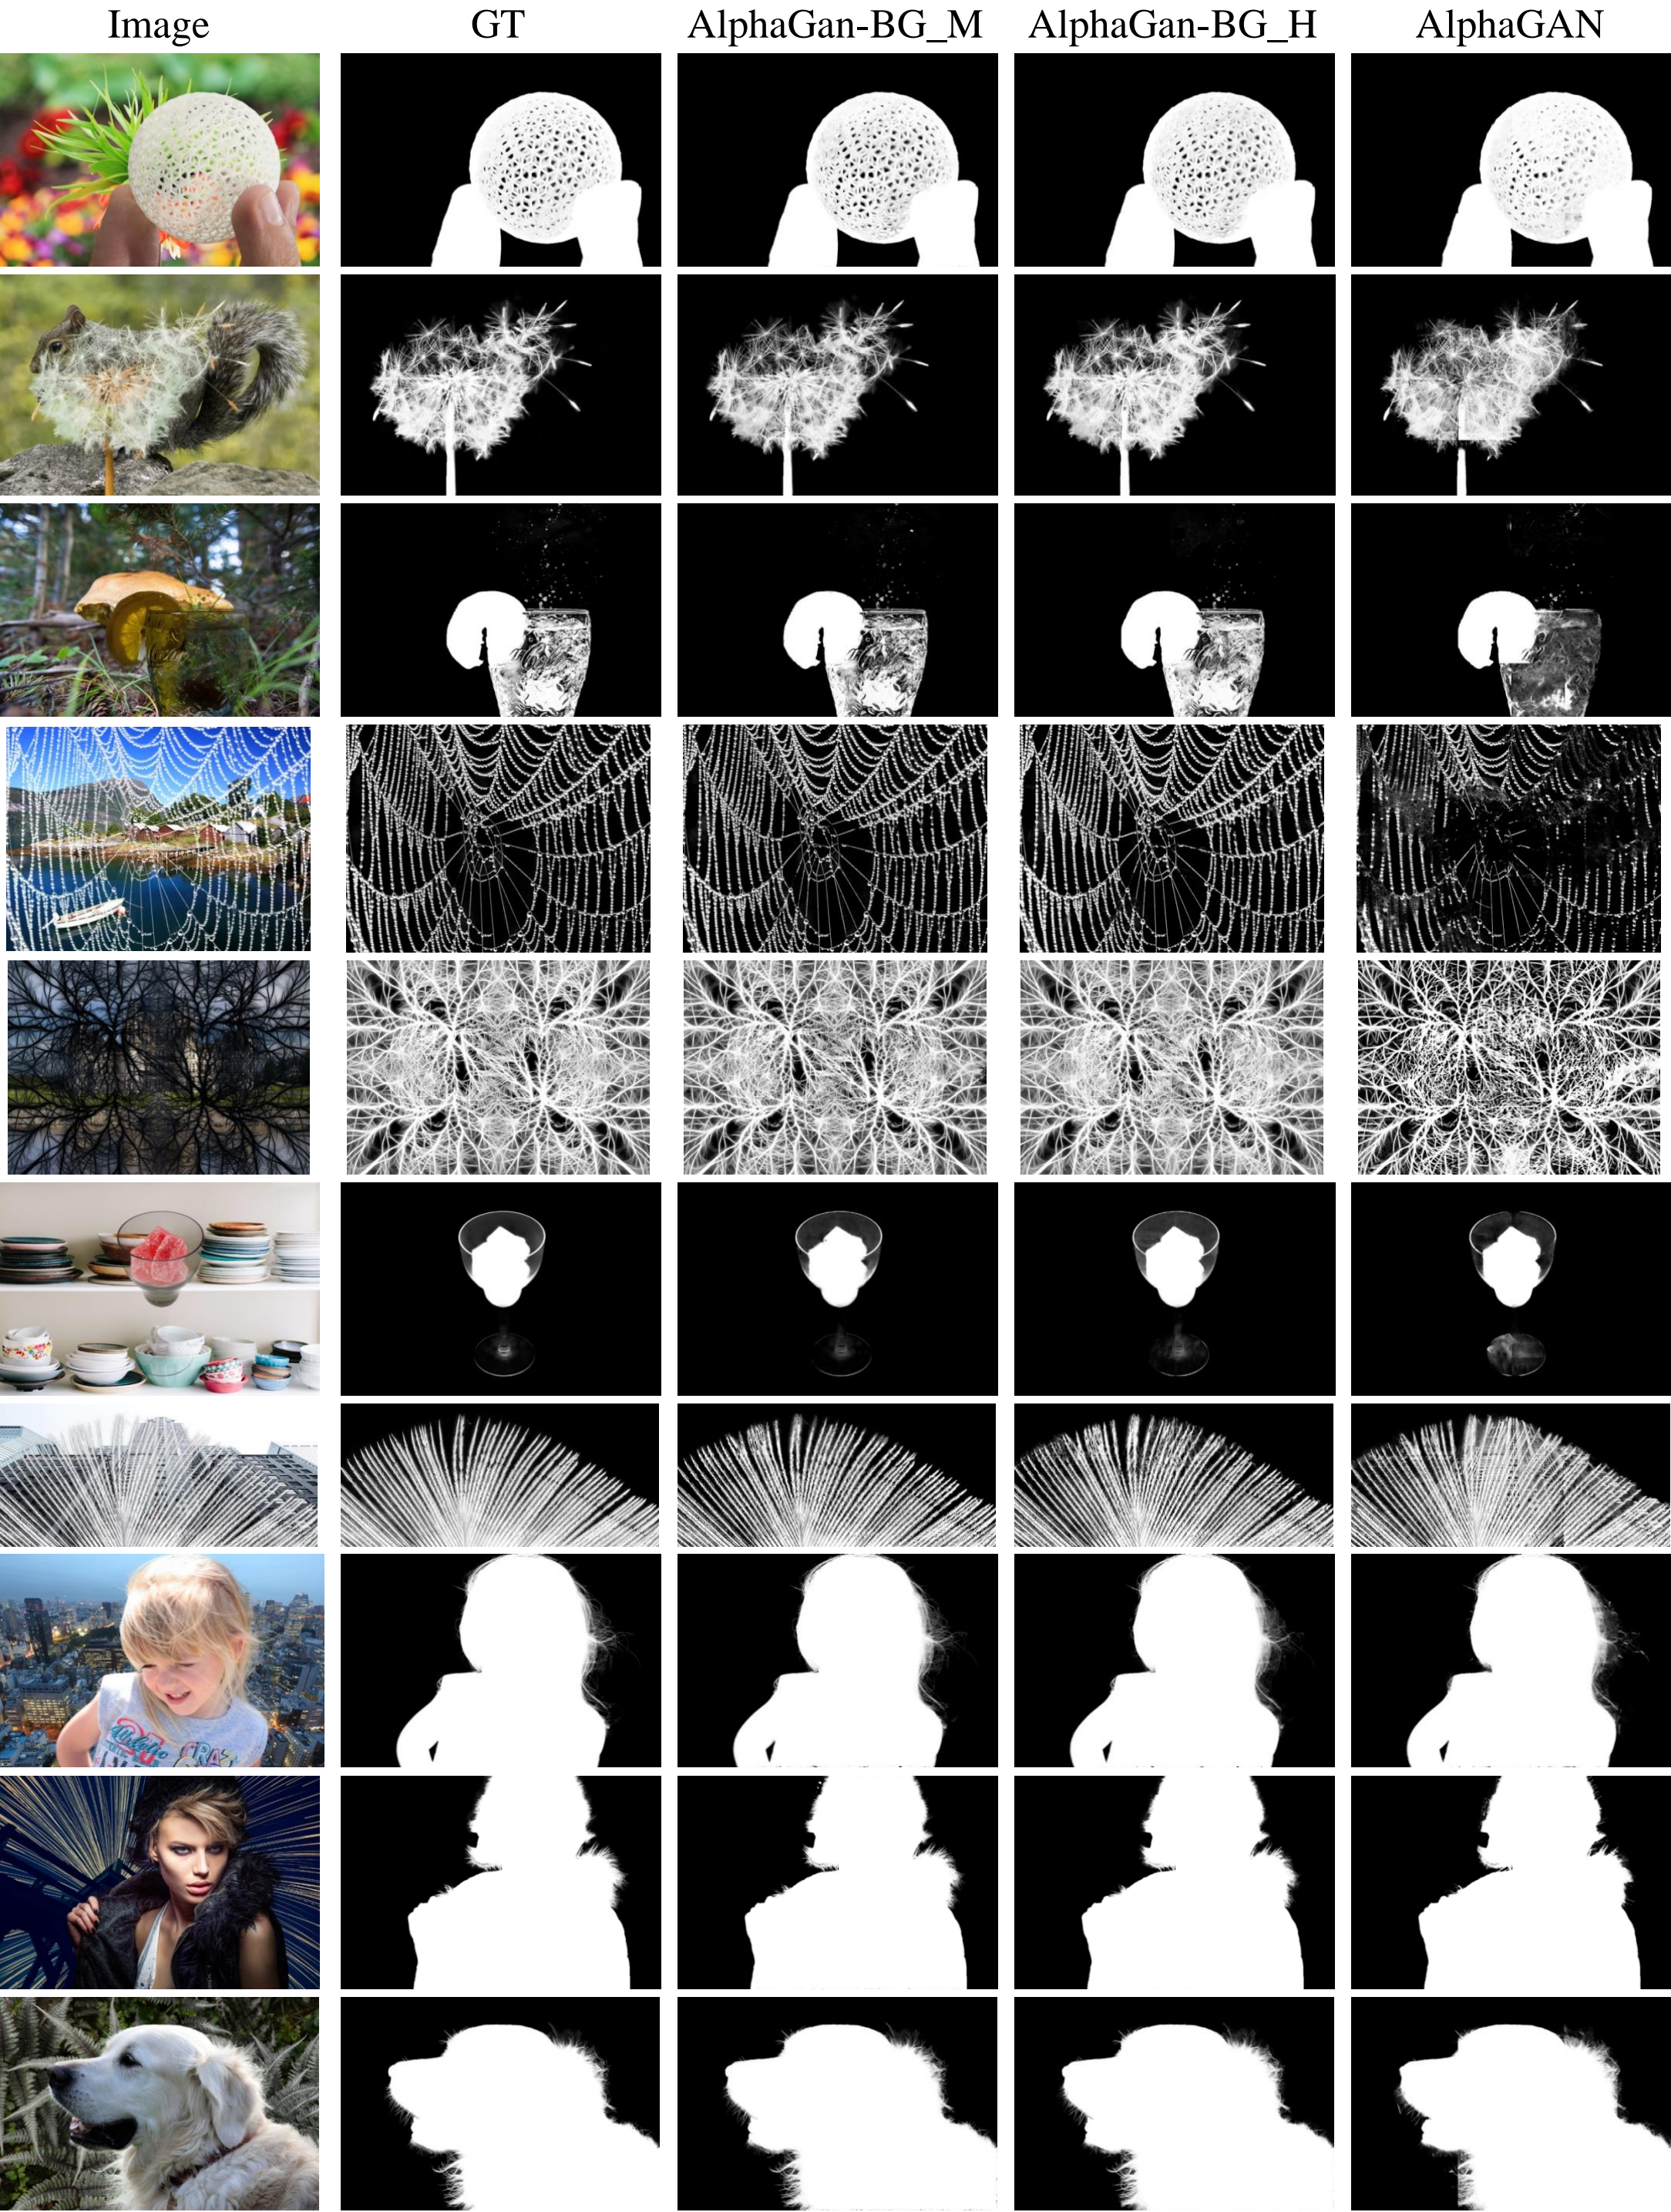   | 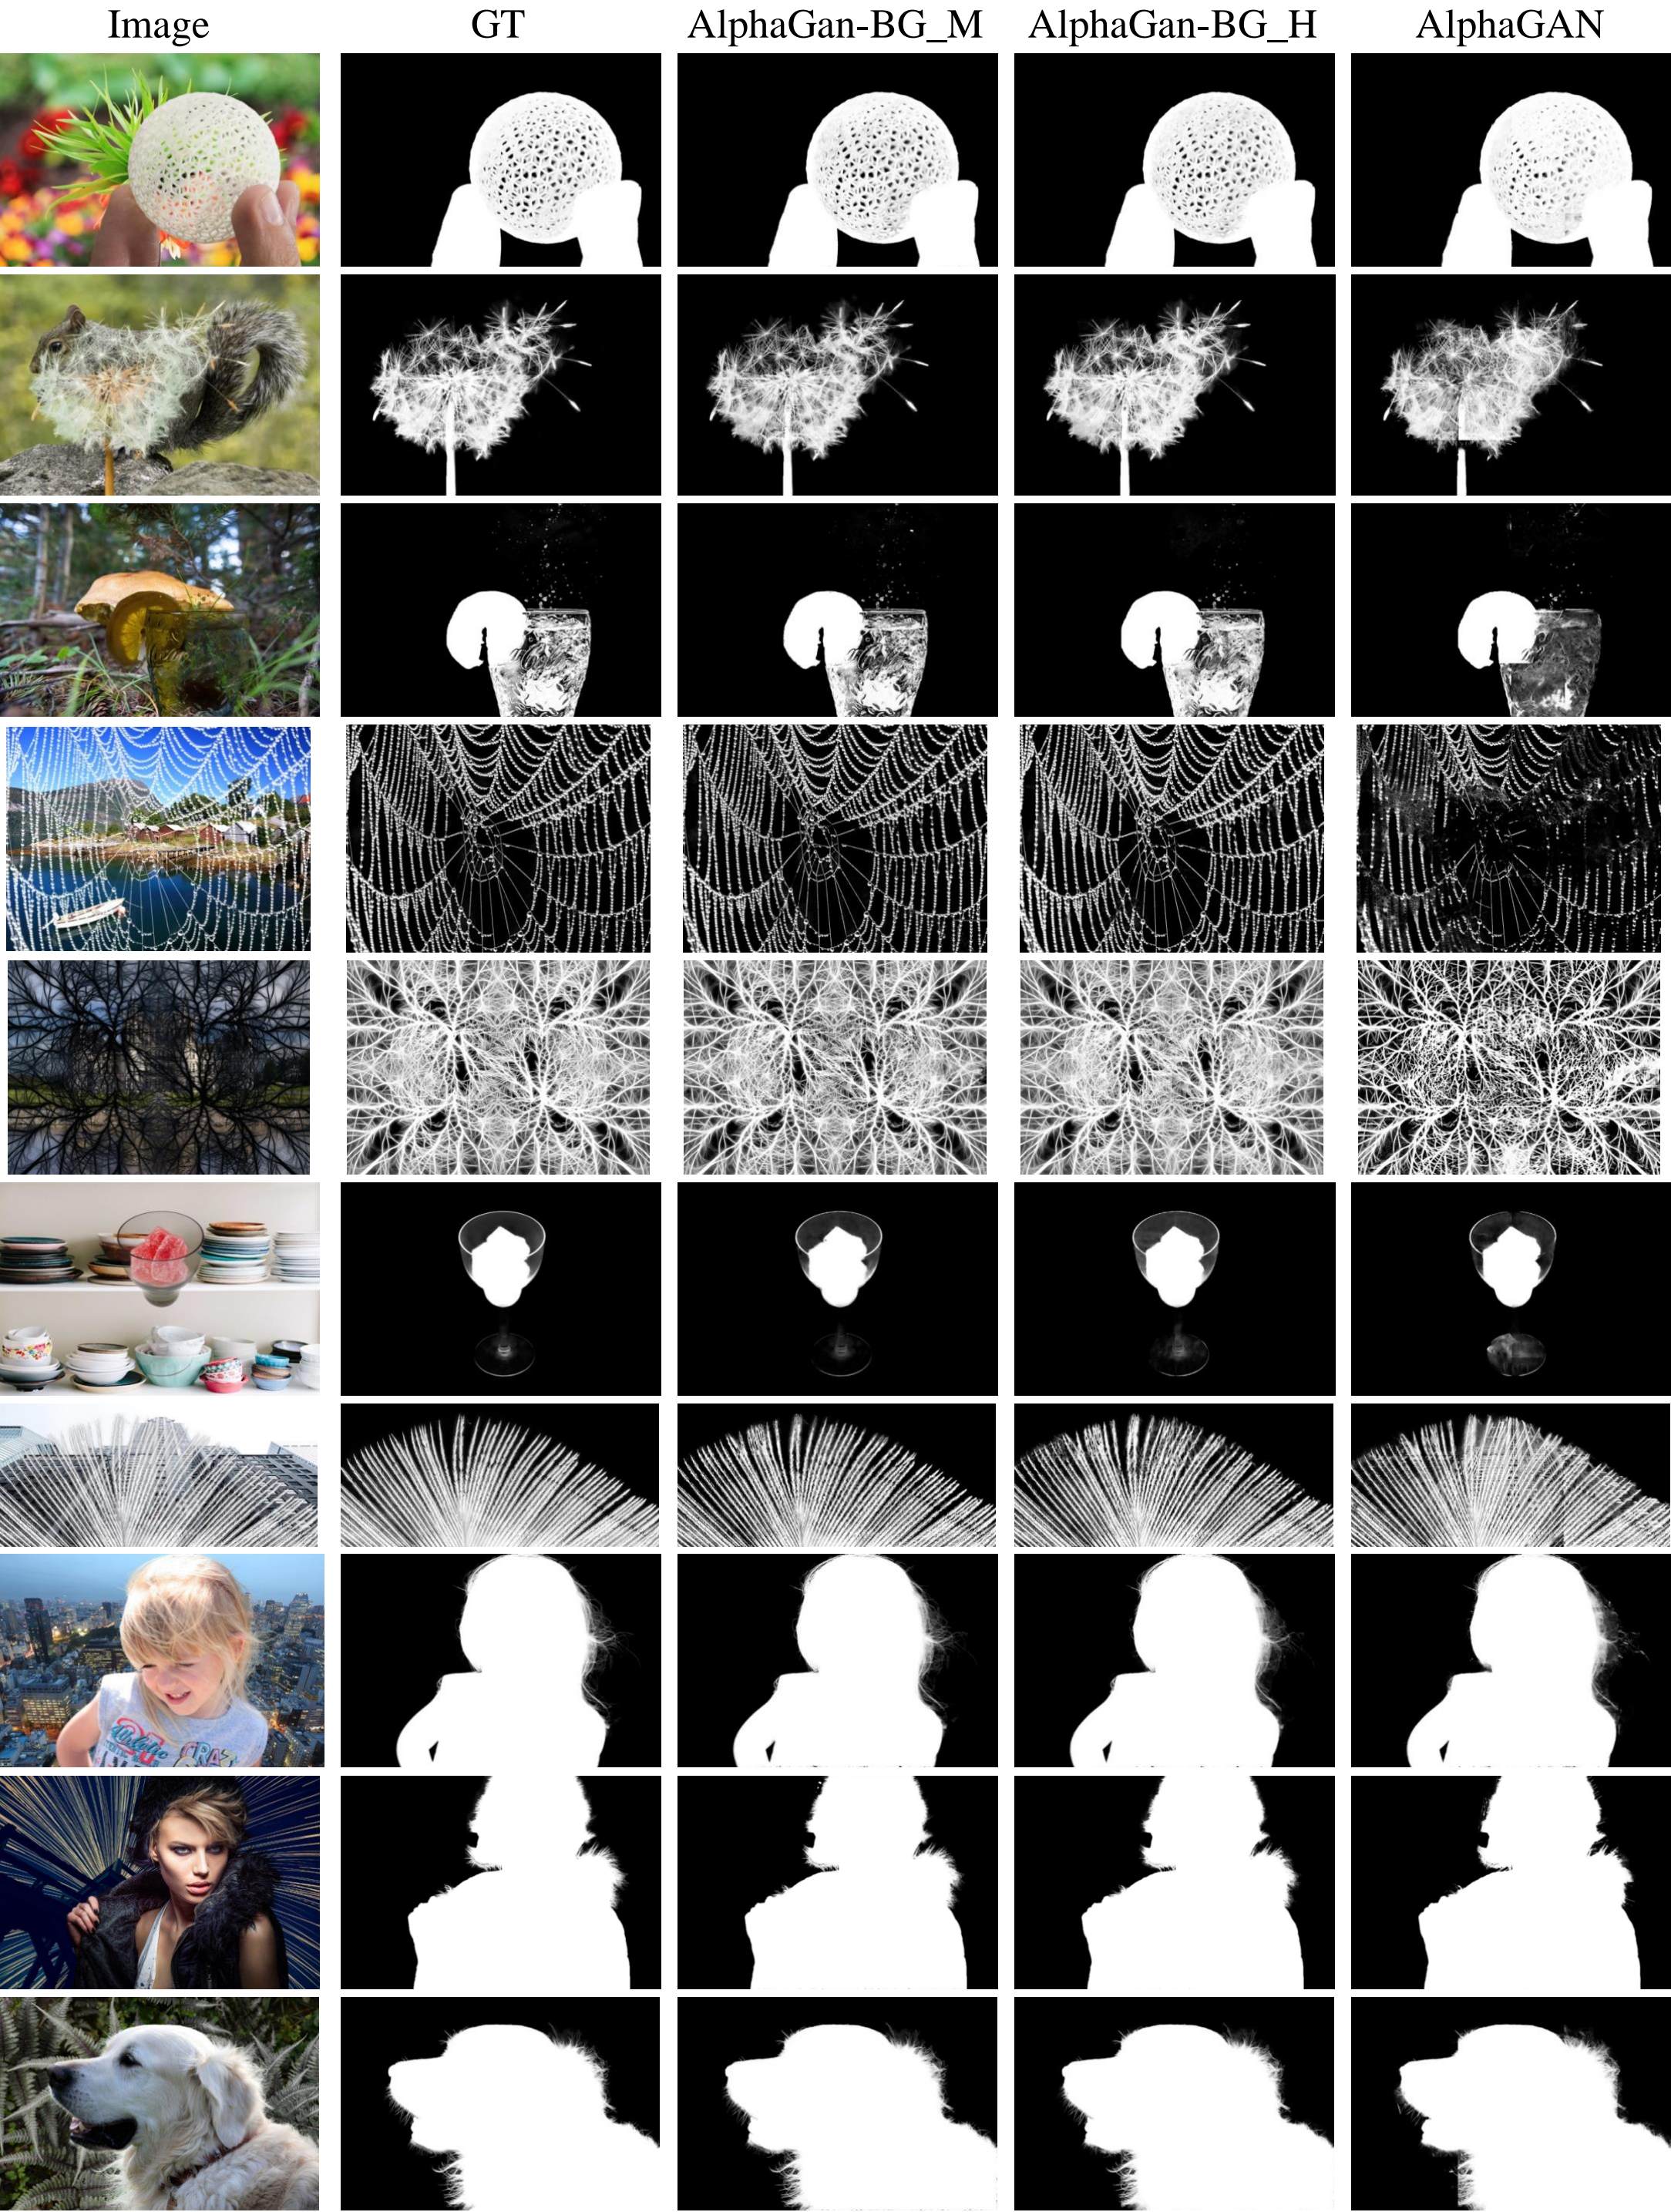   | 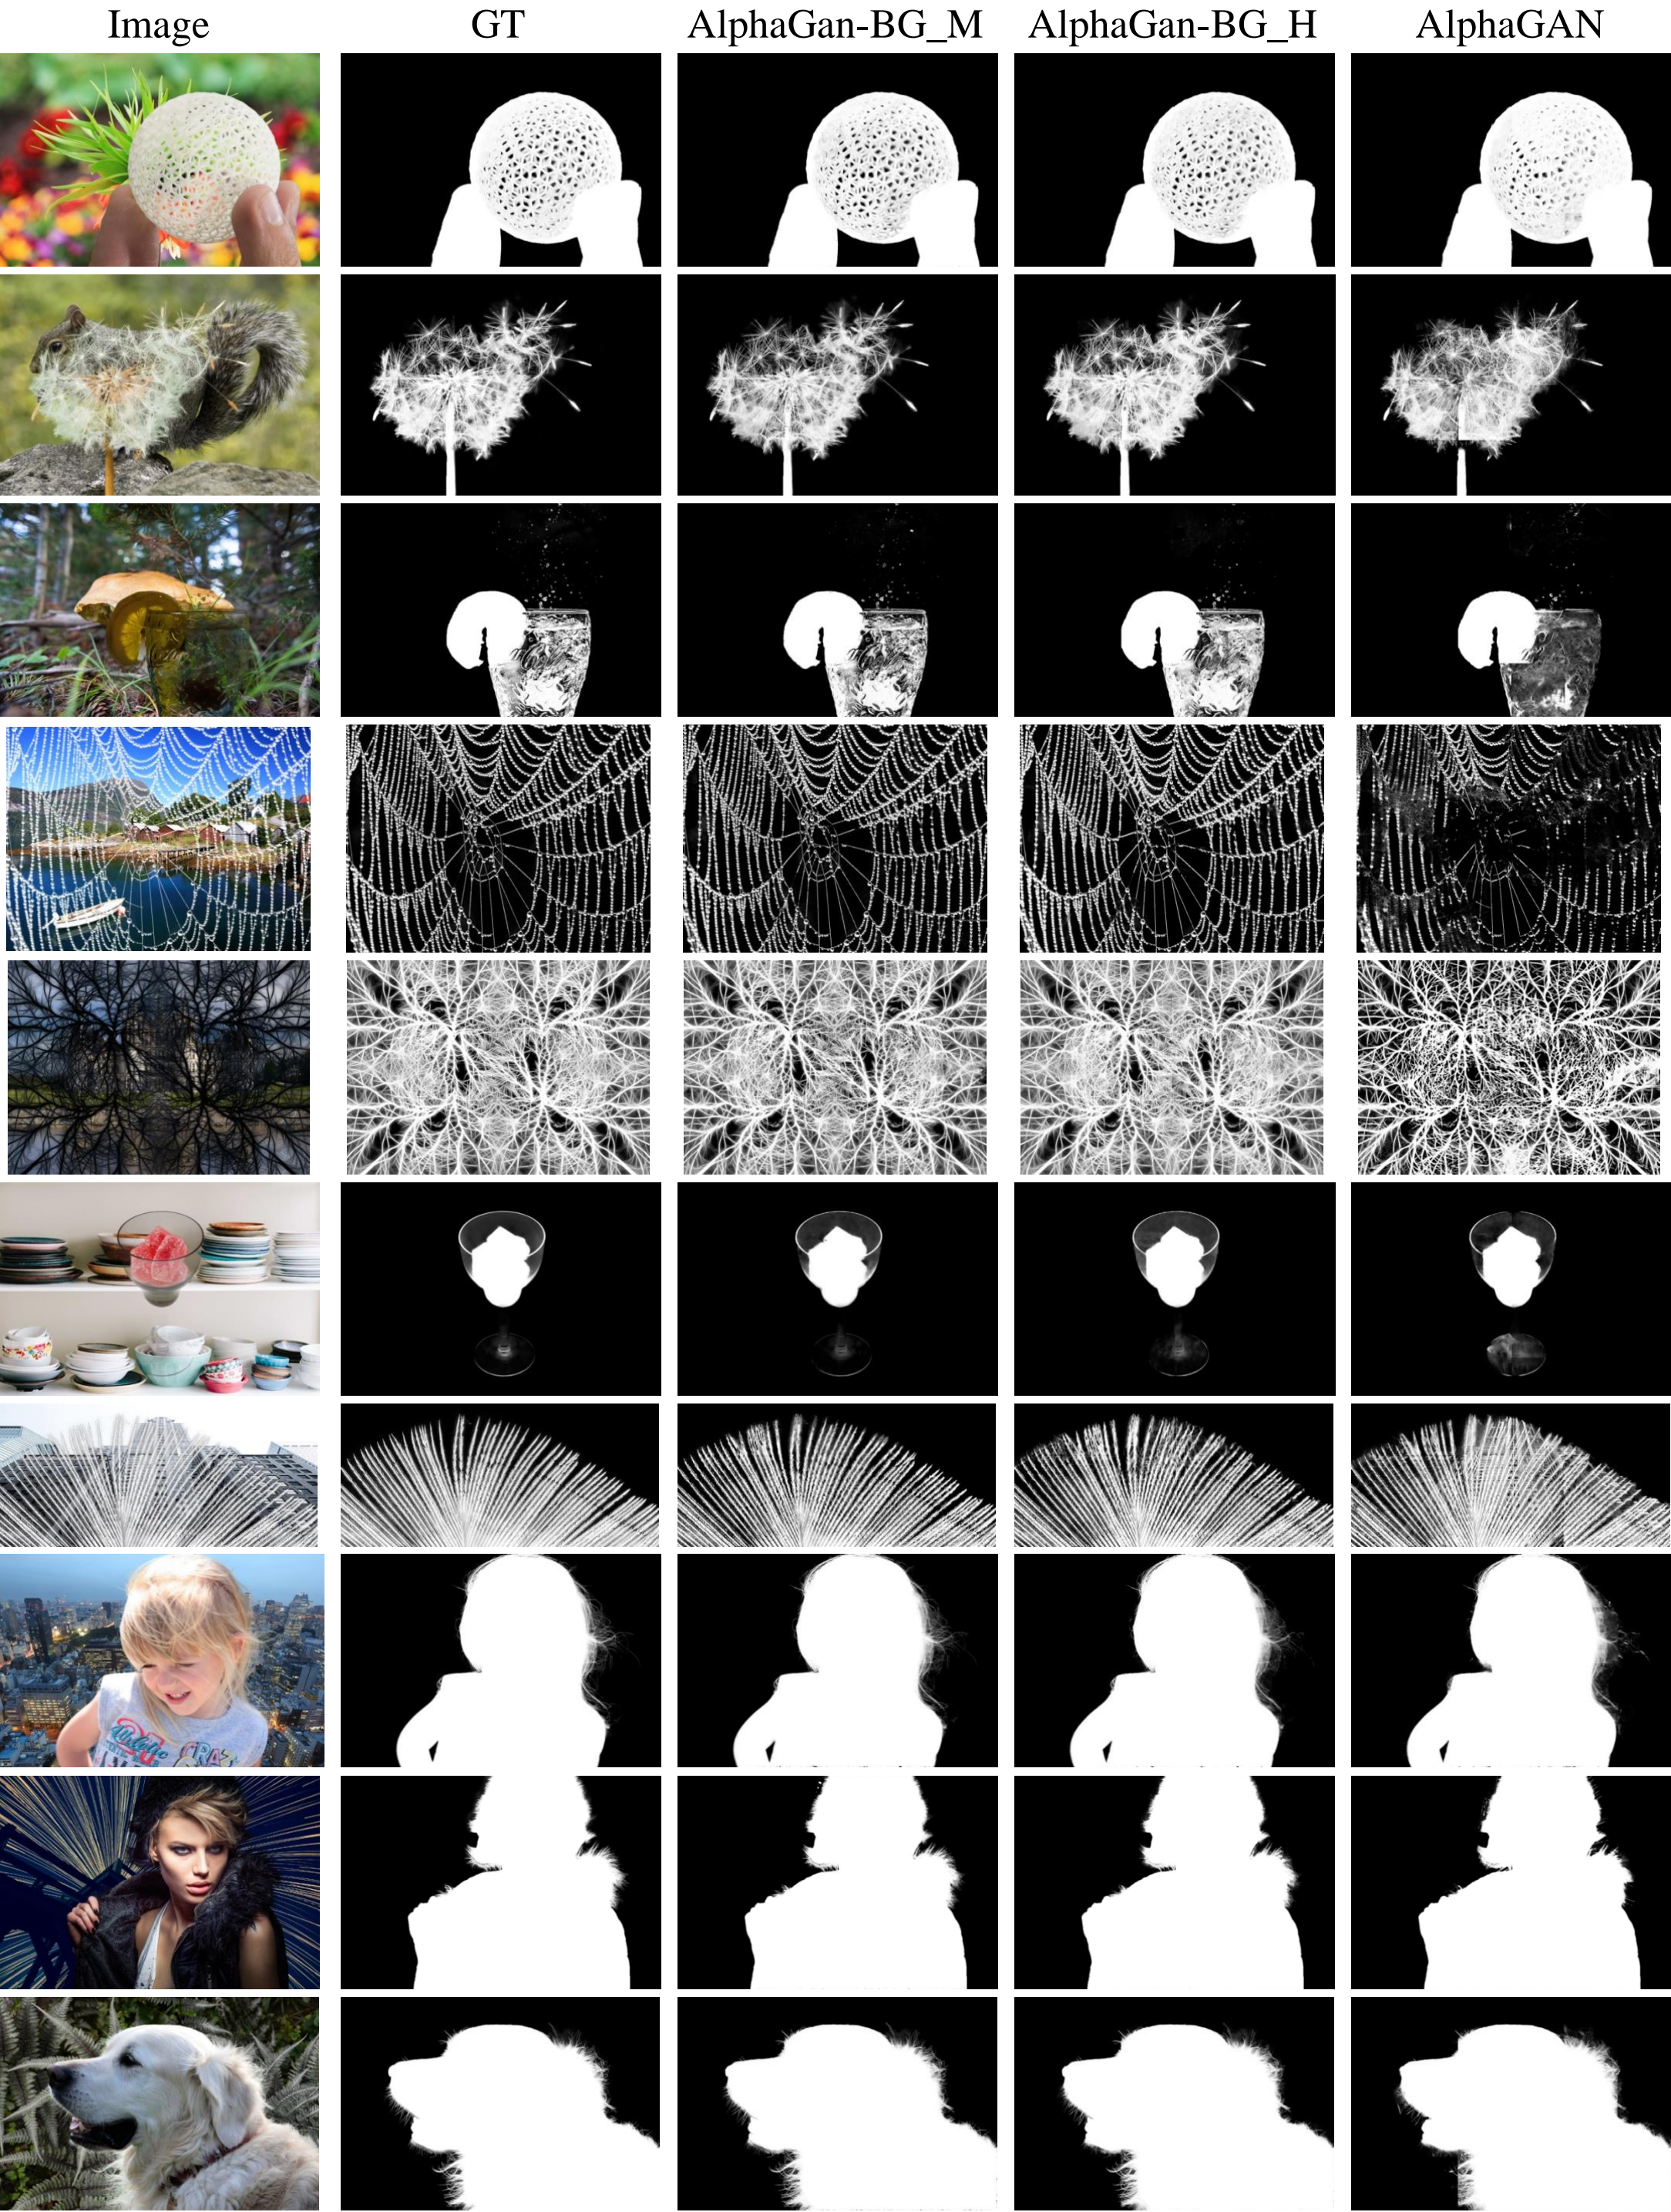   | 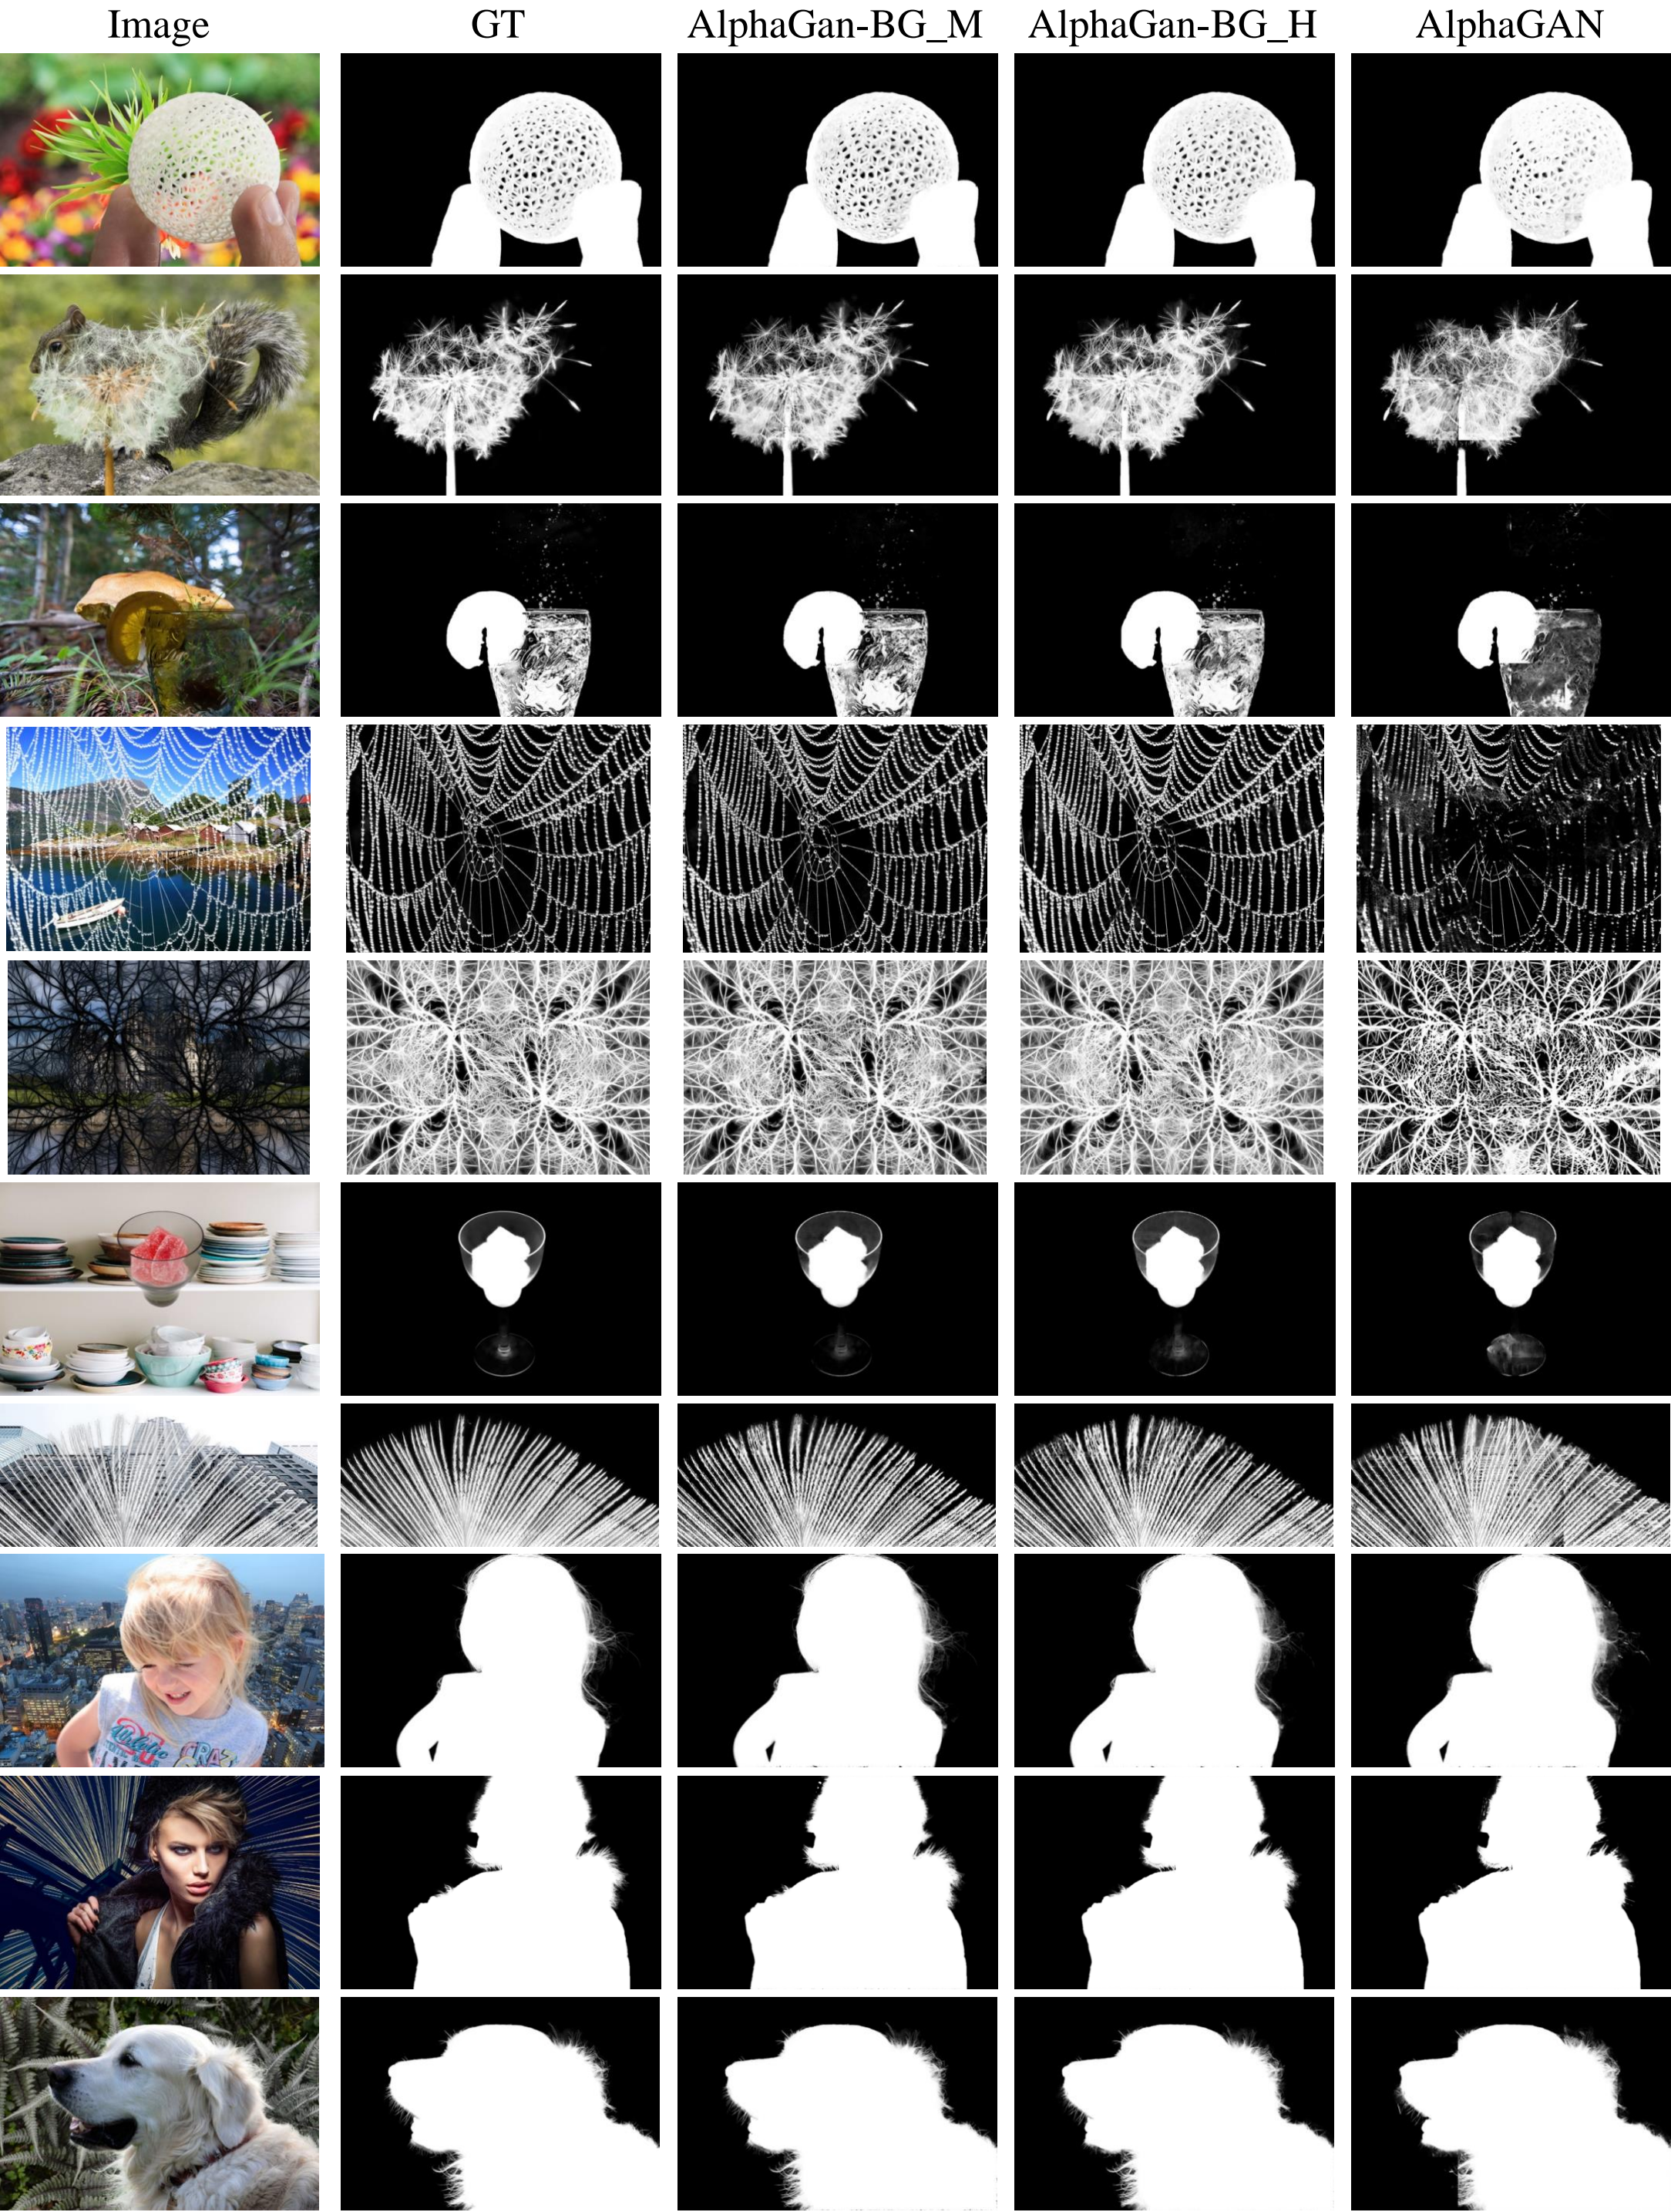   | 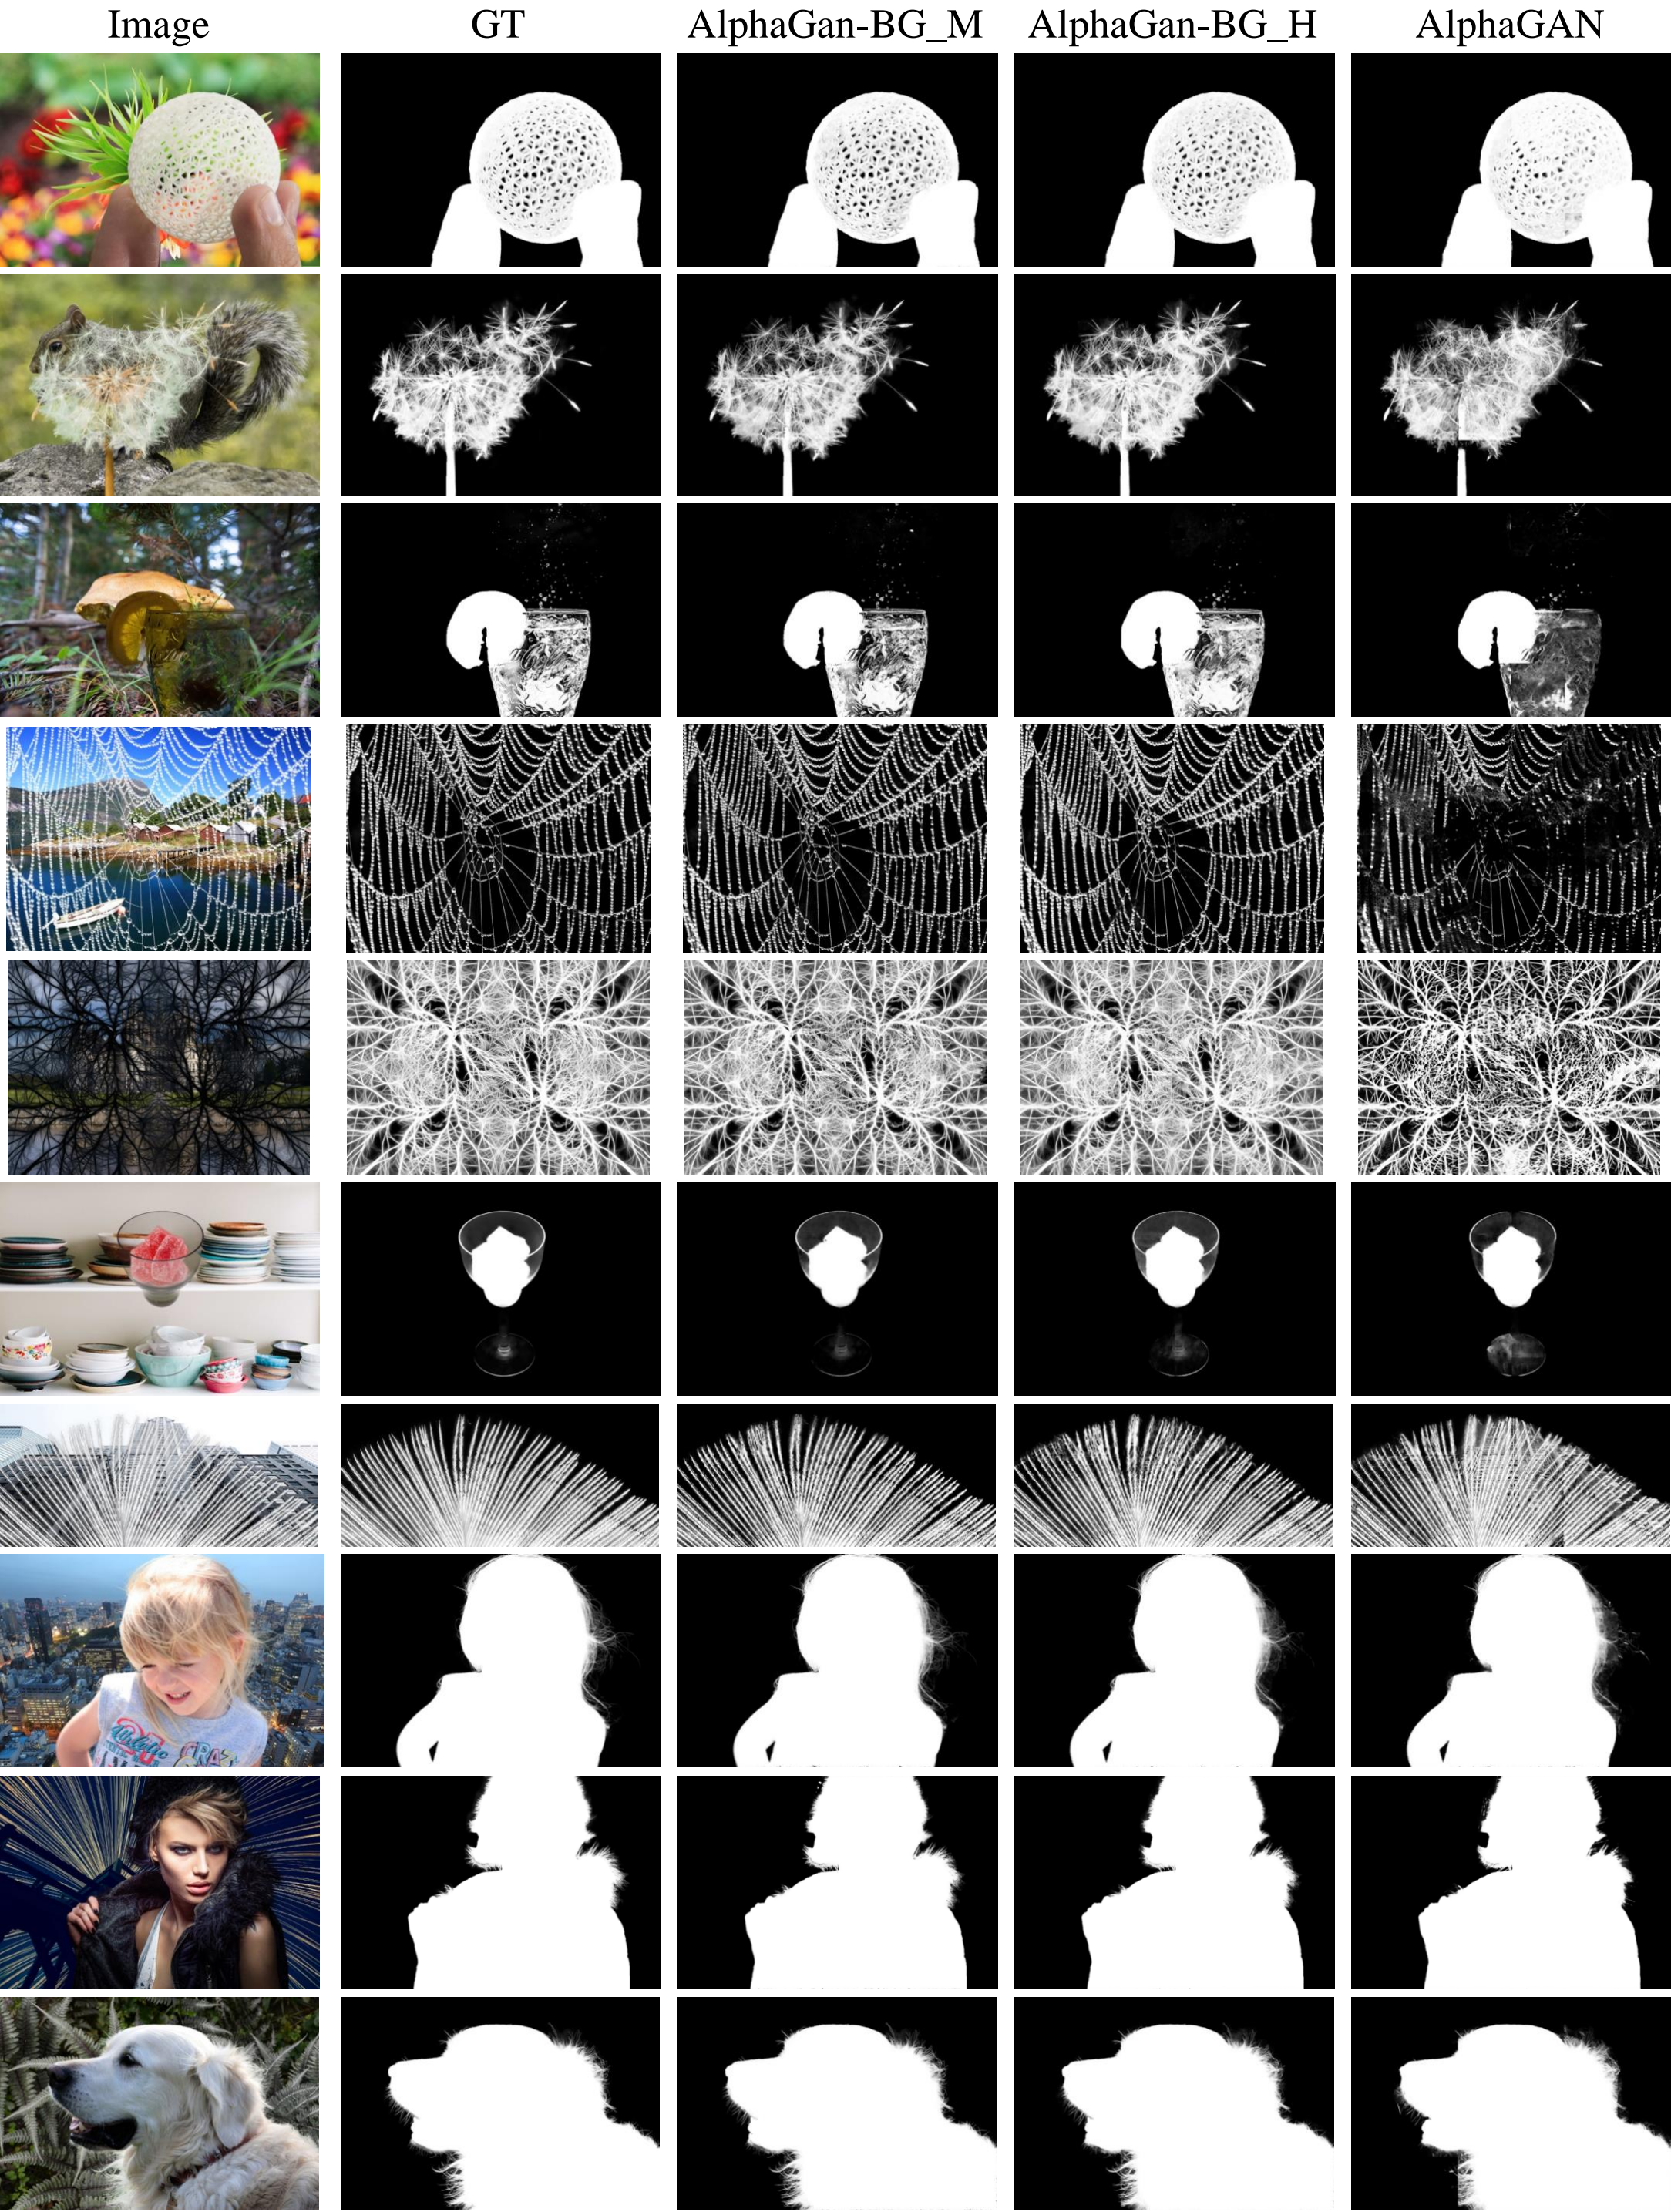   |
| 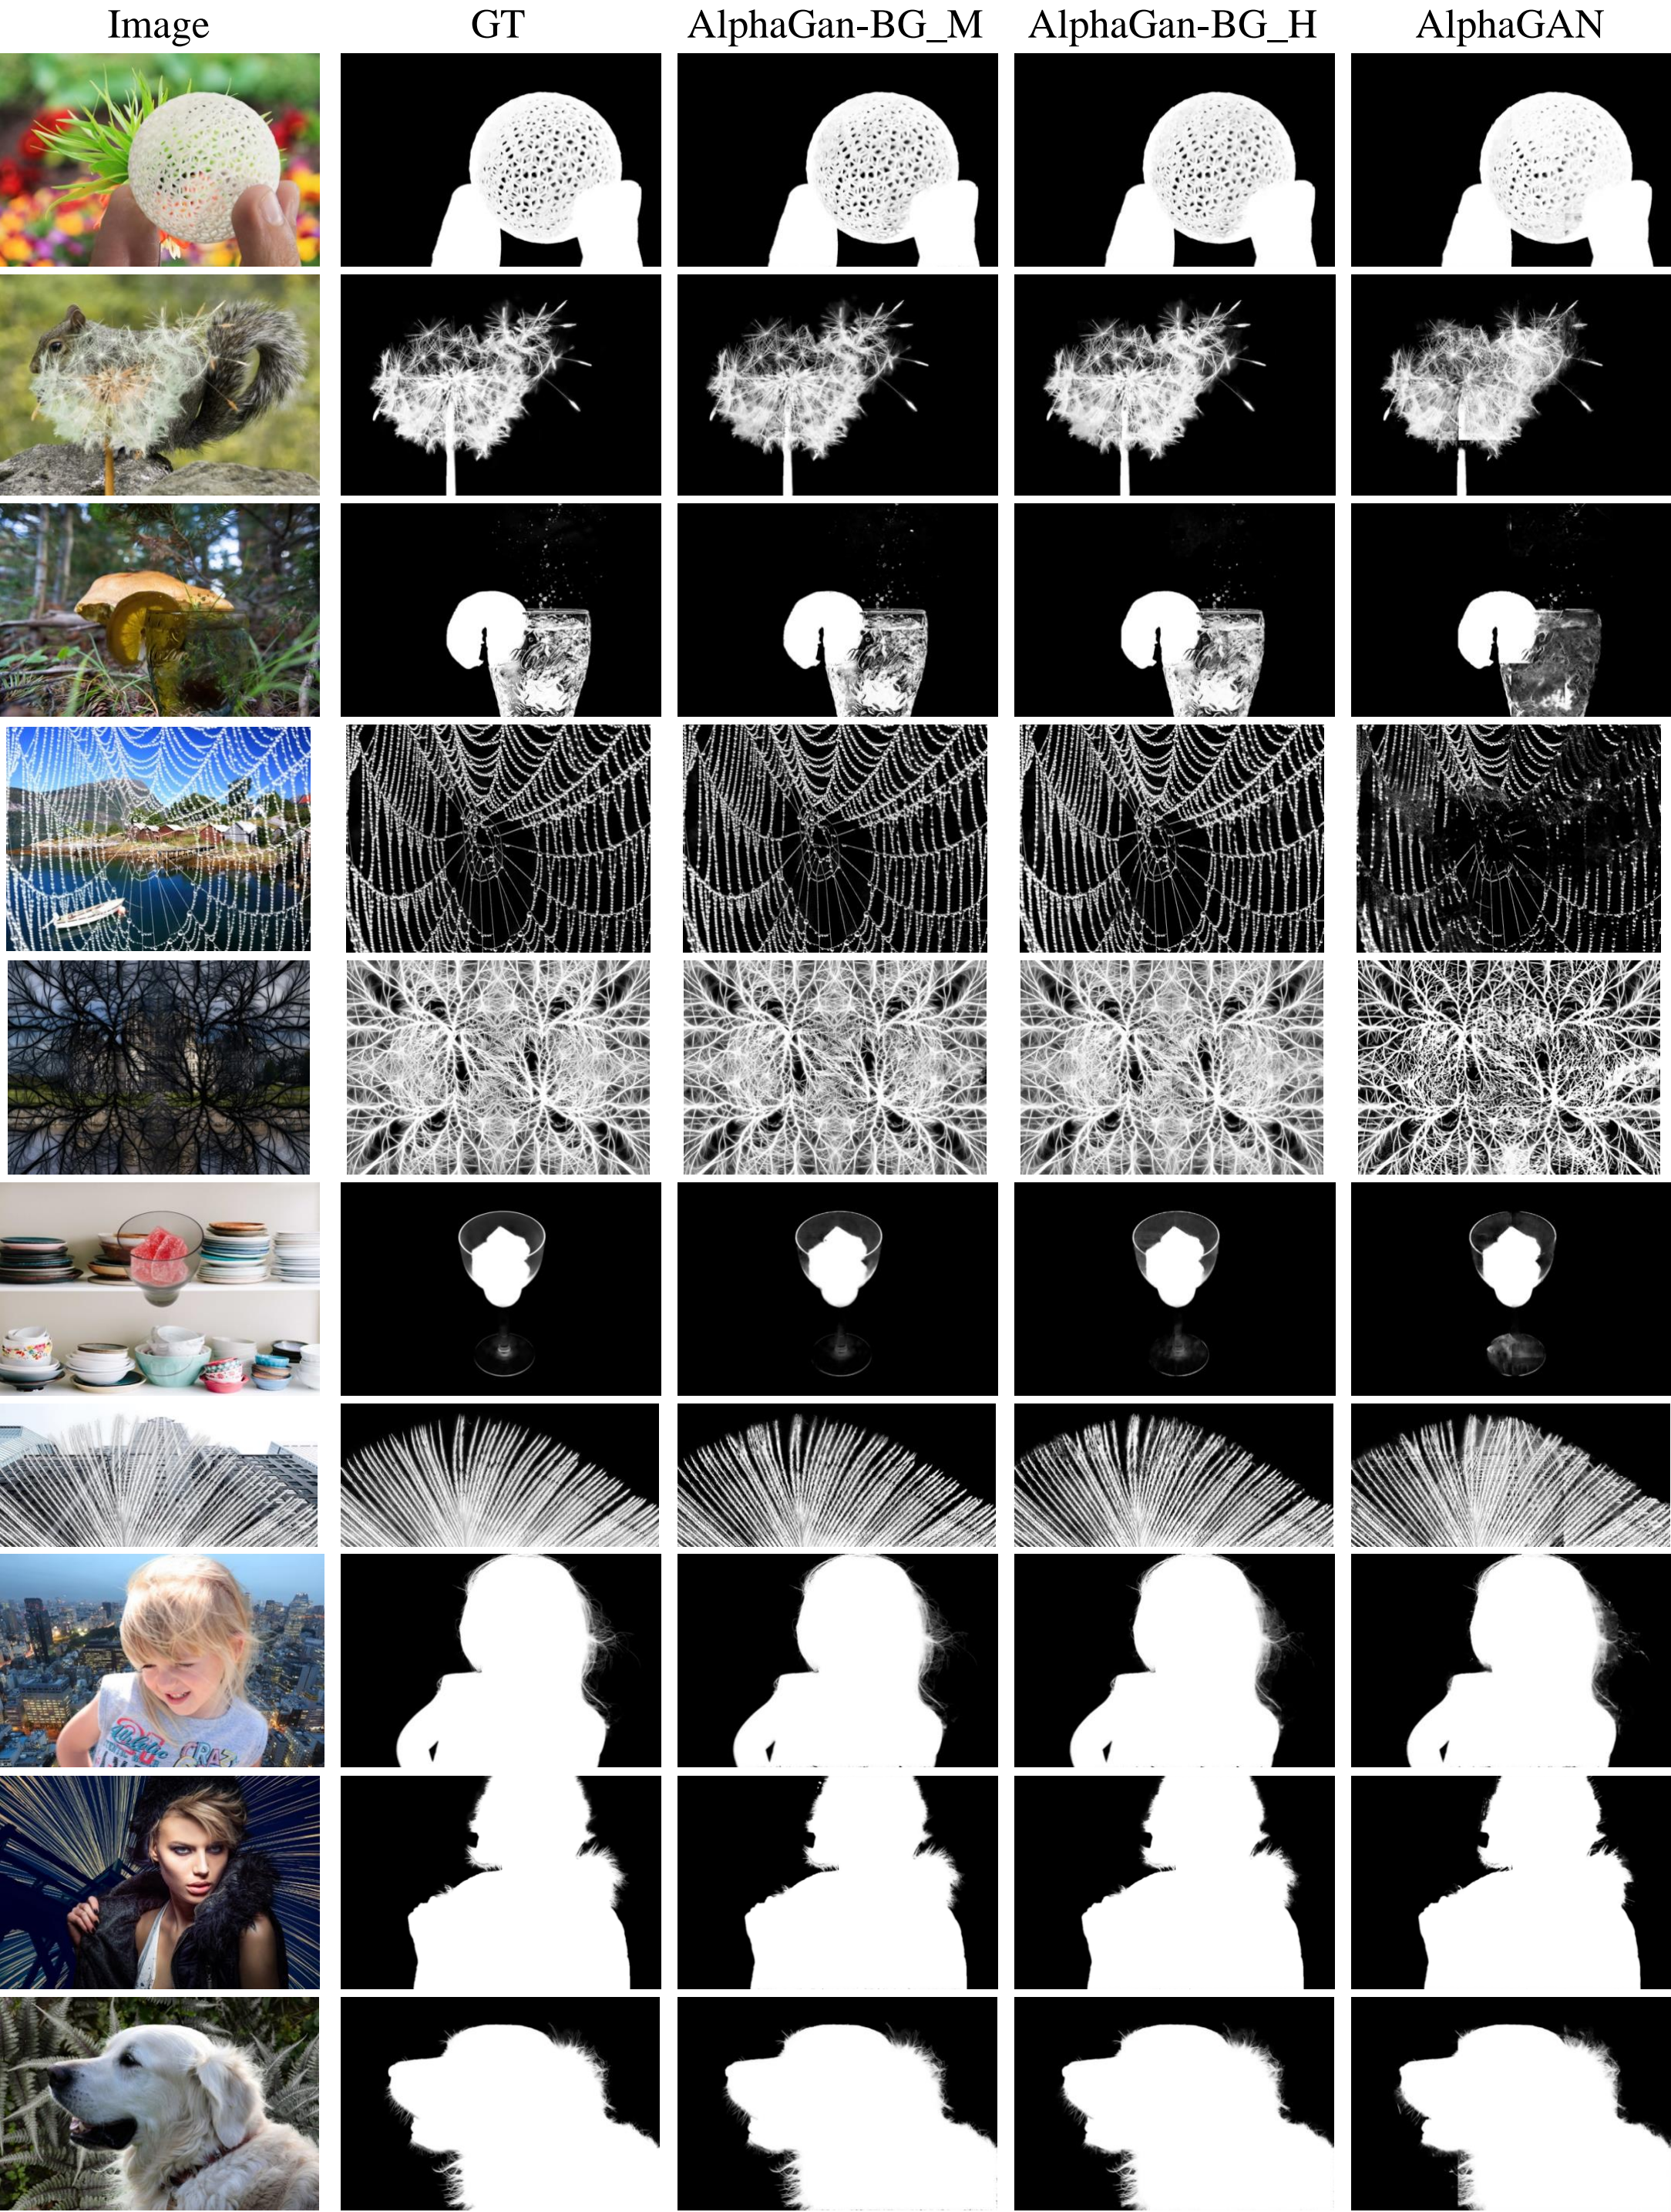   | 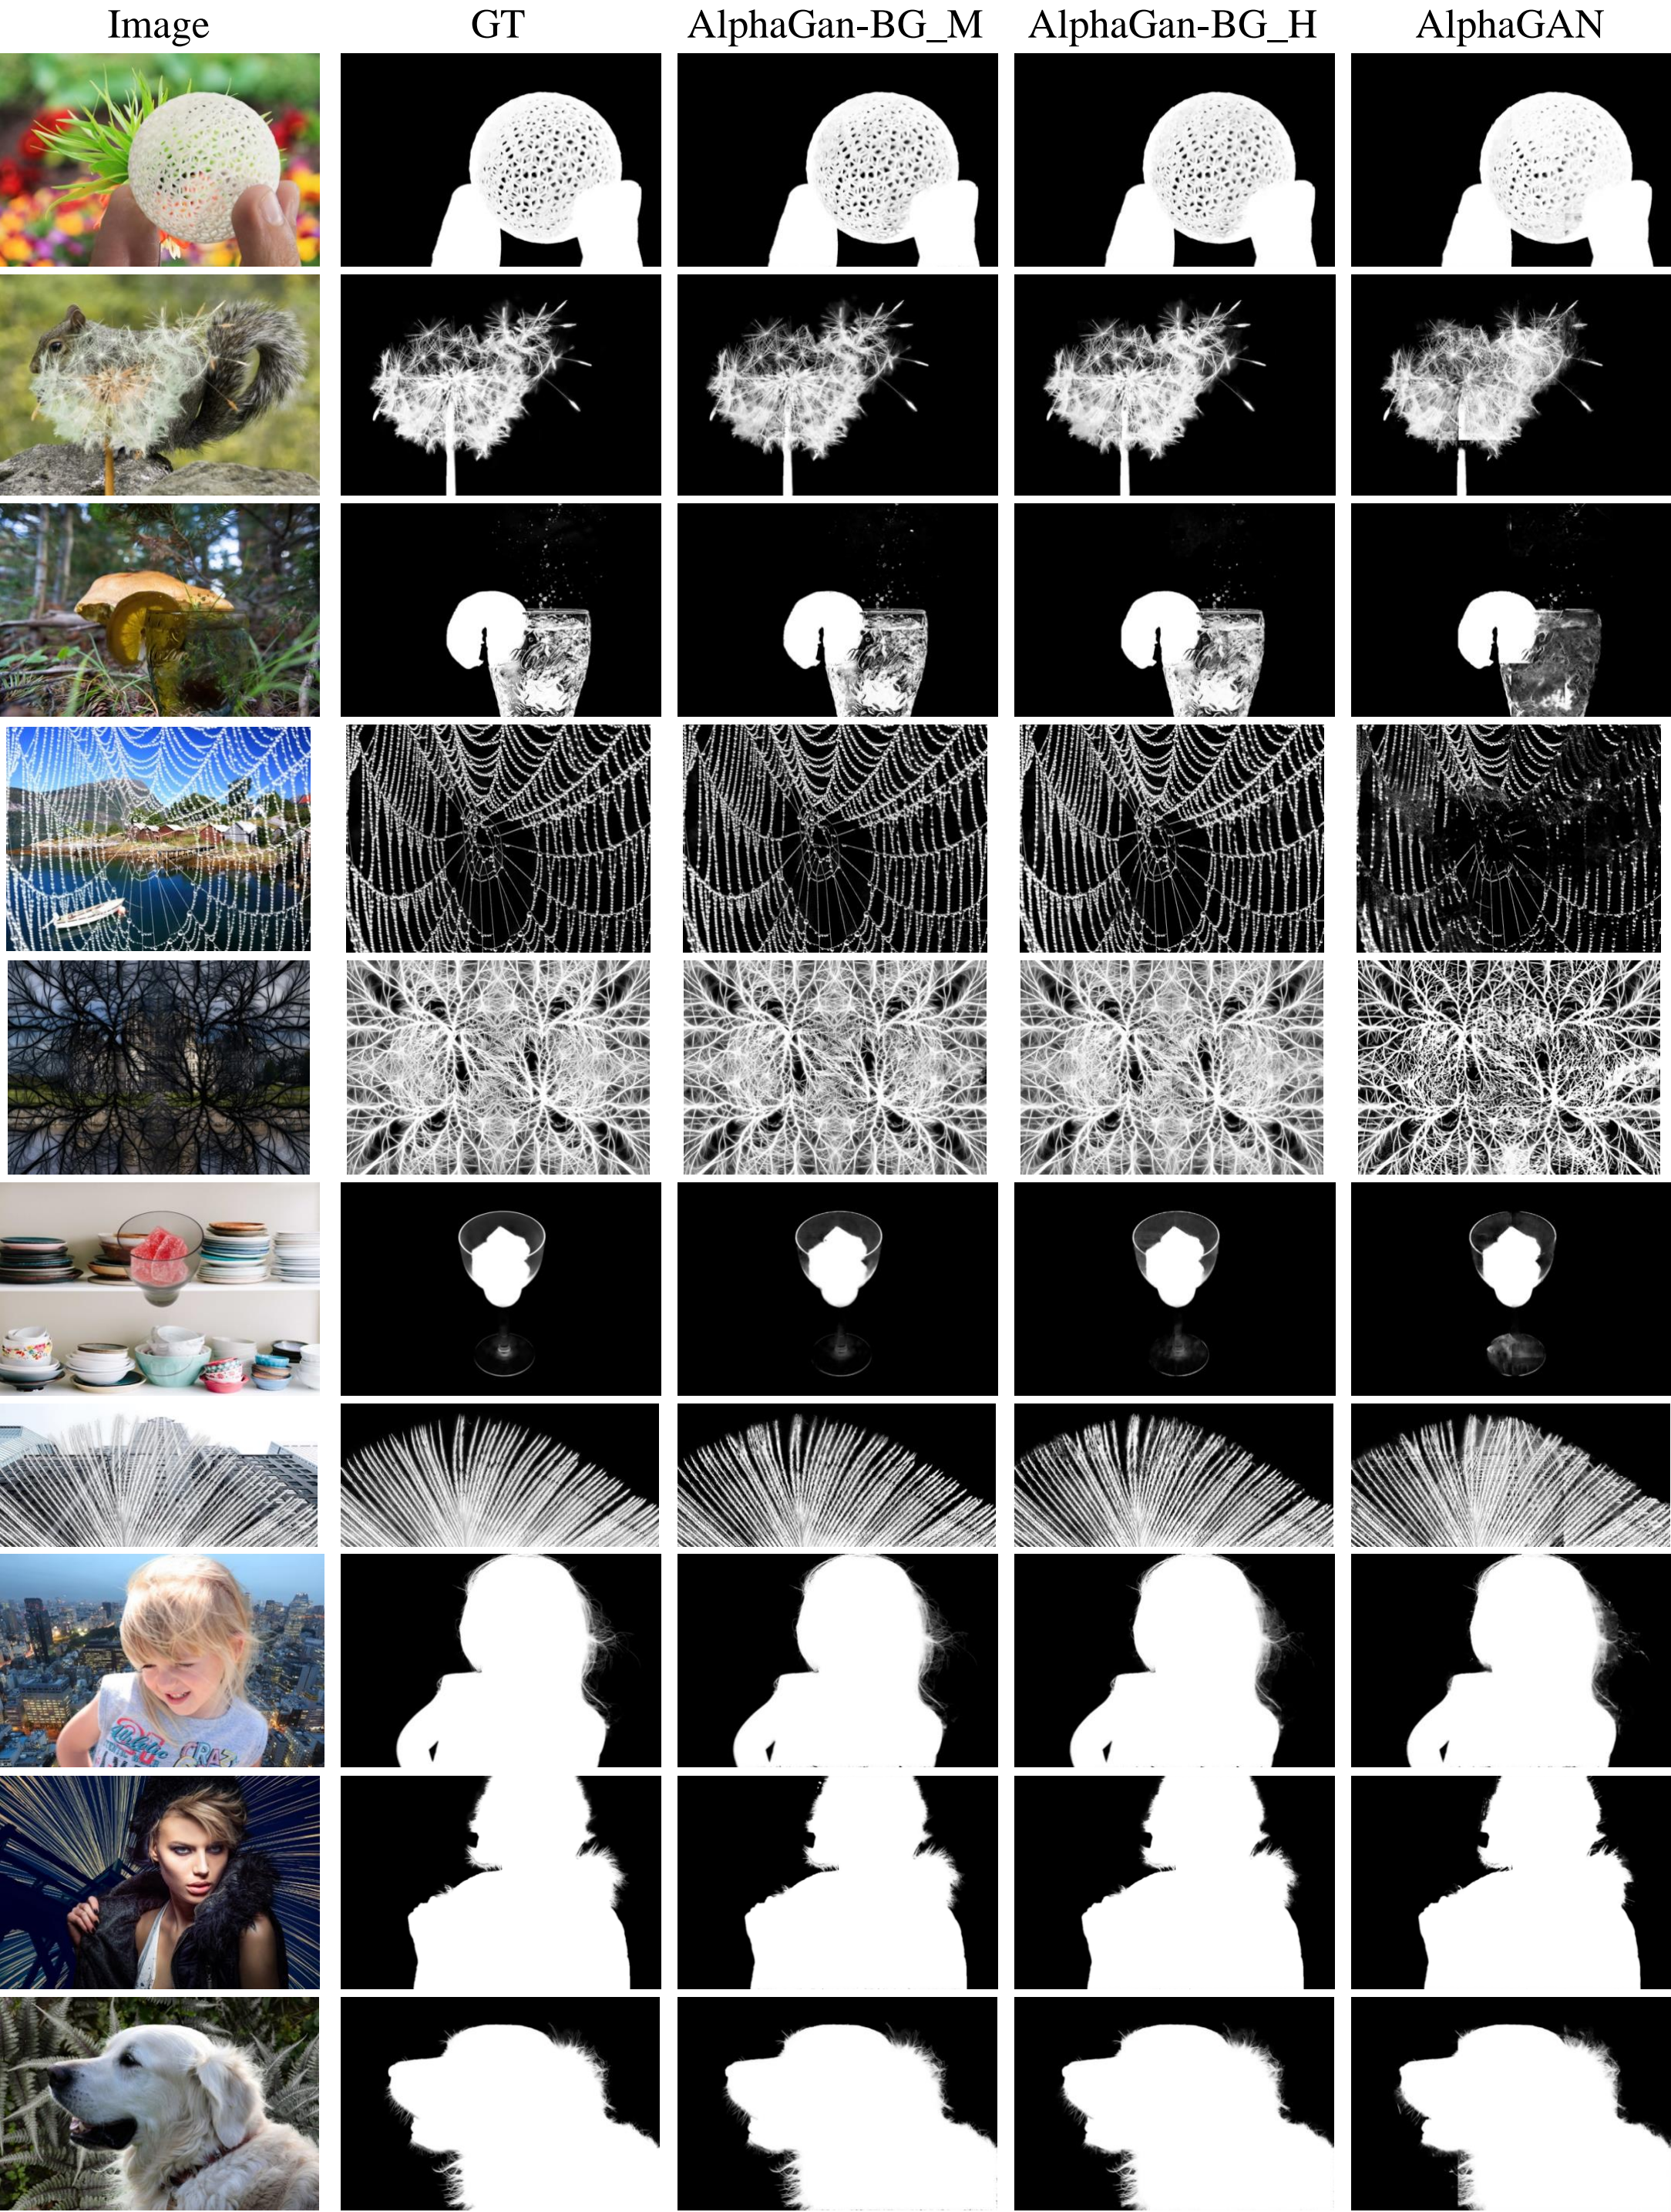   | 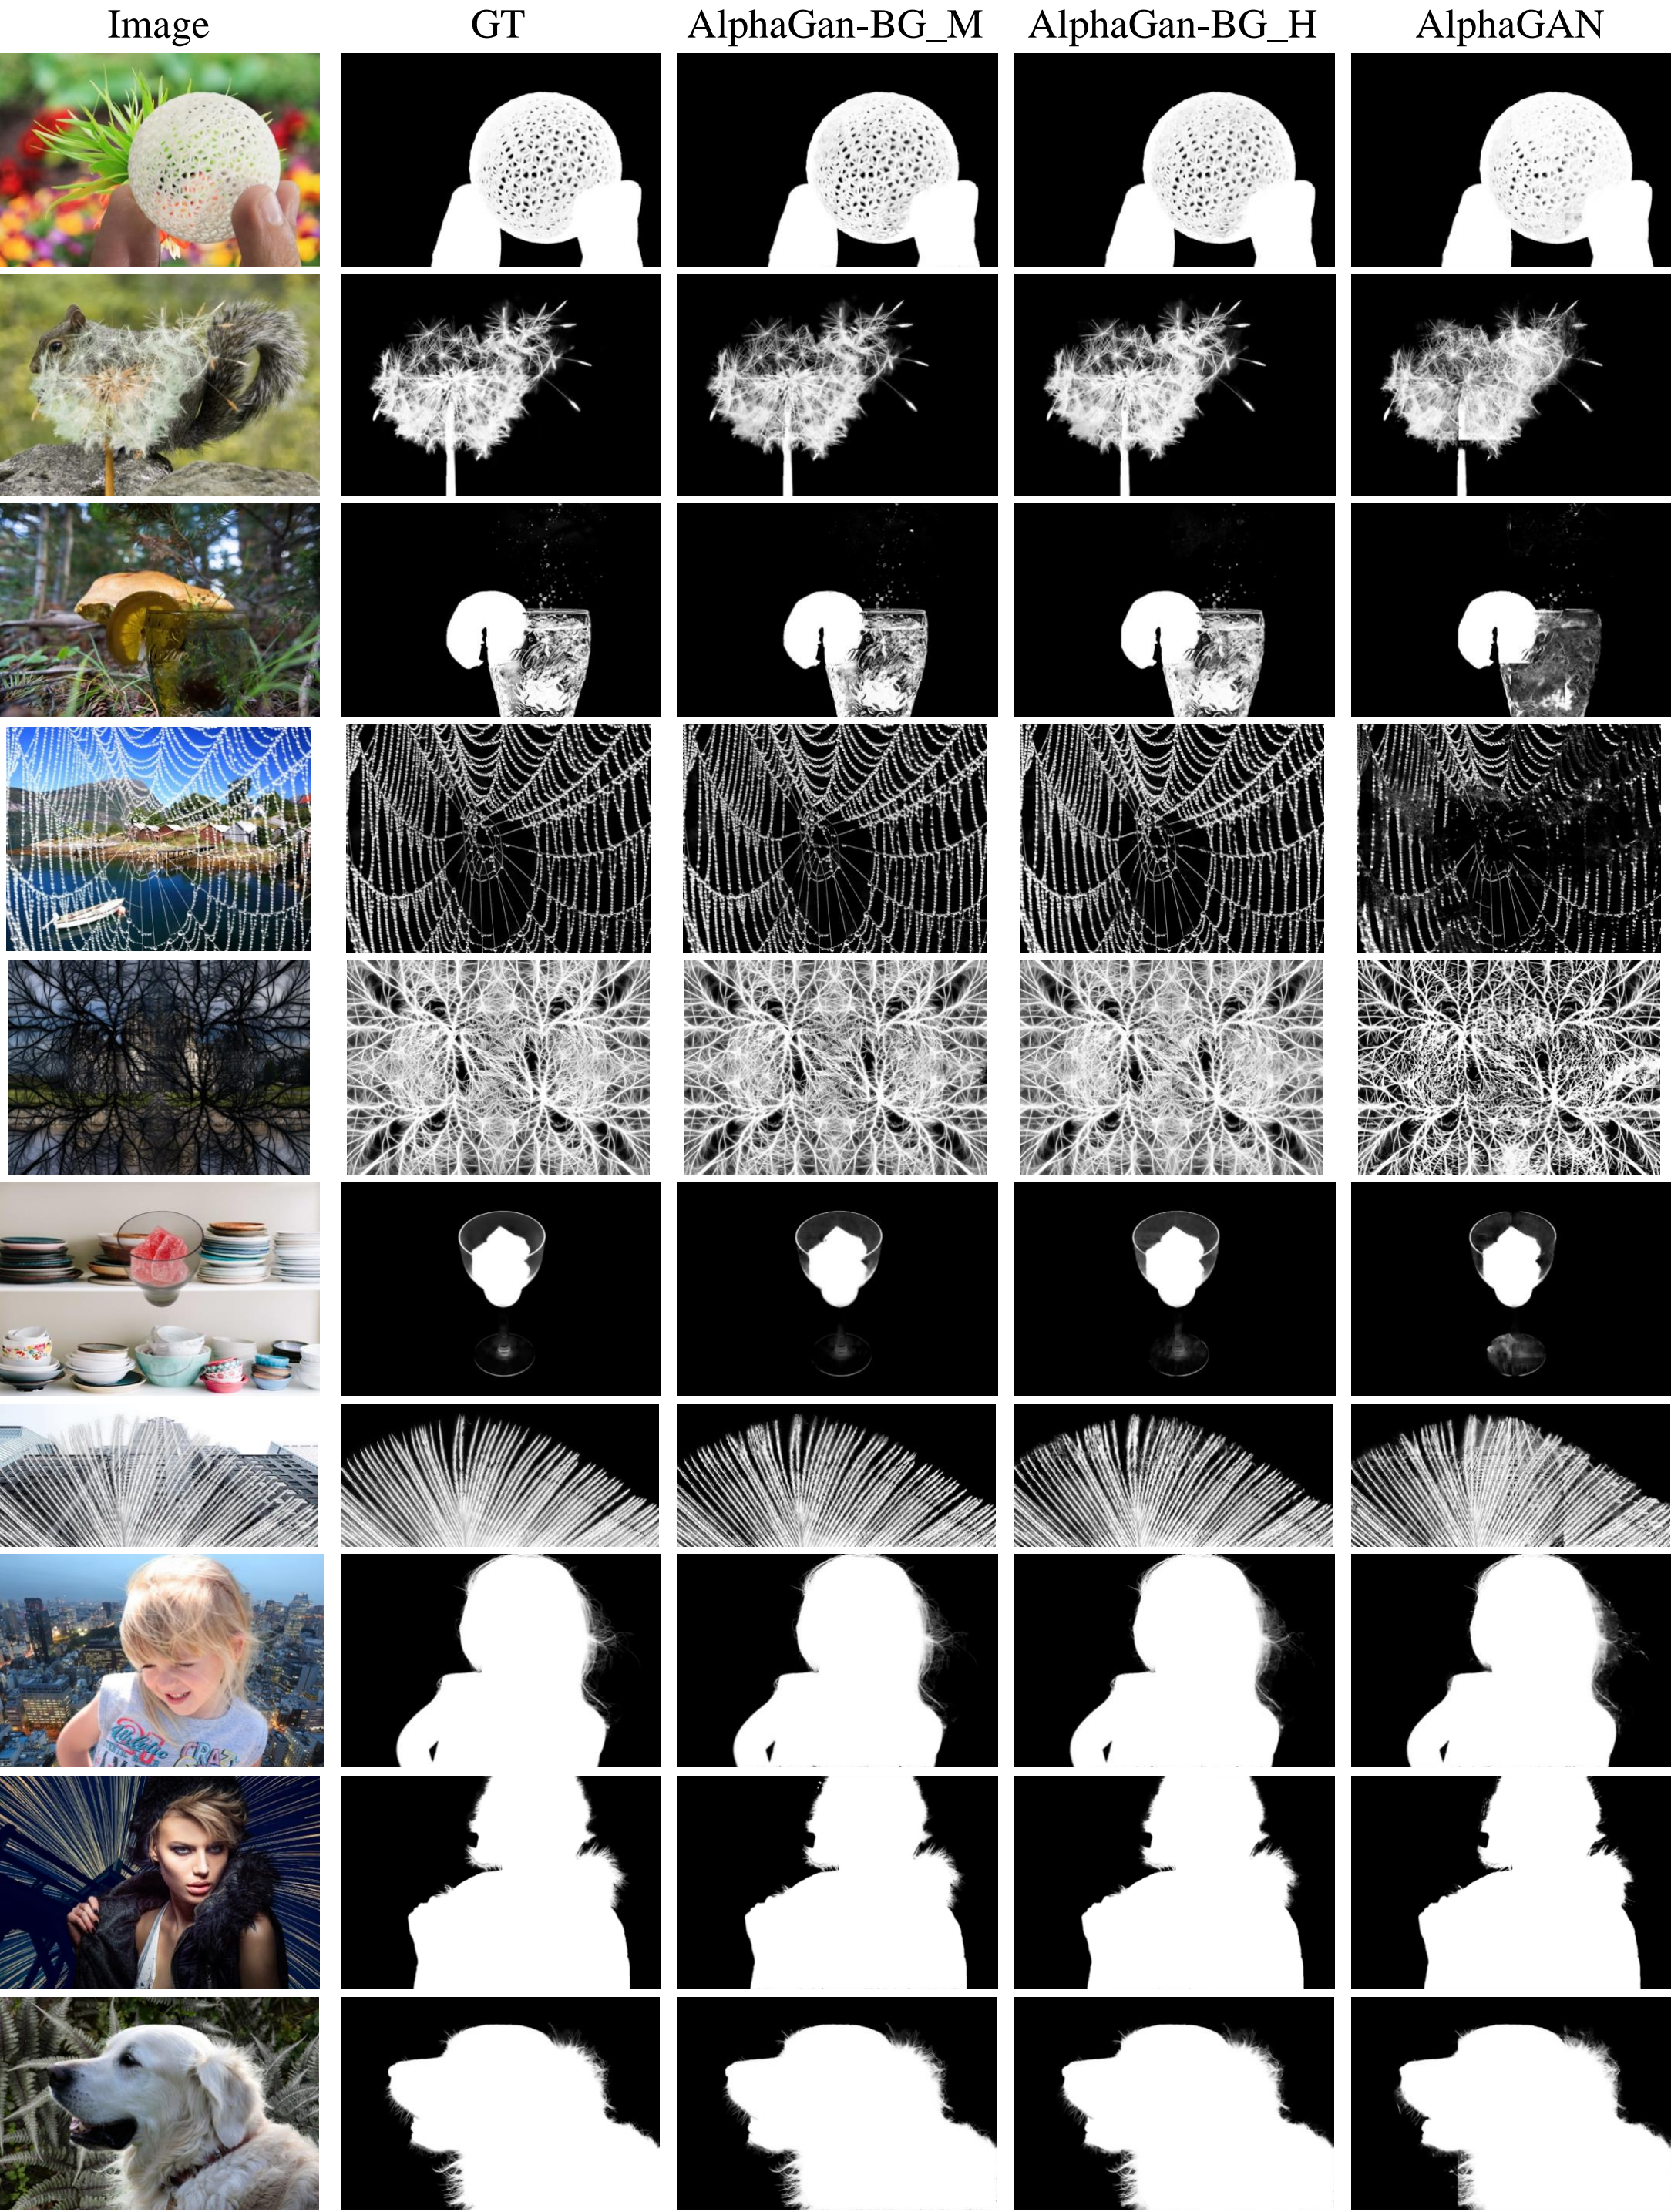   | 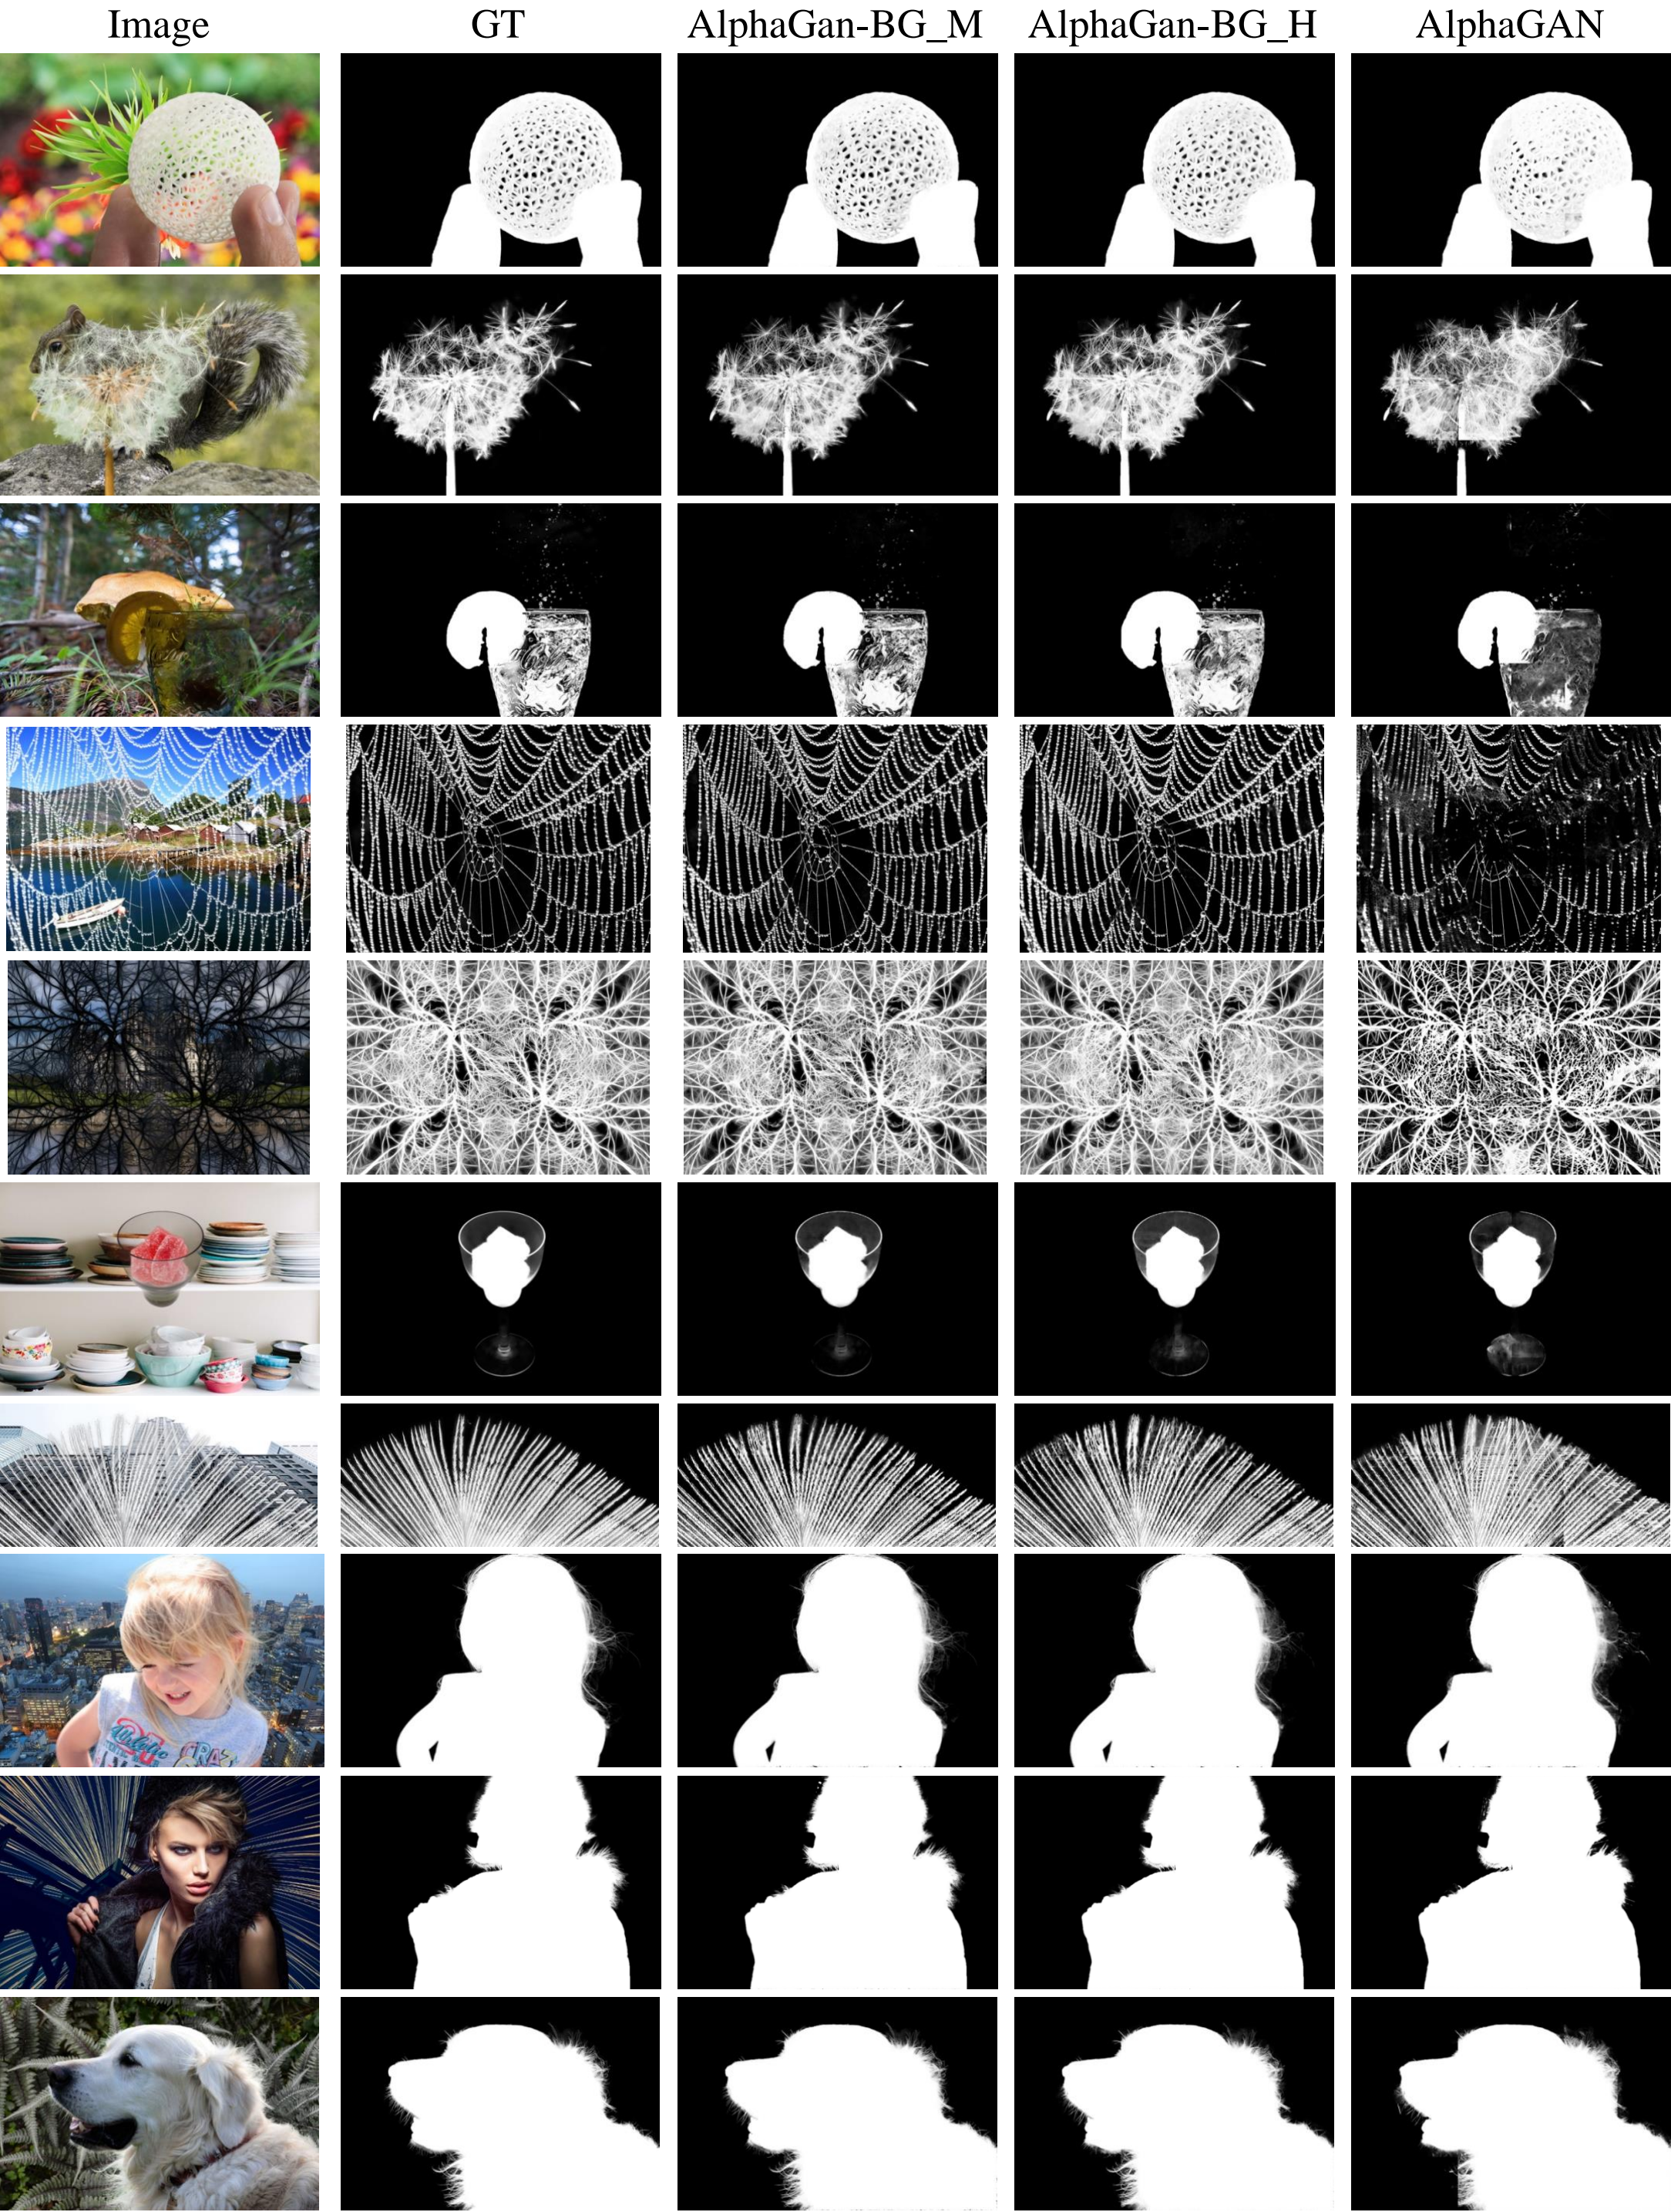   | 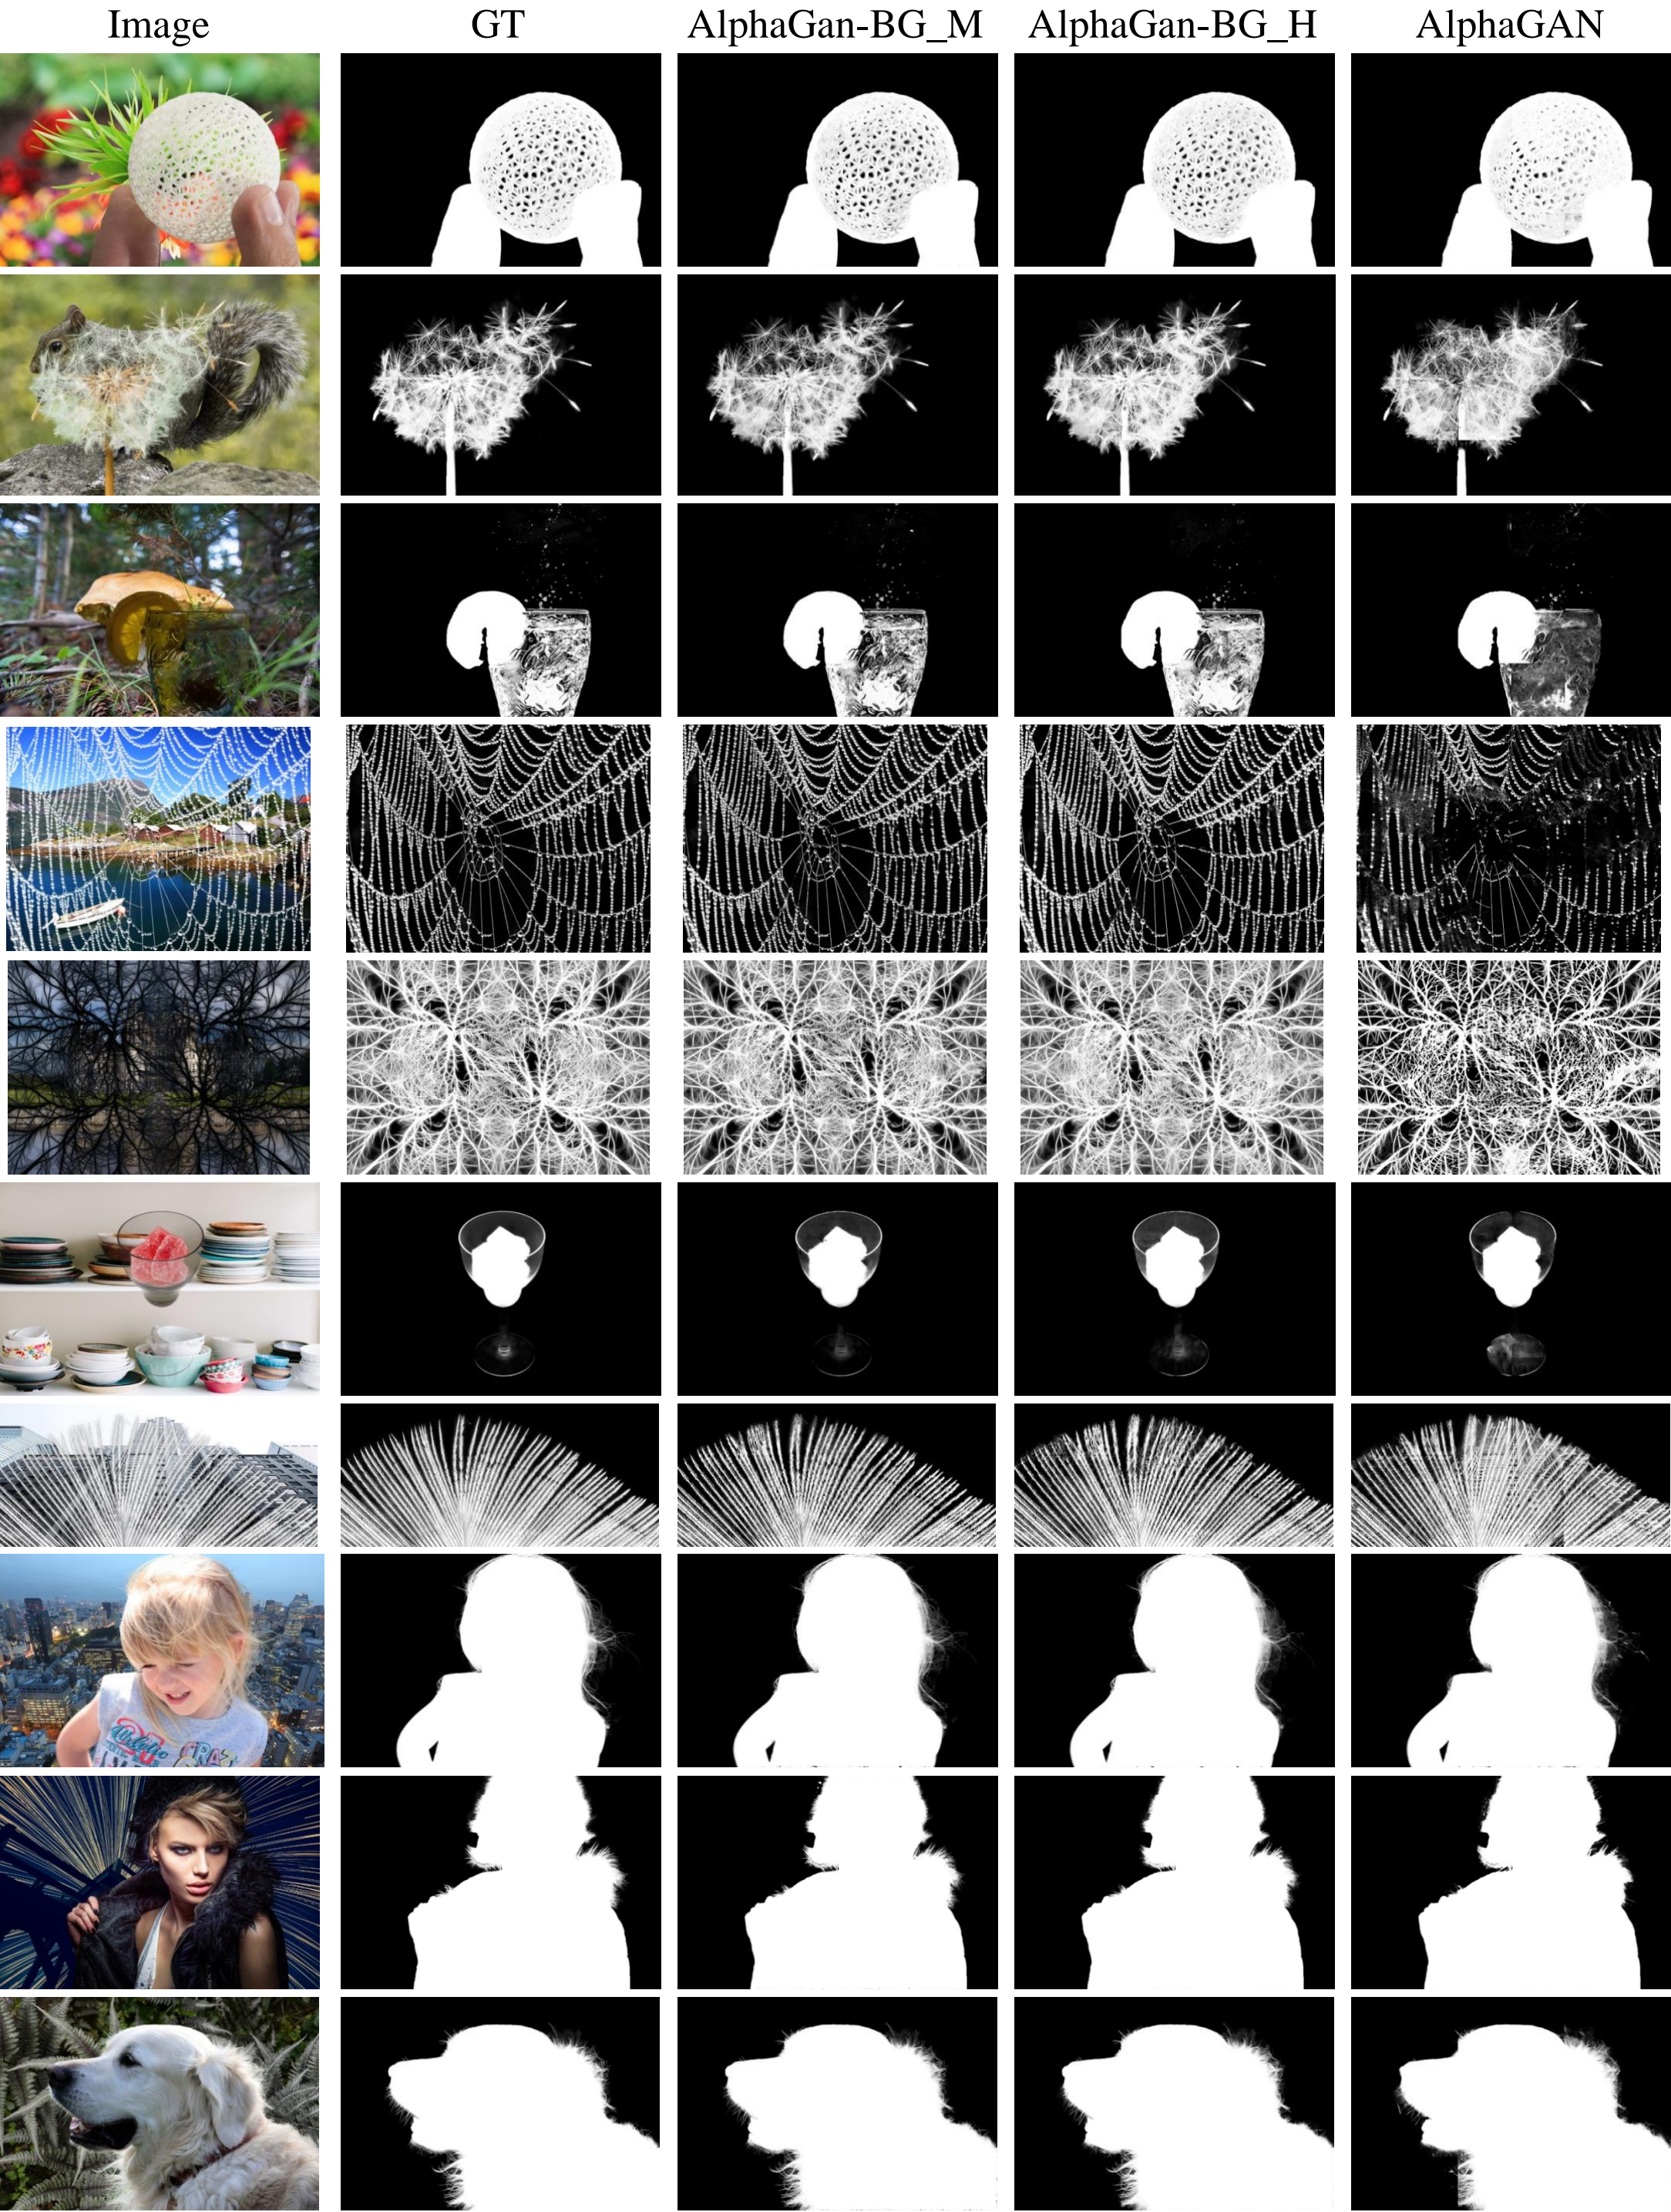   |
| 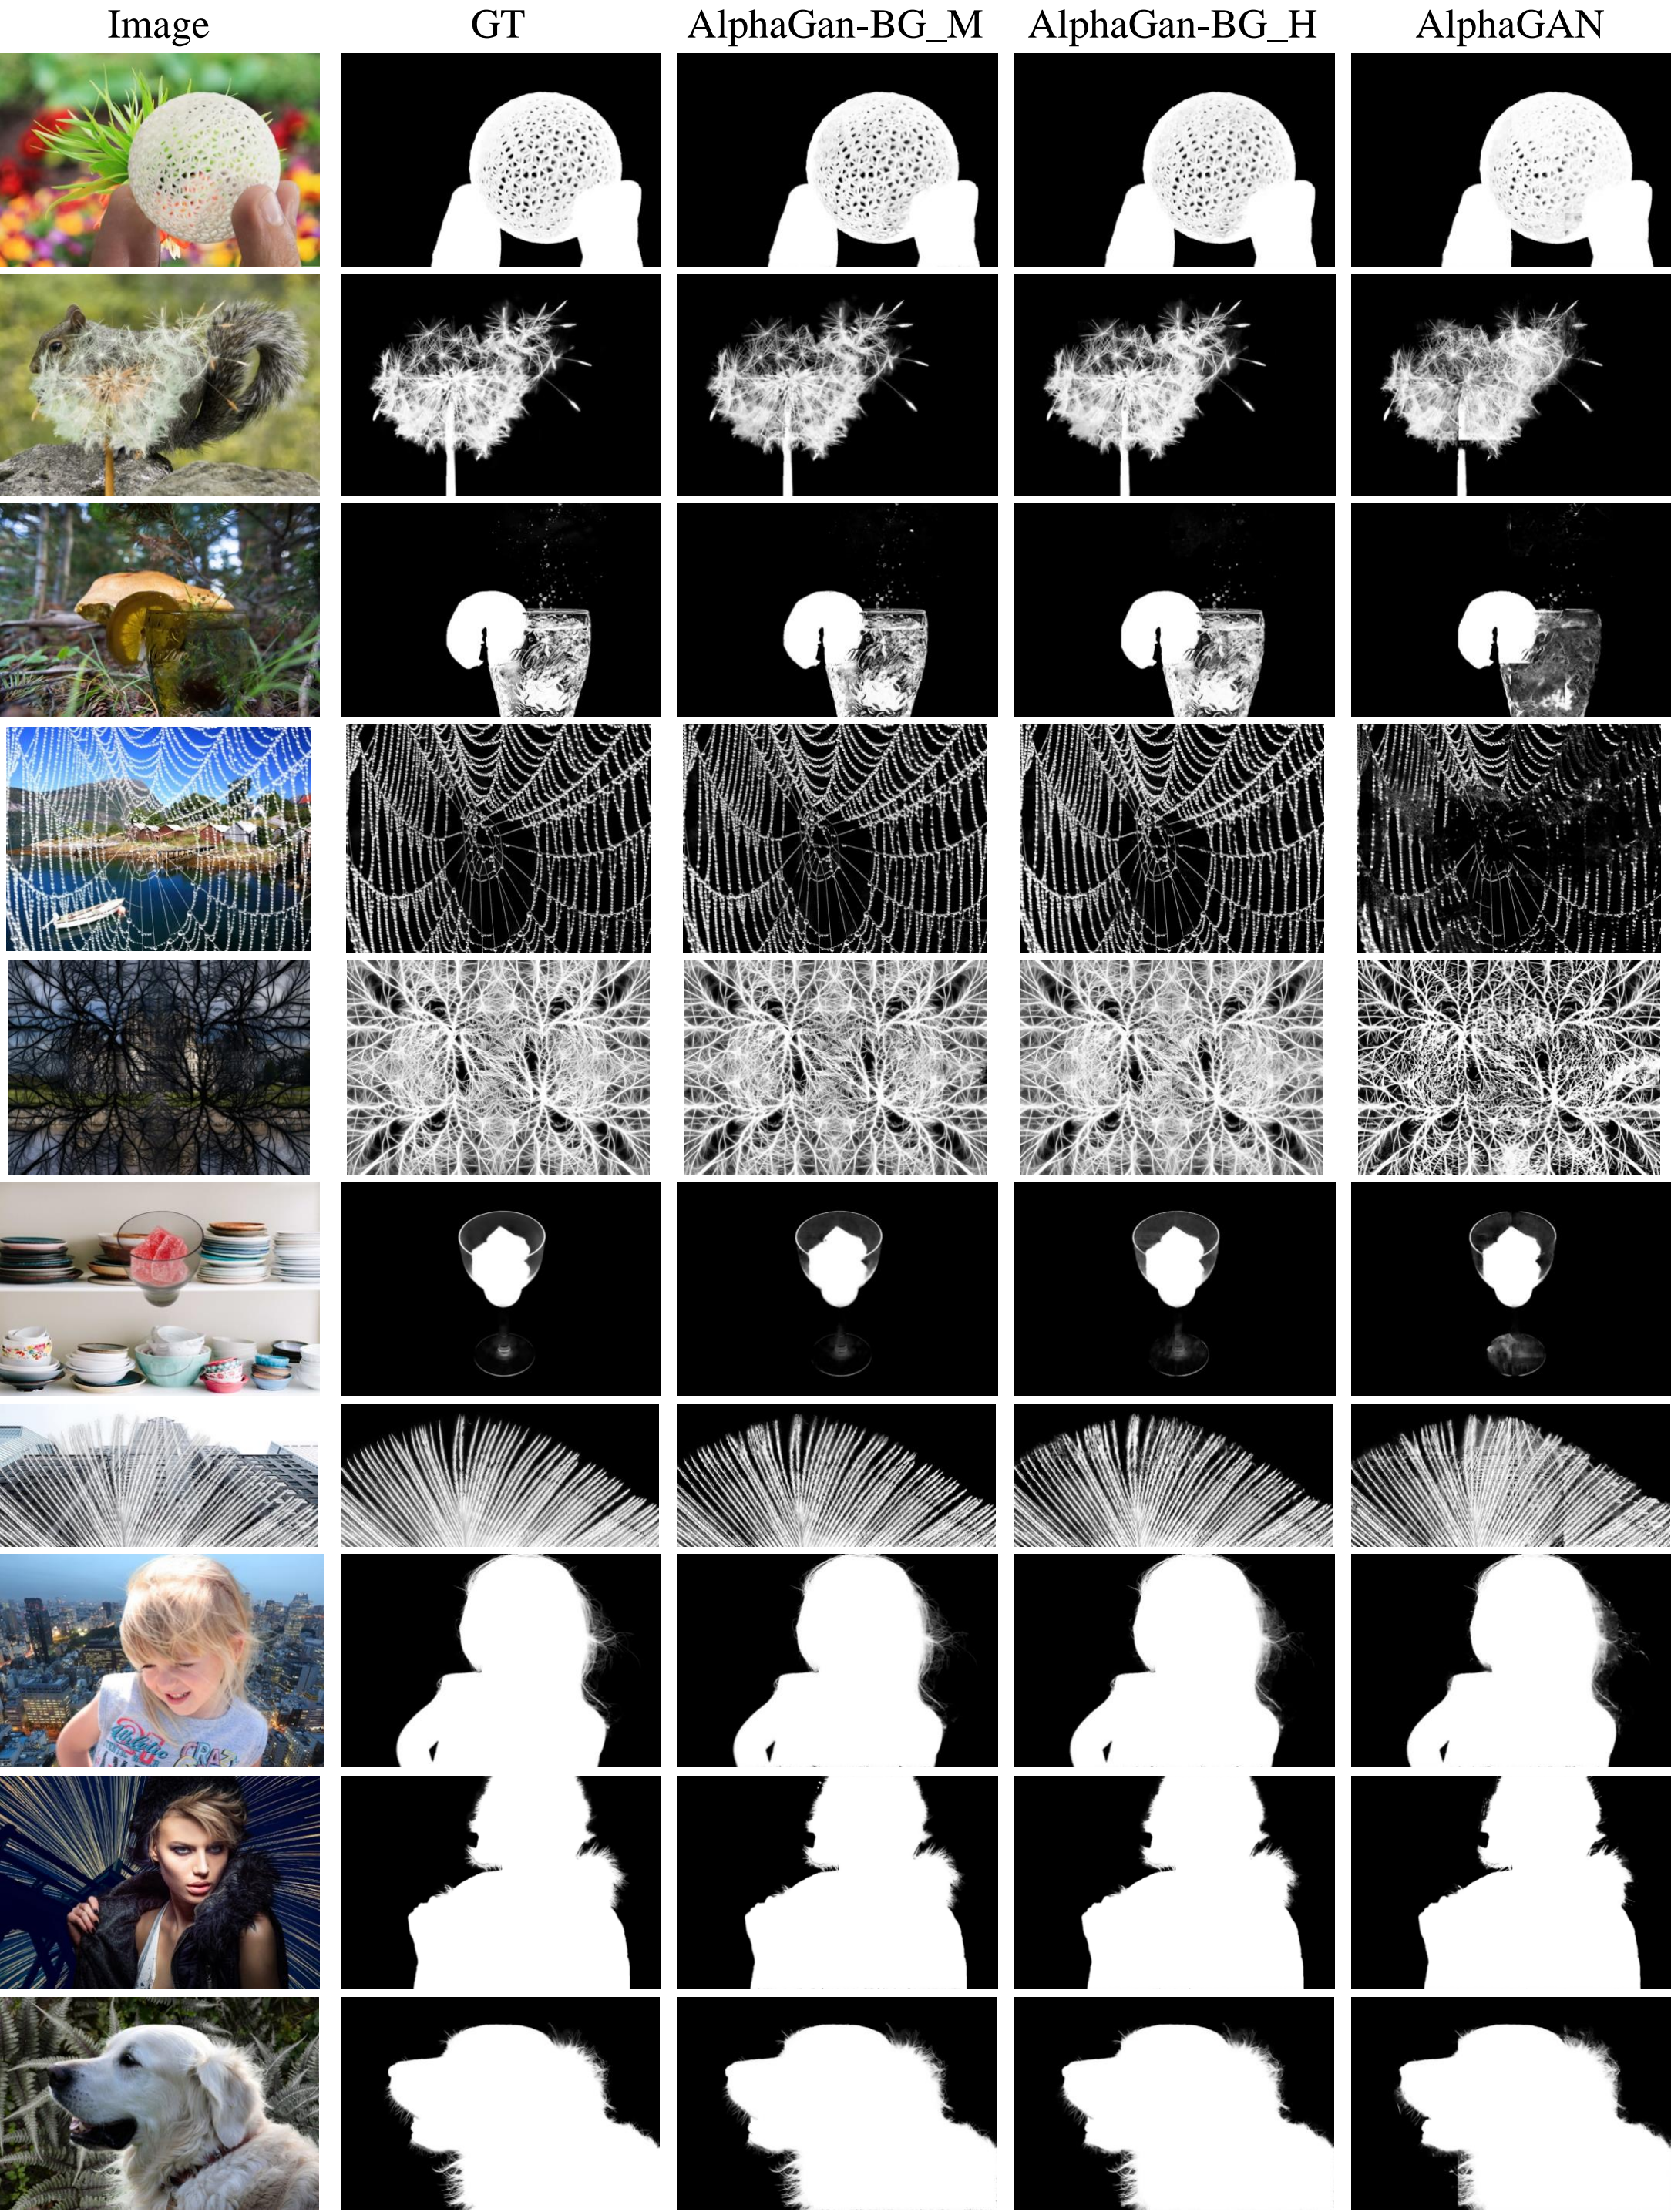  | 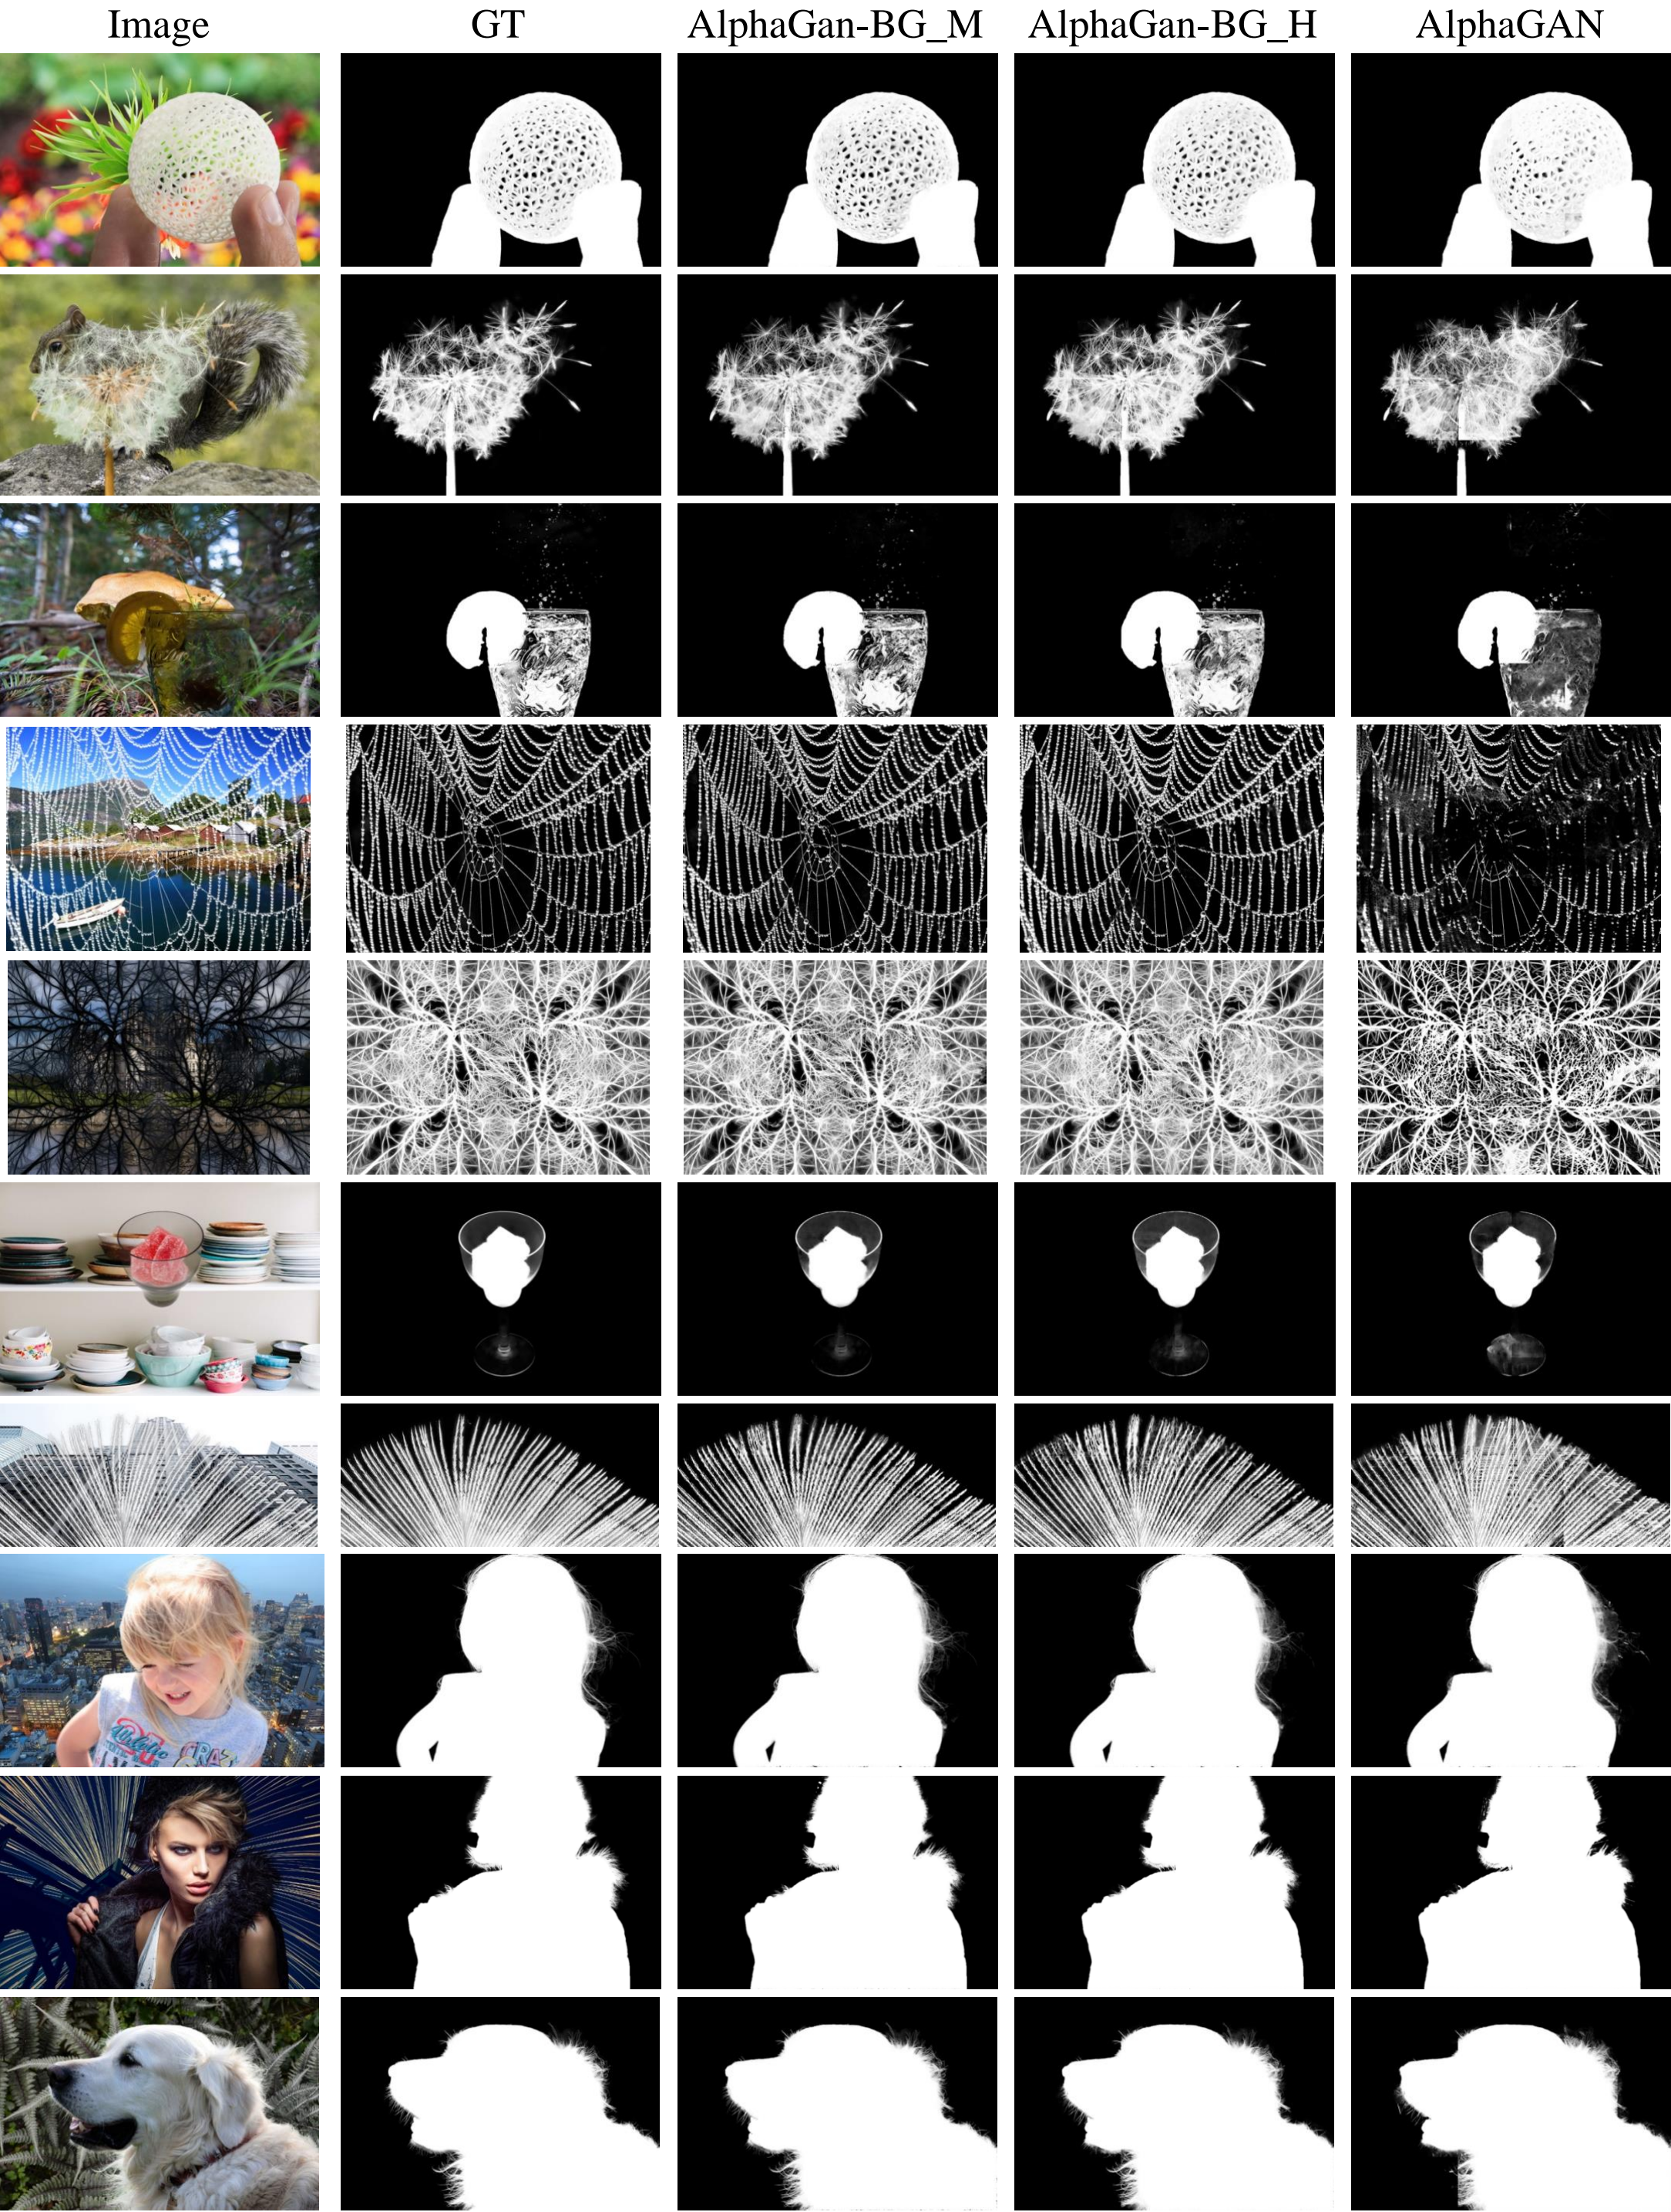  | 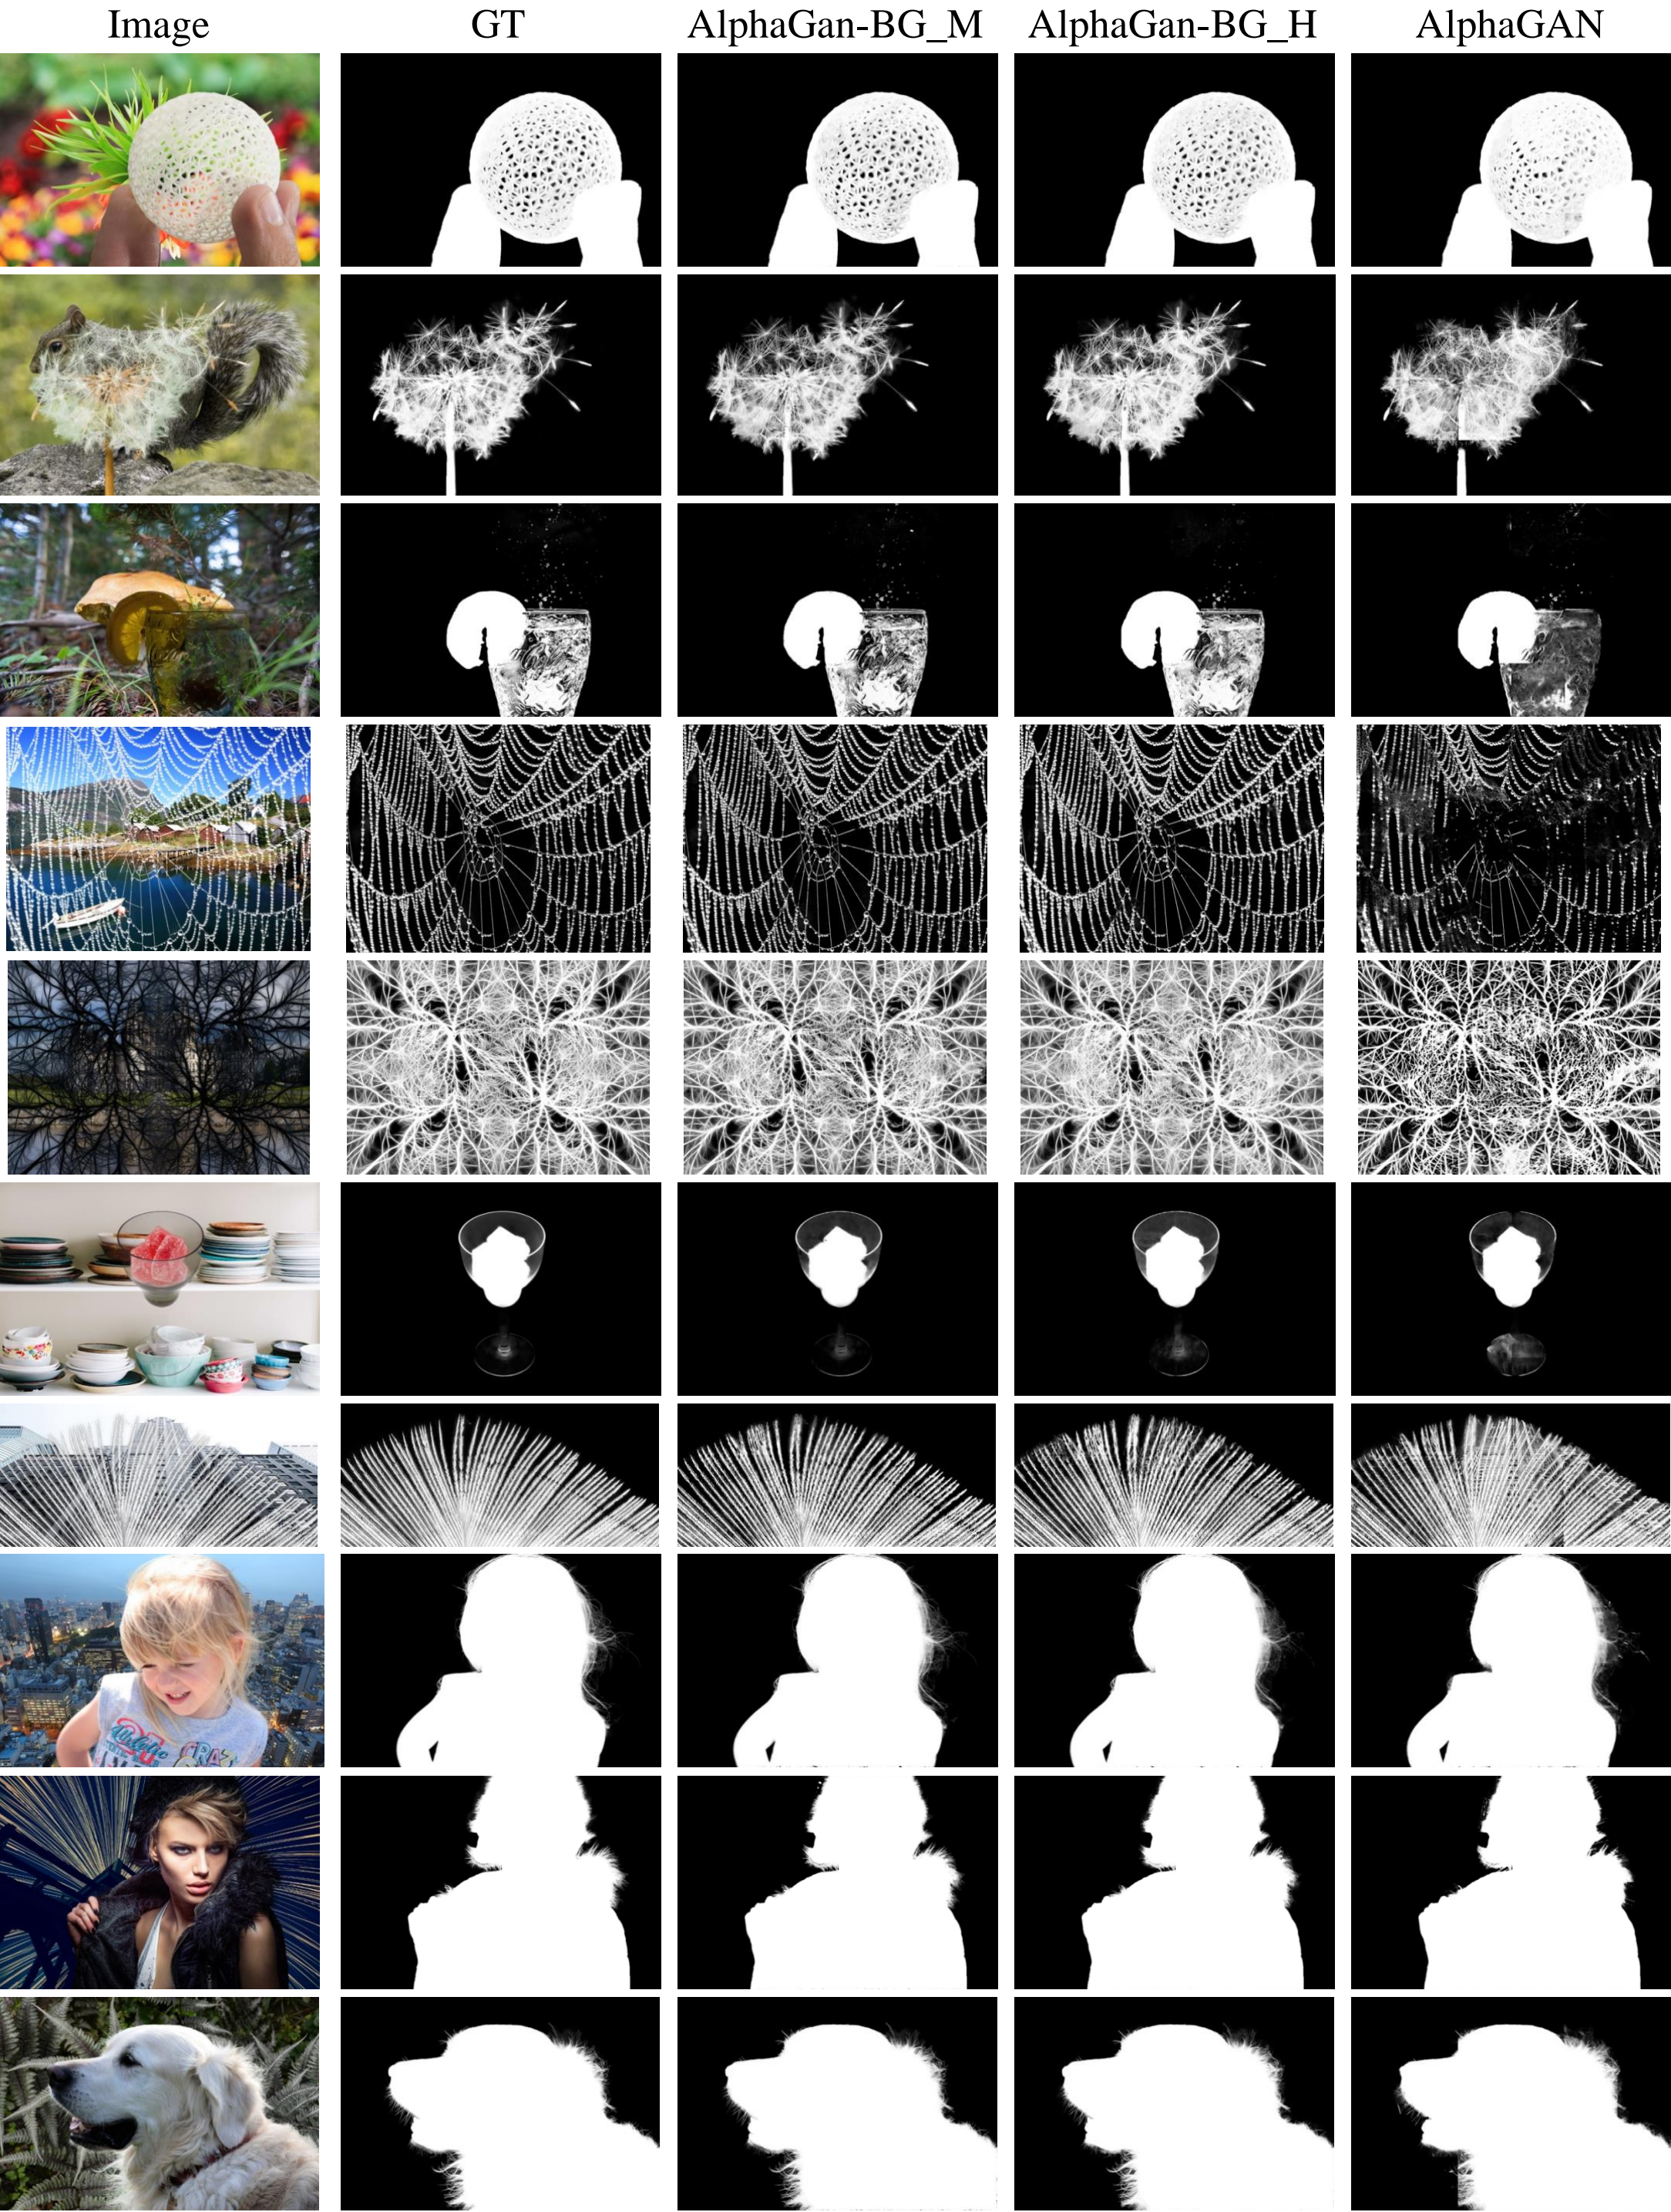  | 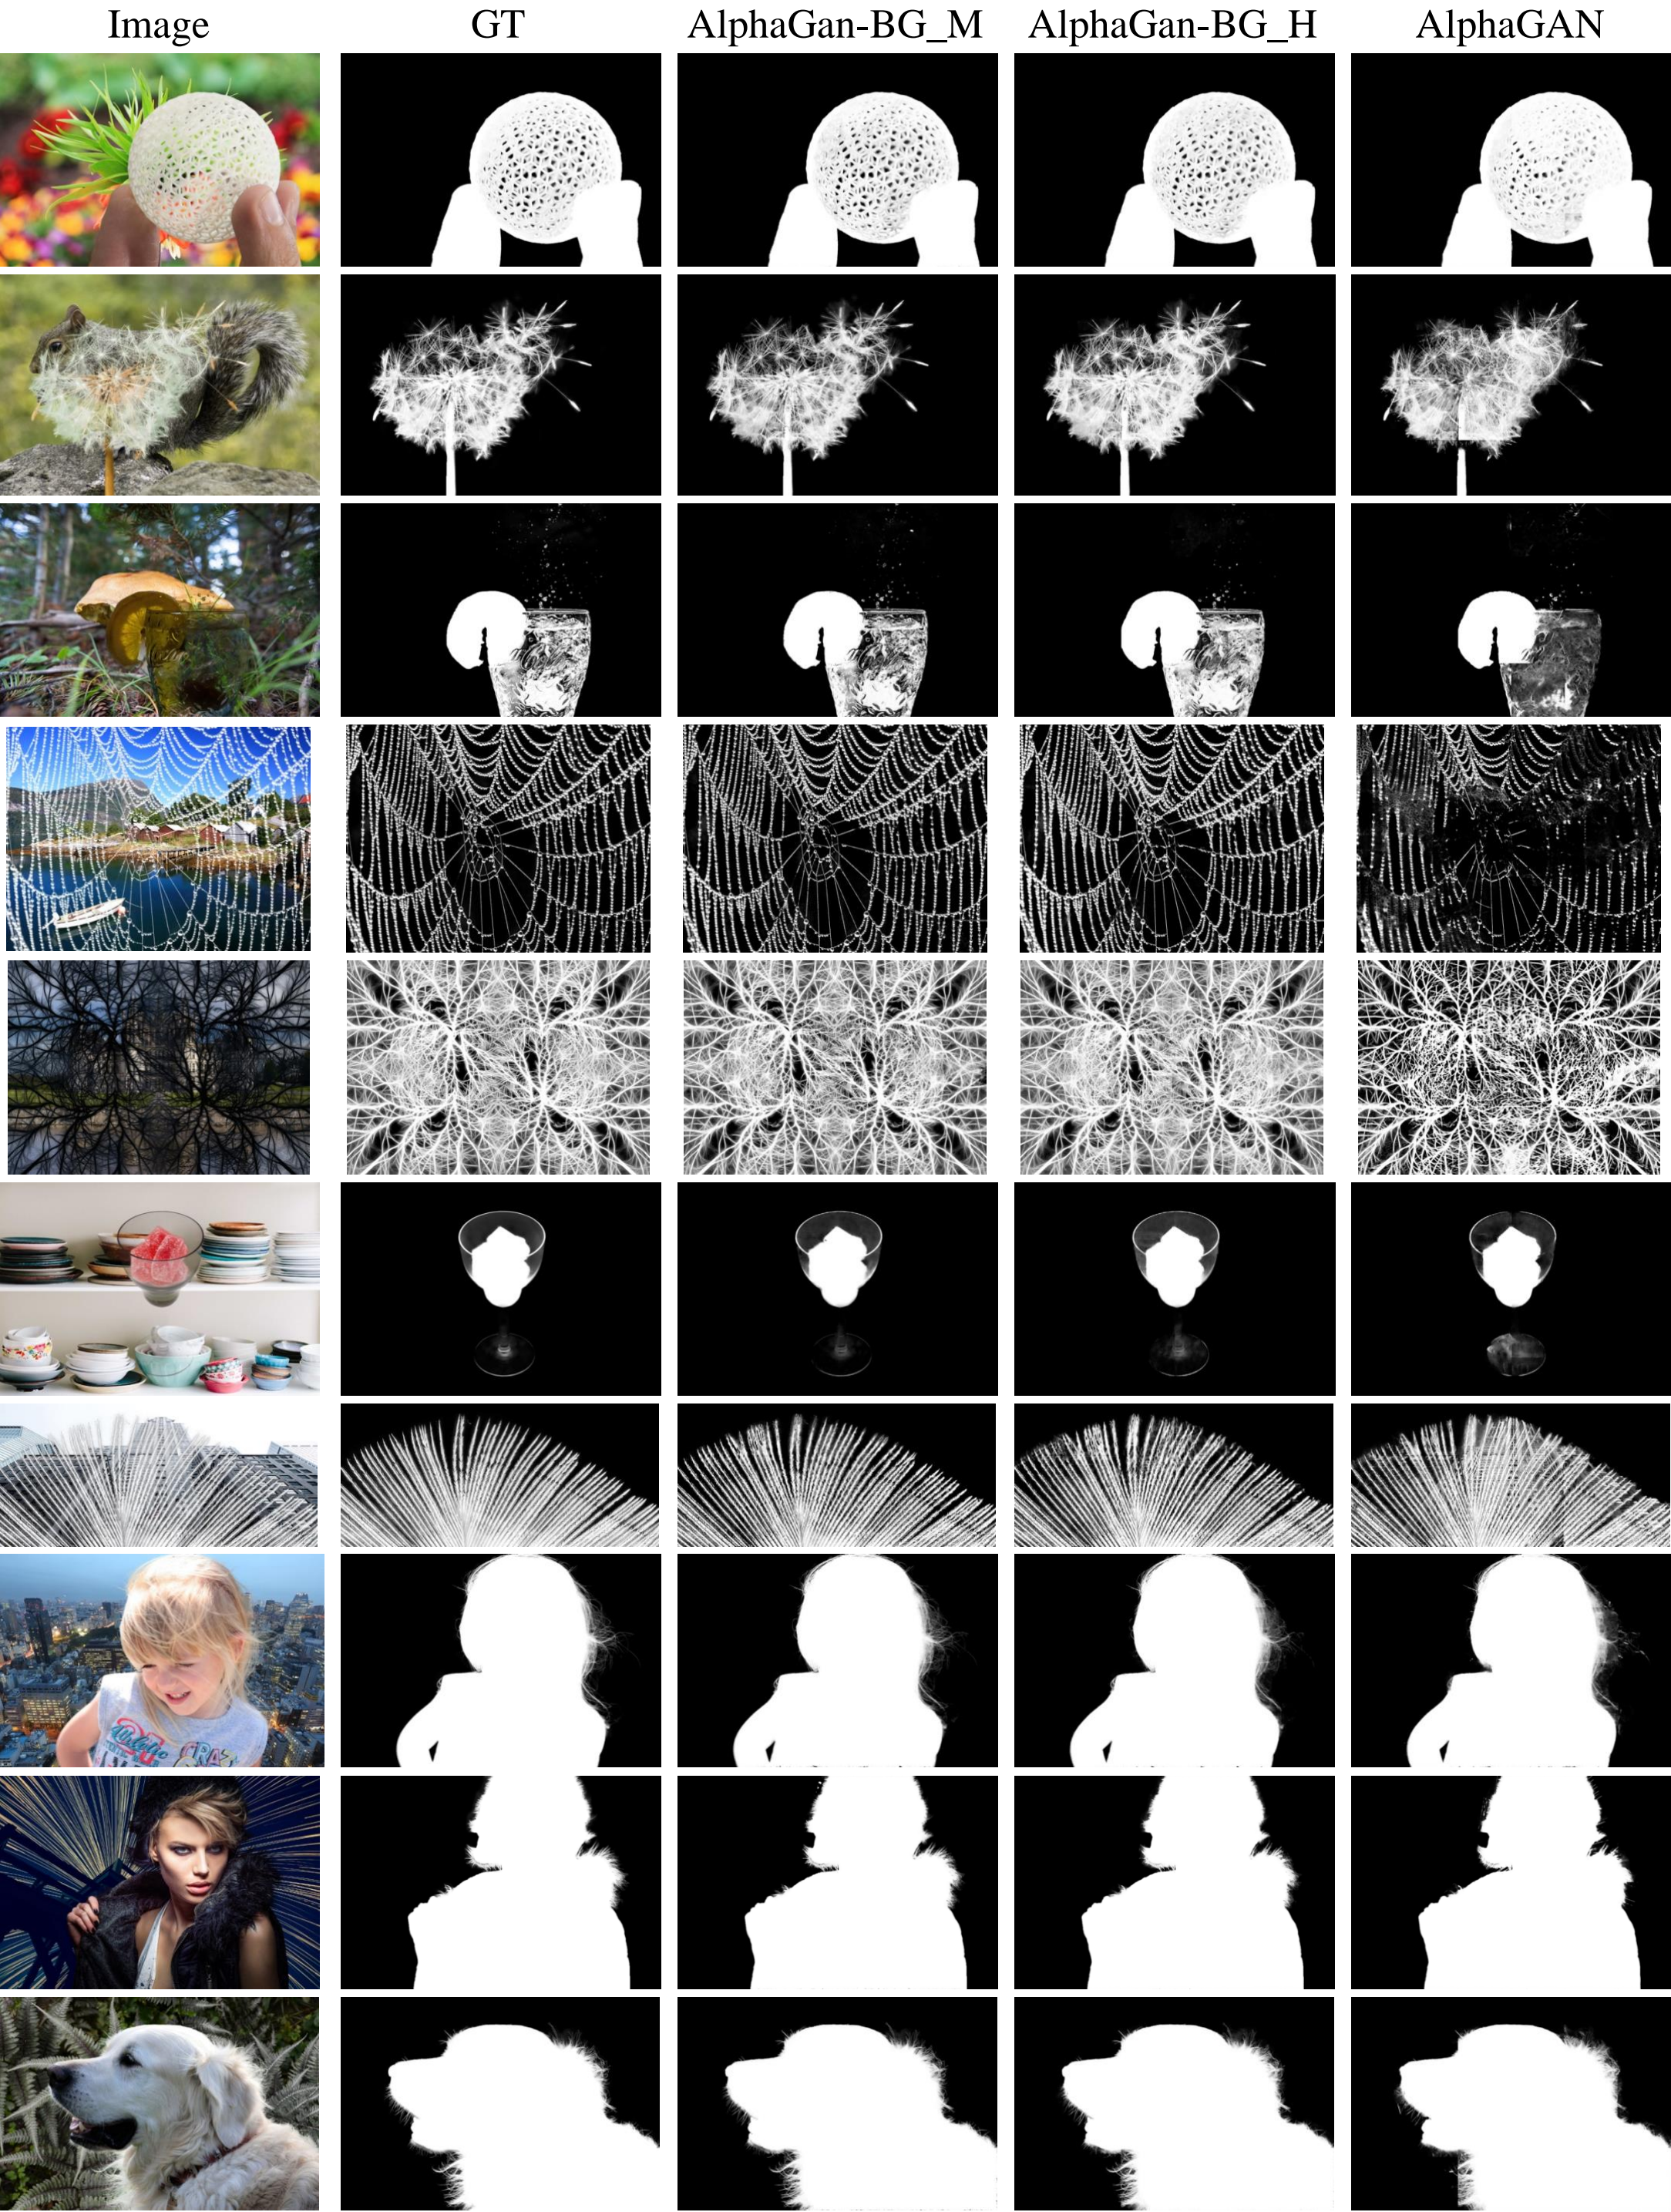  | 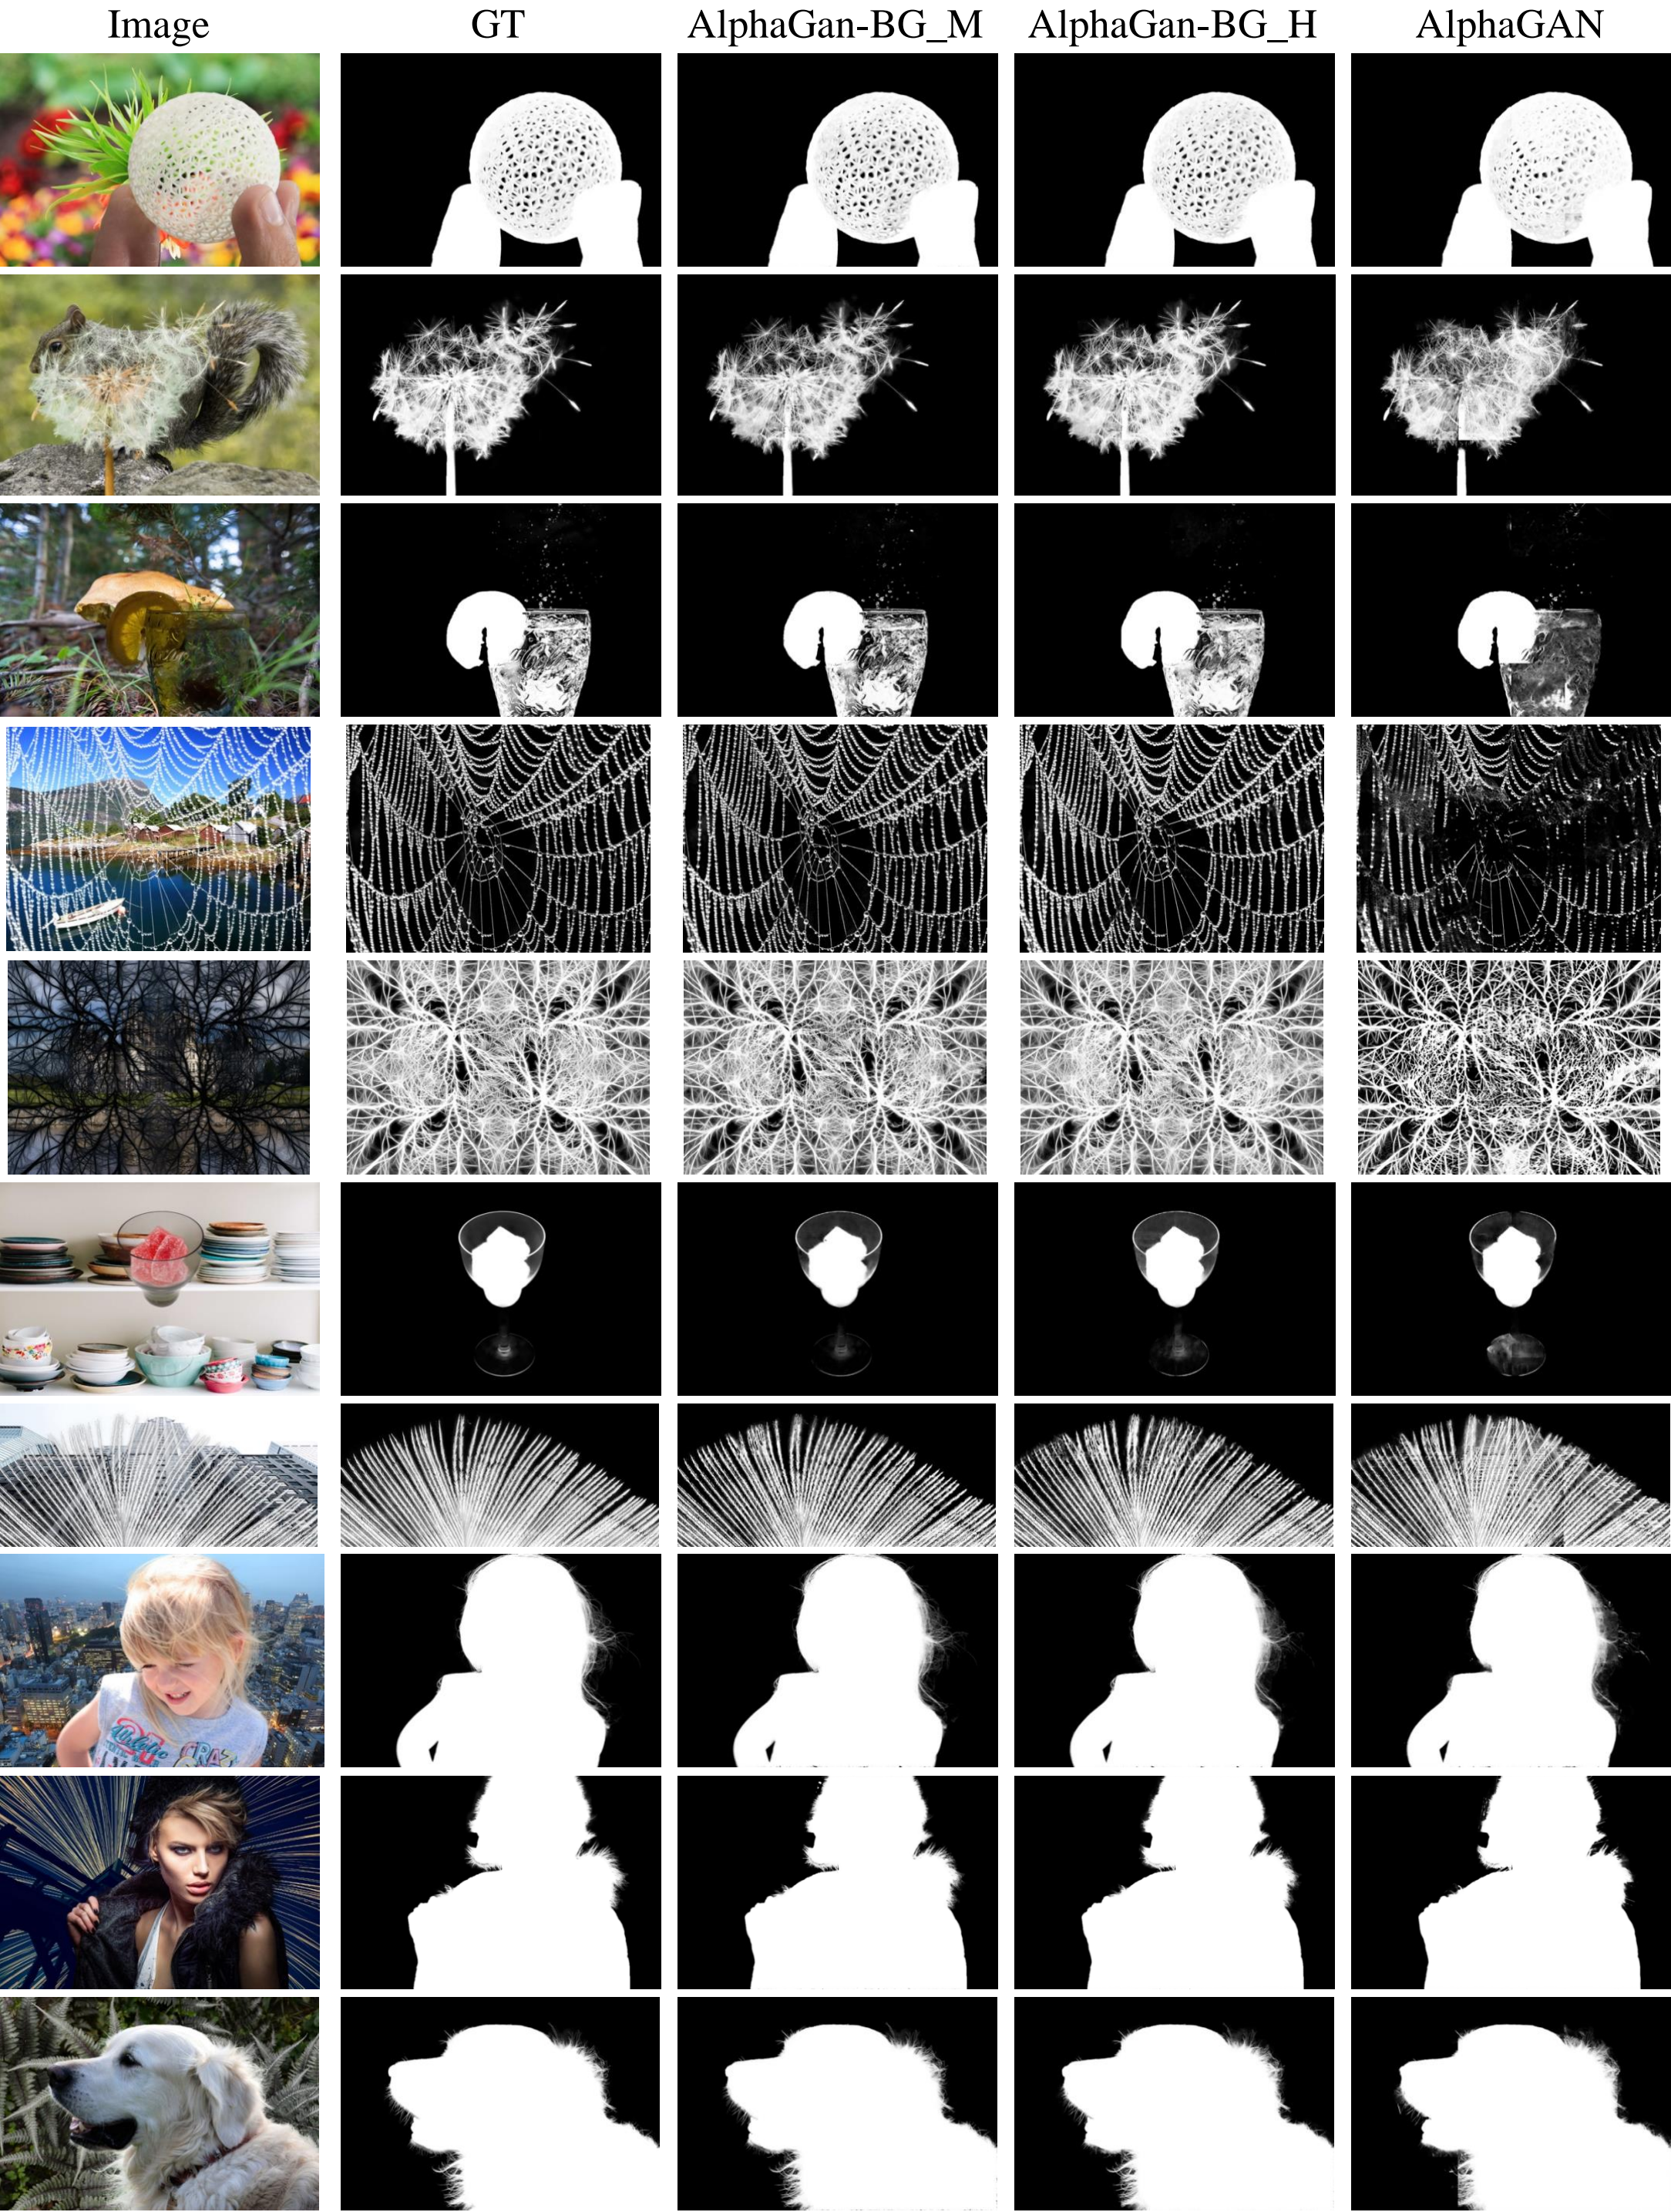  |
| 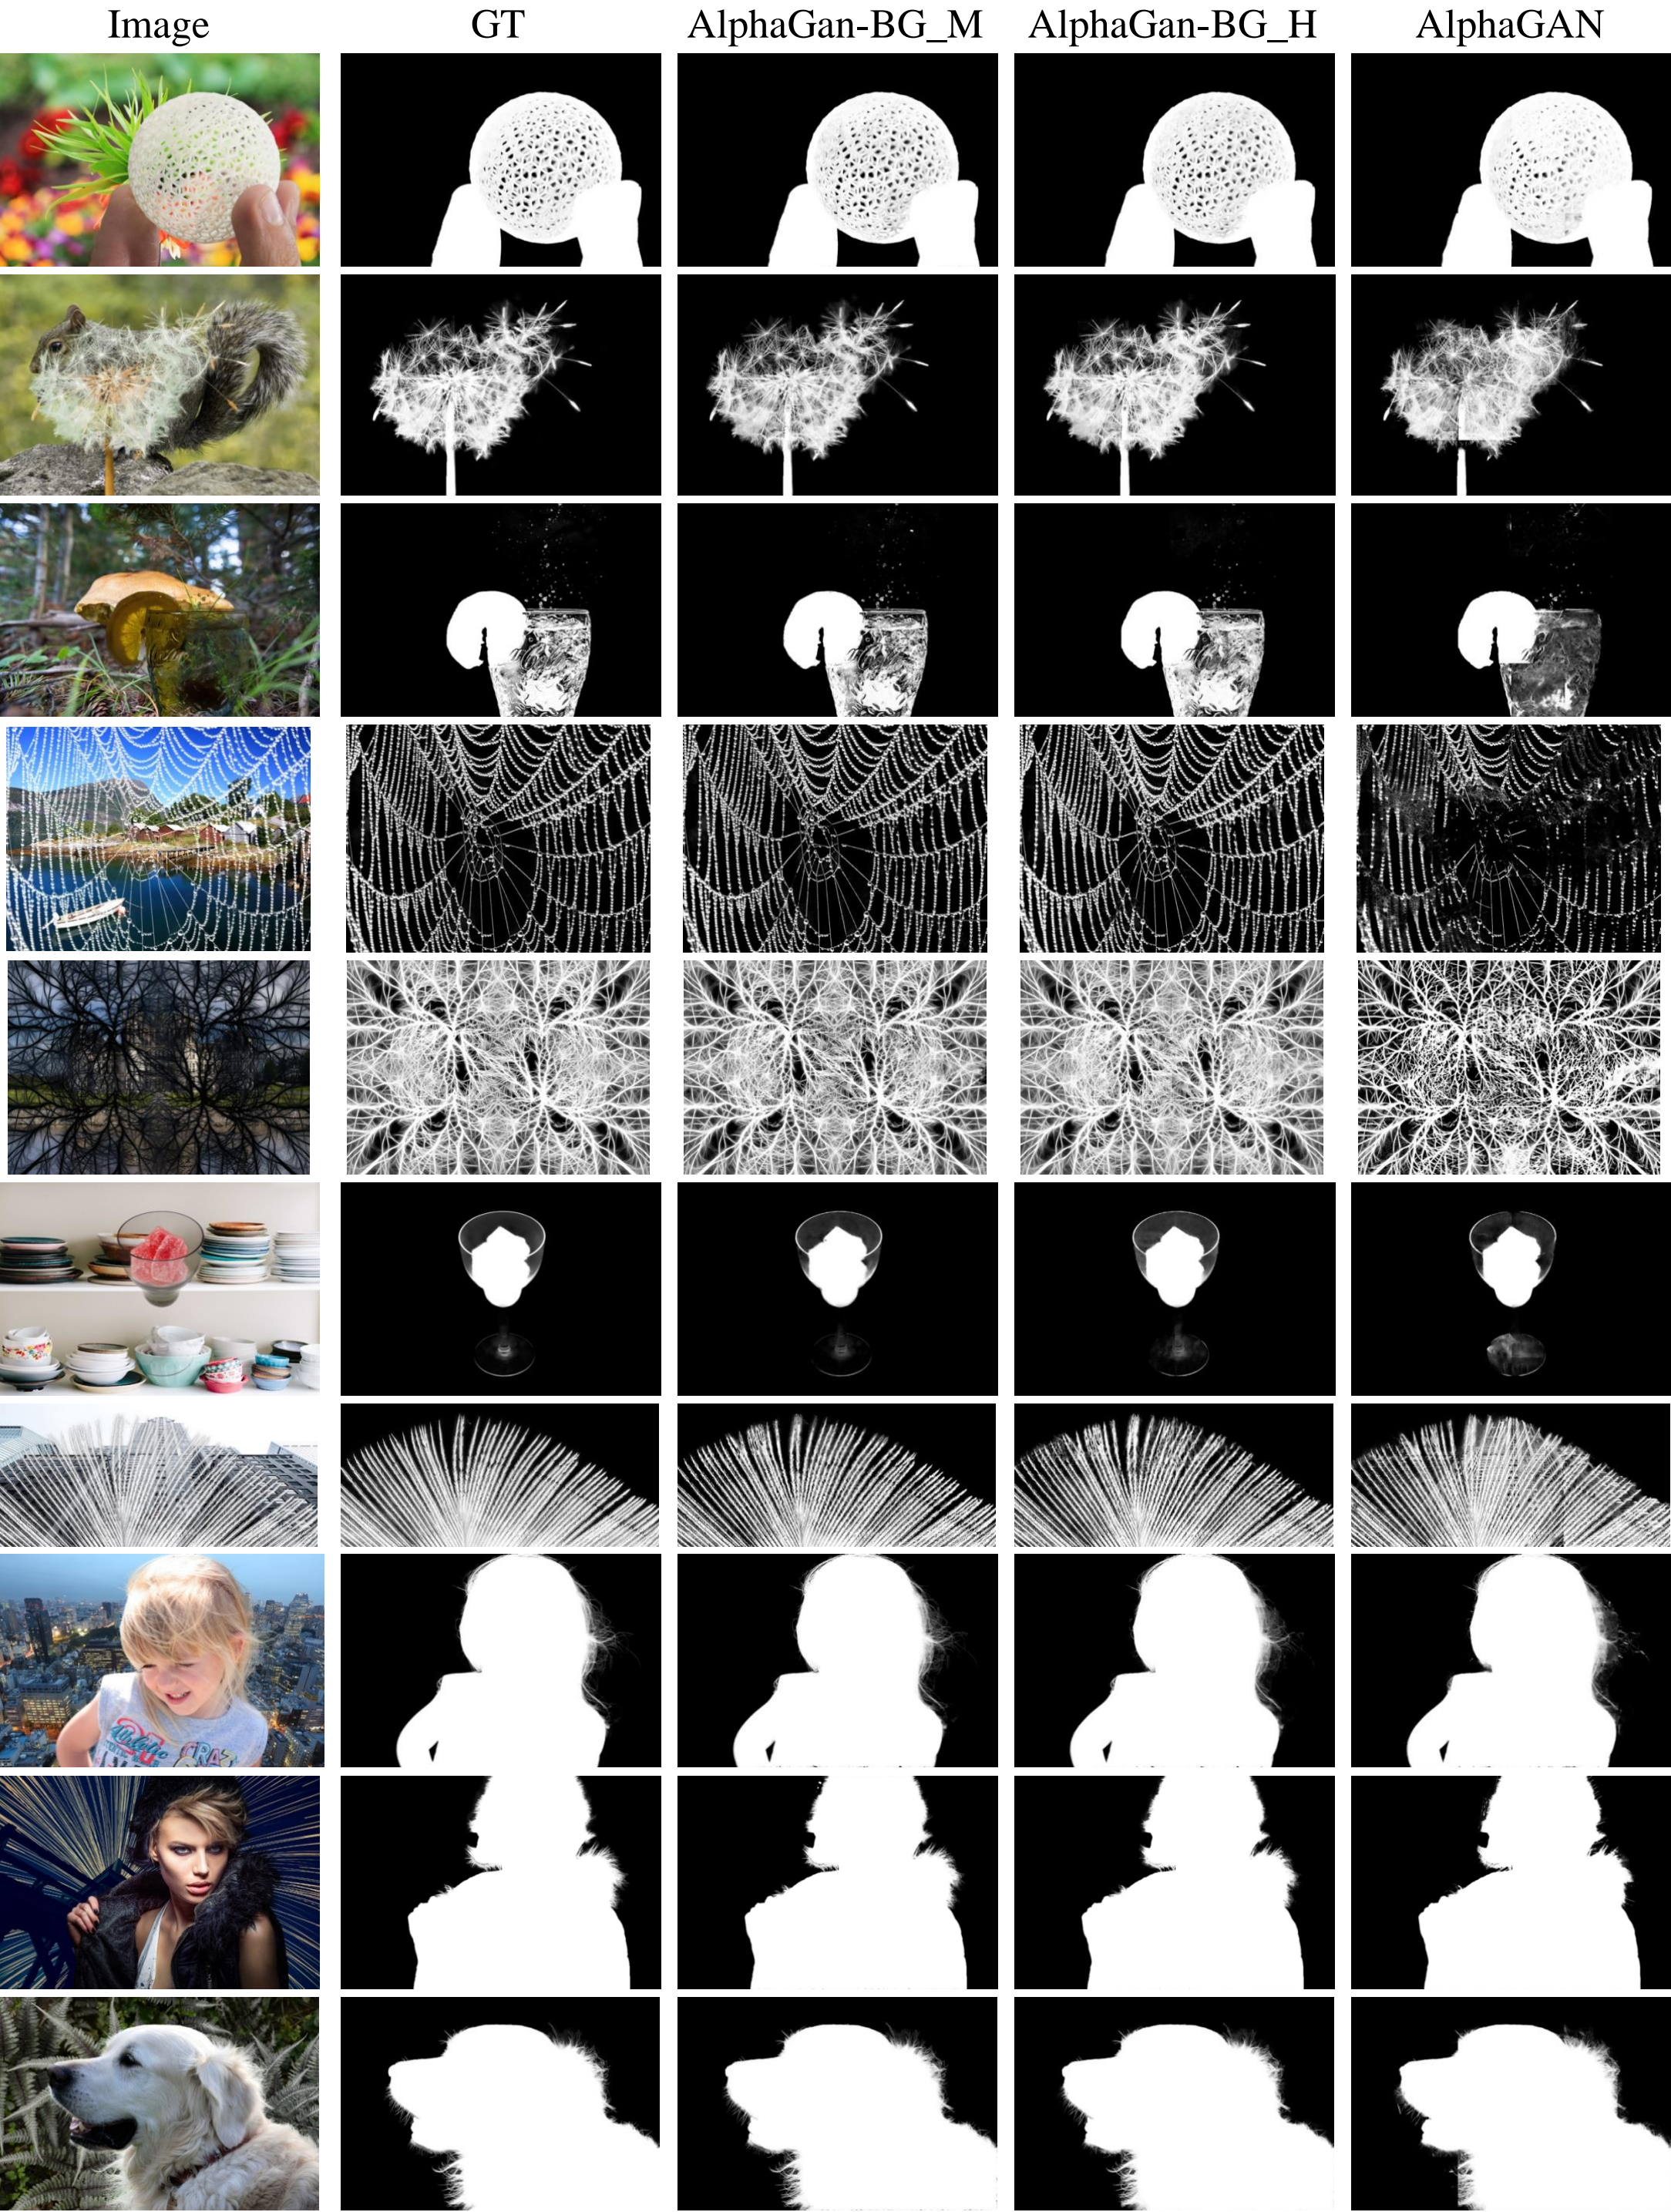 | 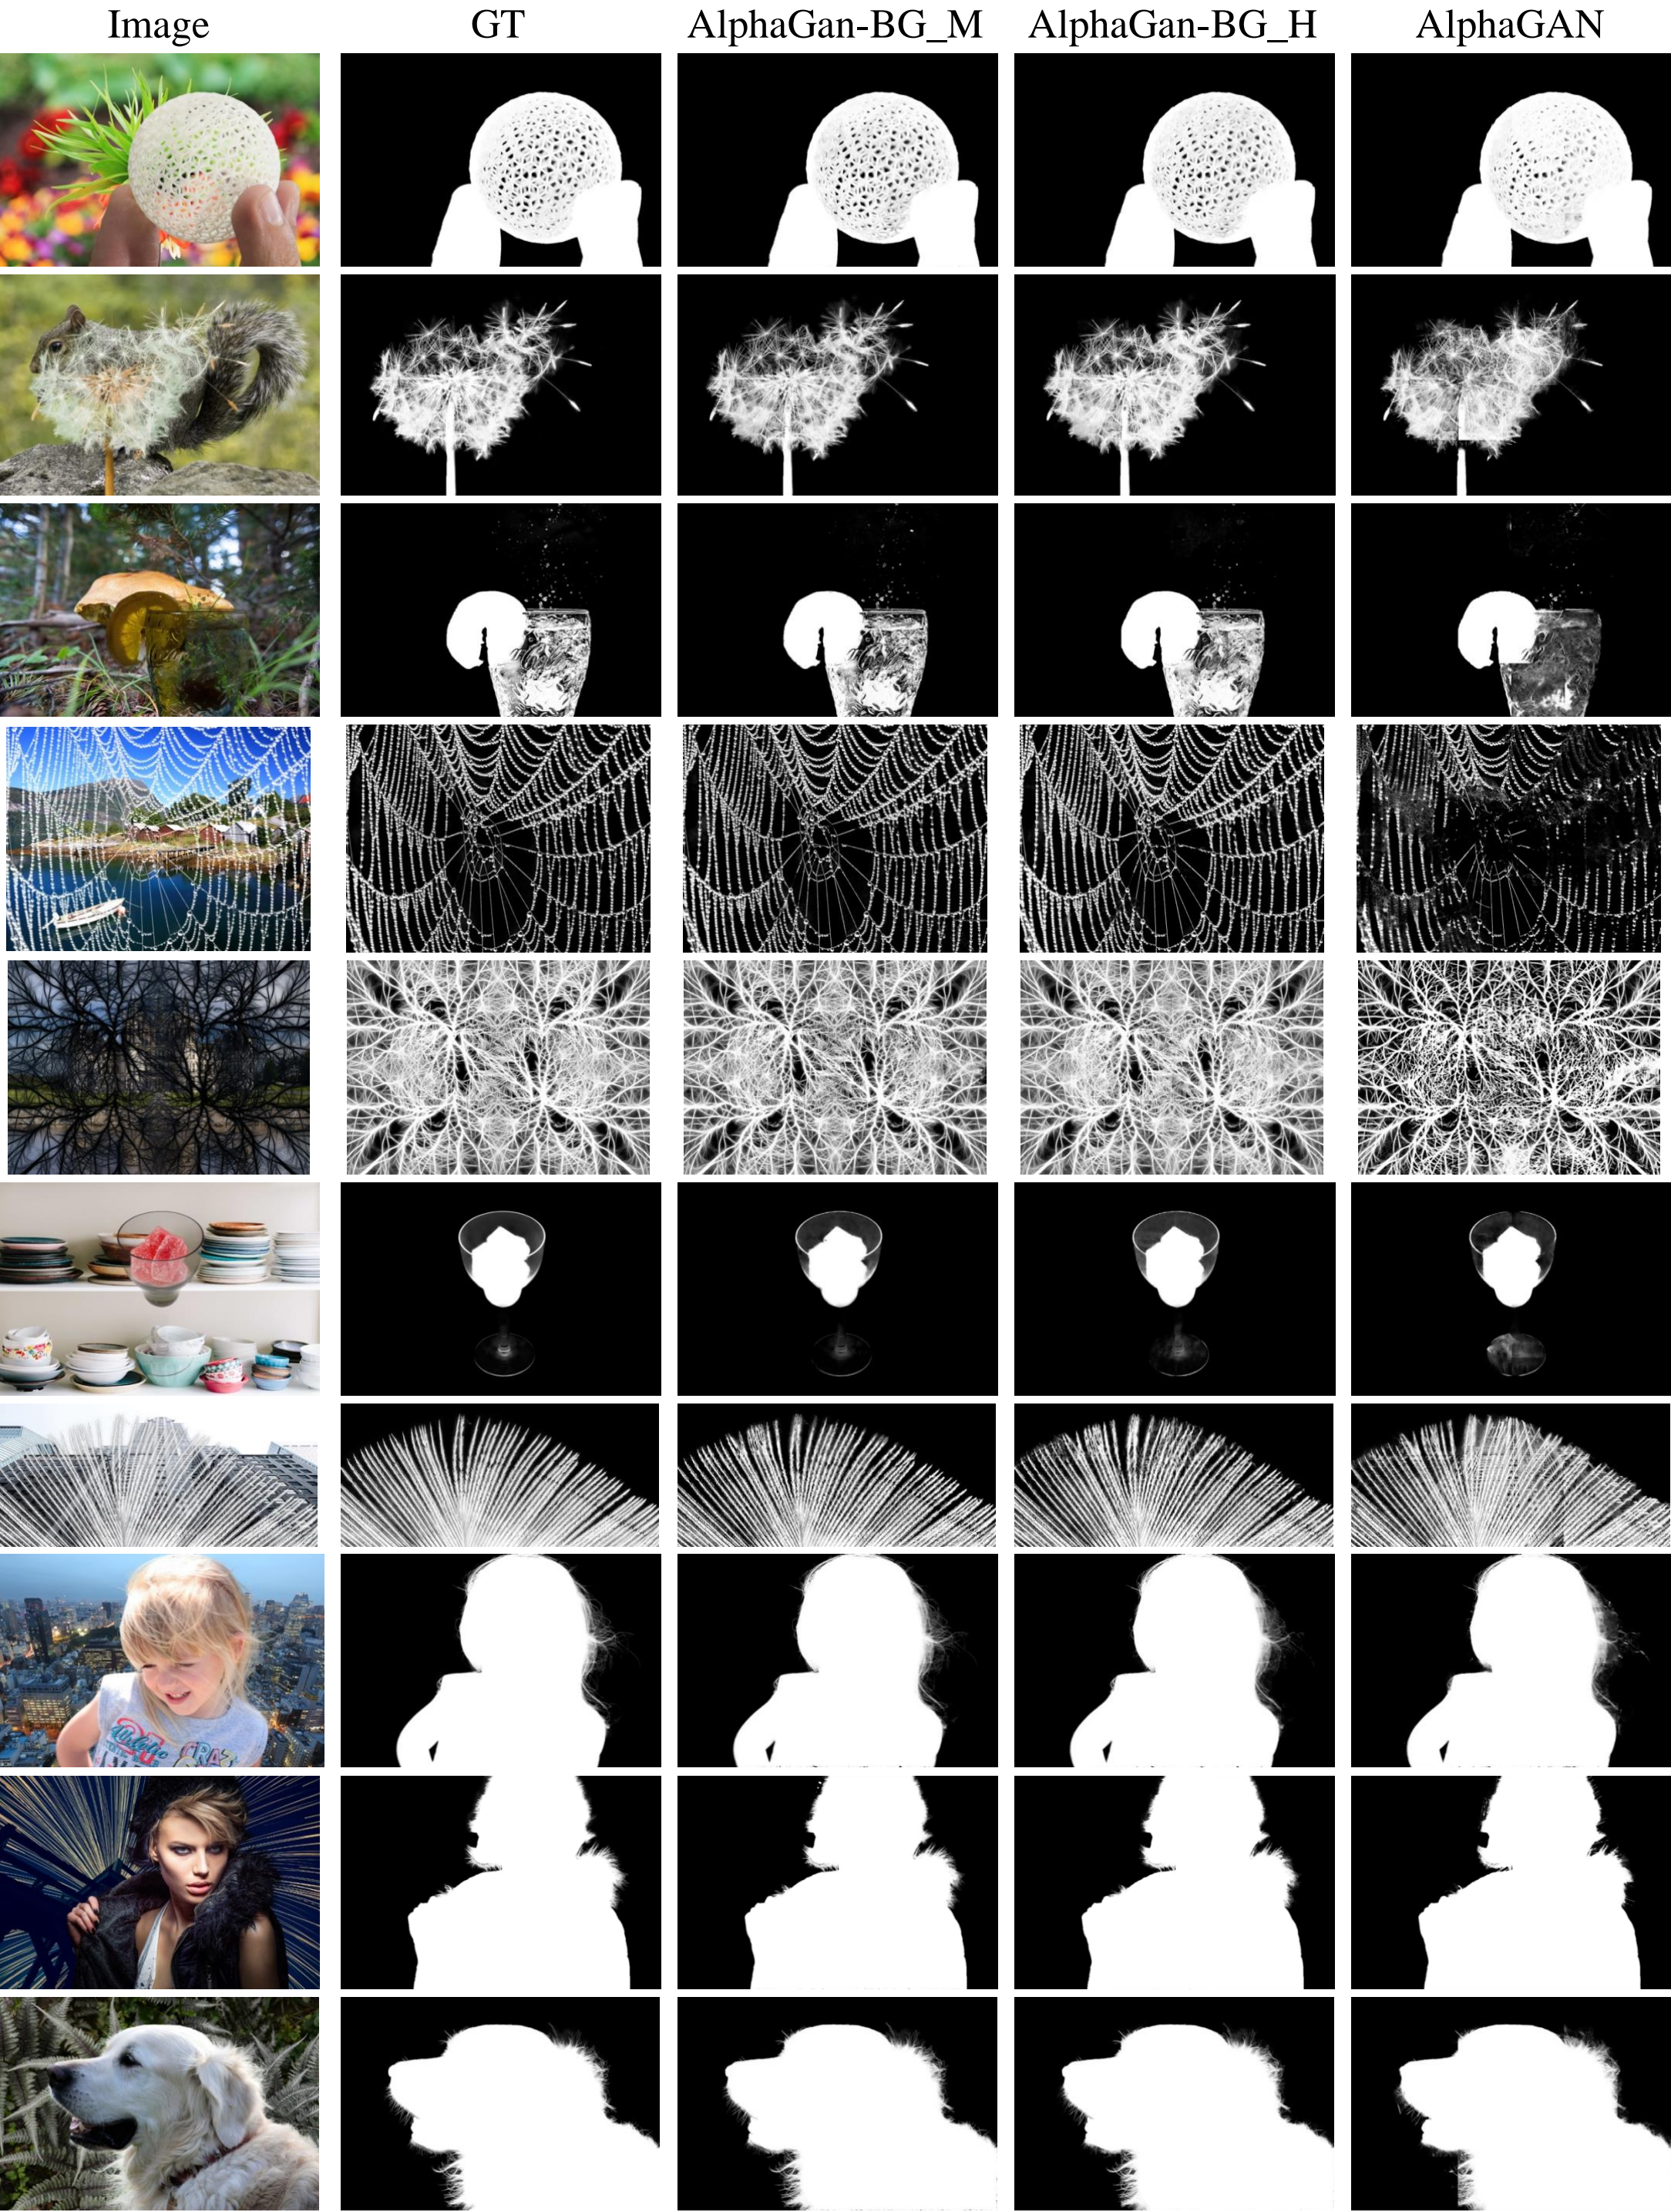 | 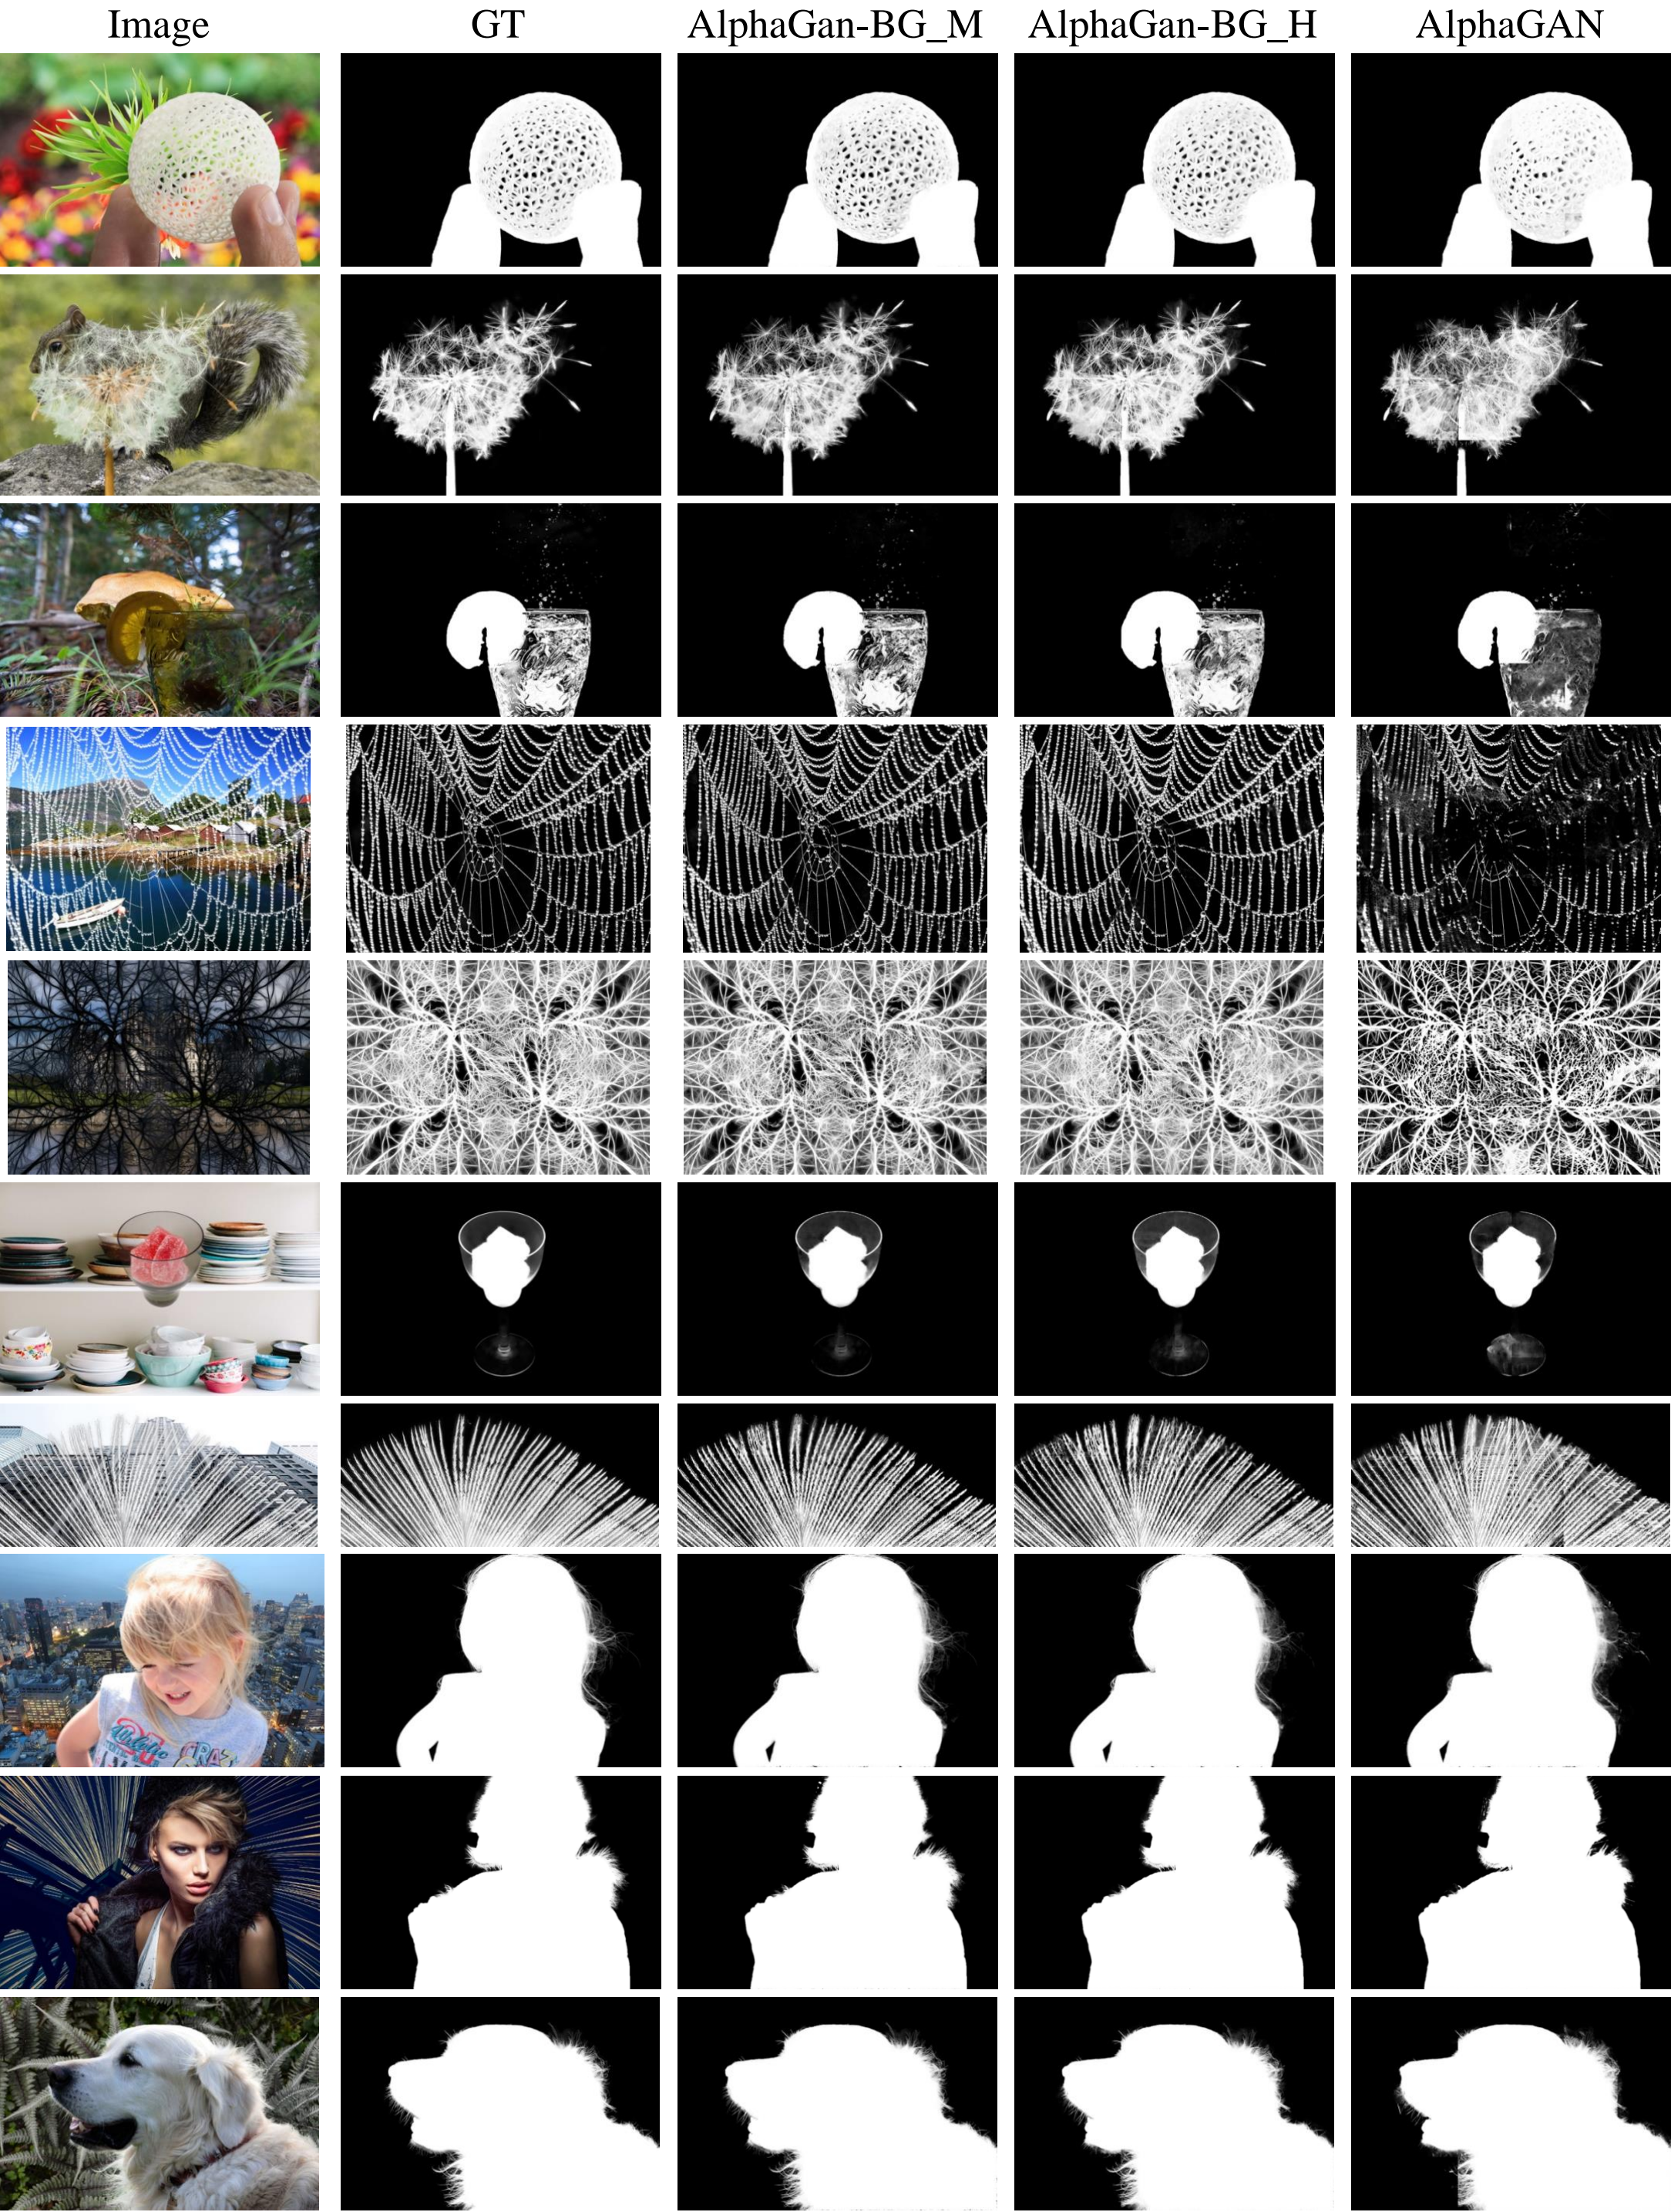 | 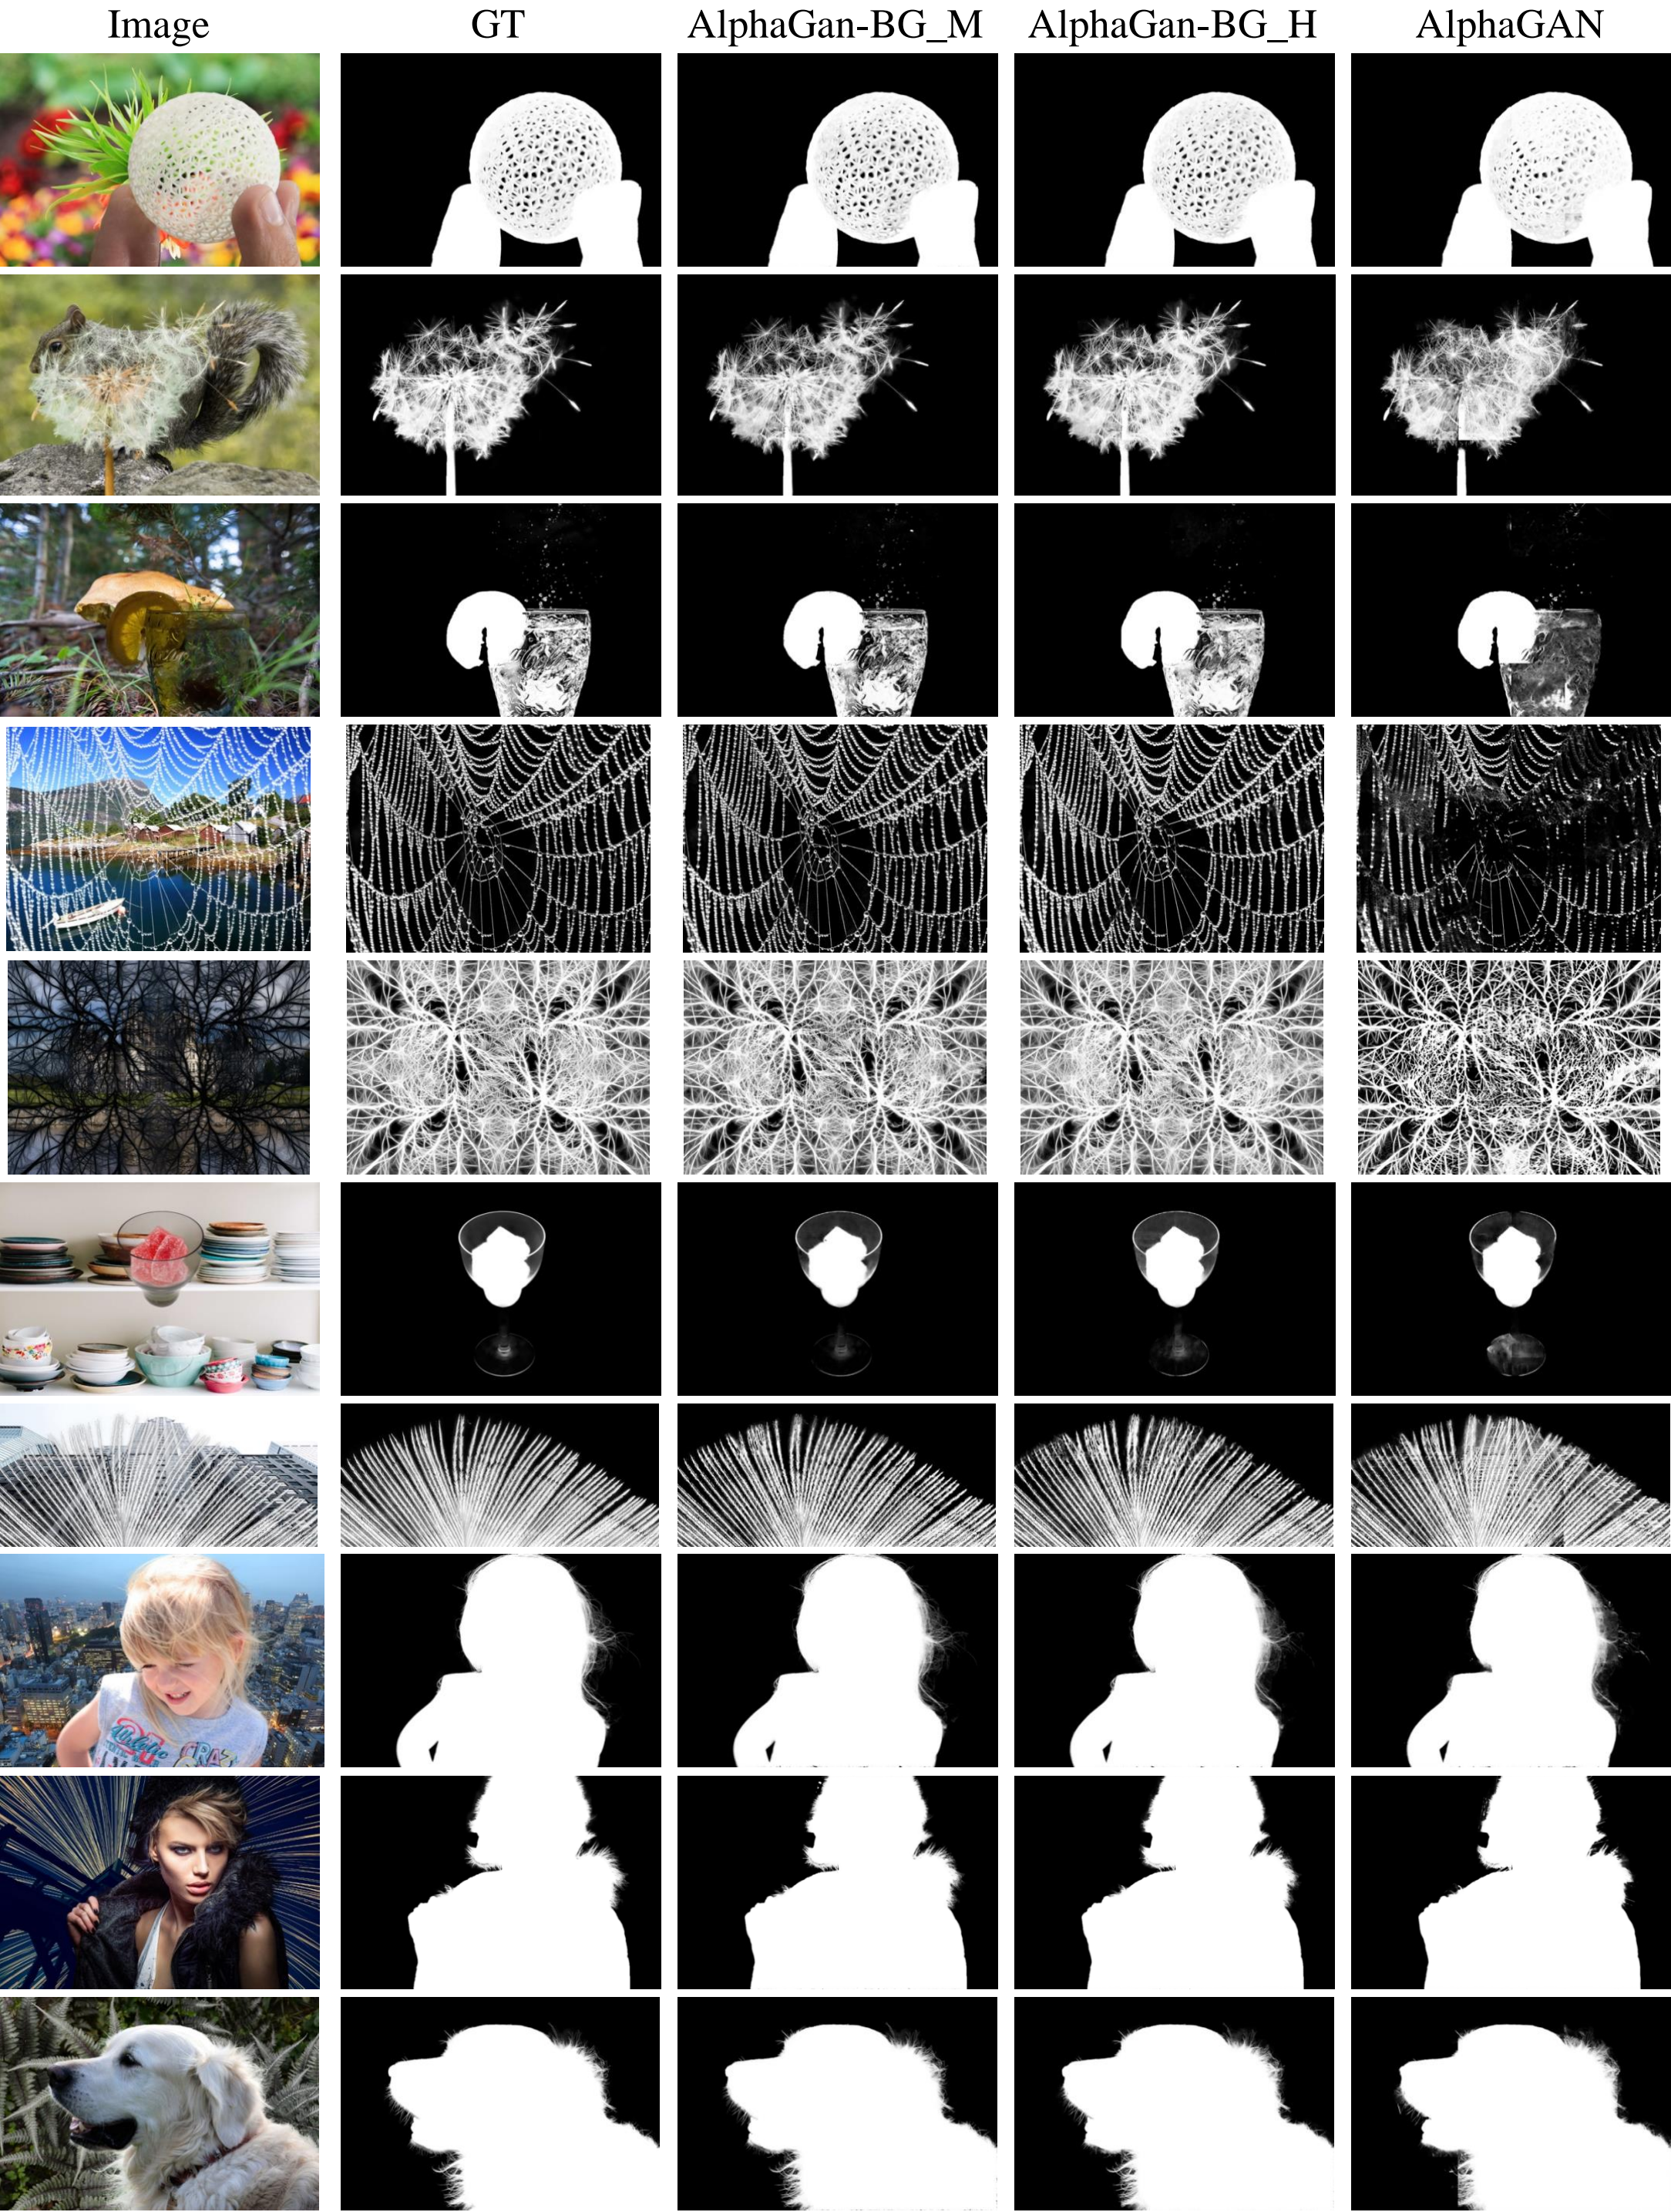 | 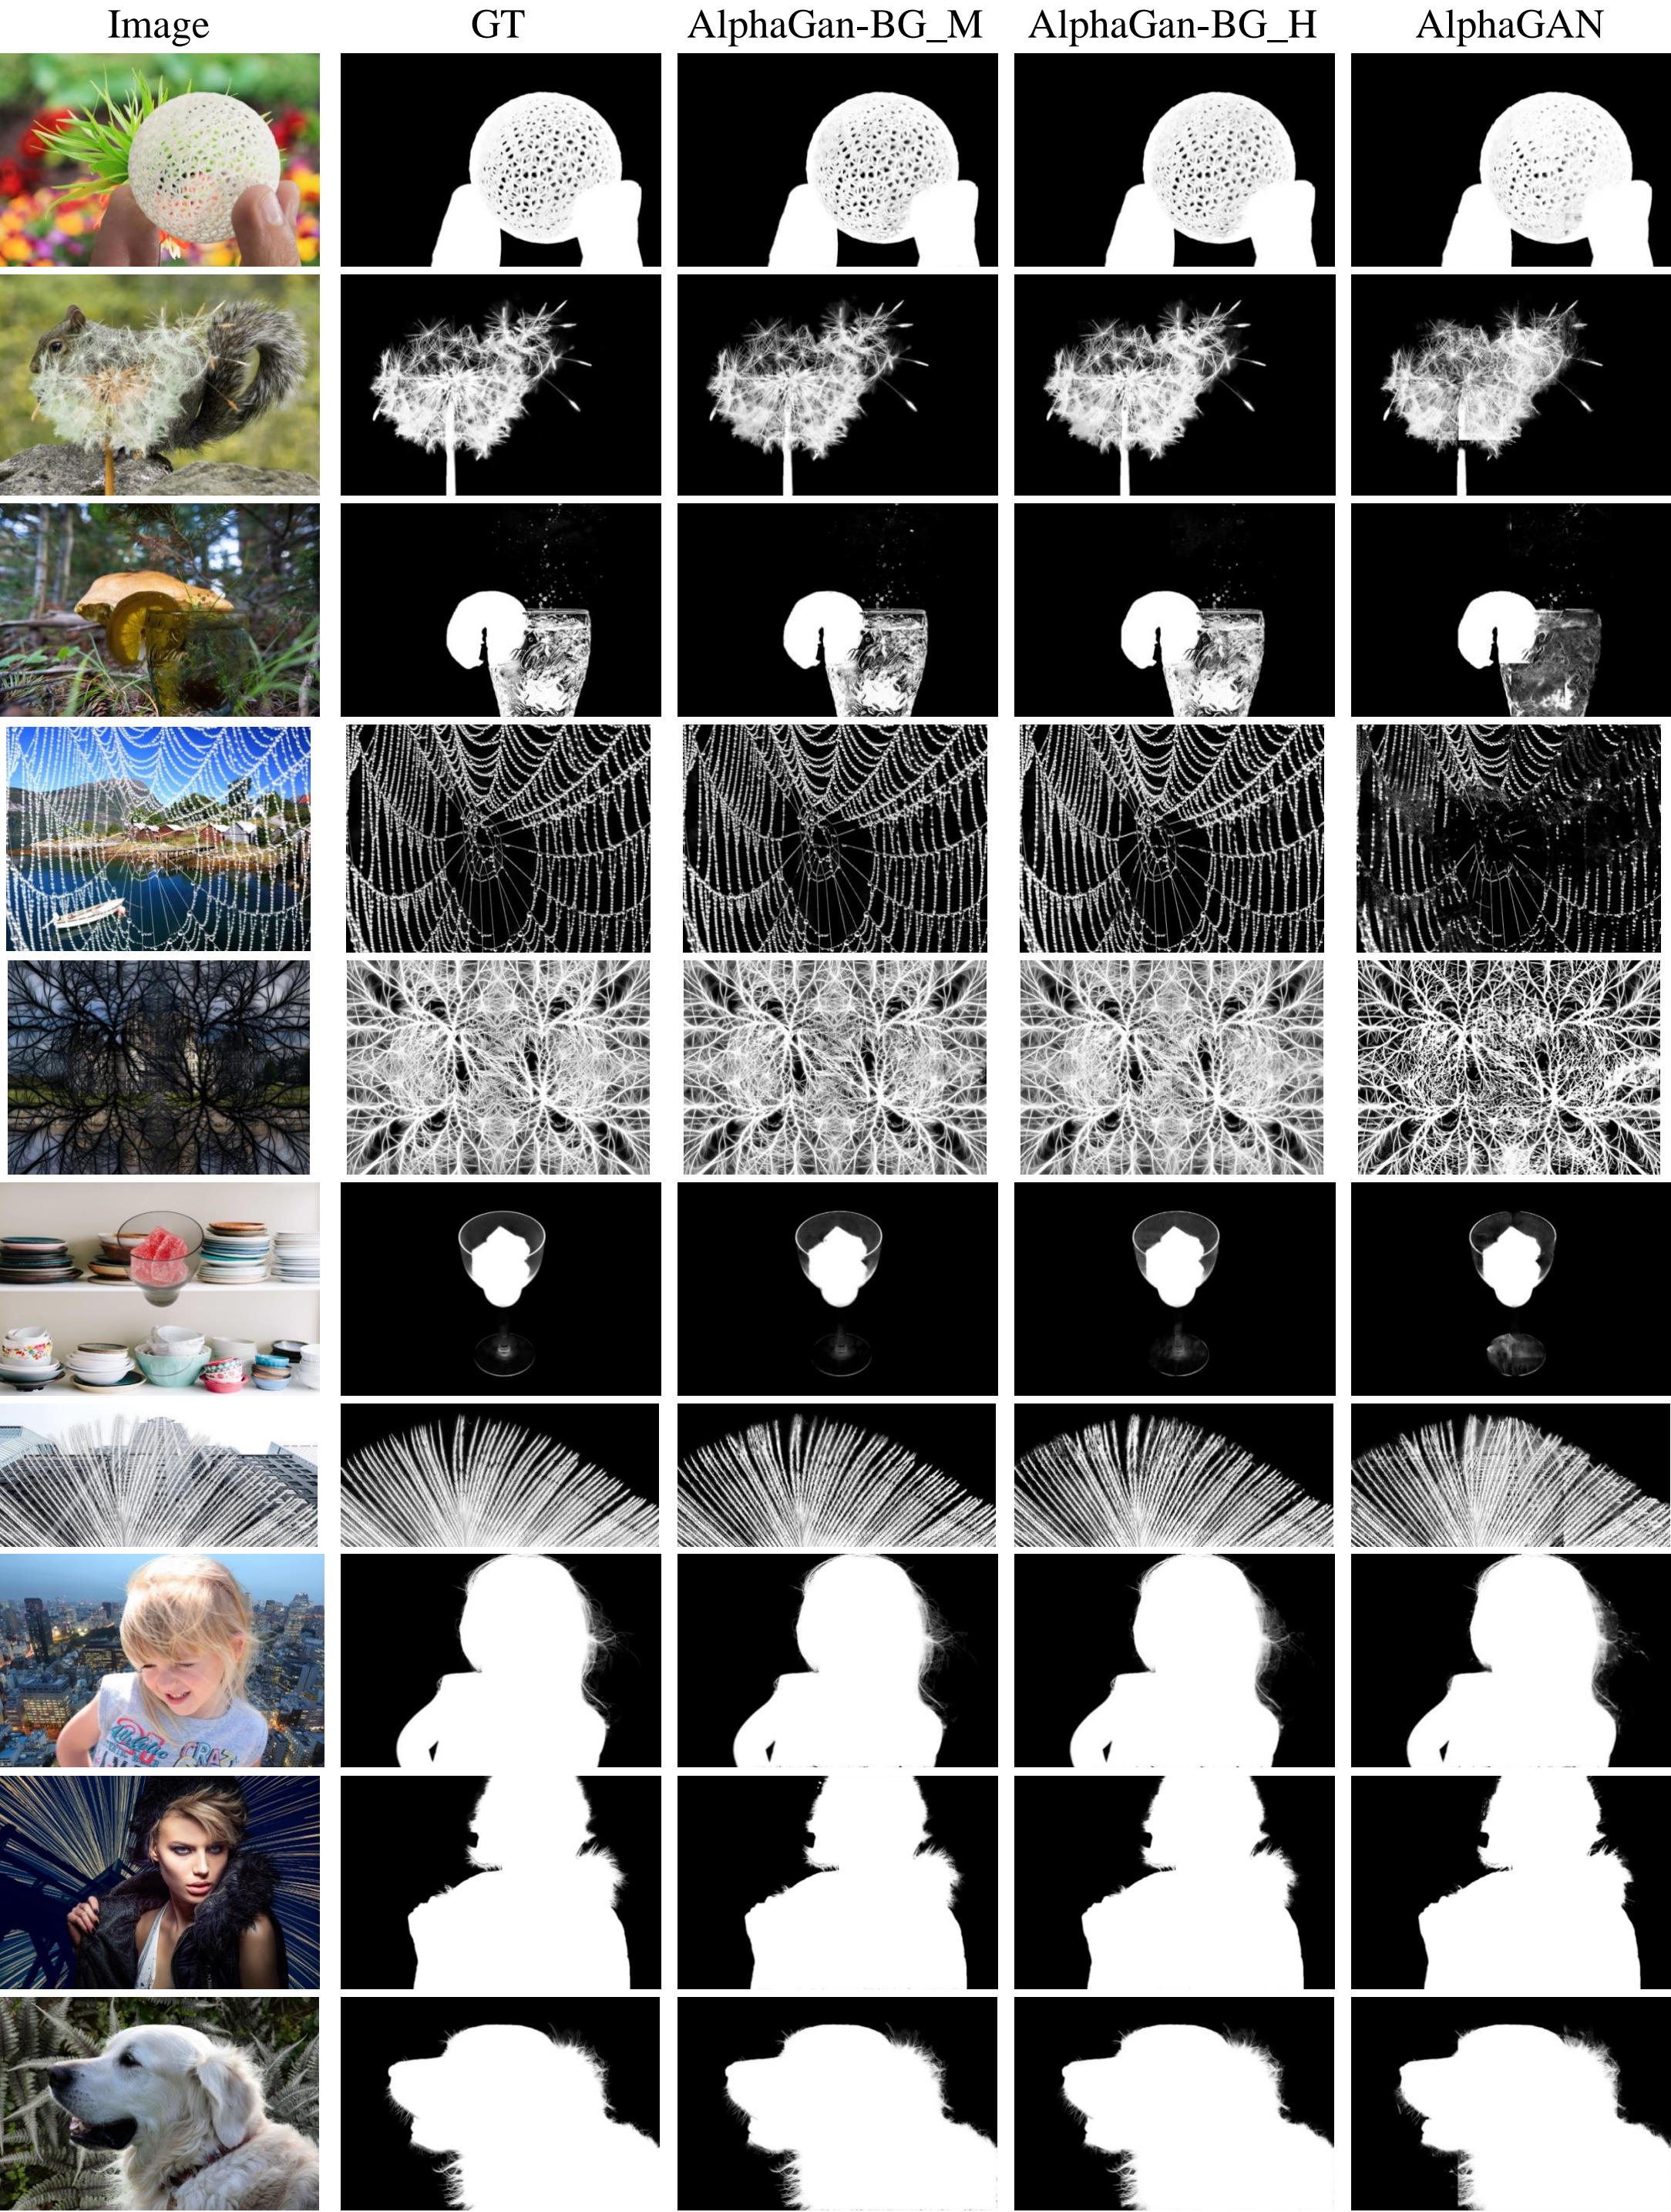 |
| 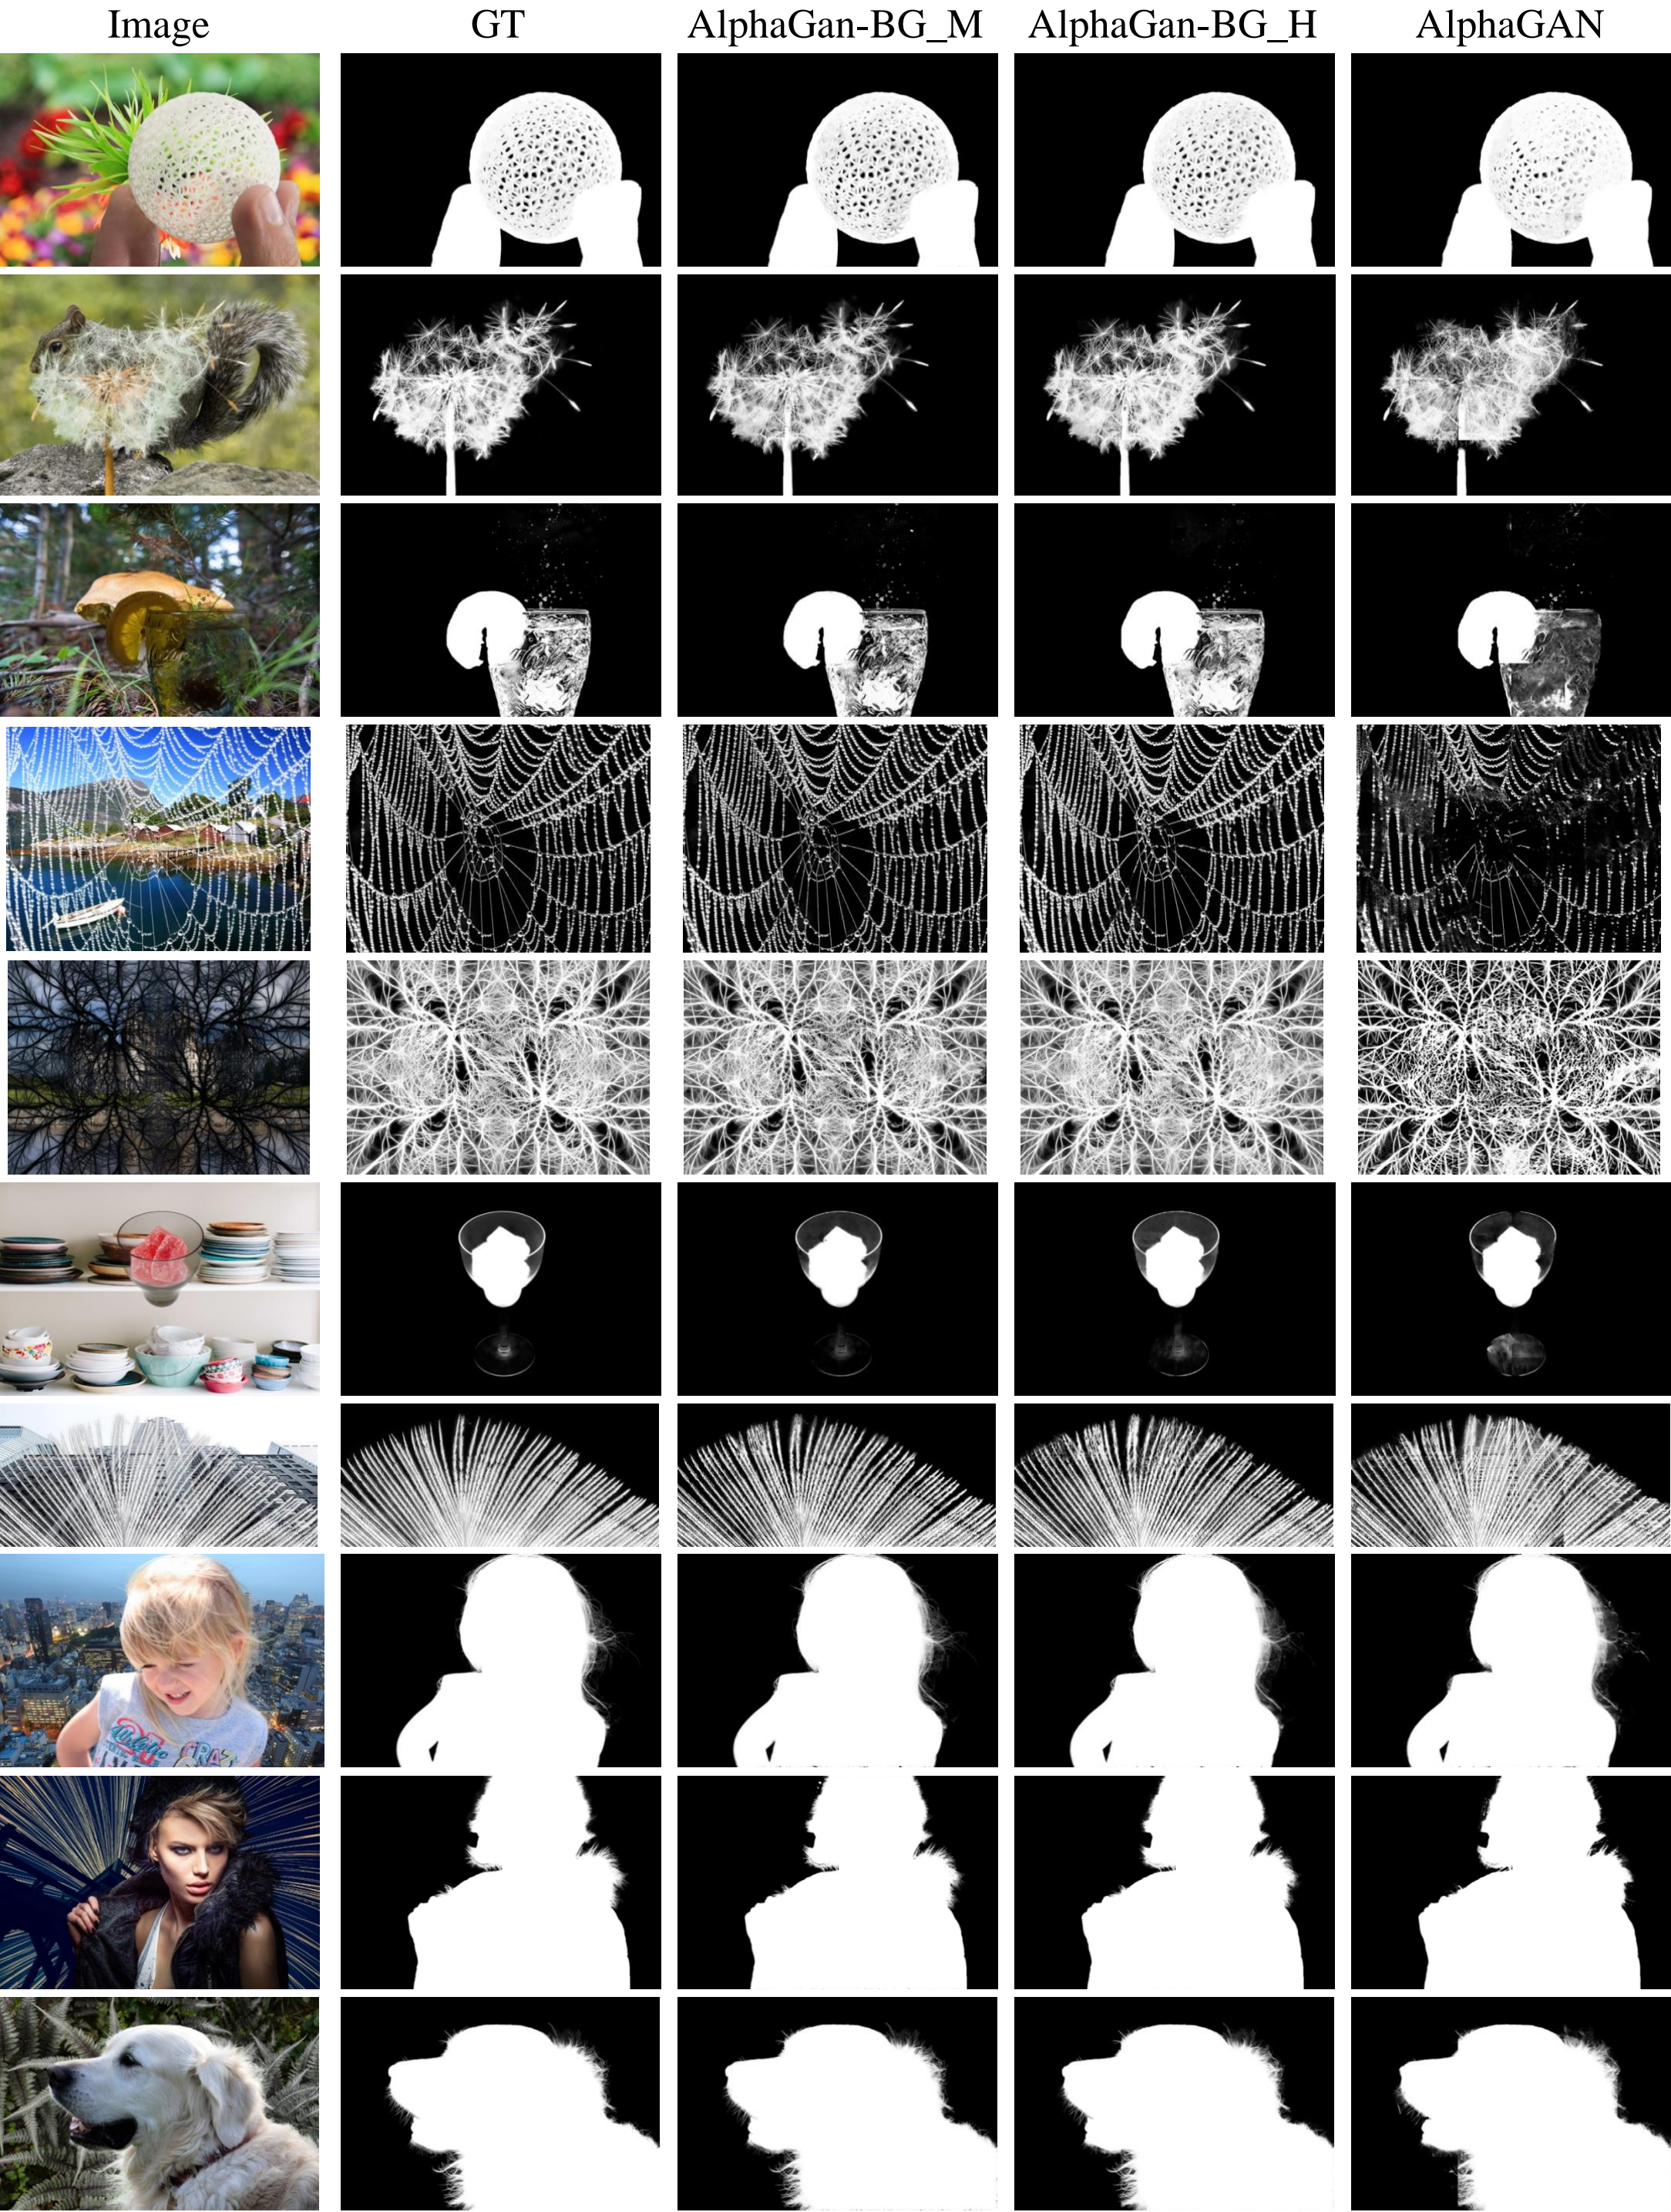 | 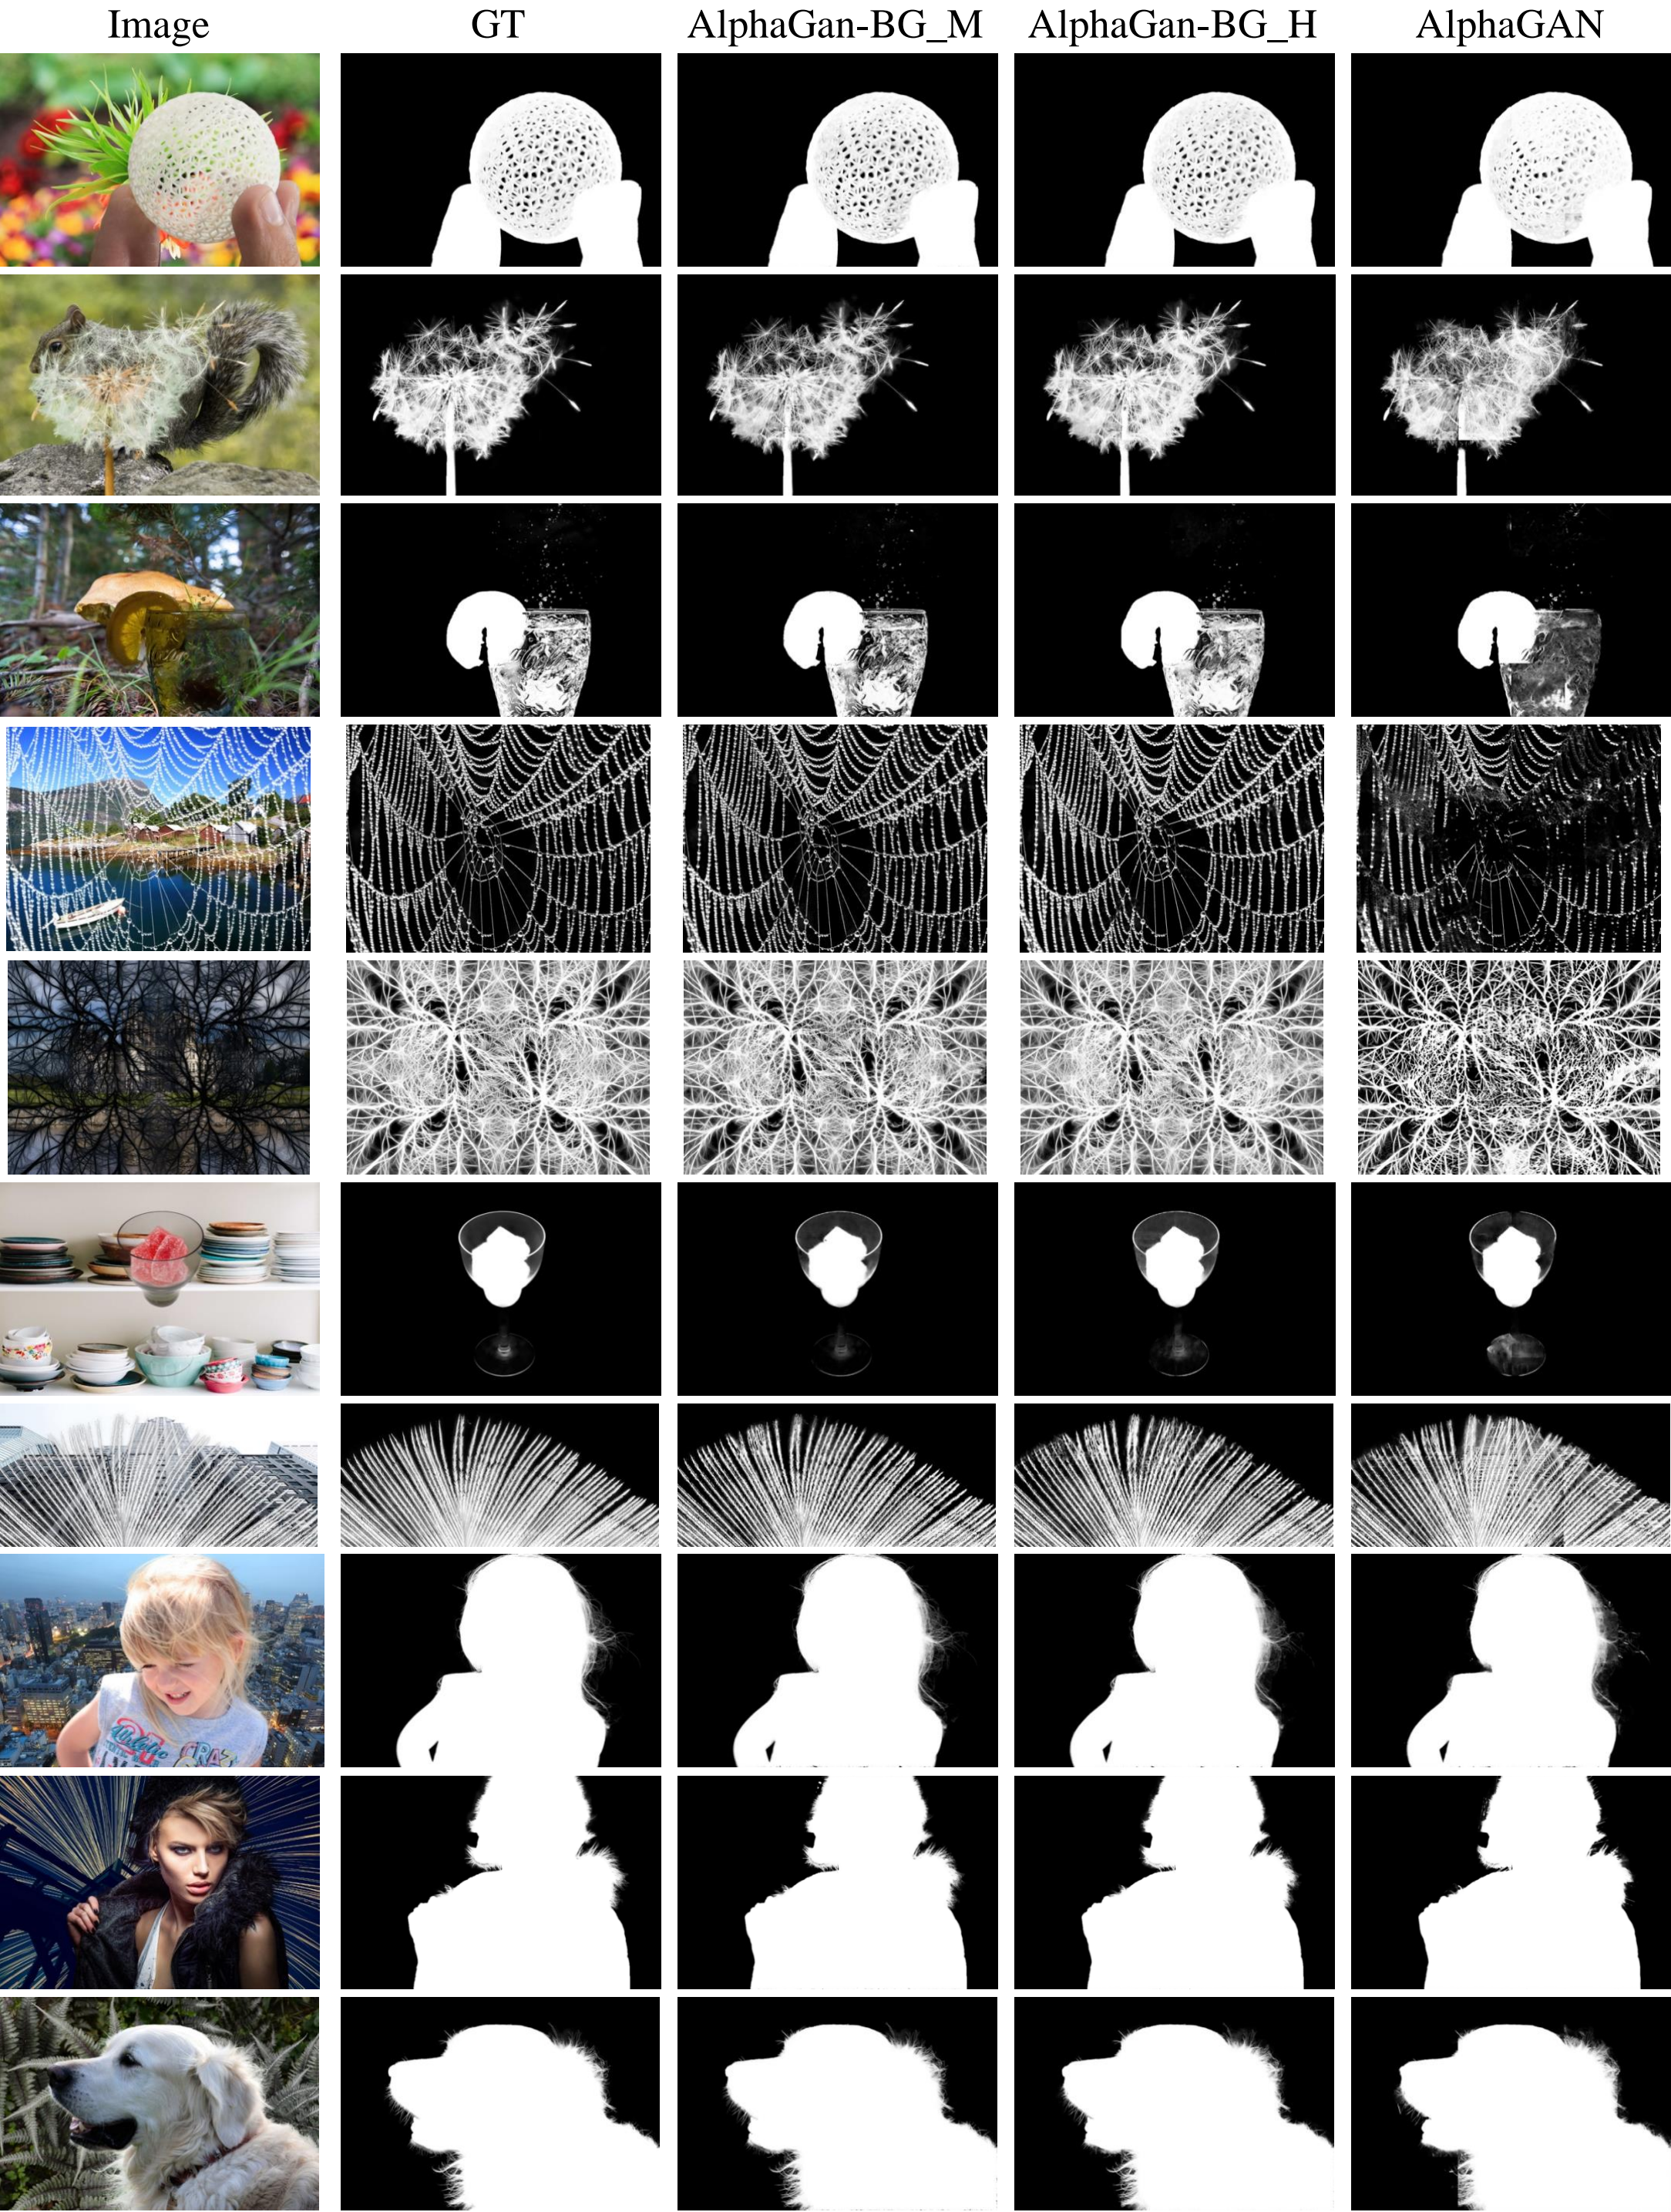 | 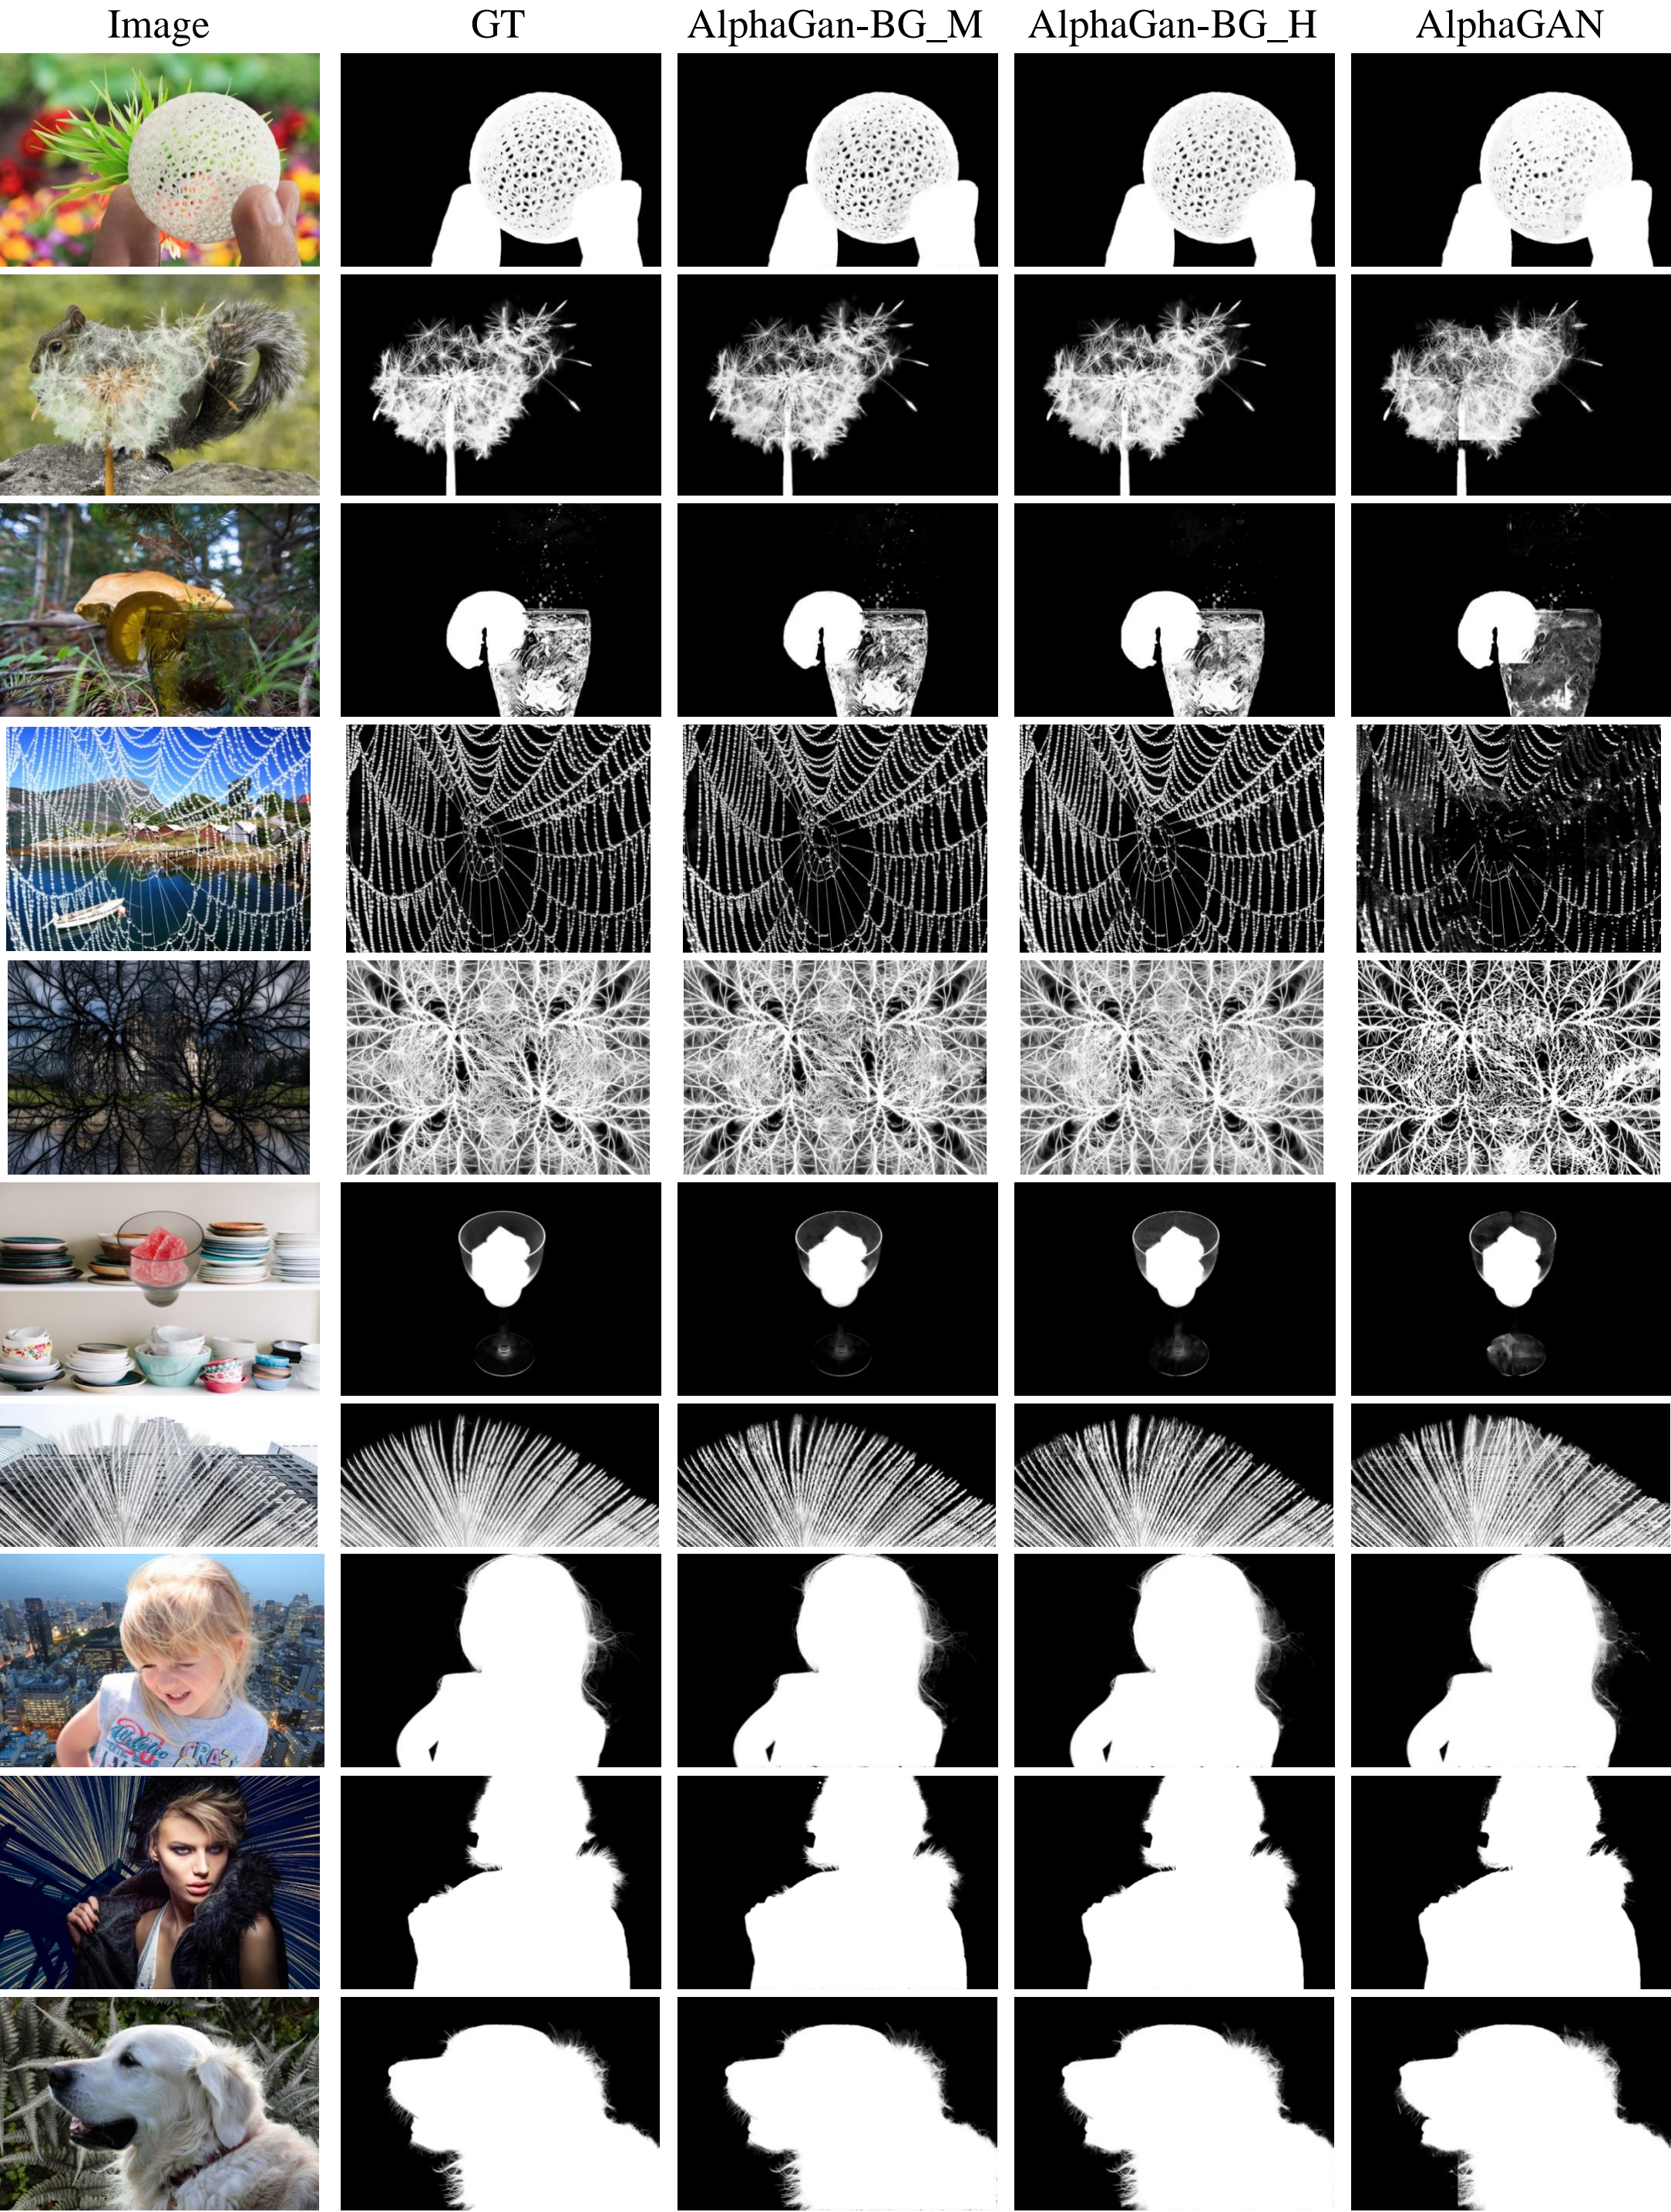 | 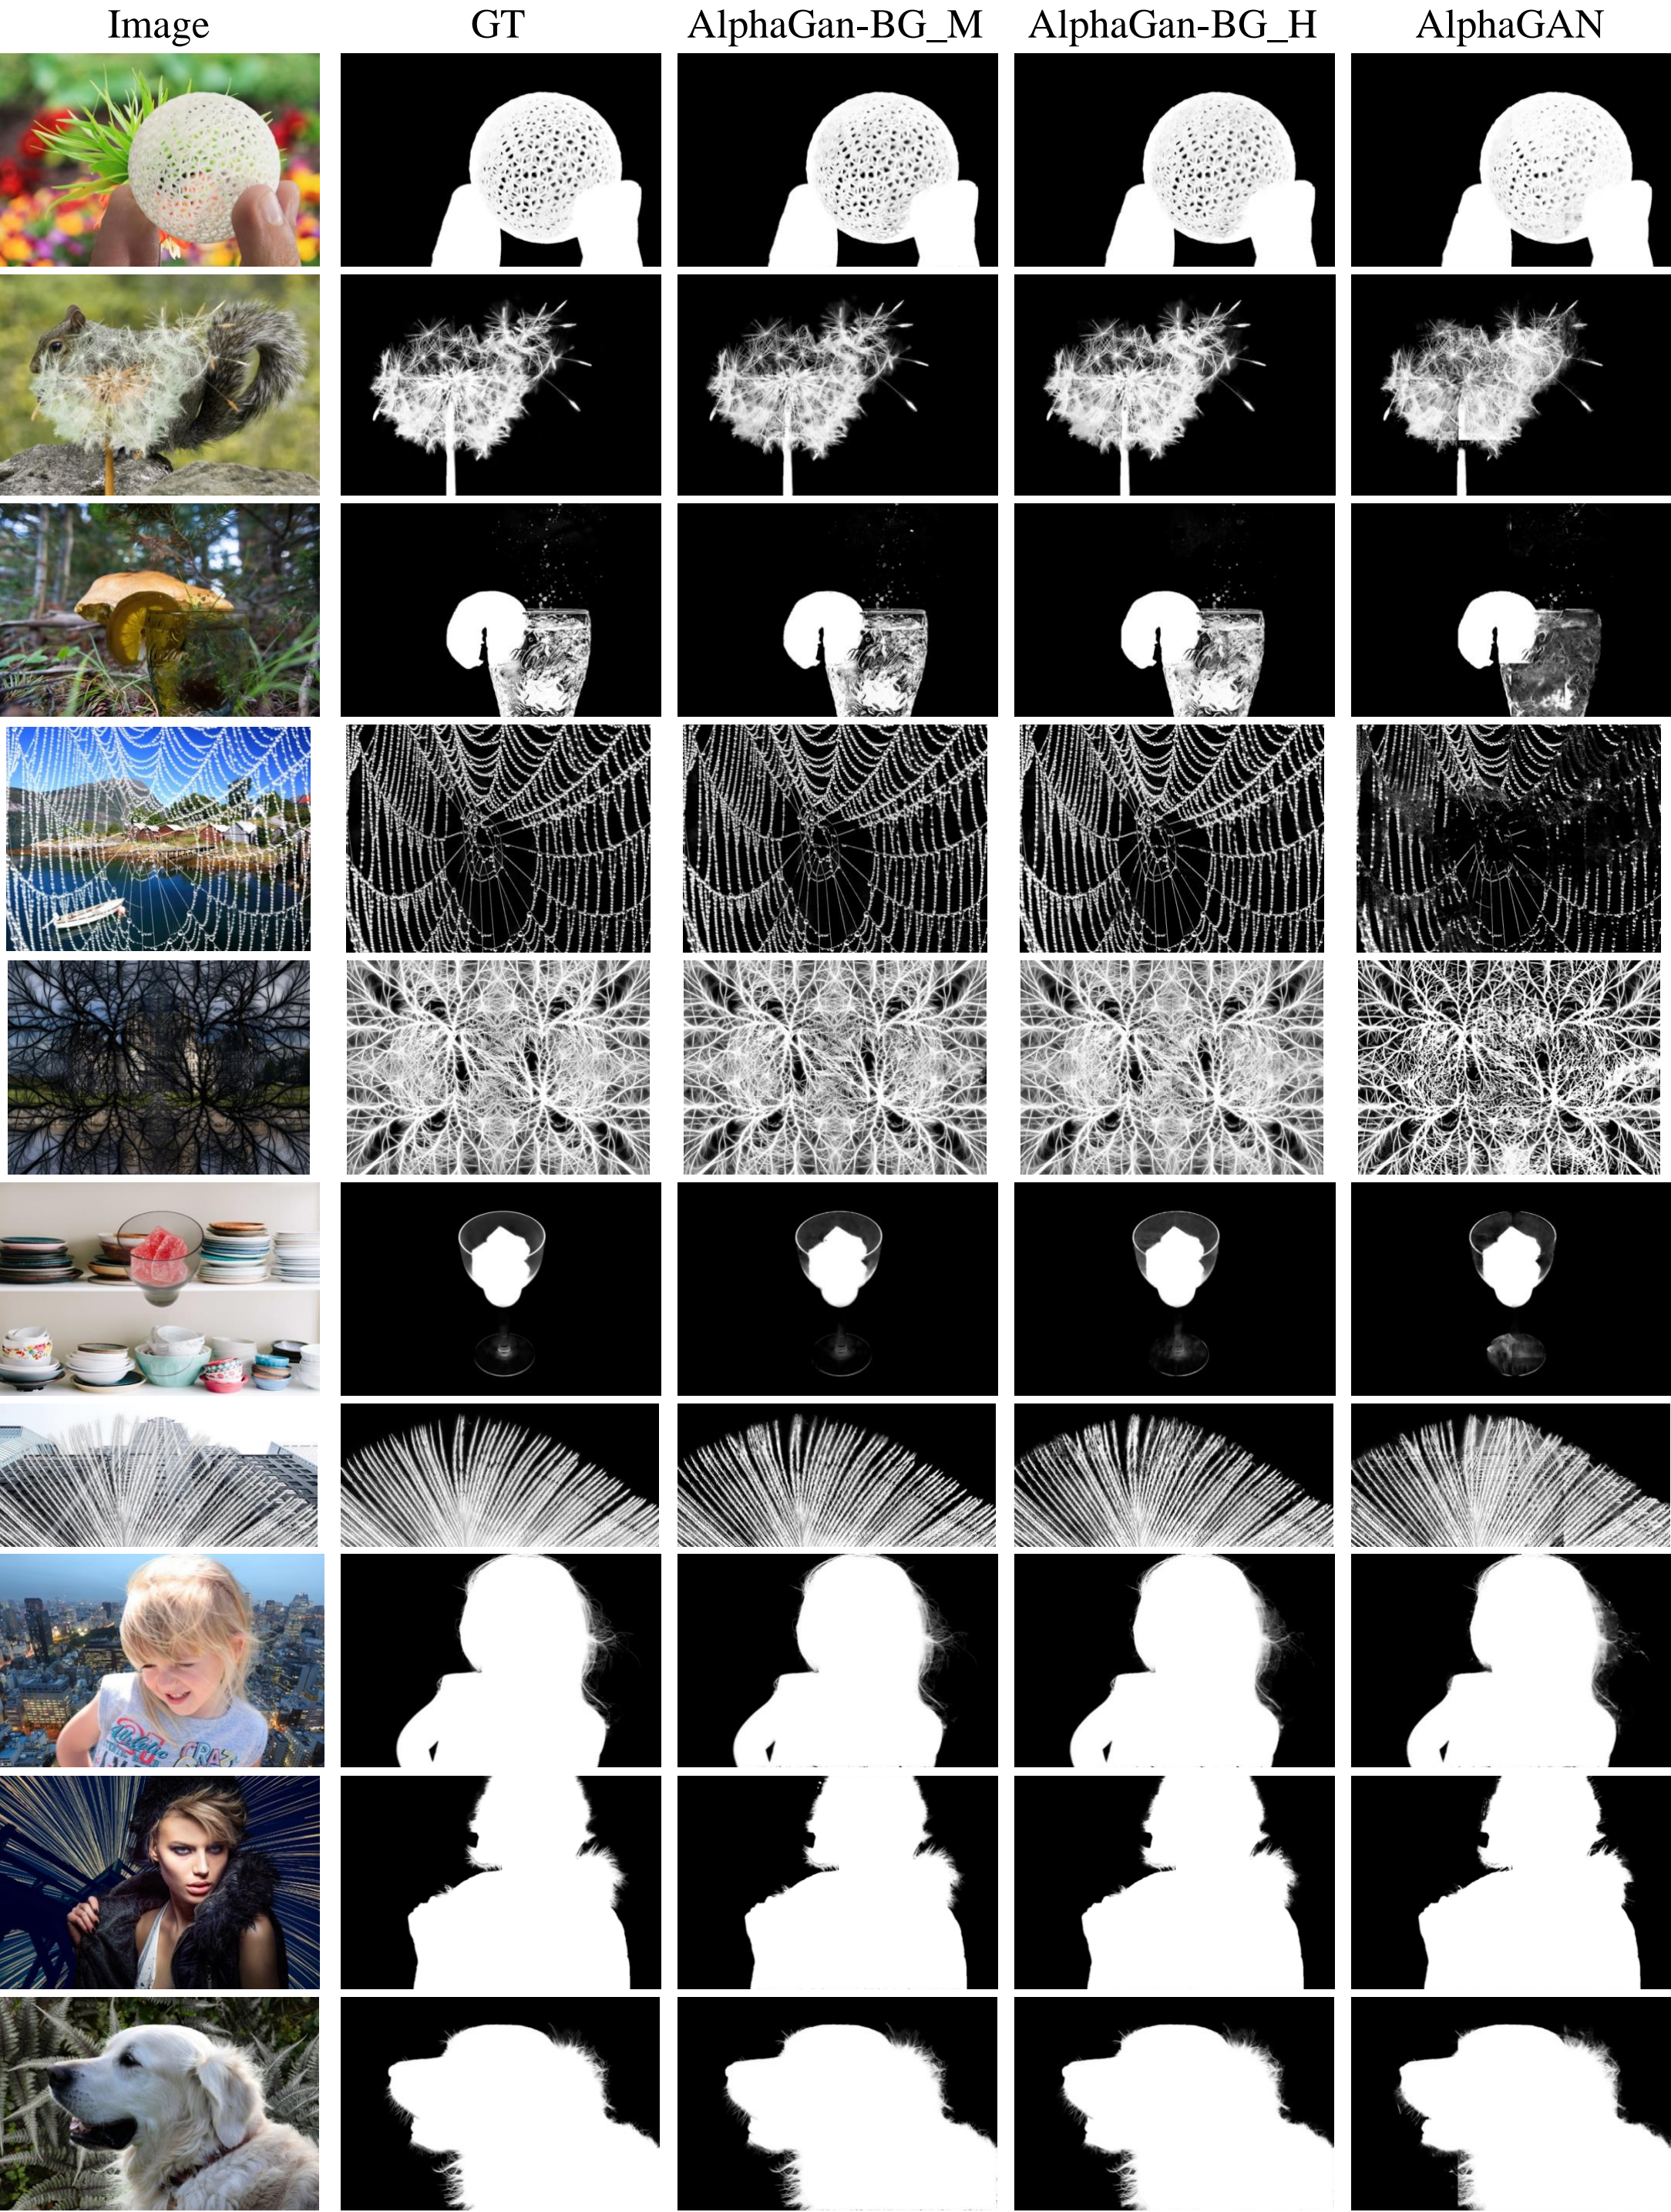 | 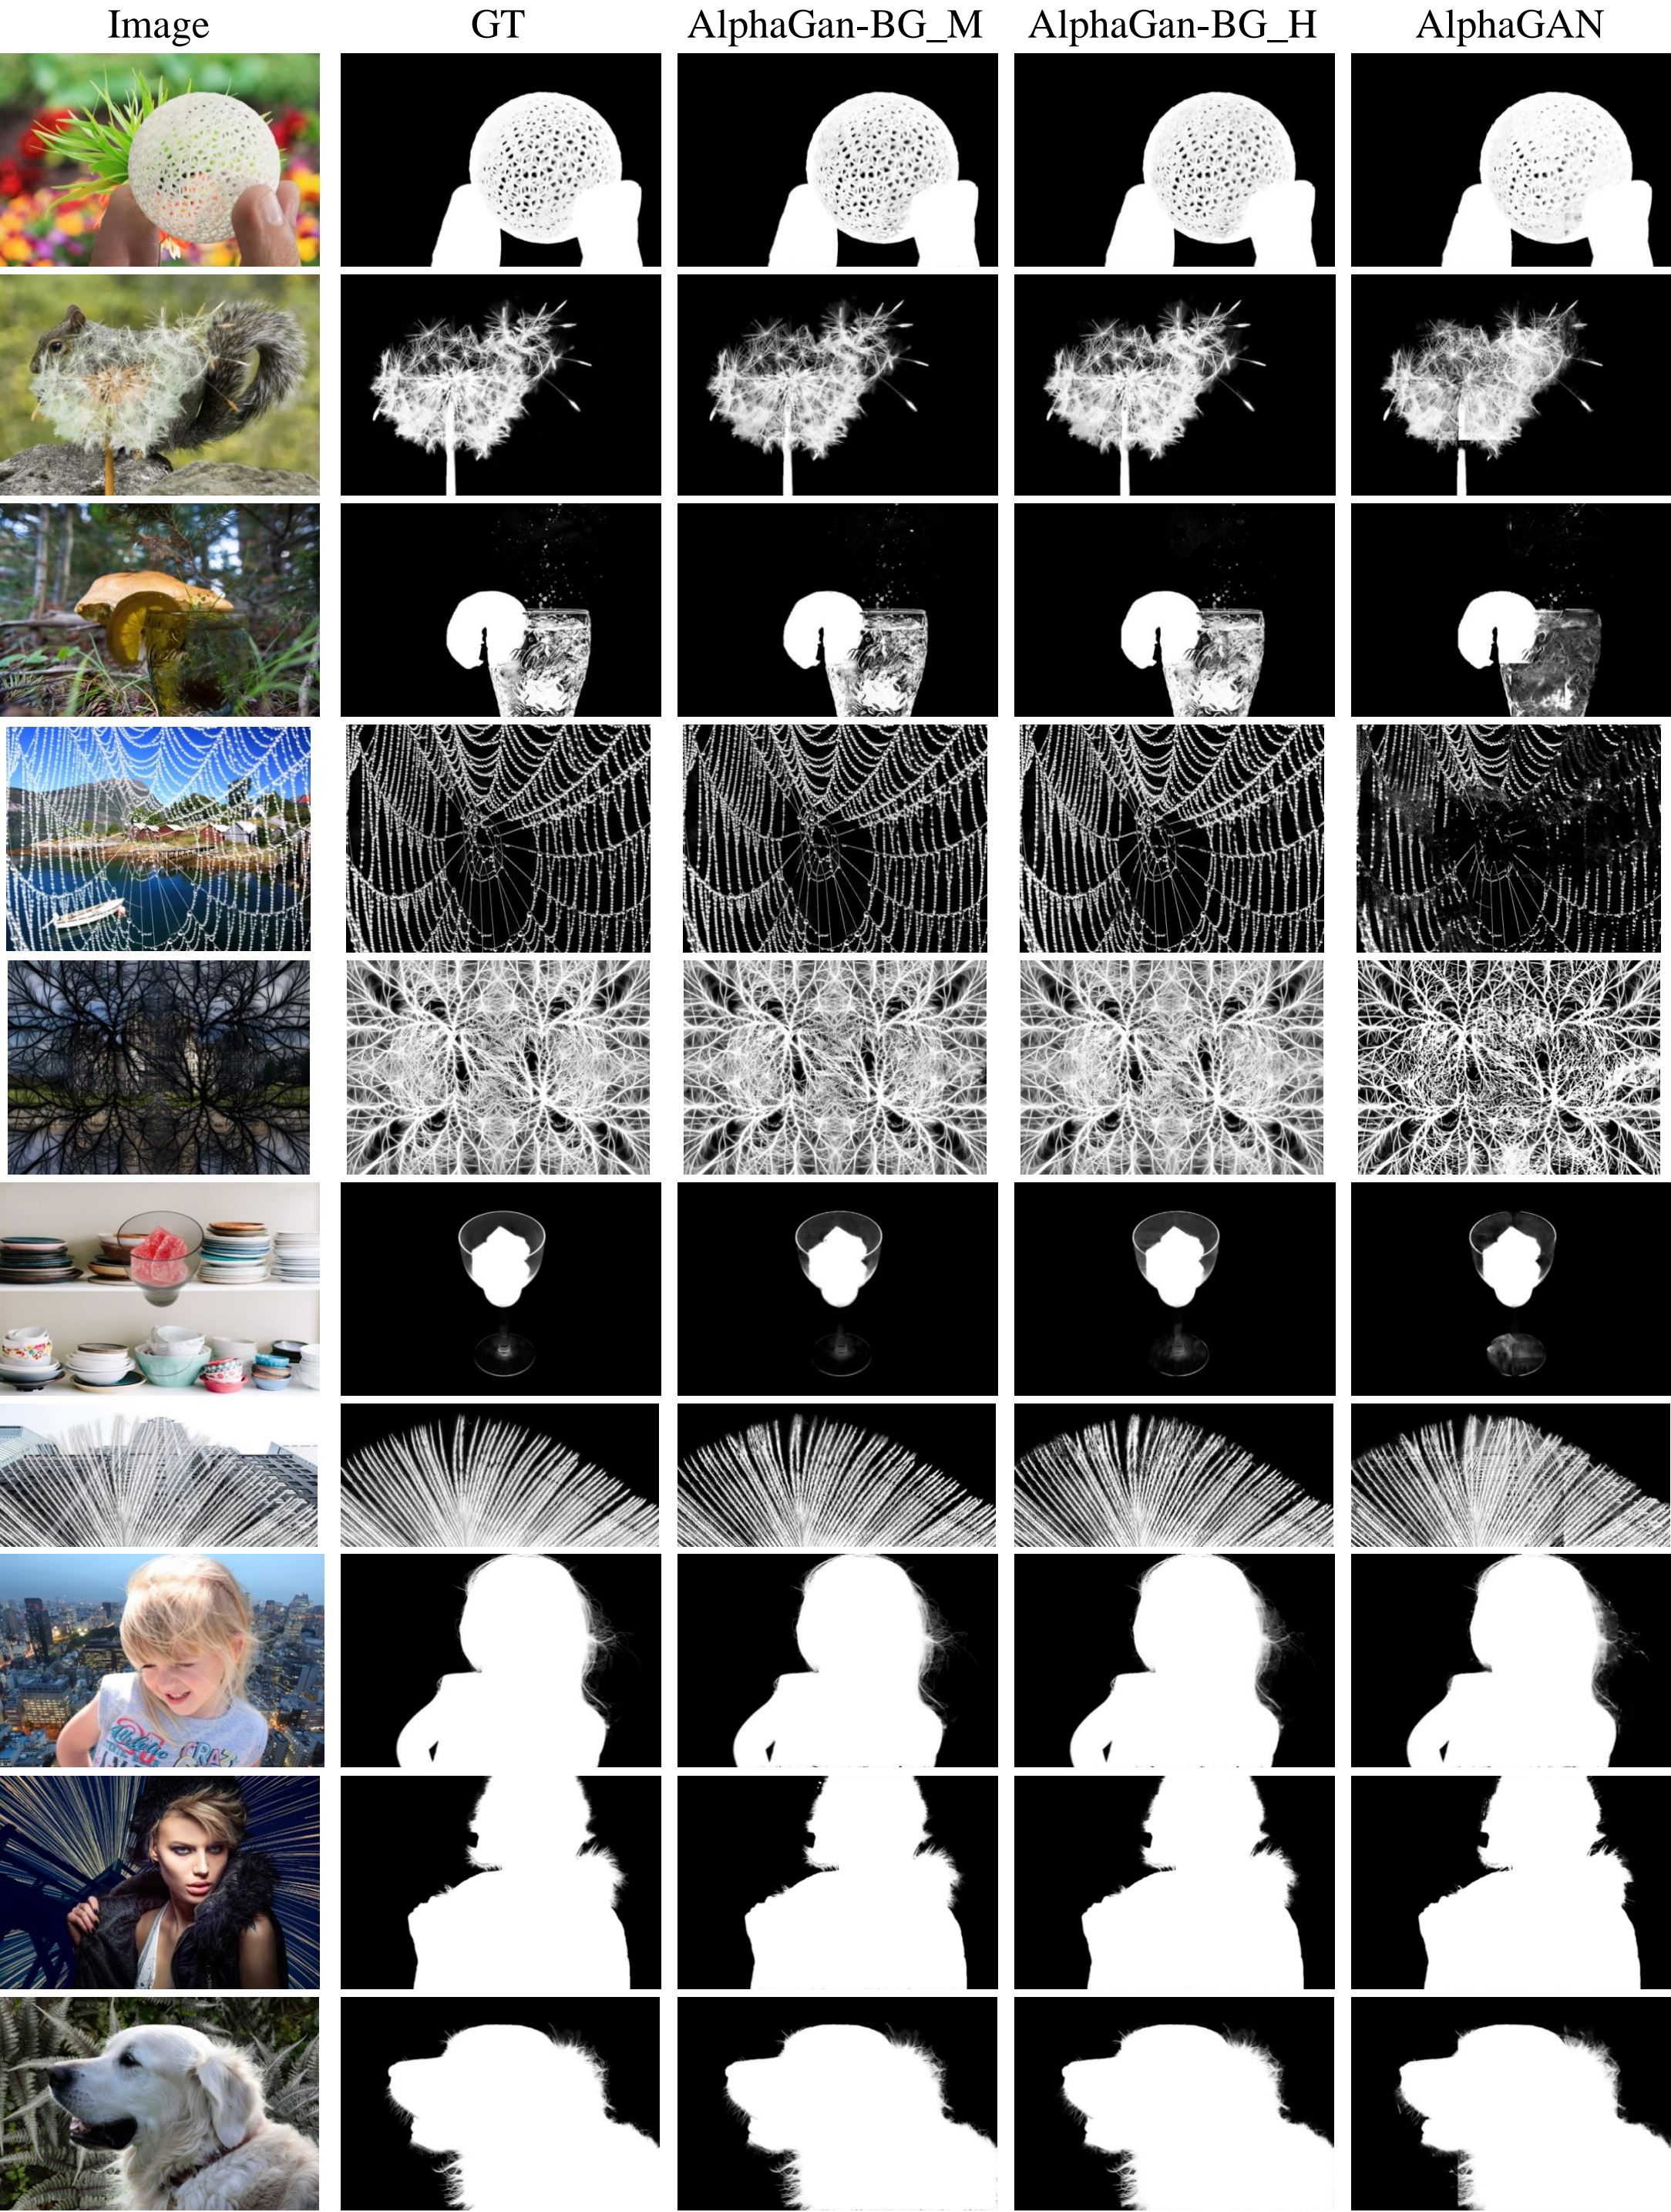 |
| 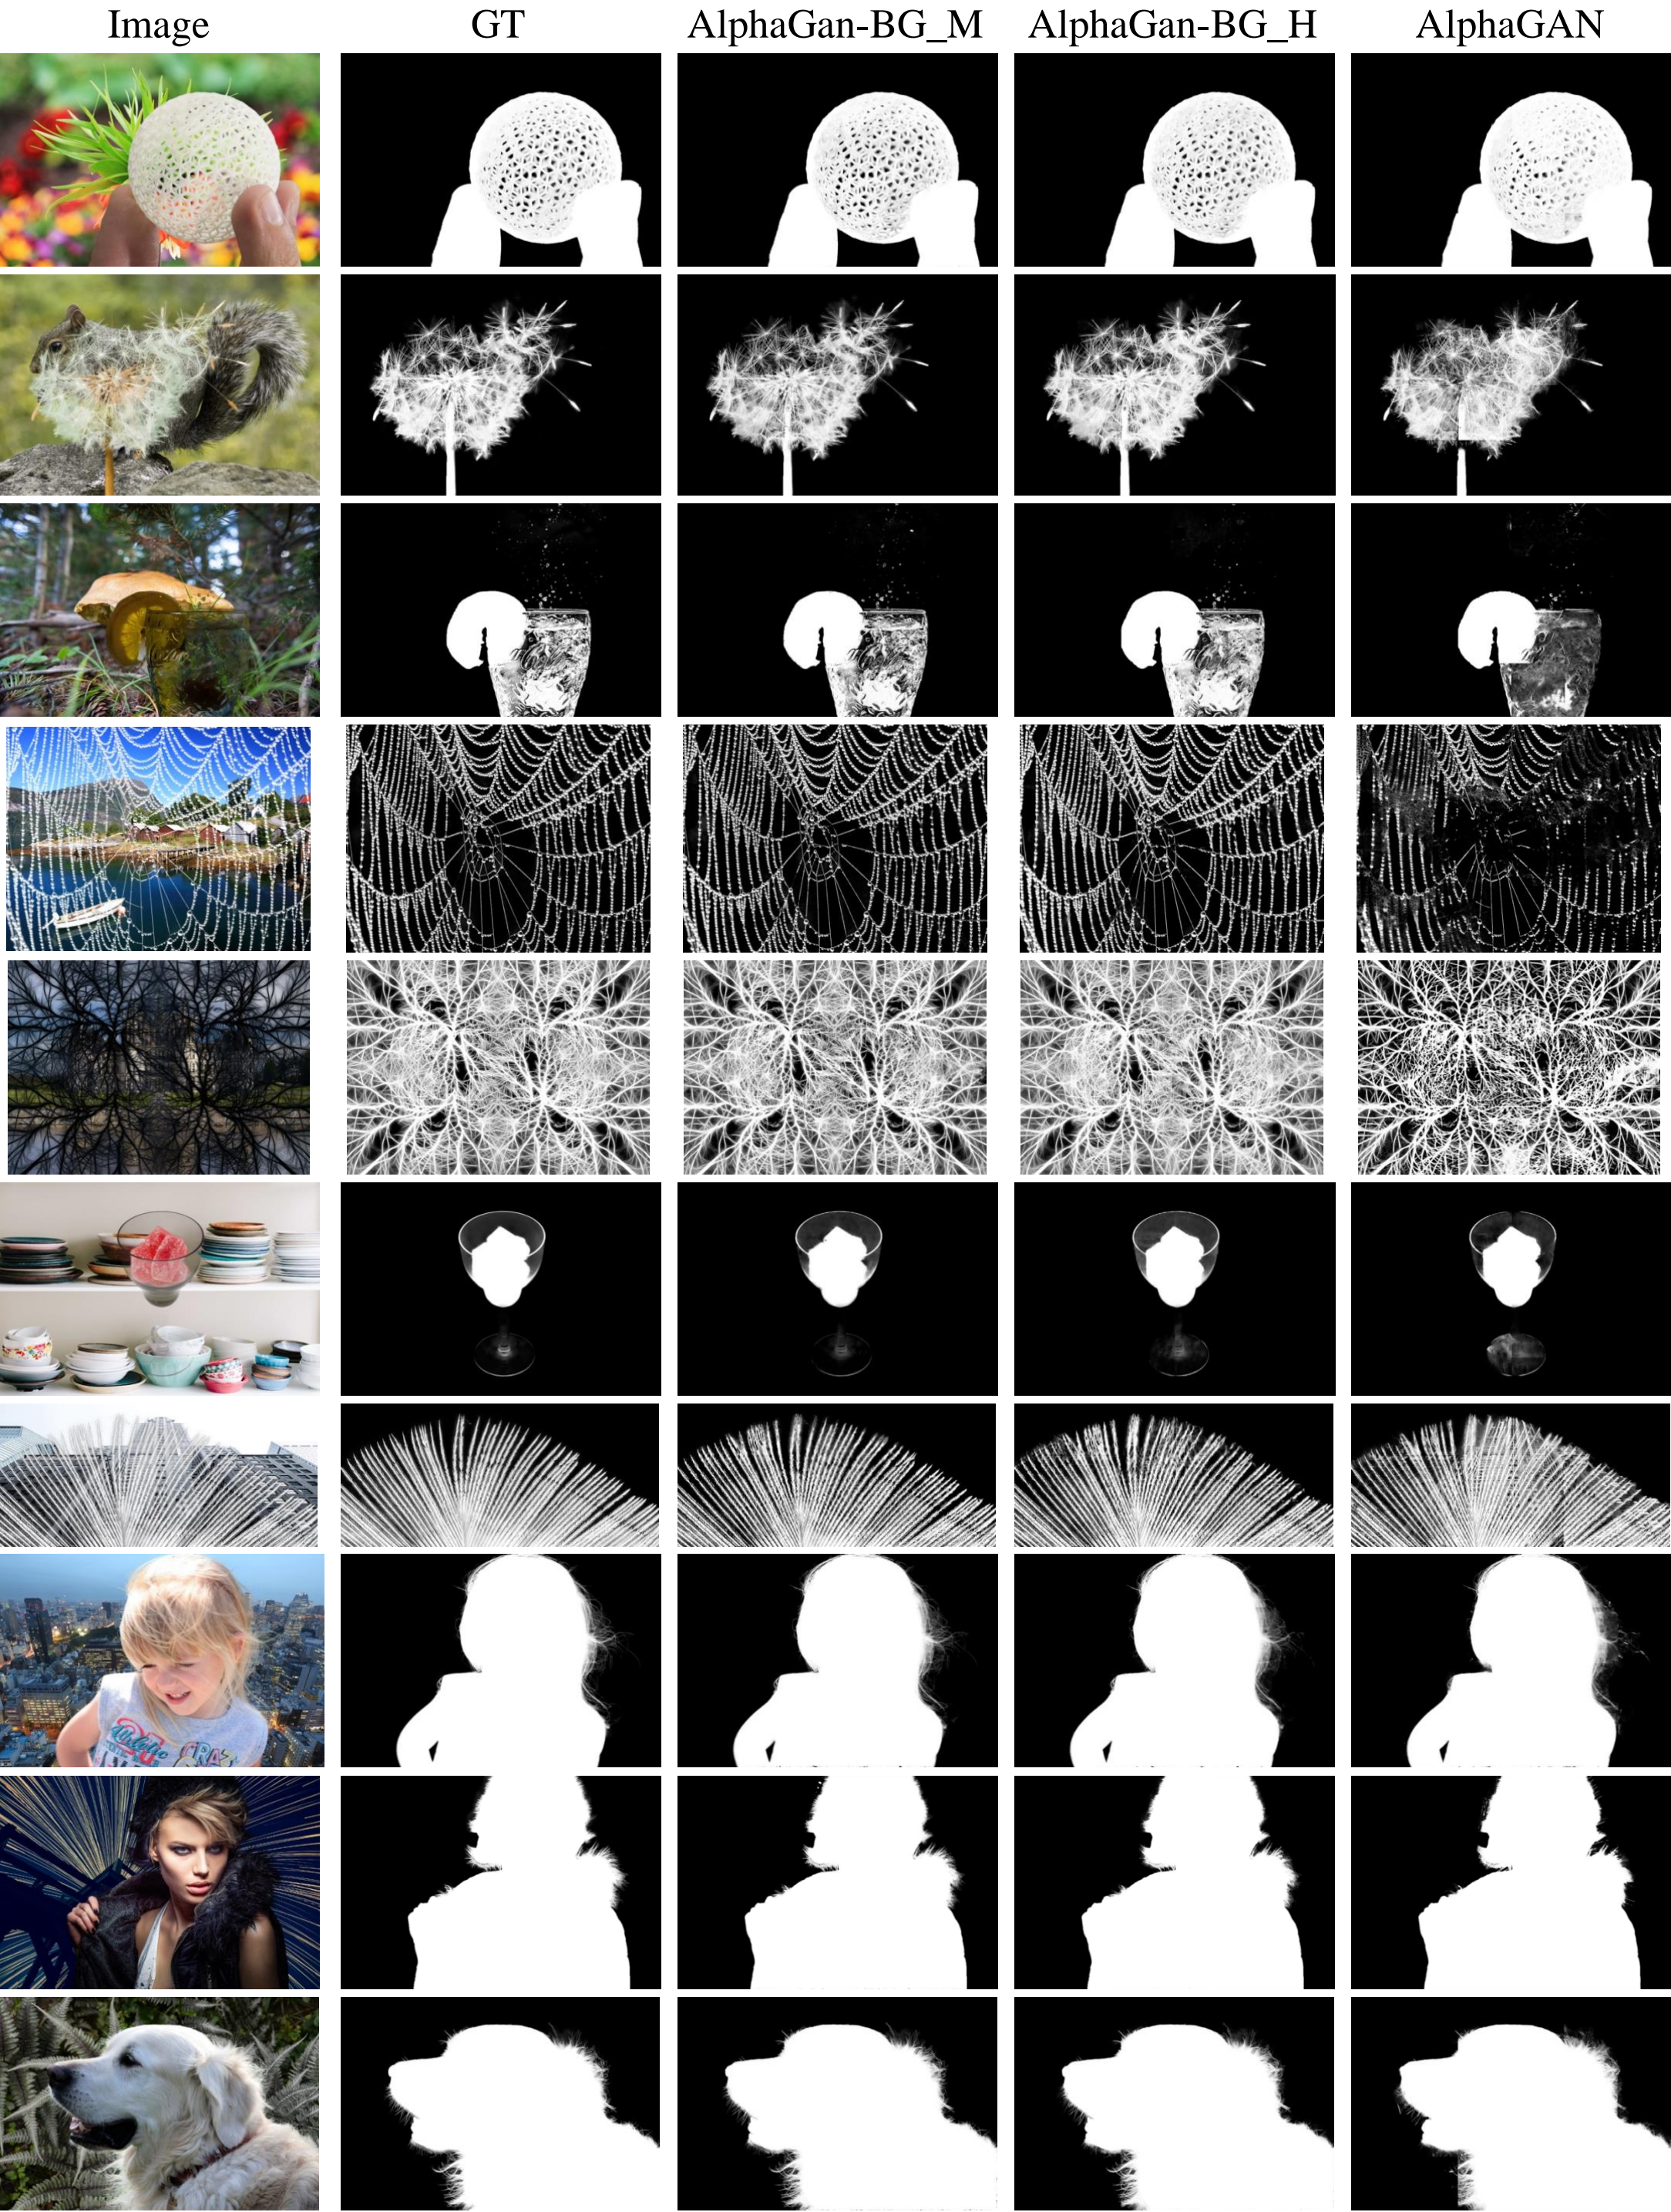 | 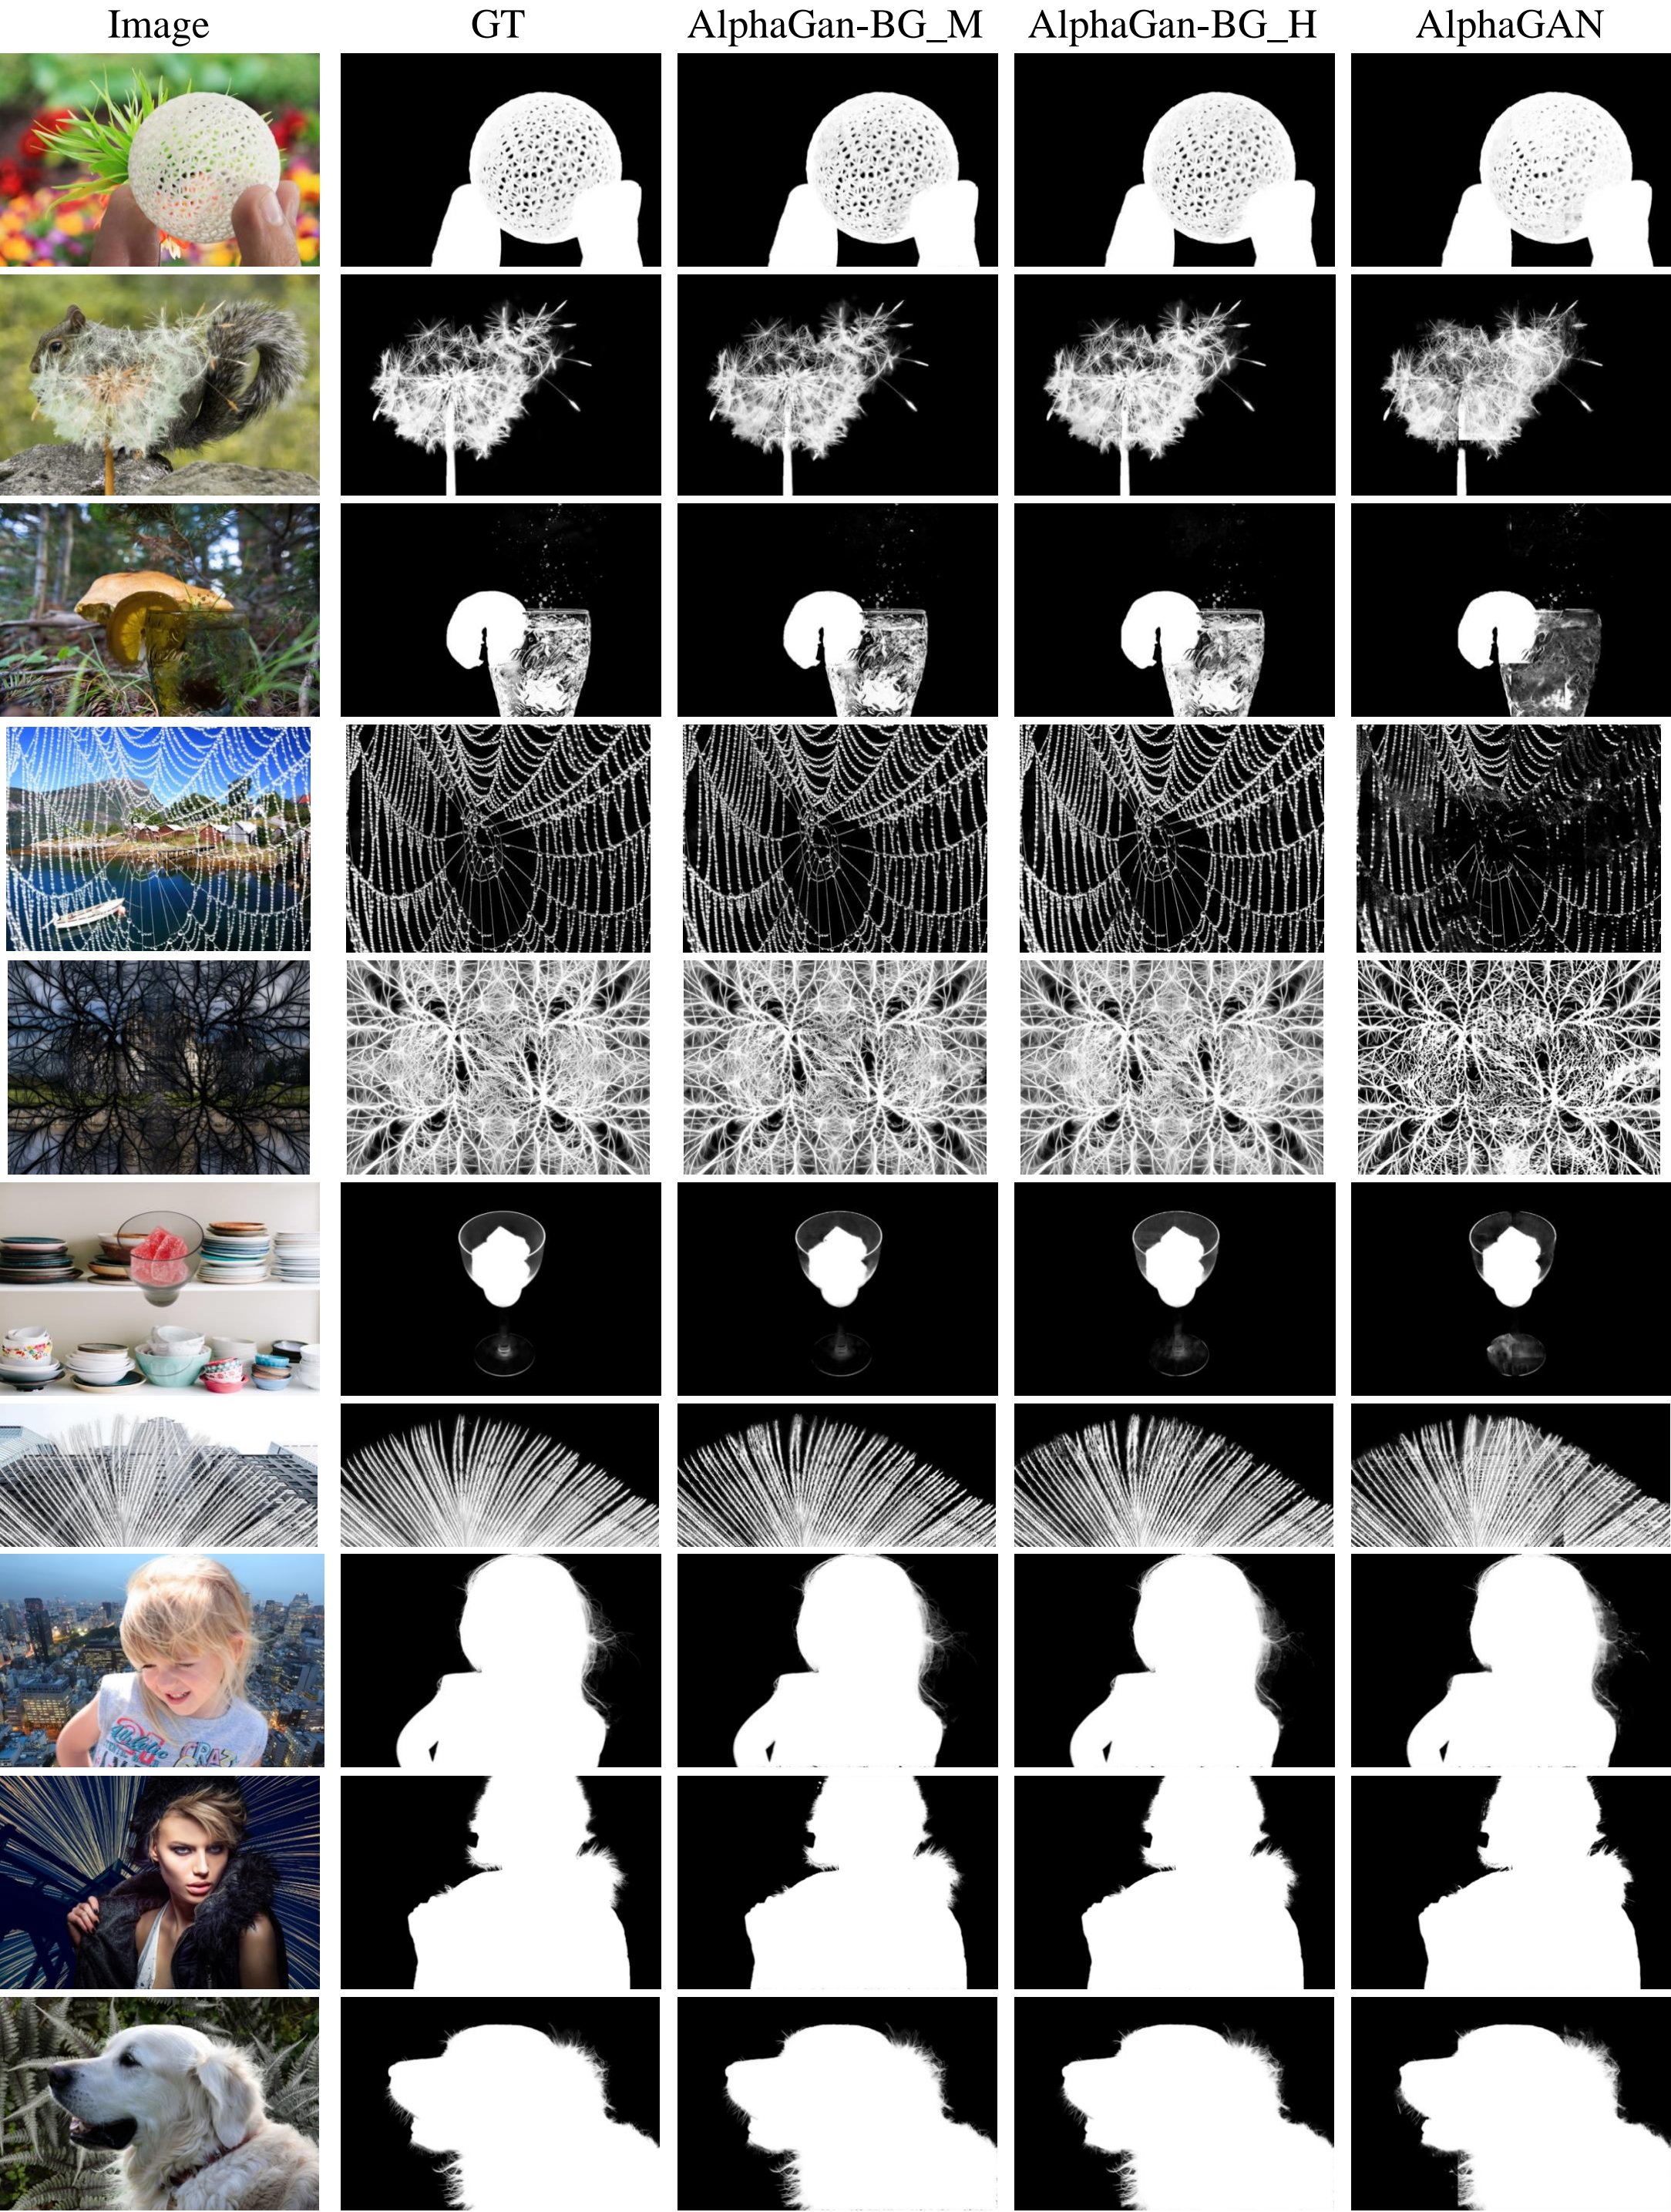 | 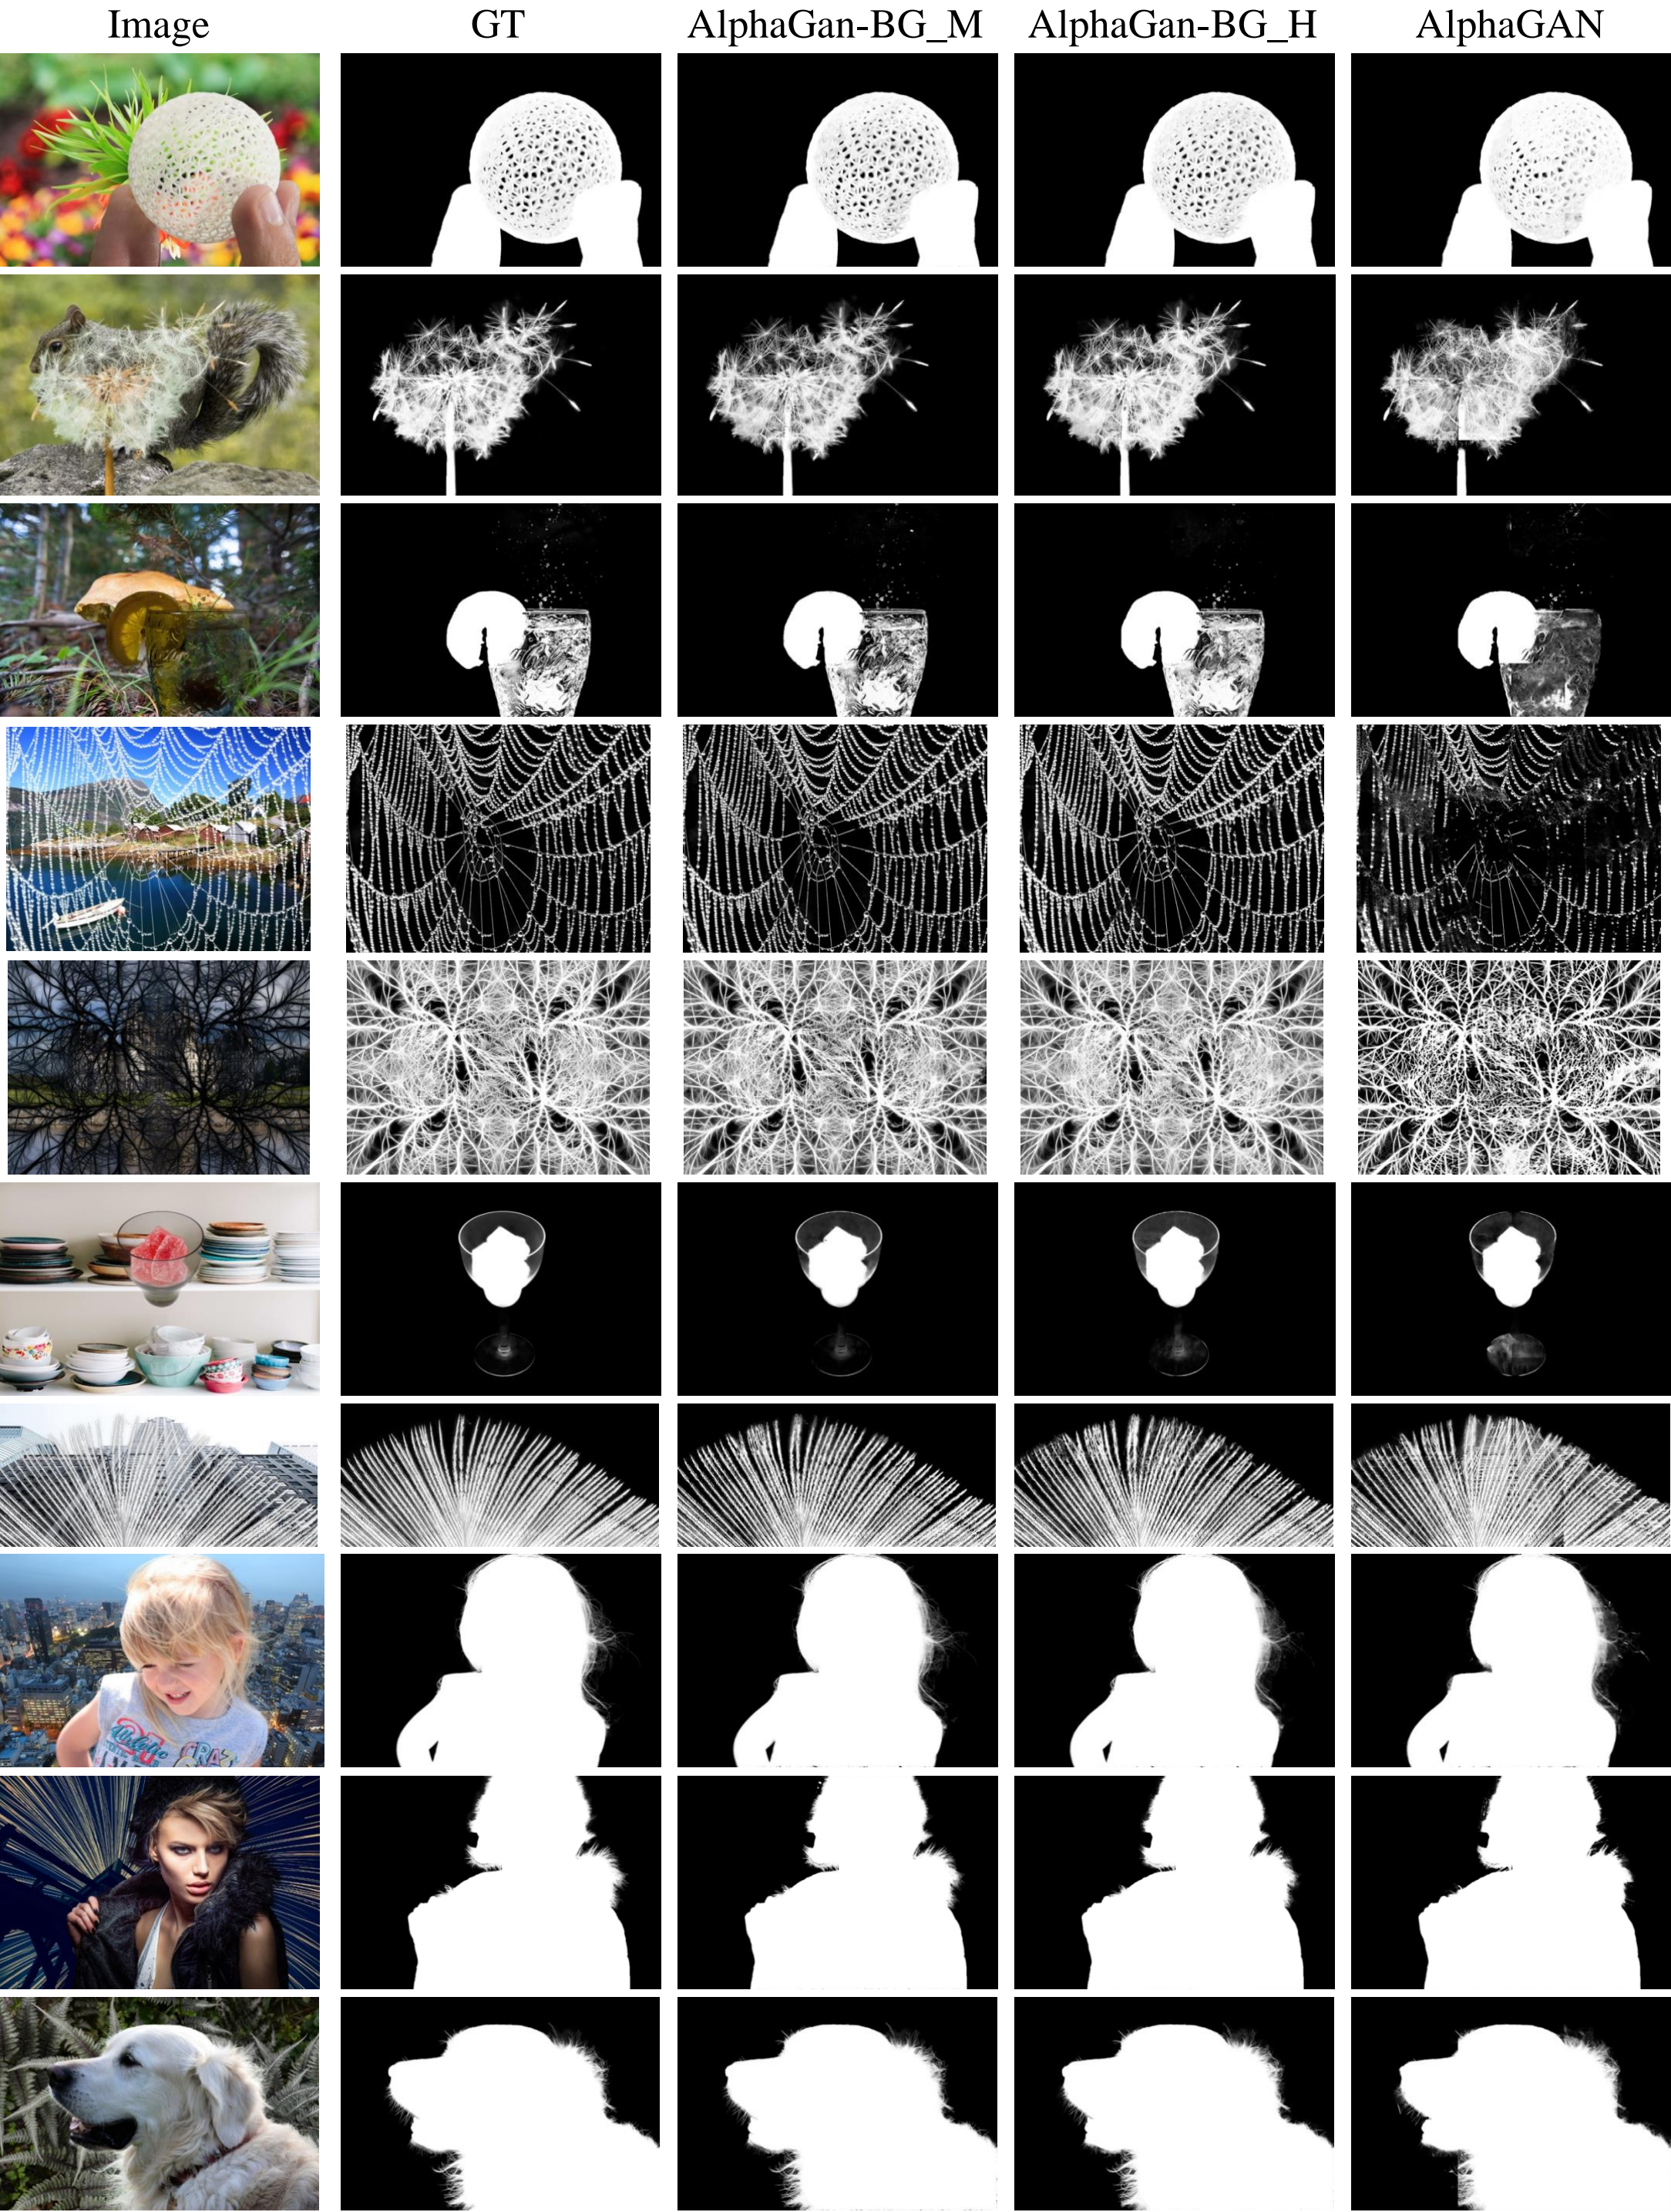 | 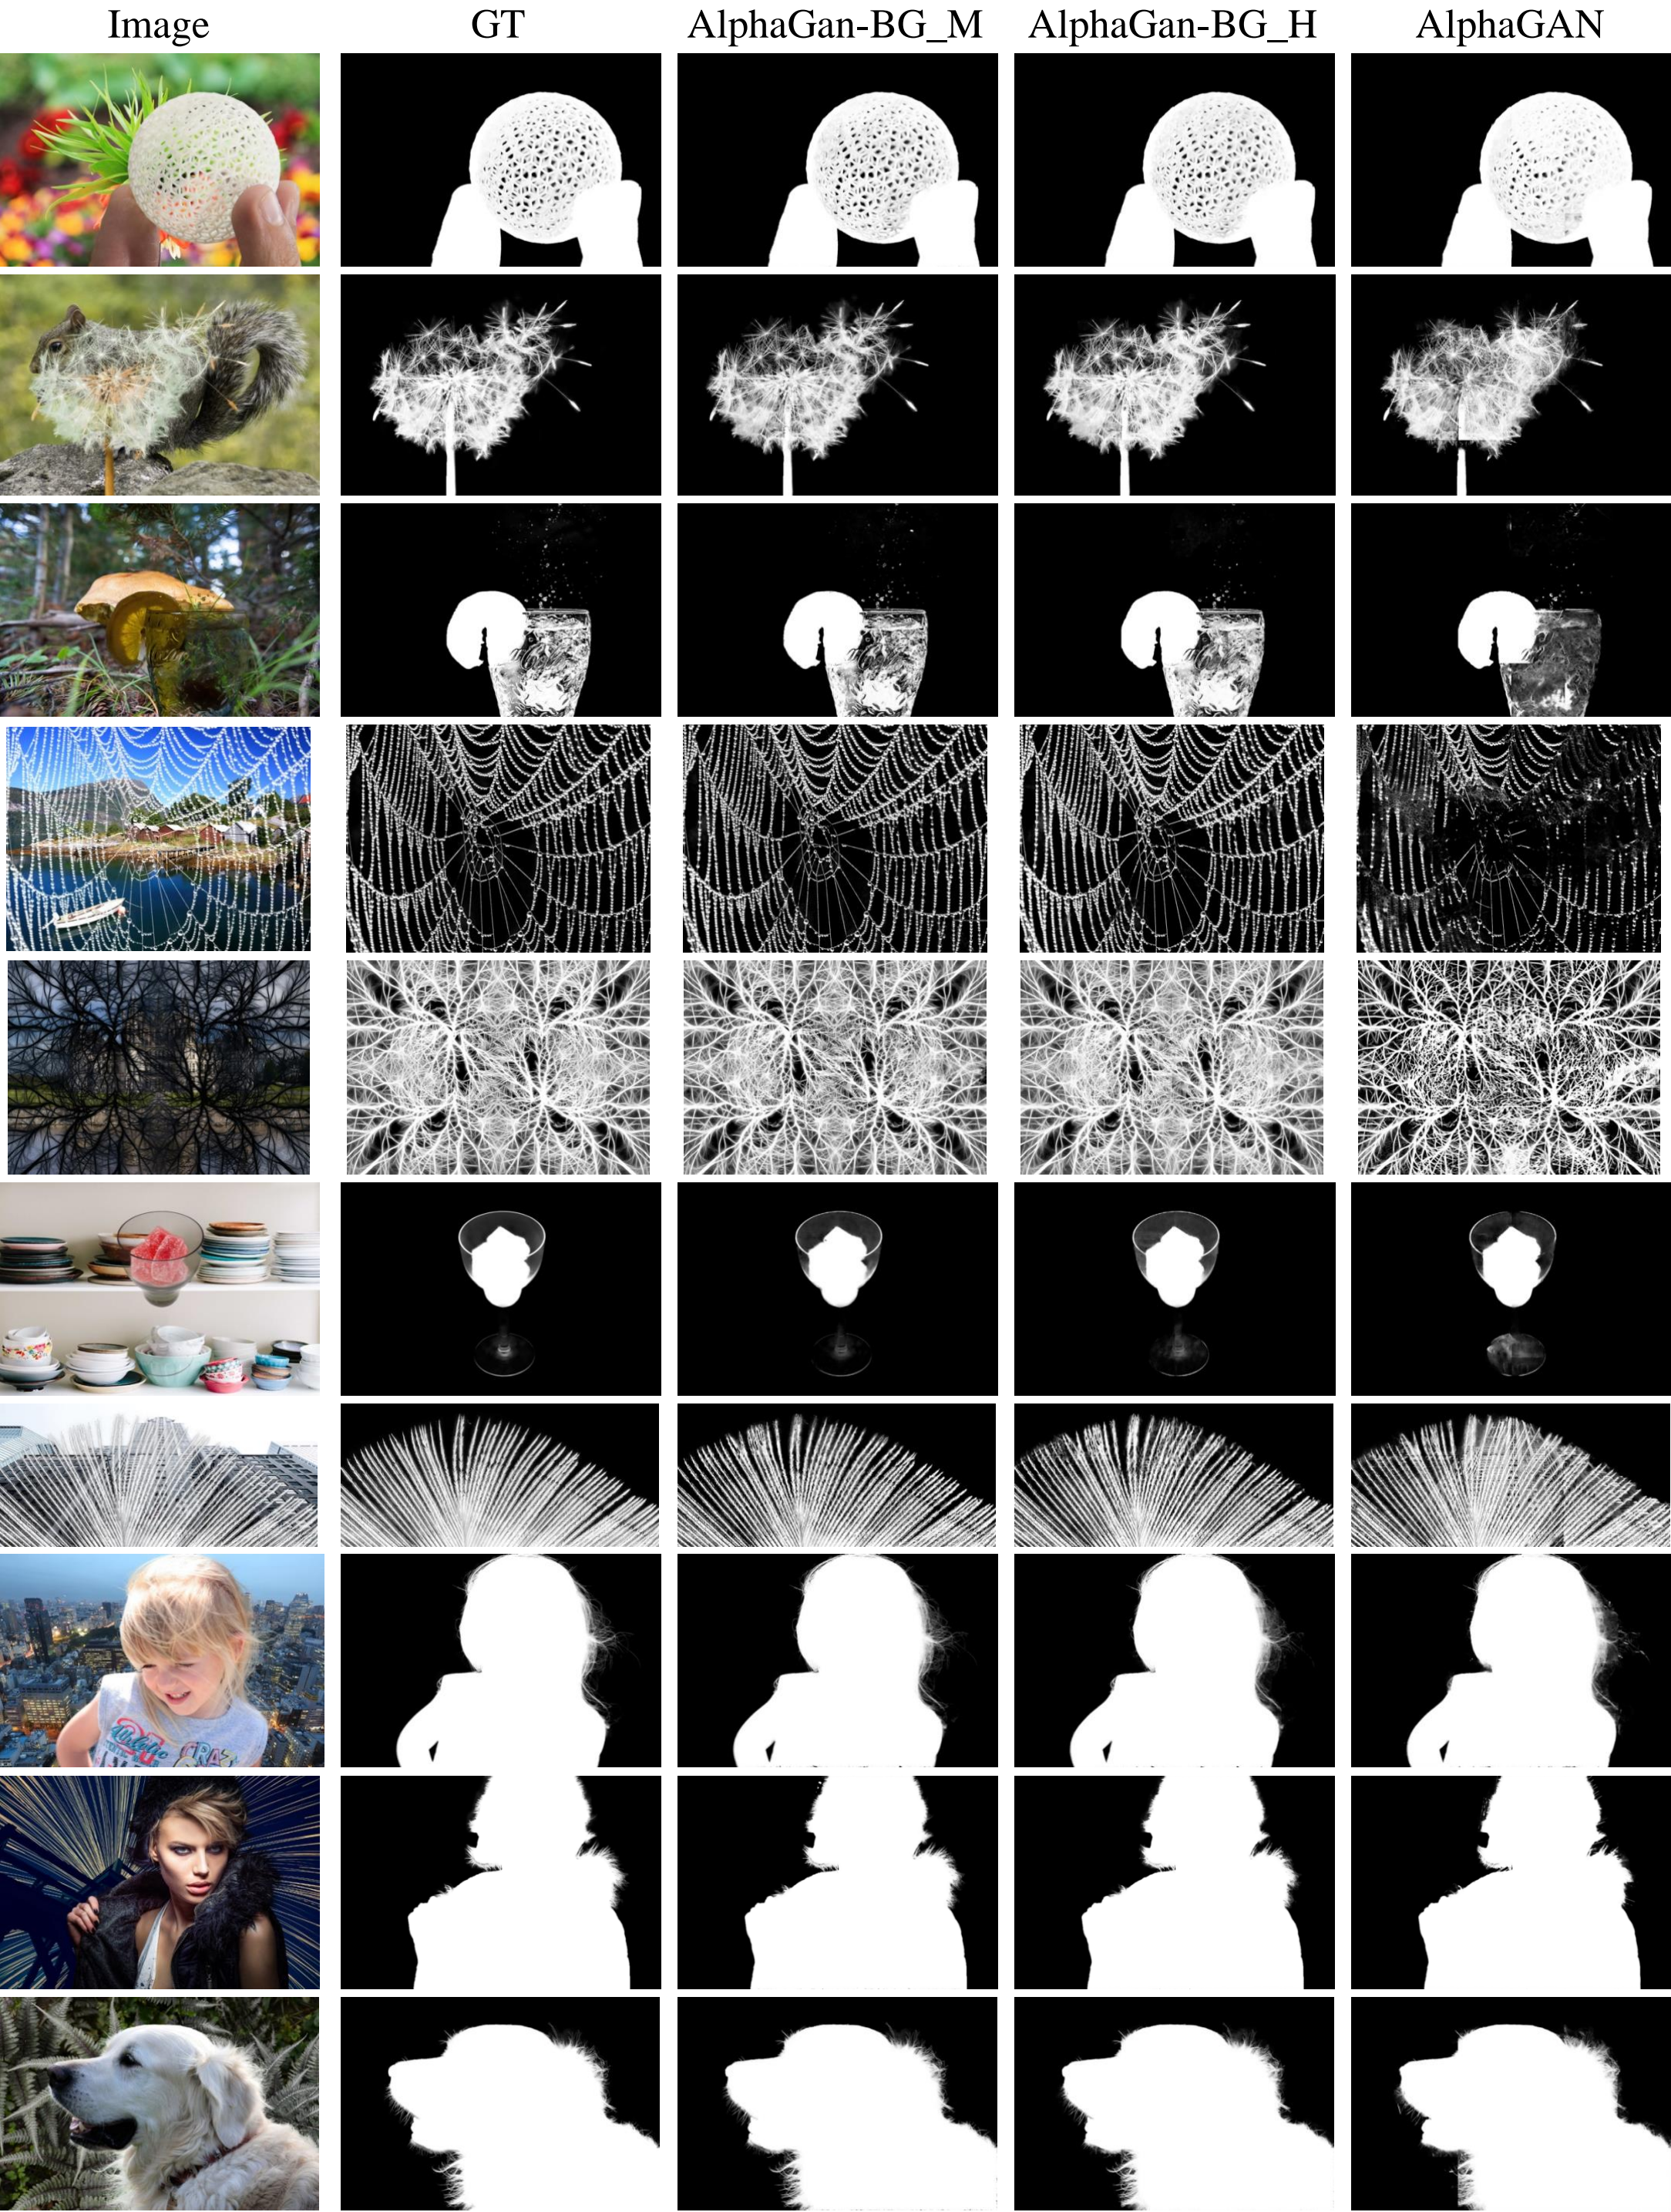 | 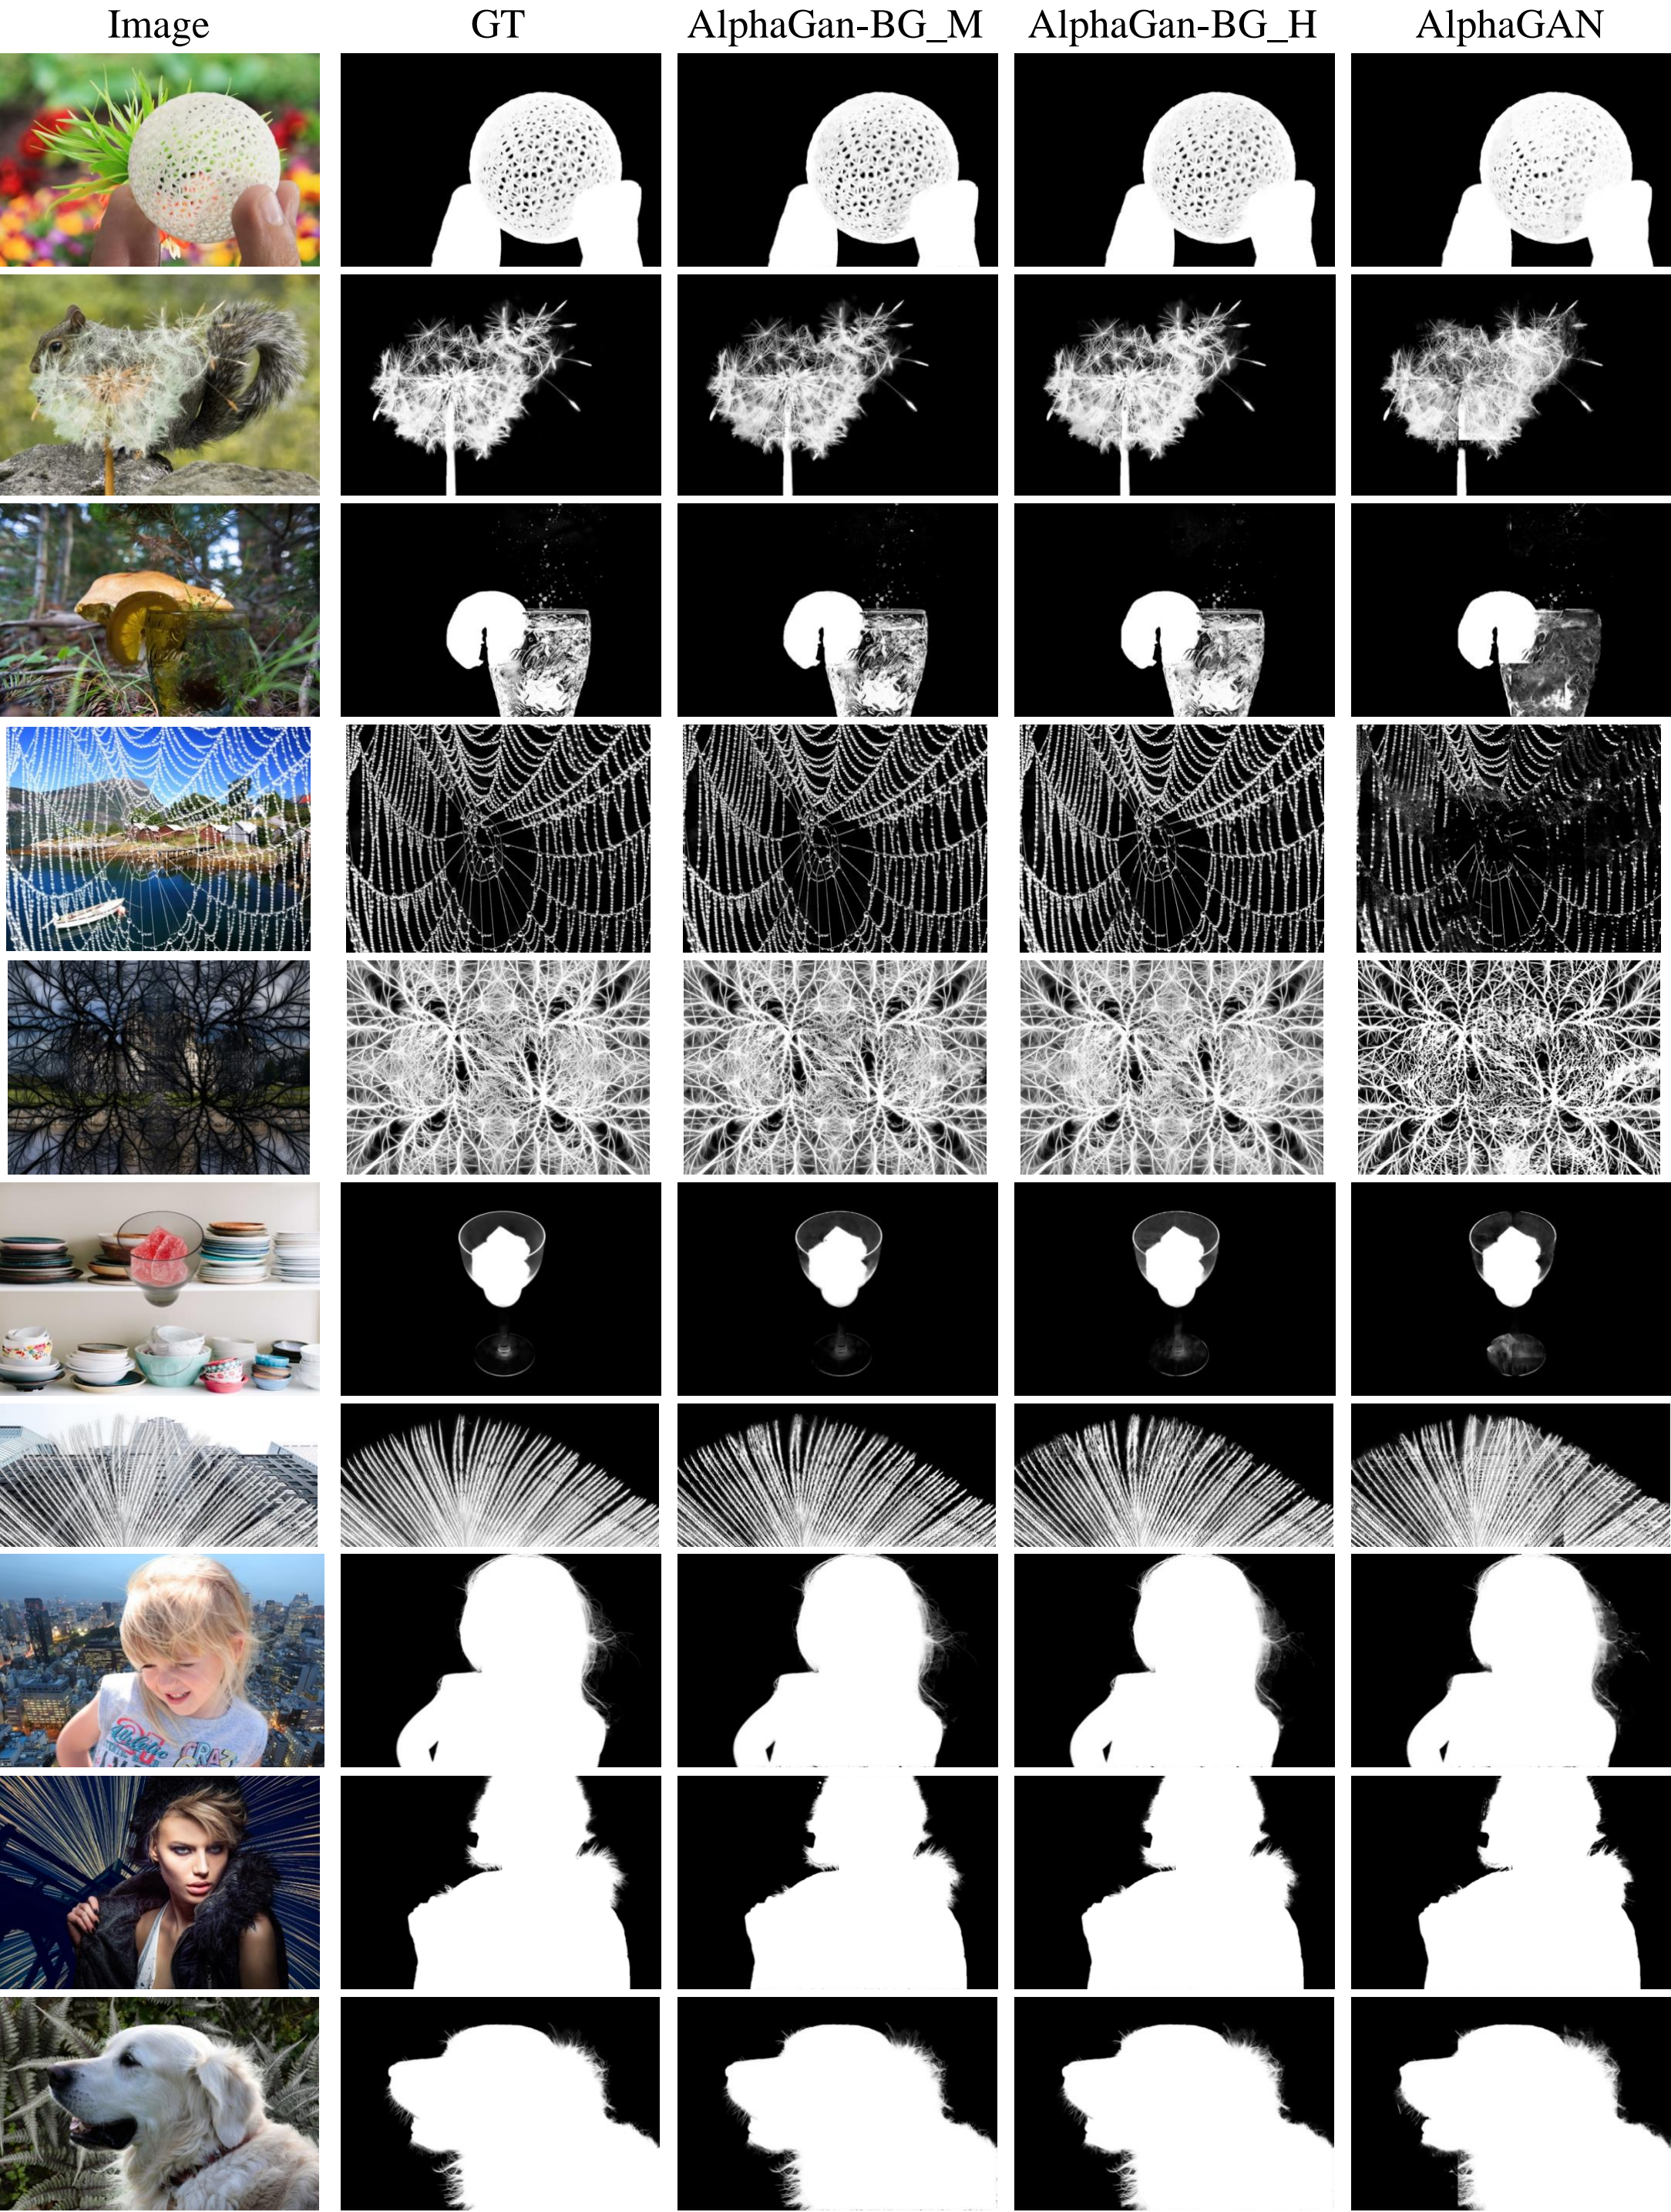 |
| 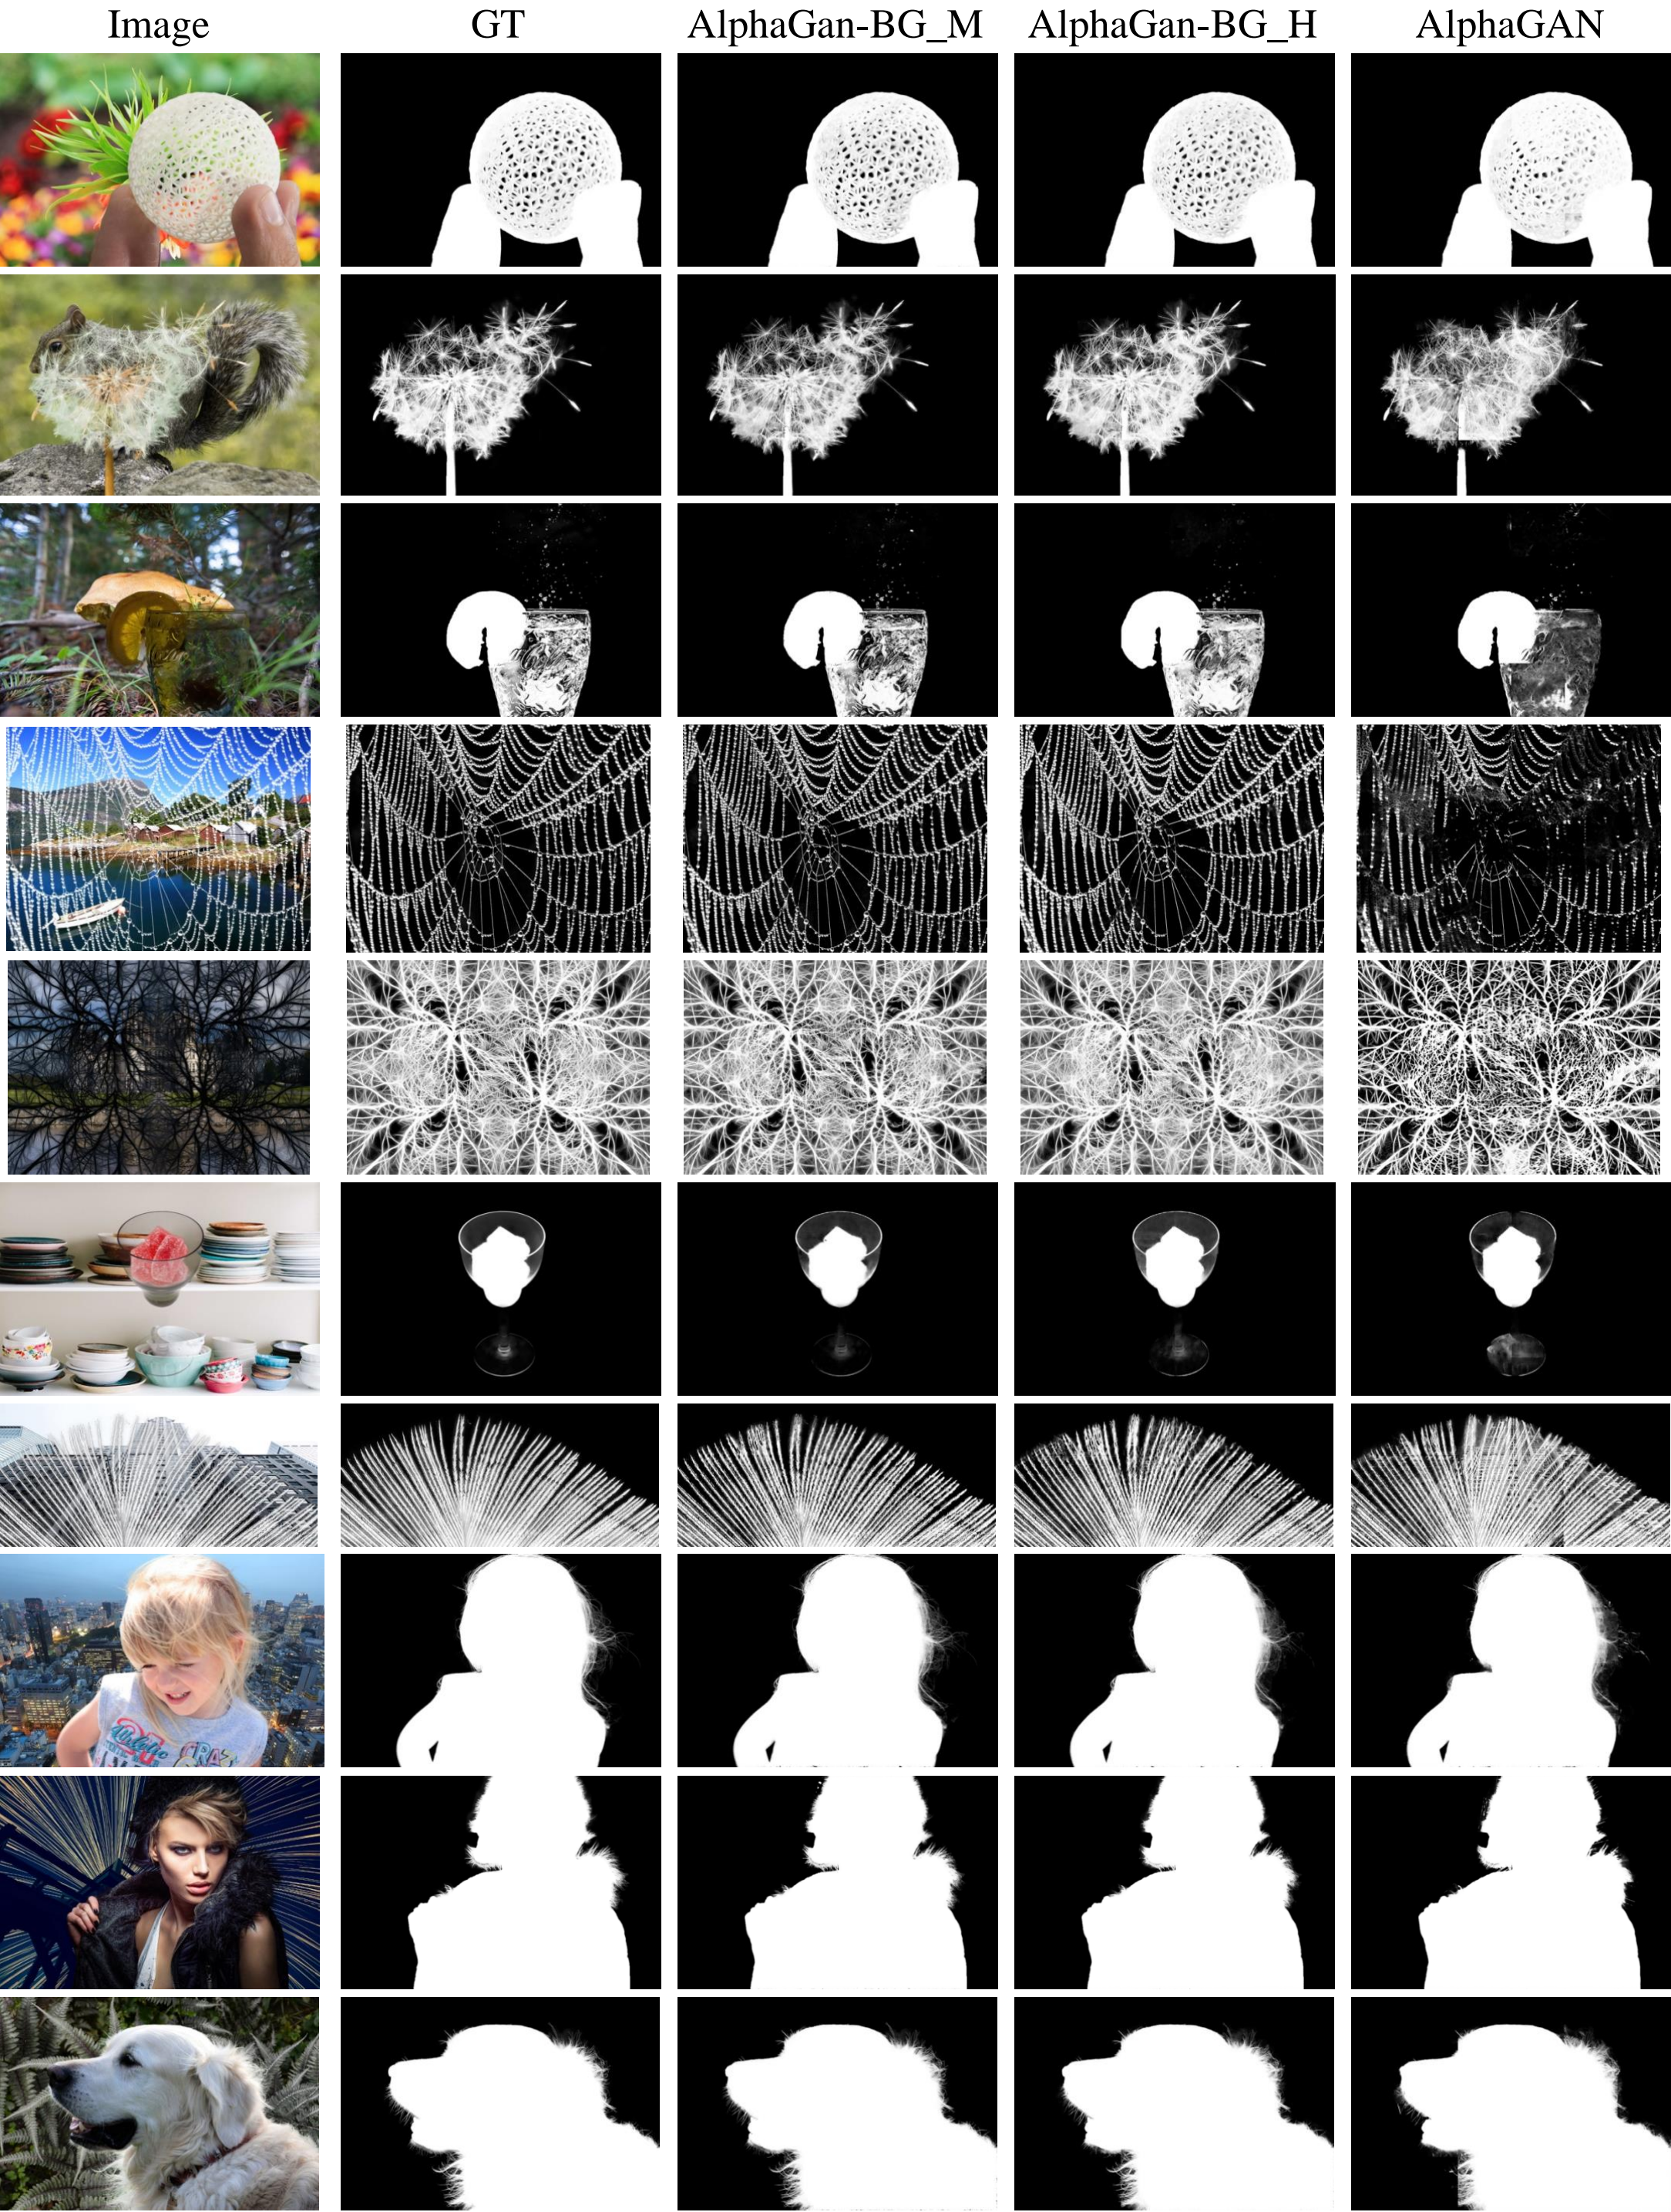 | 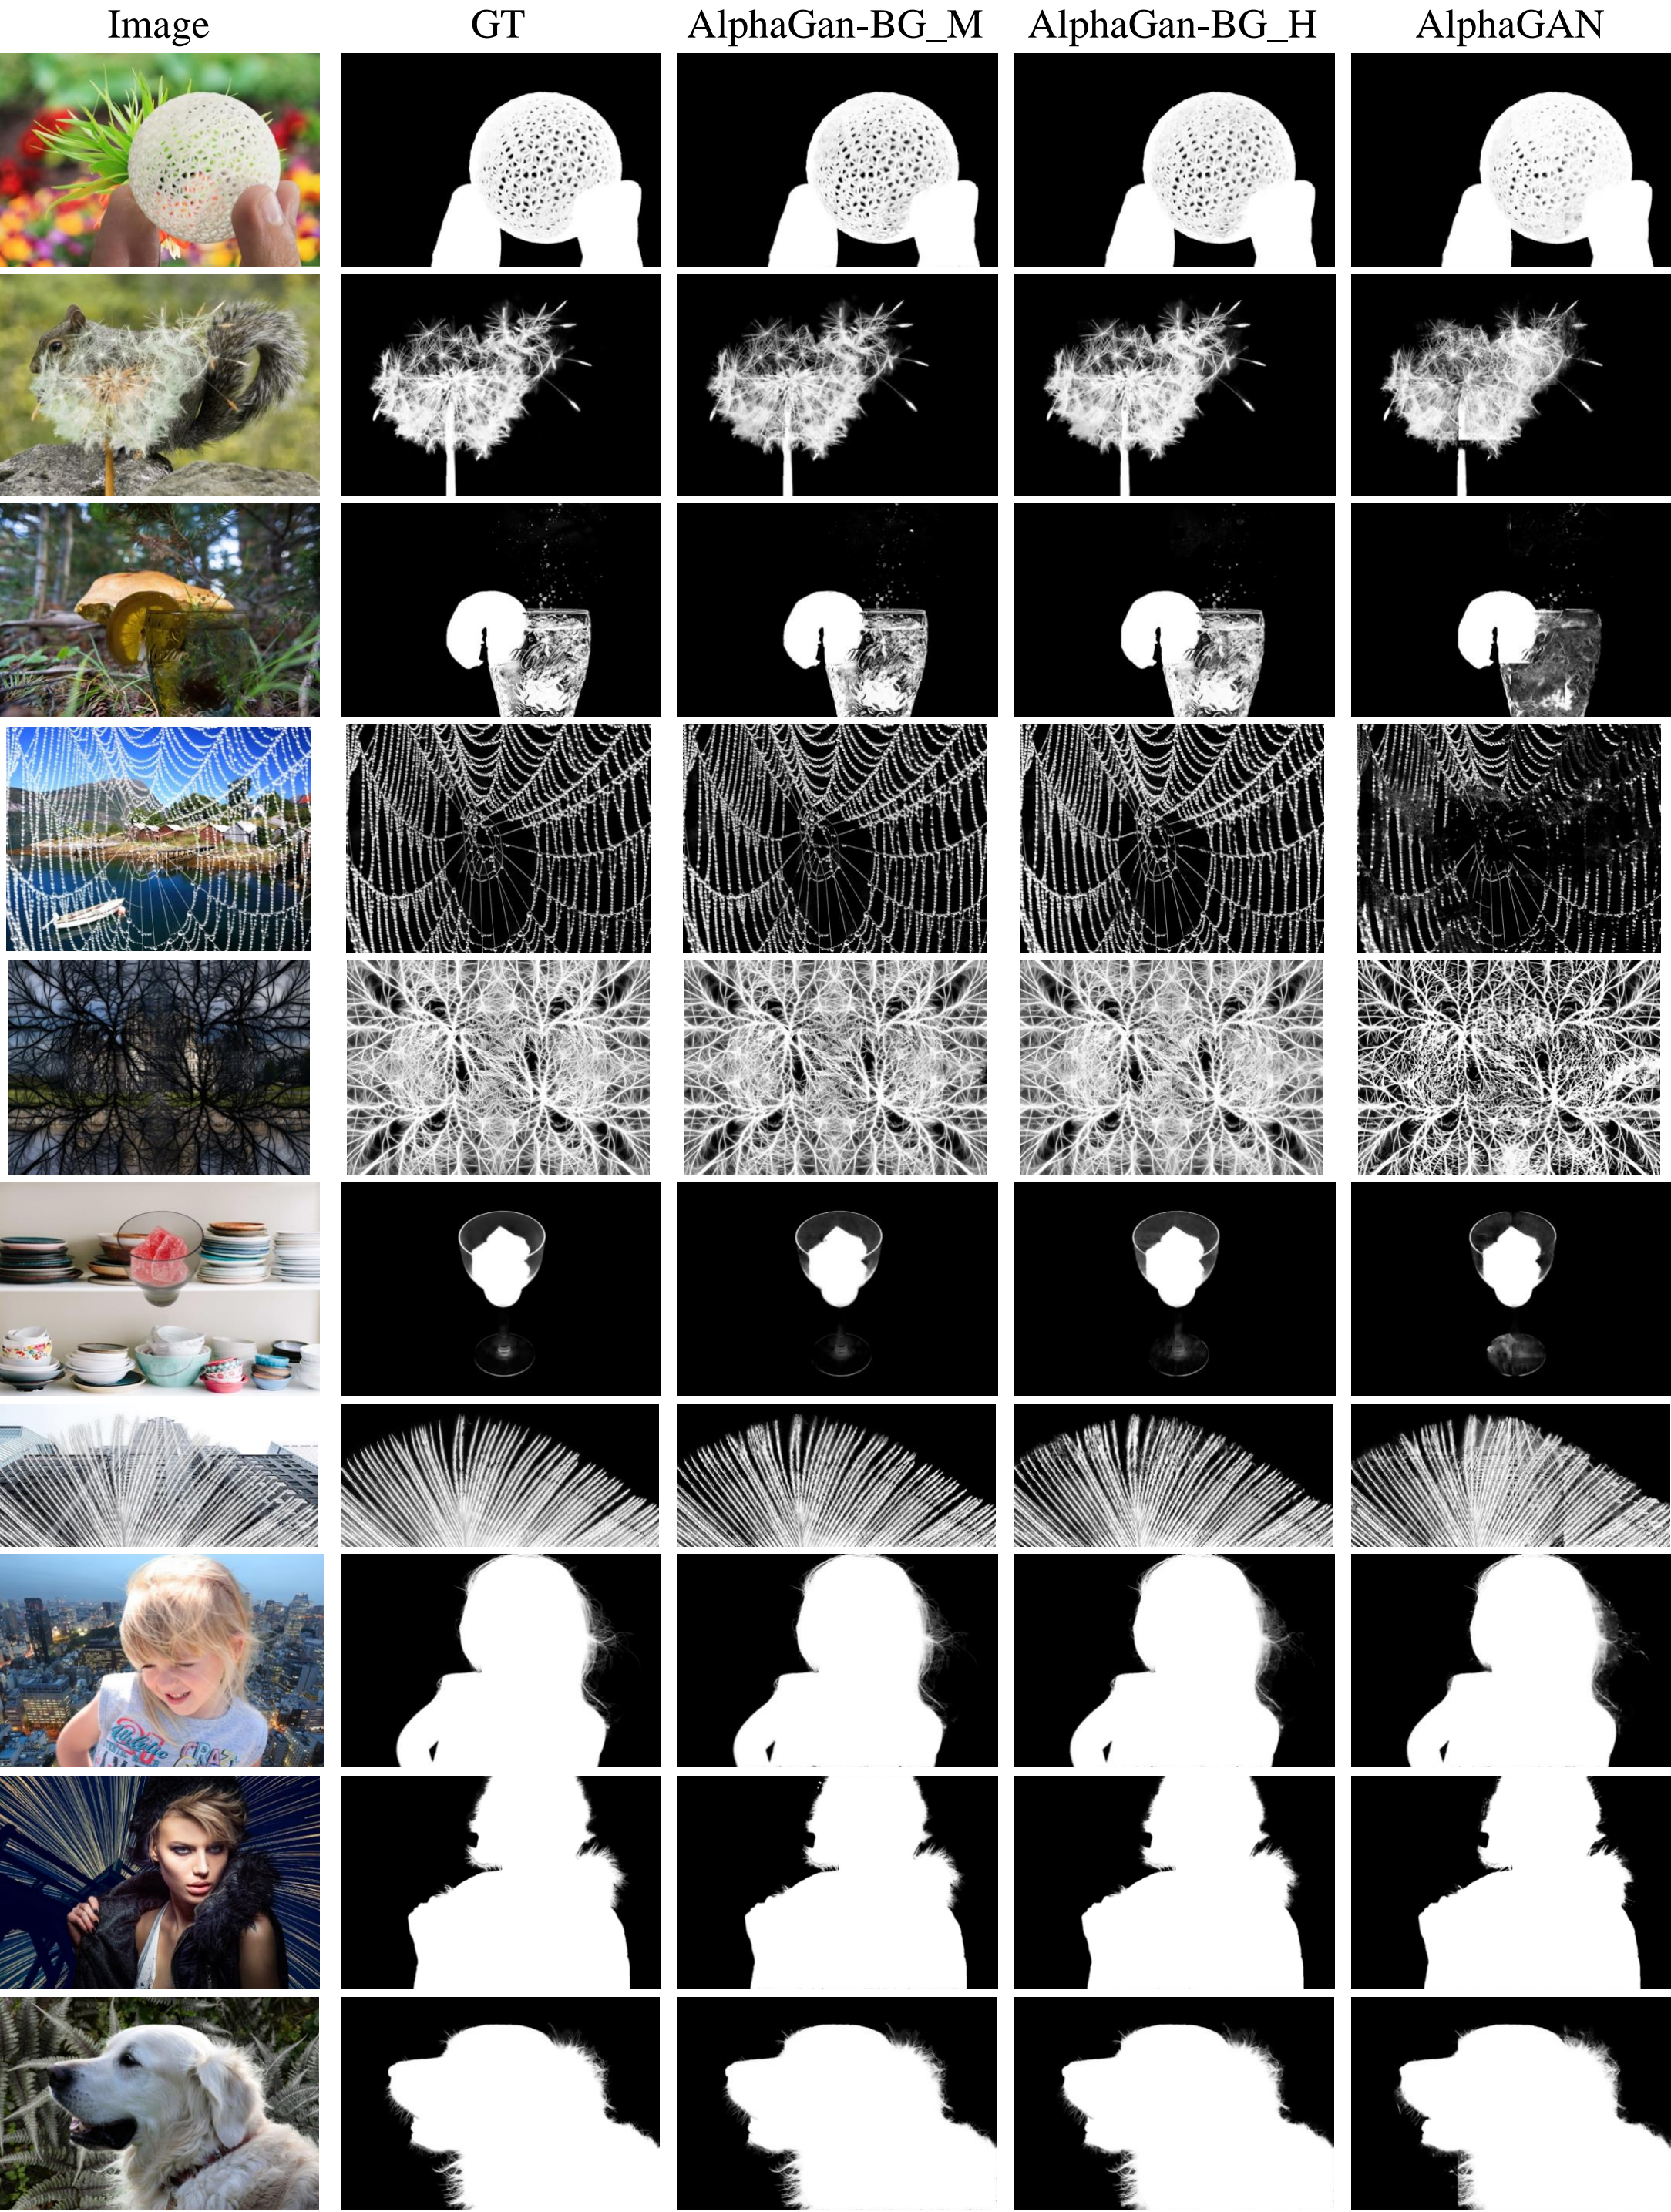 | 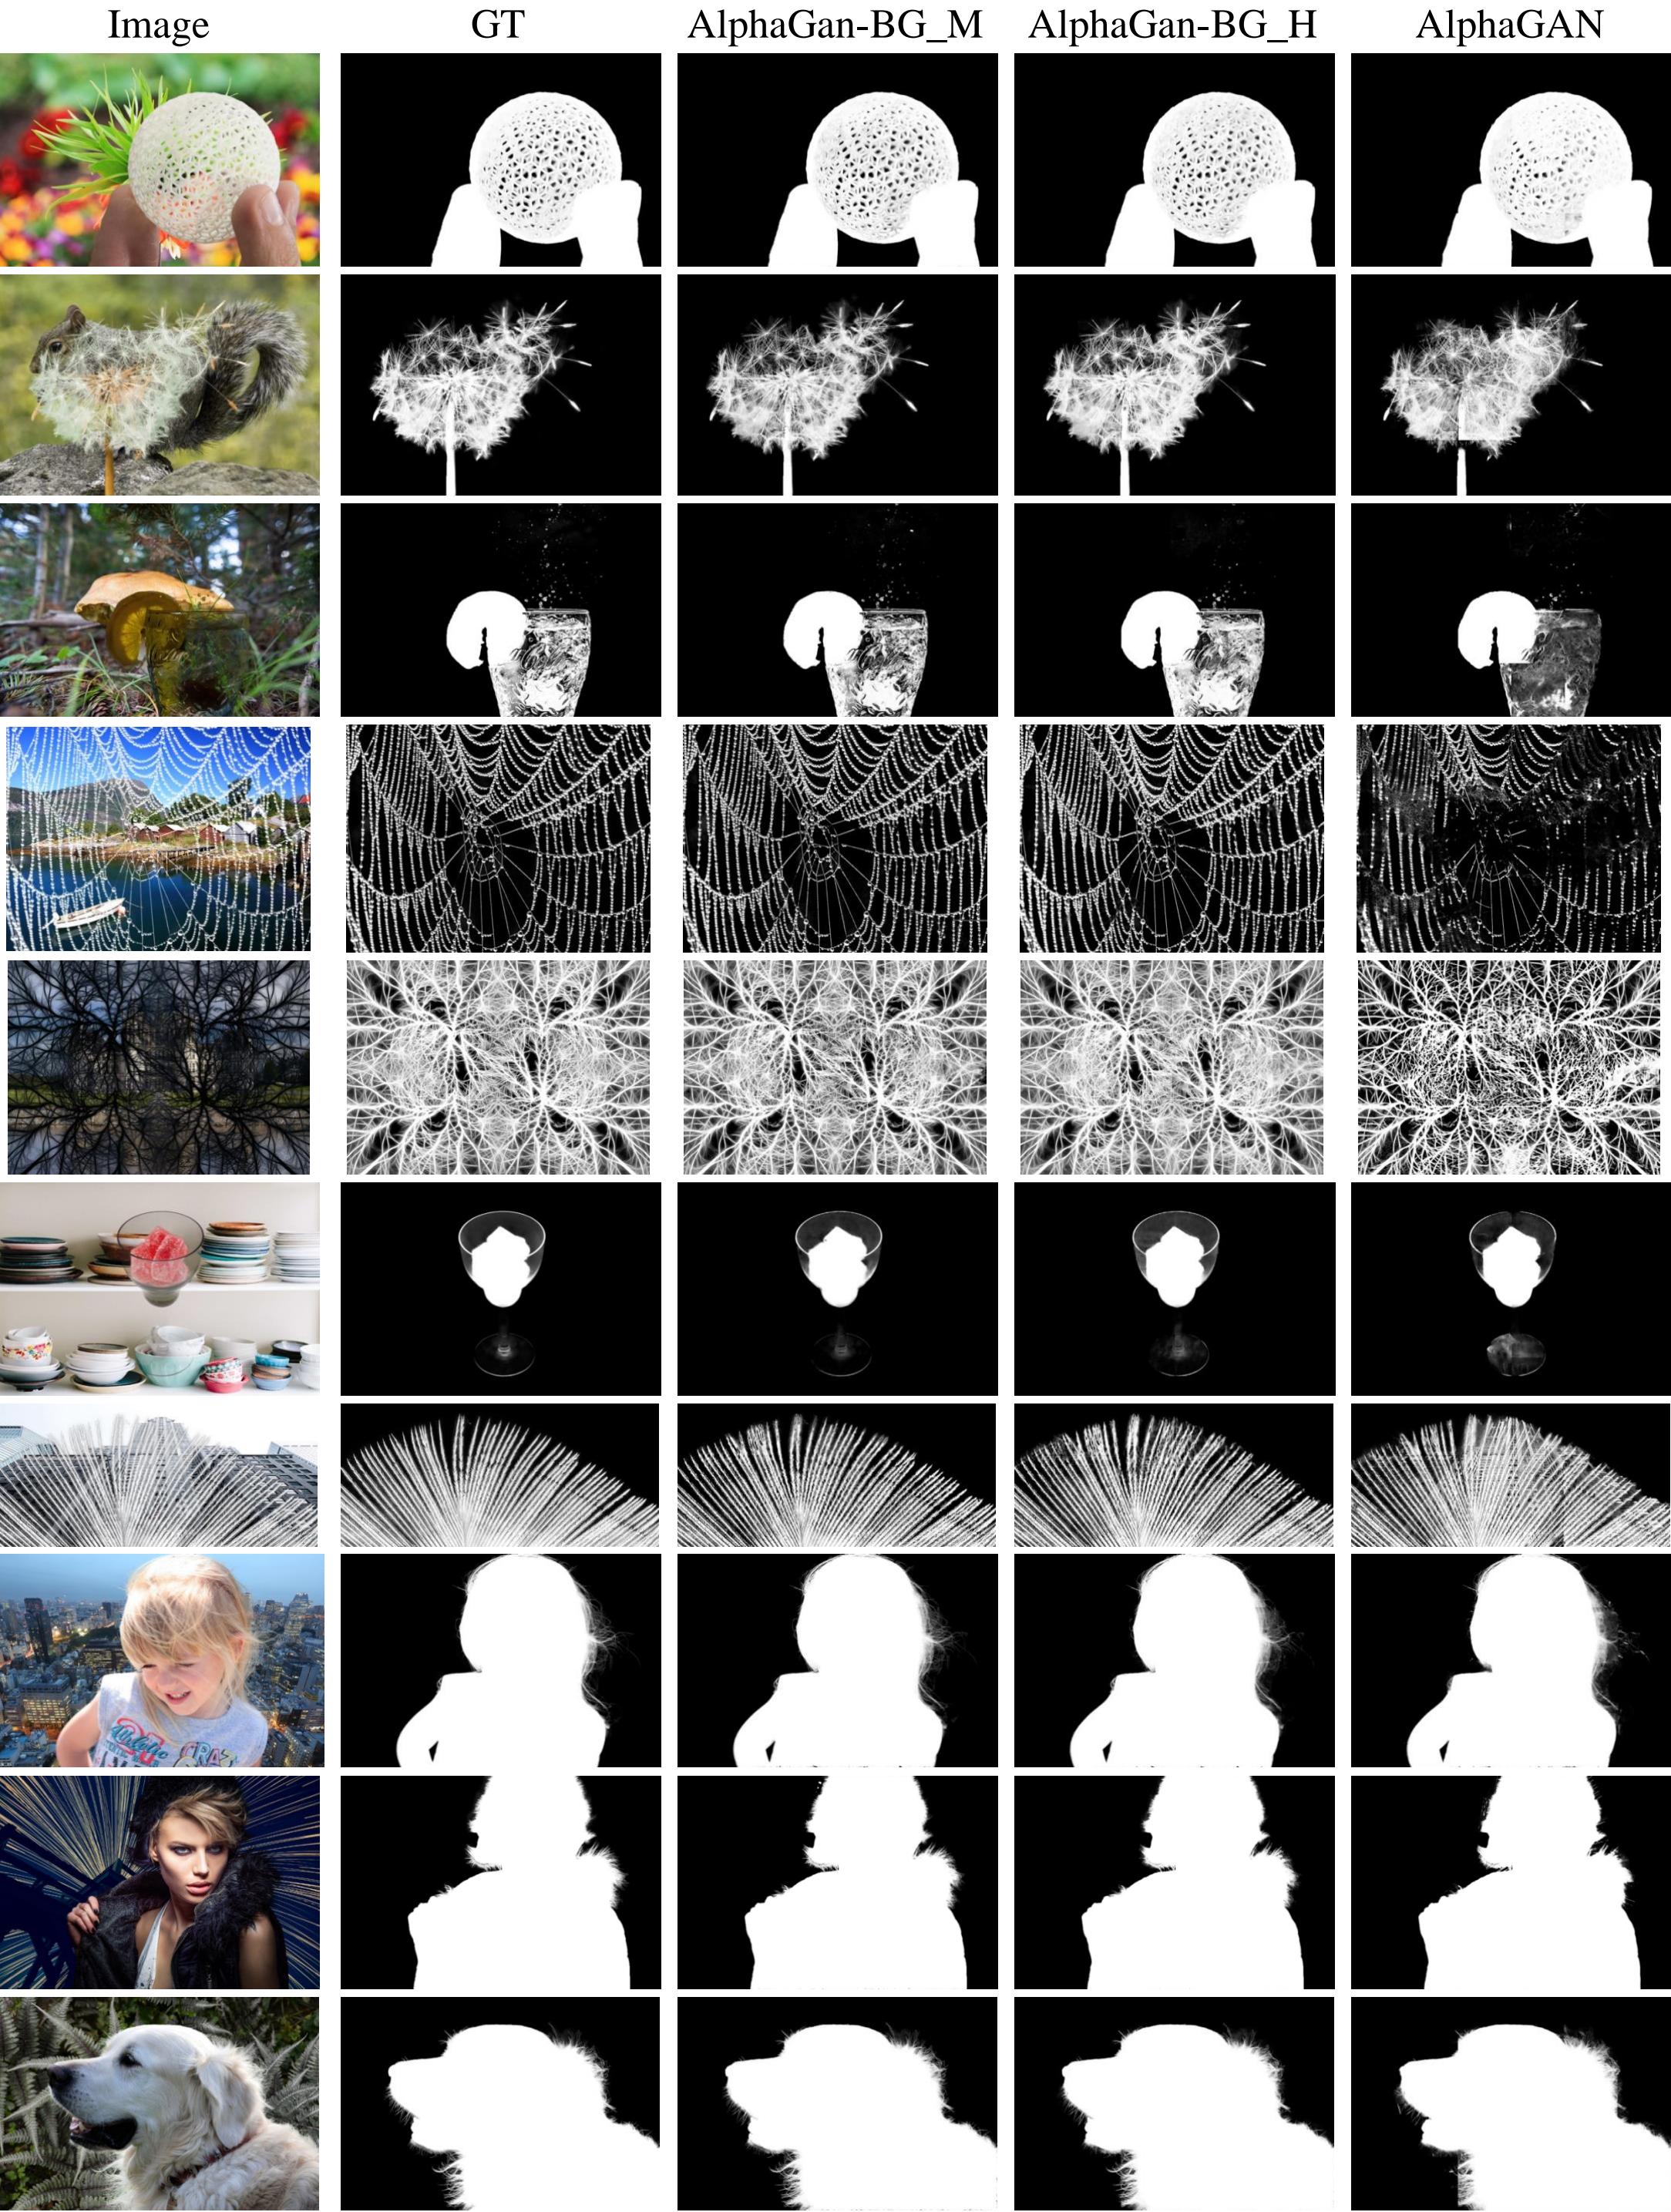 | 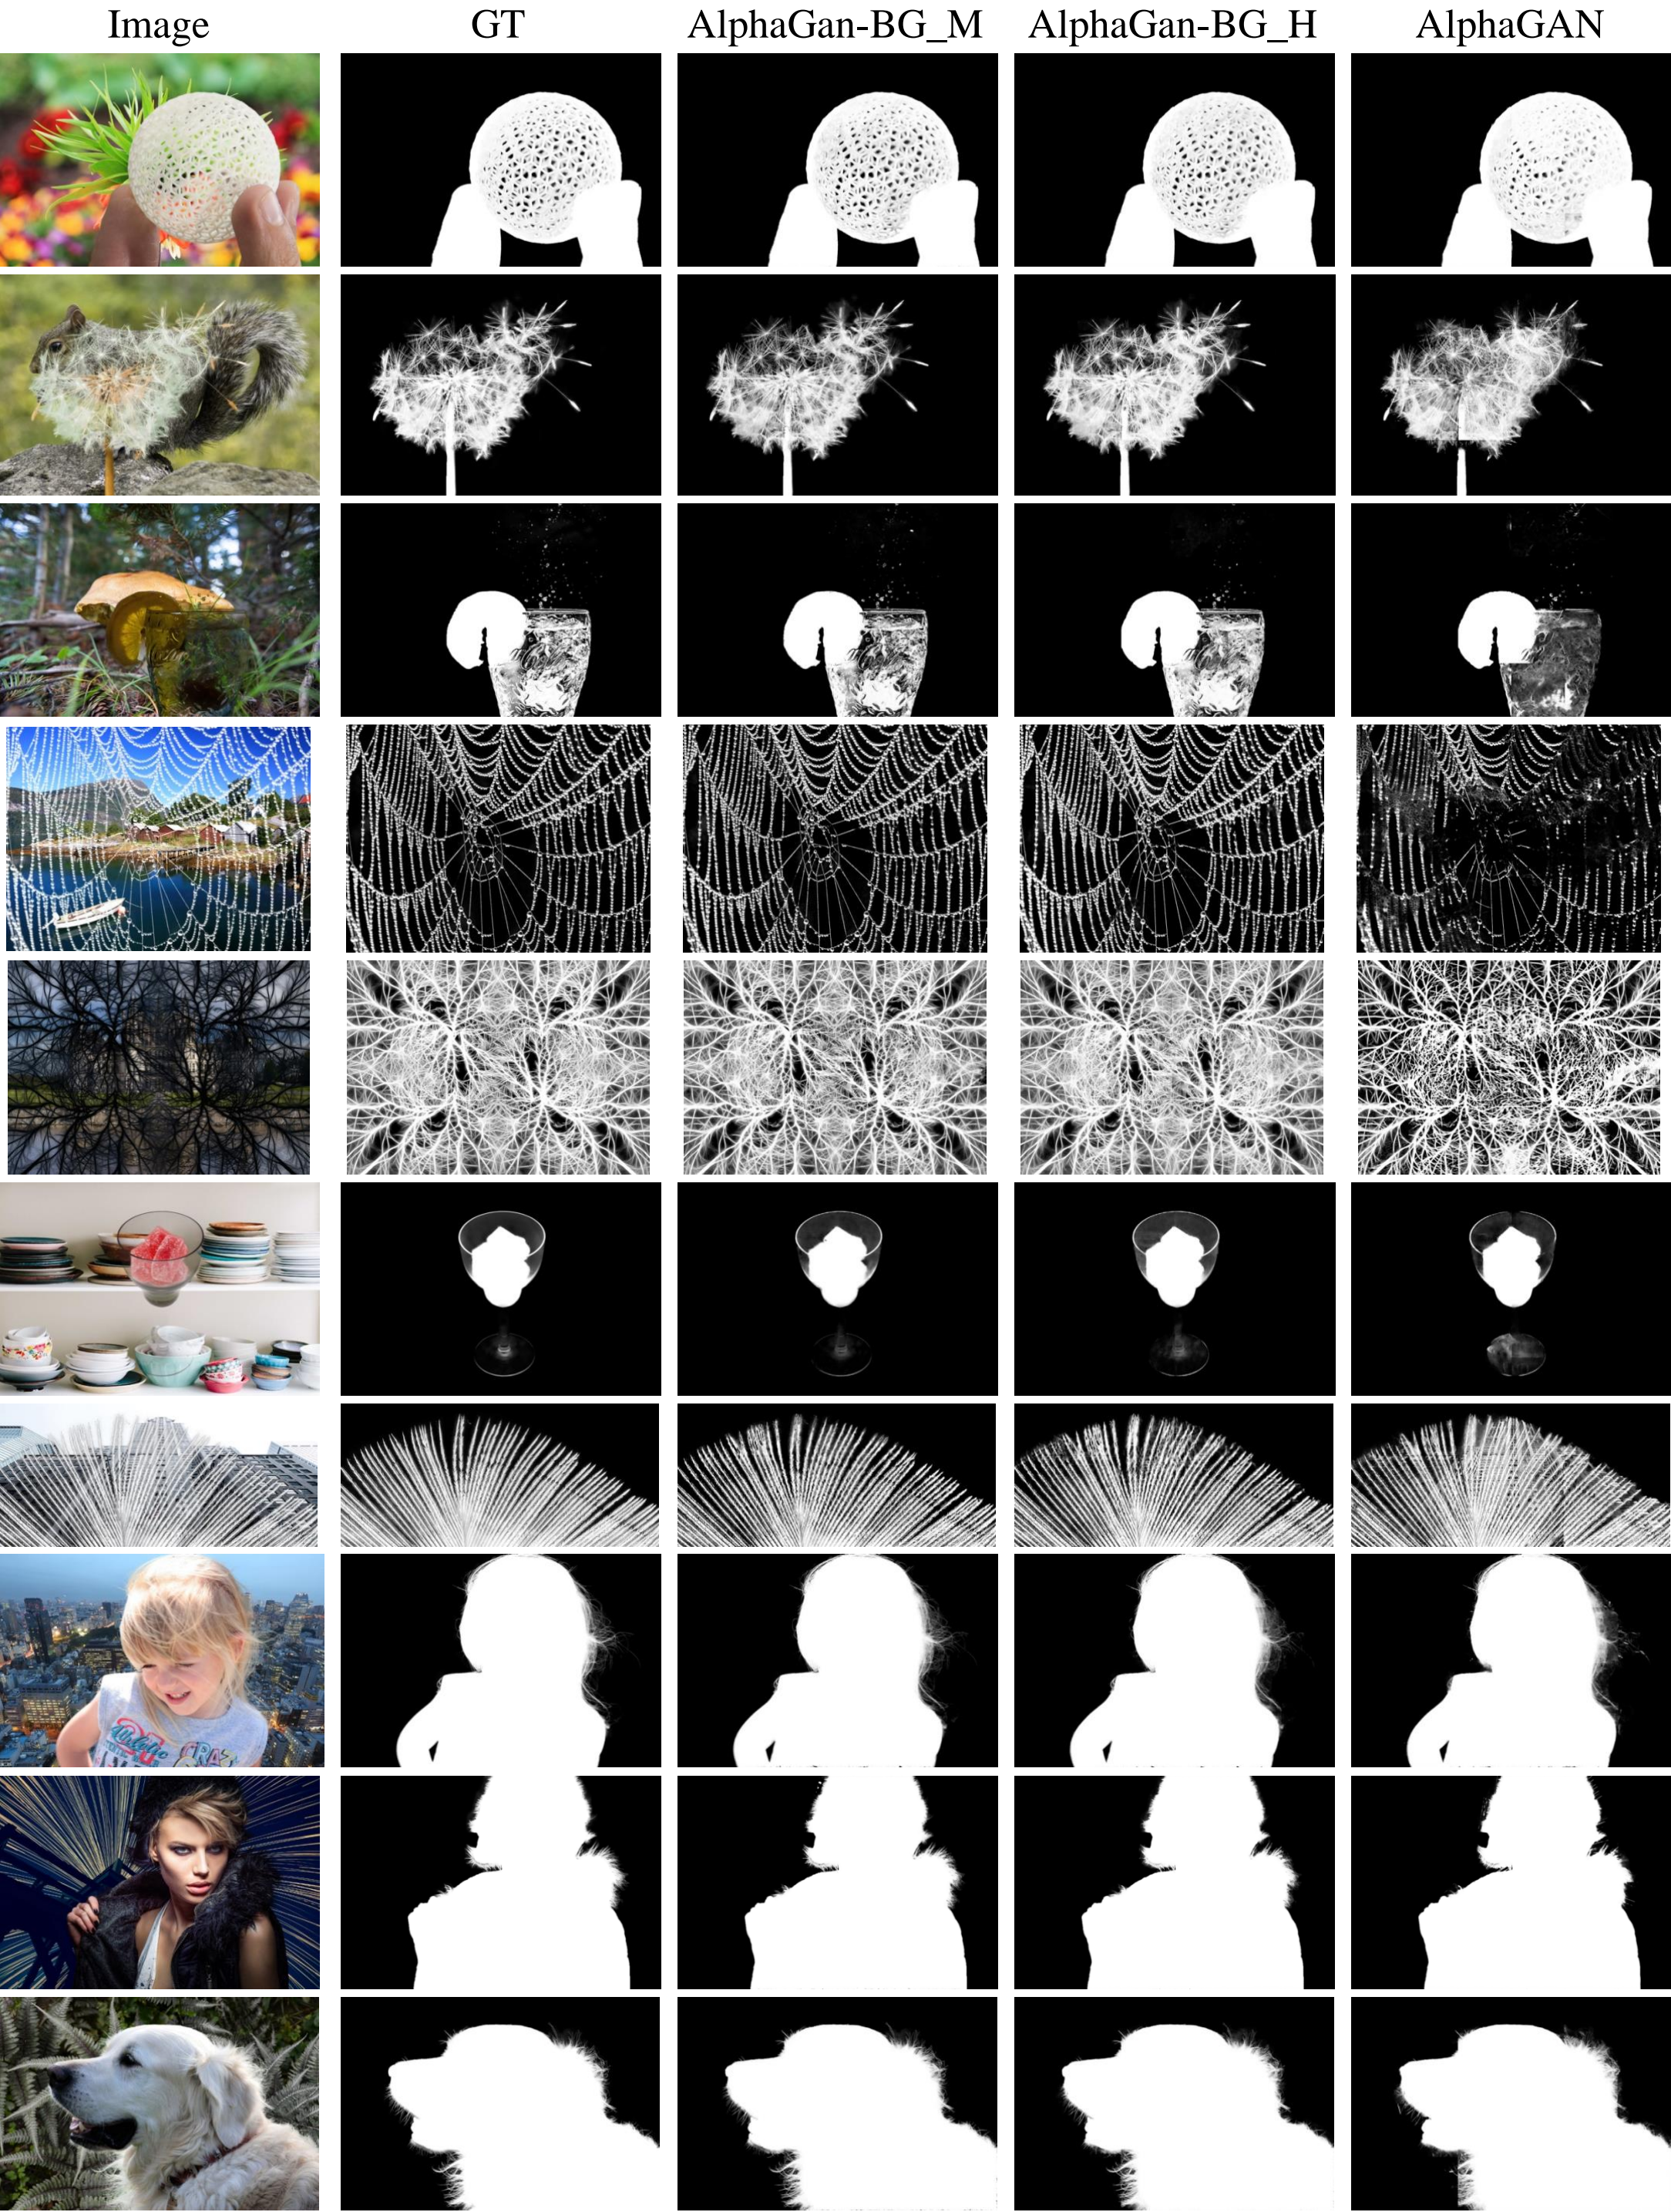 | 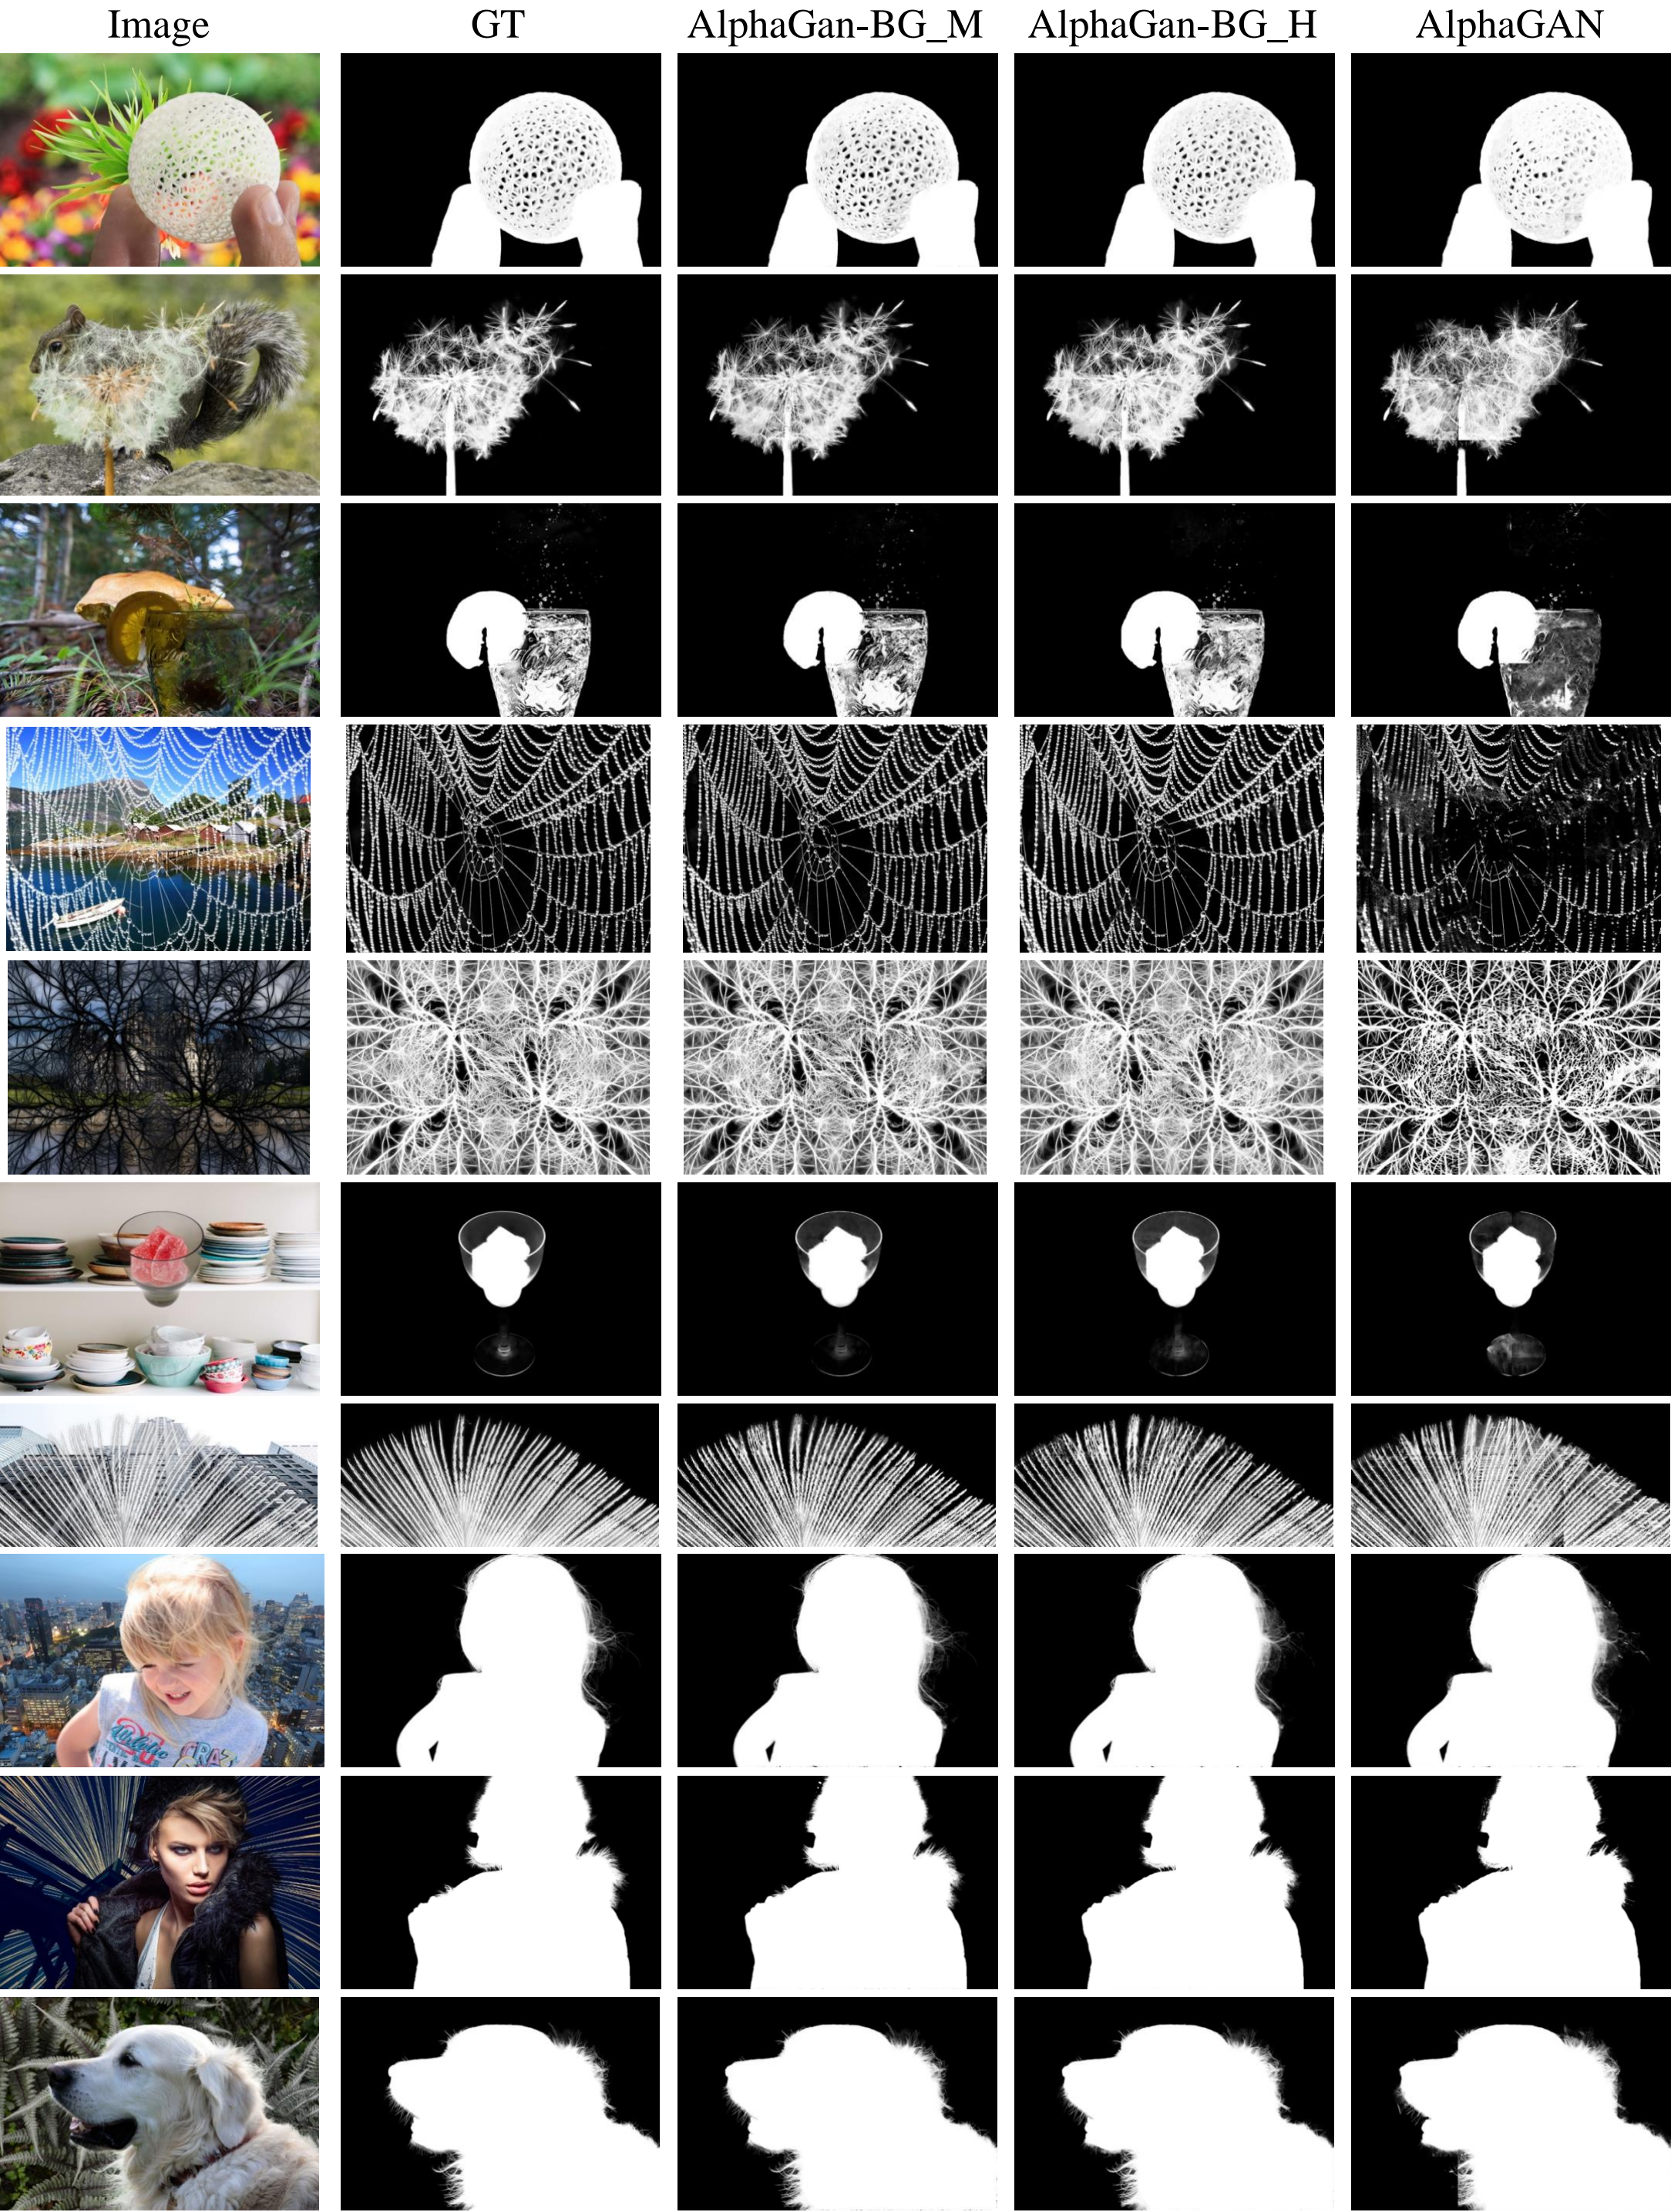 |
| 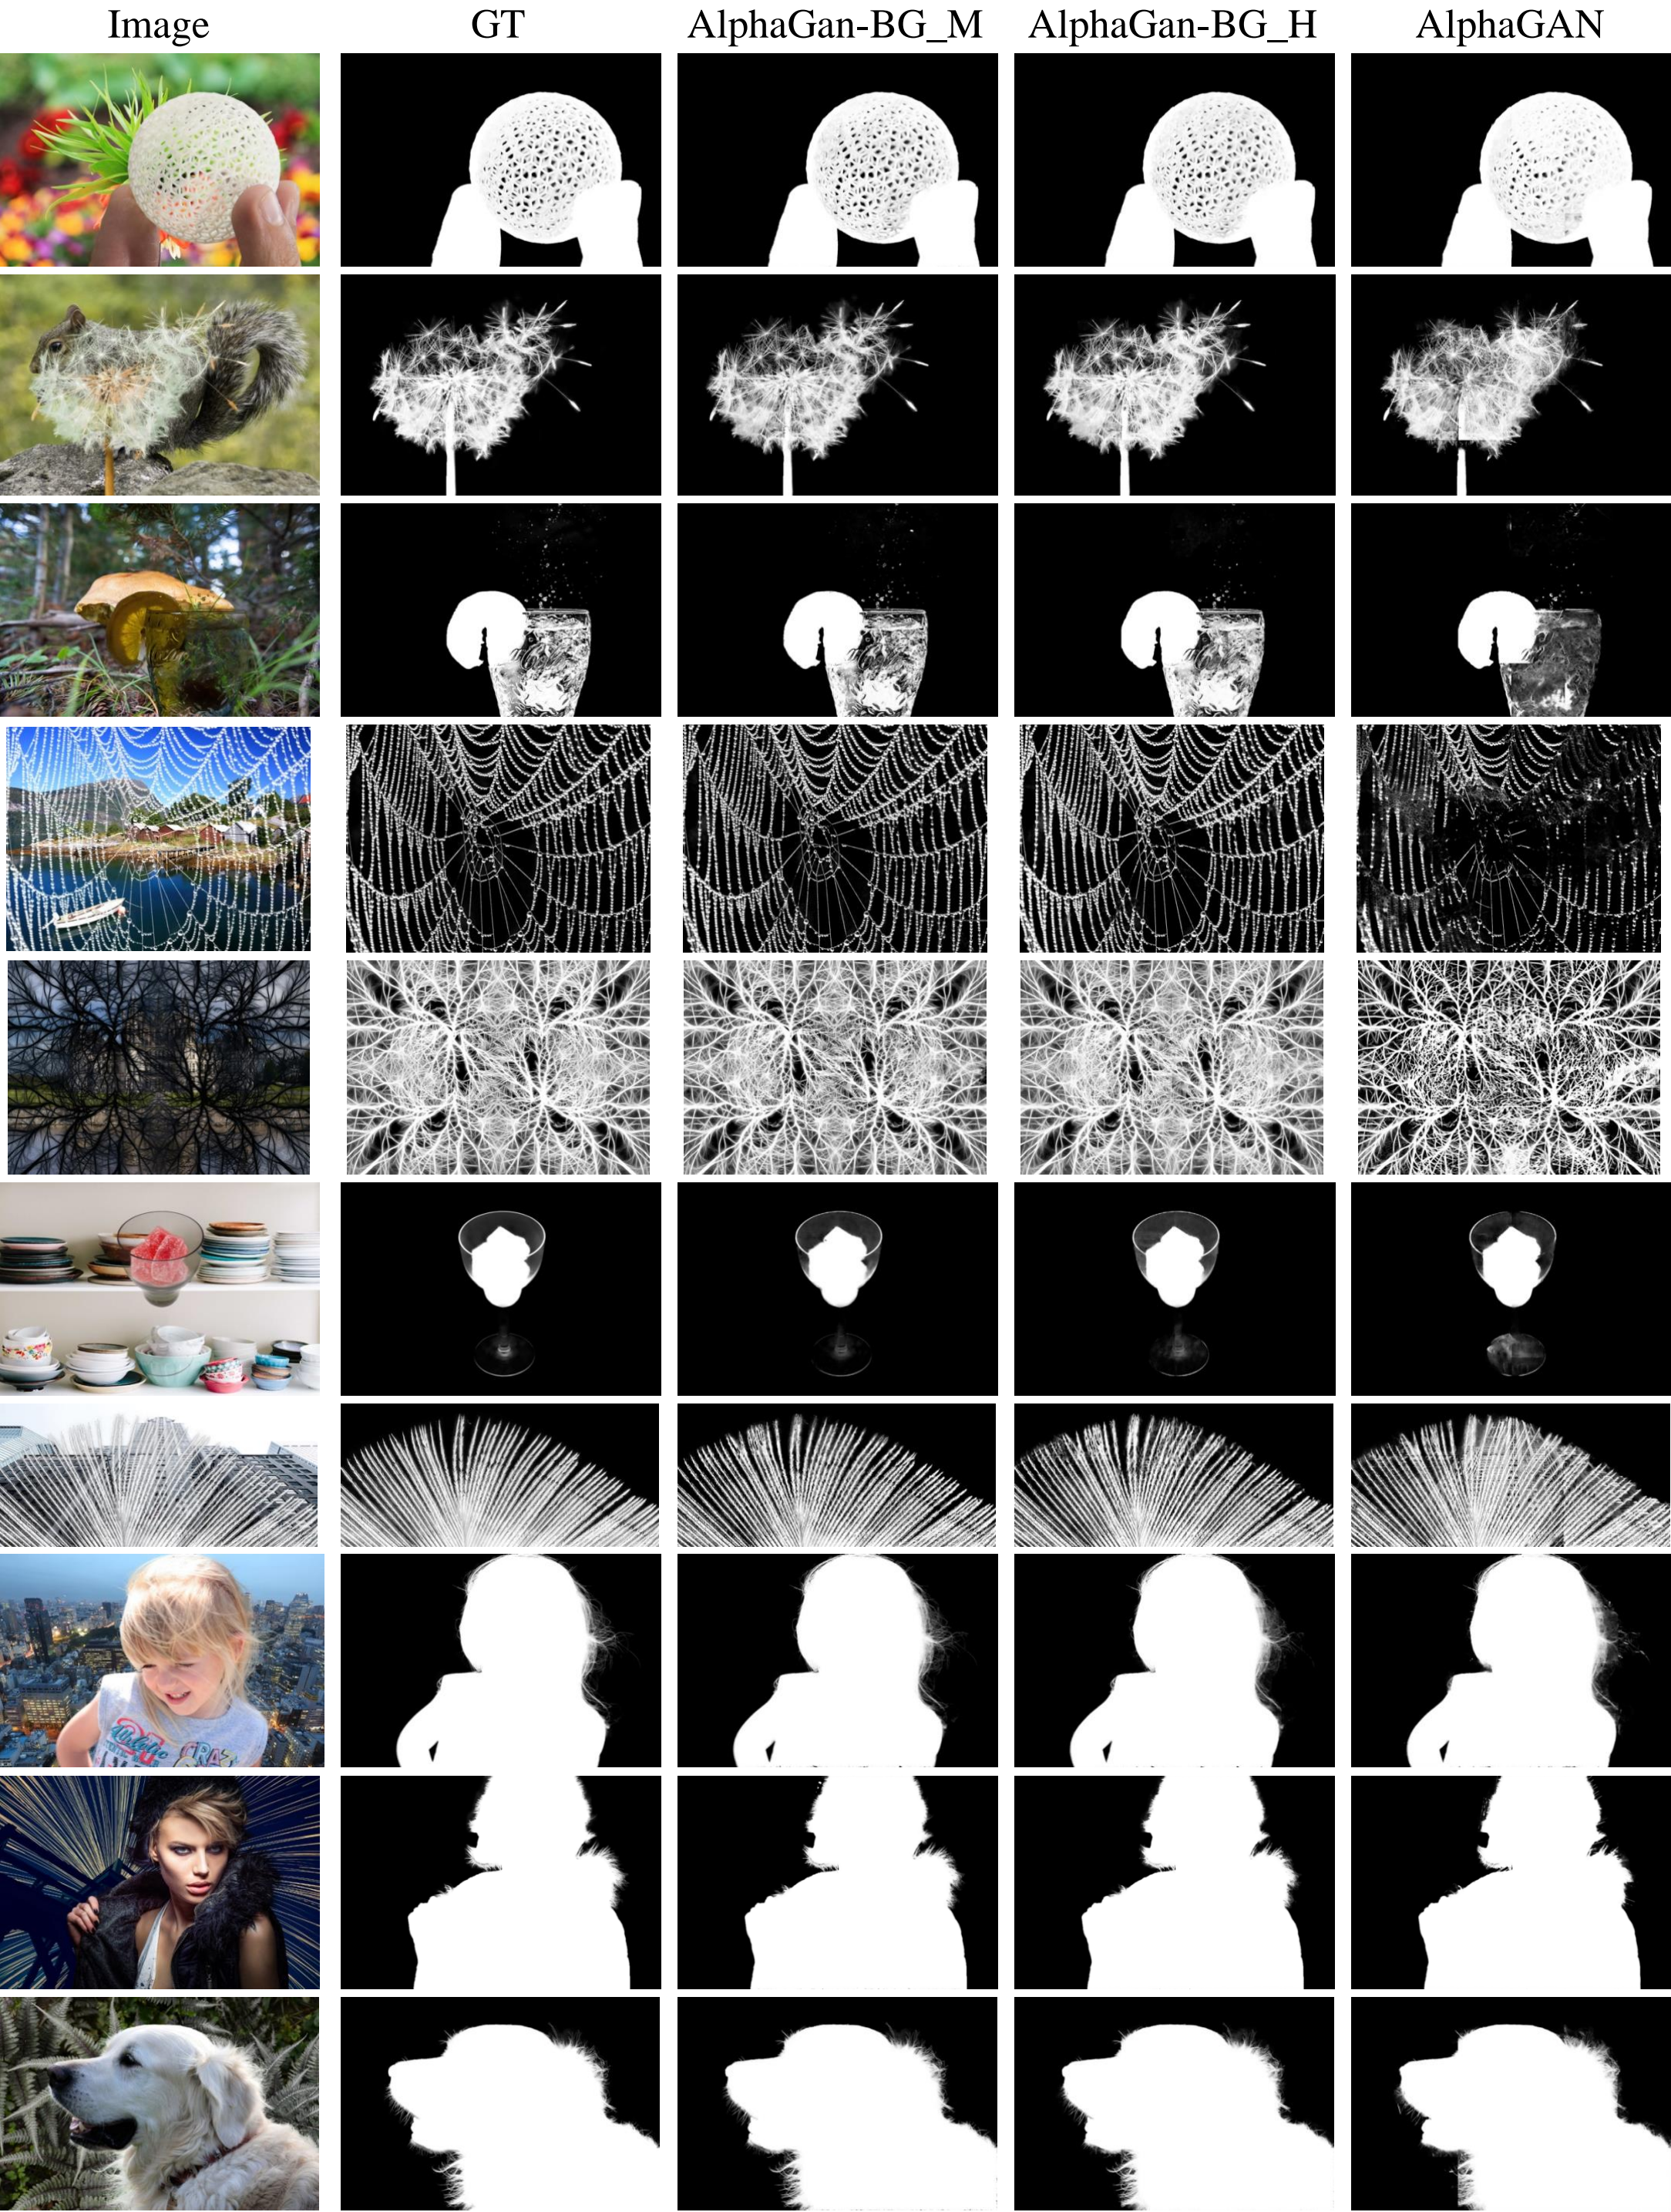 | 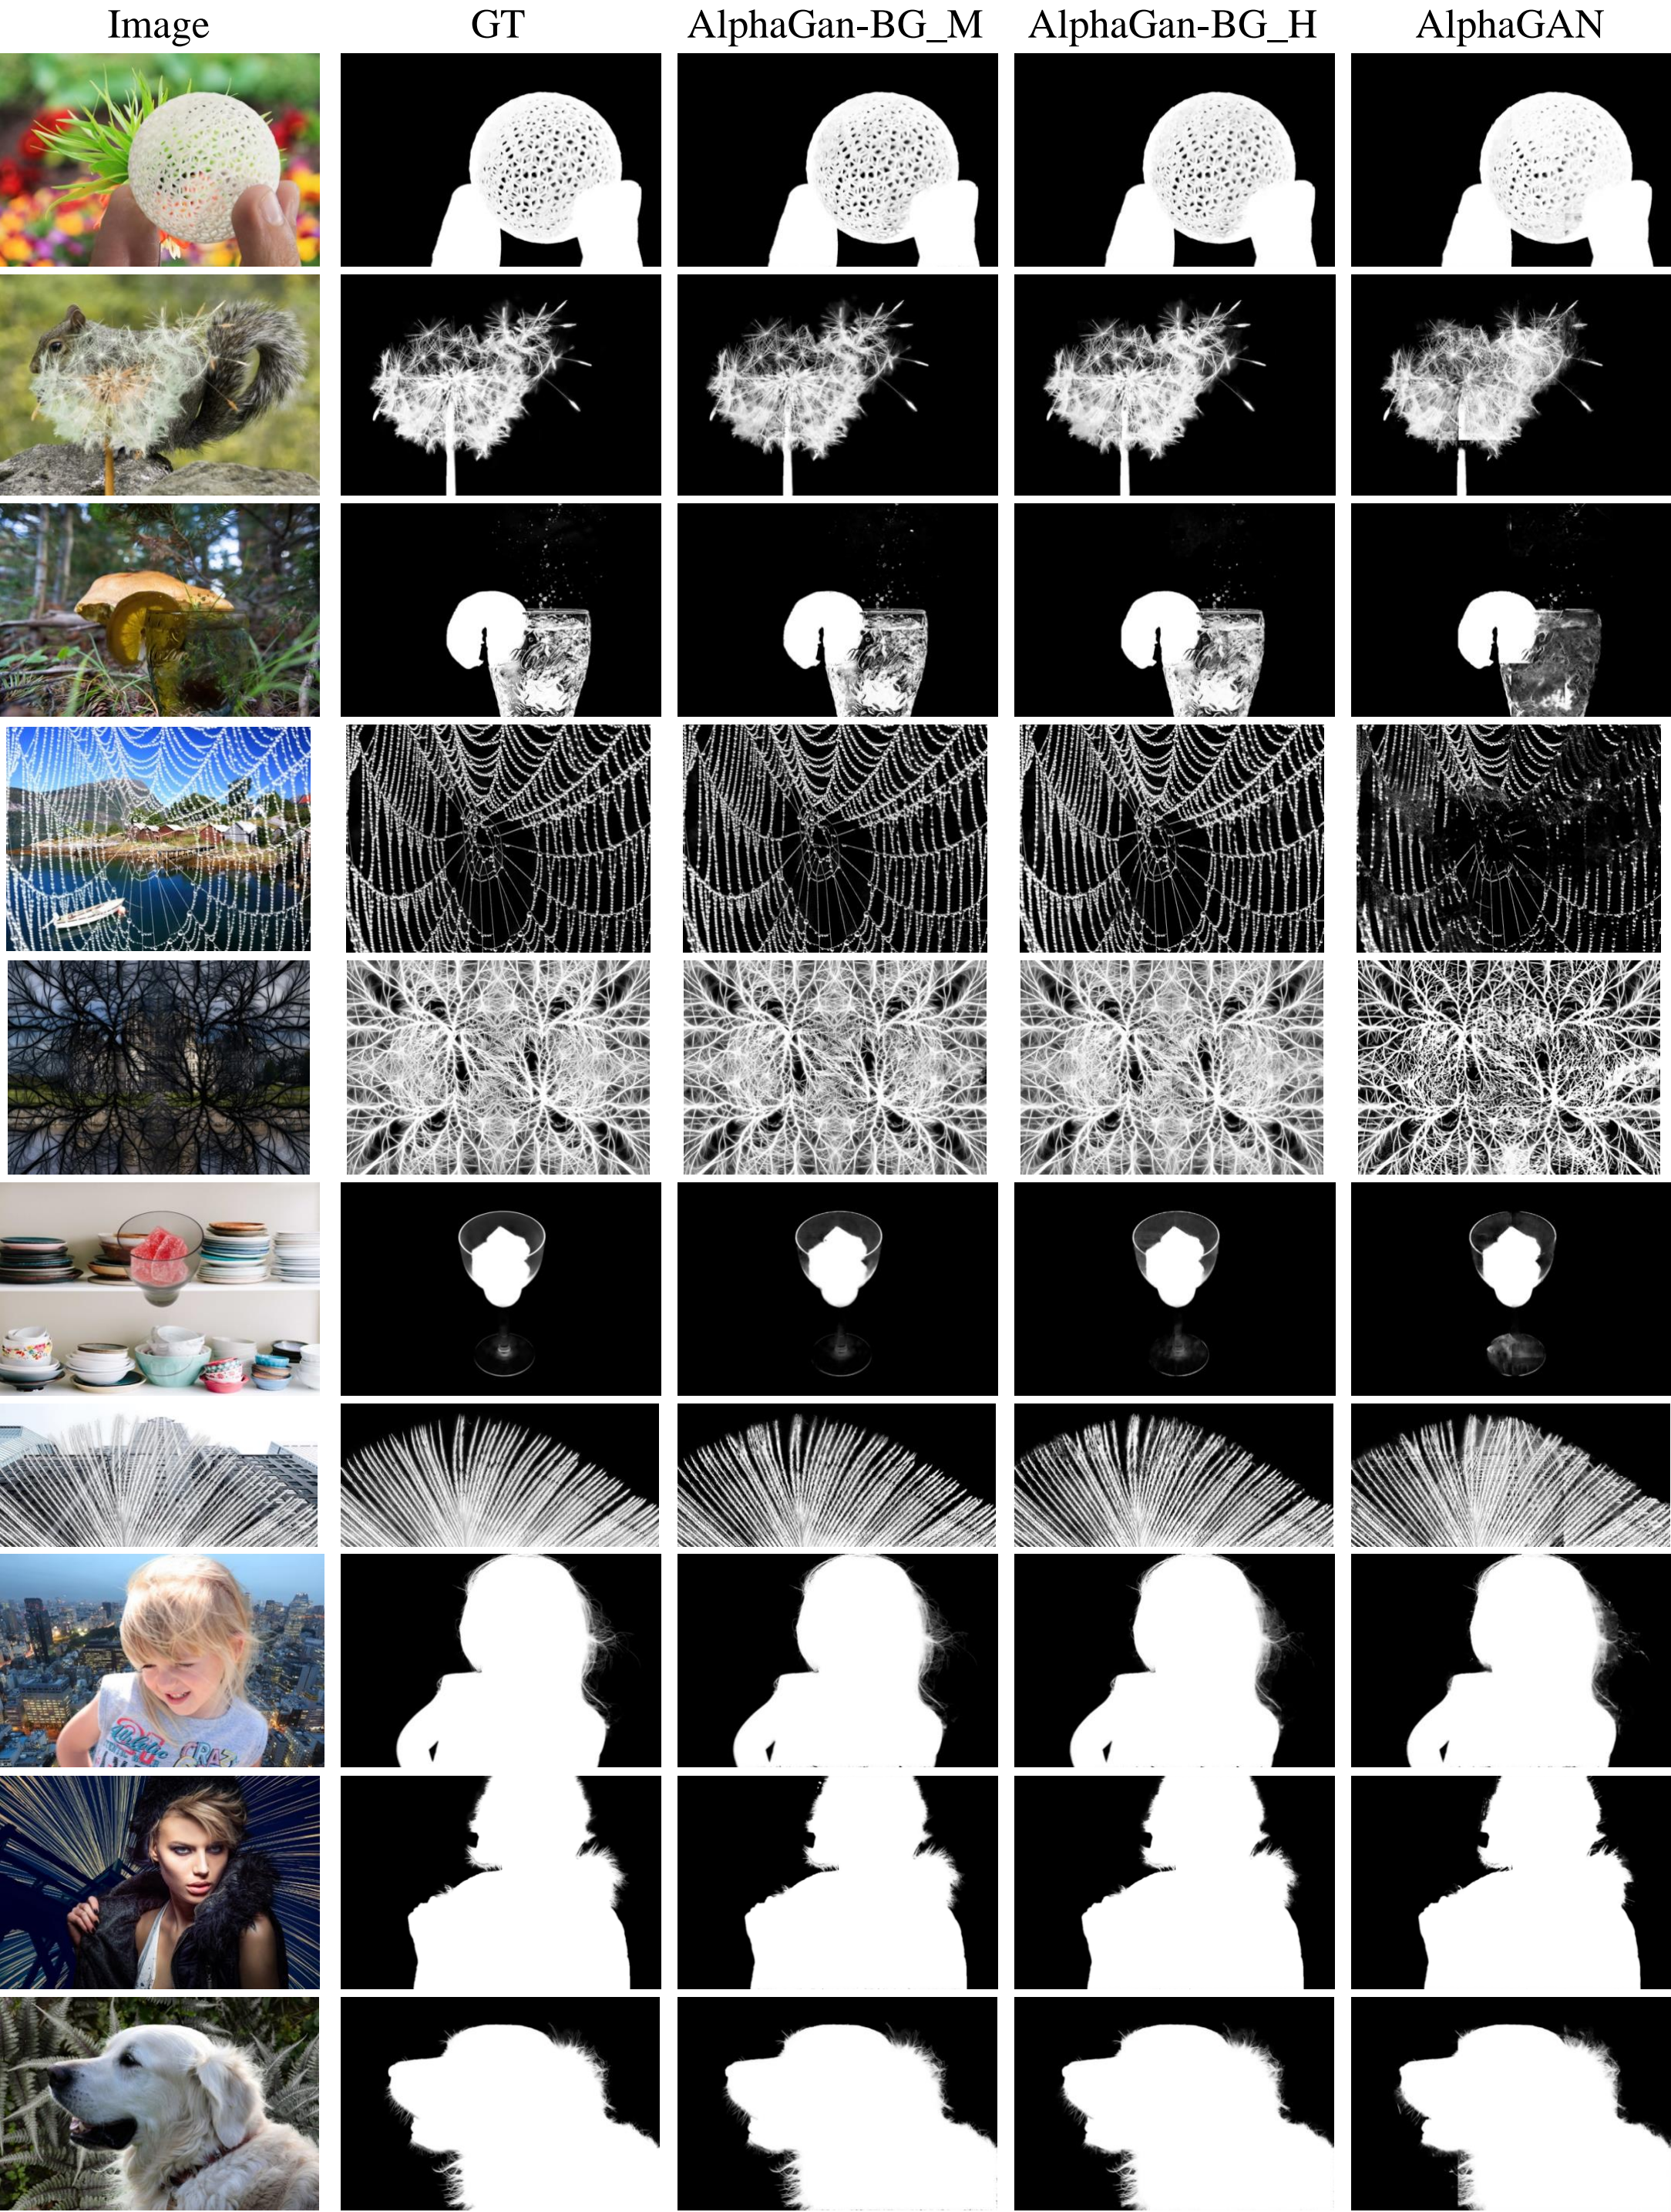 | 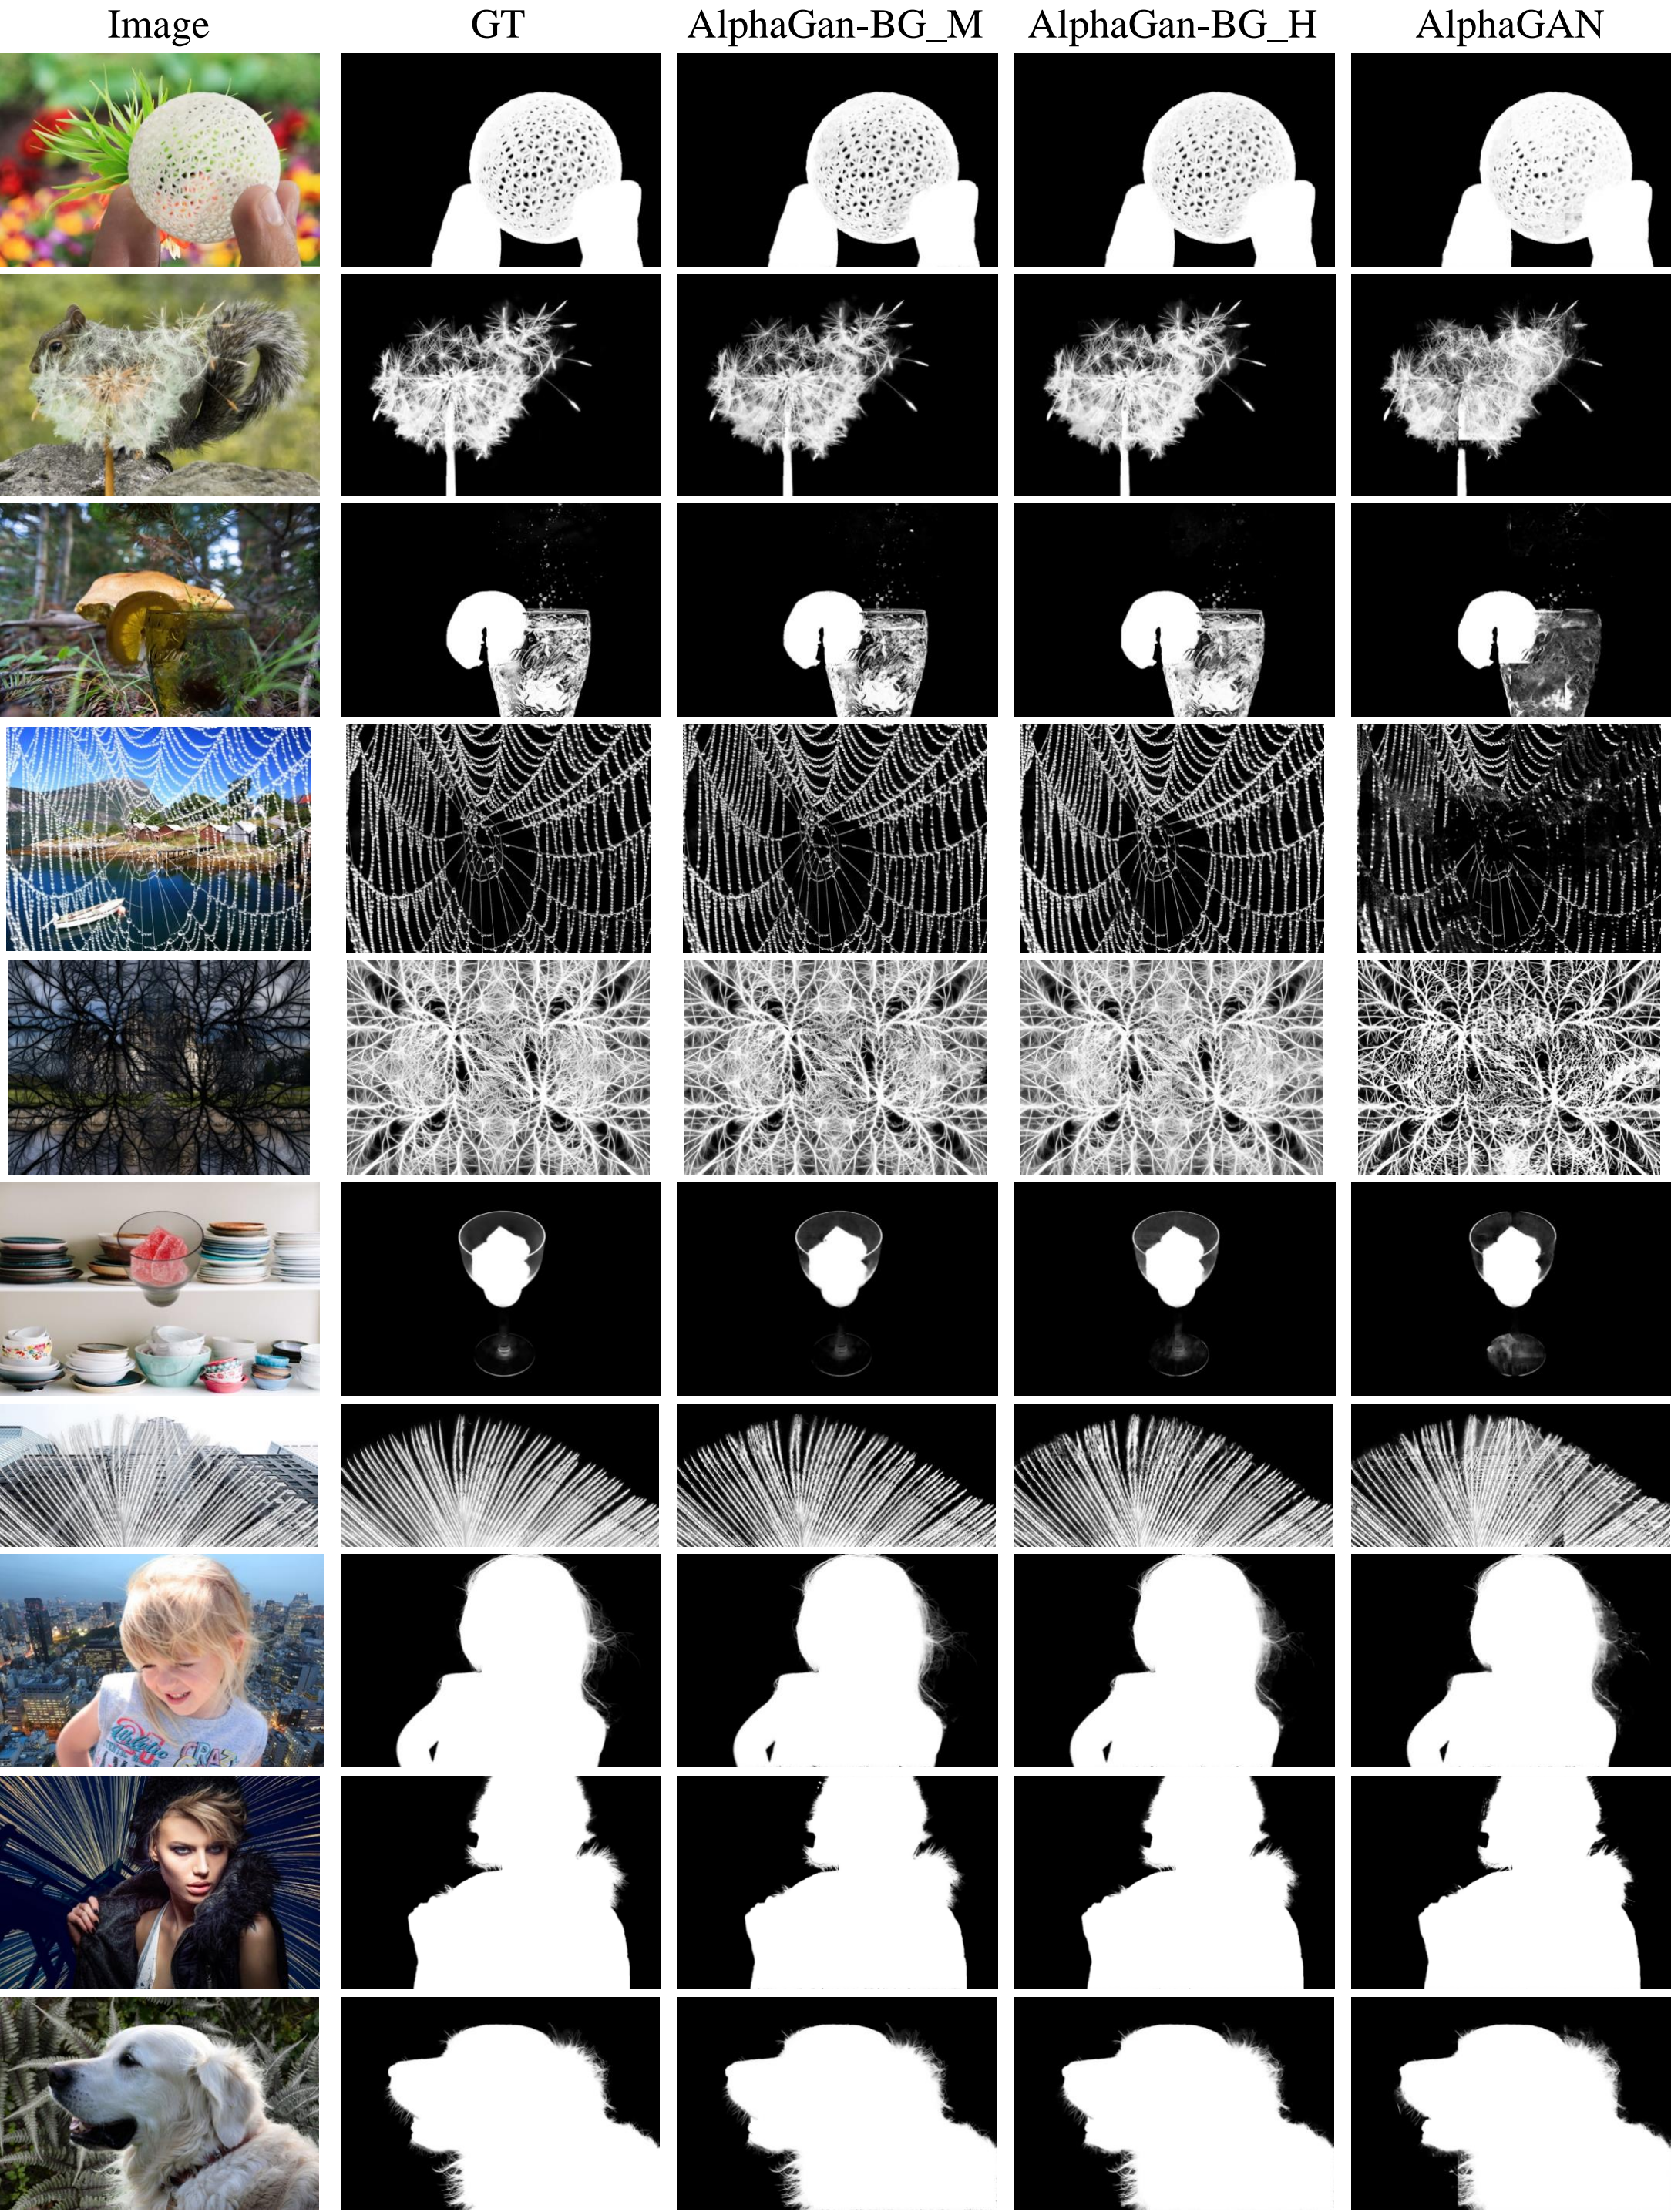 | 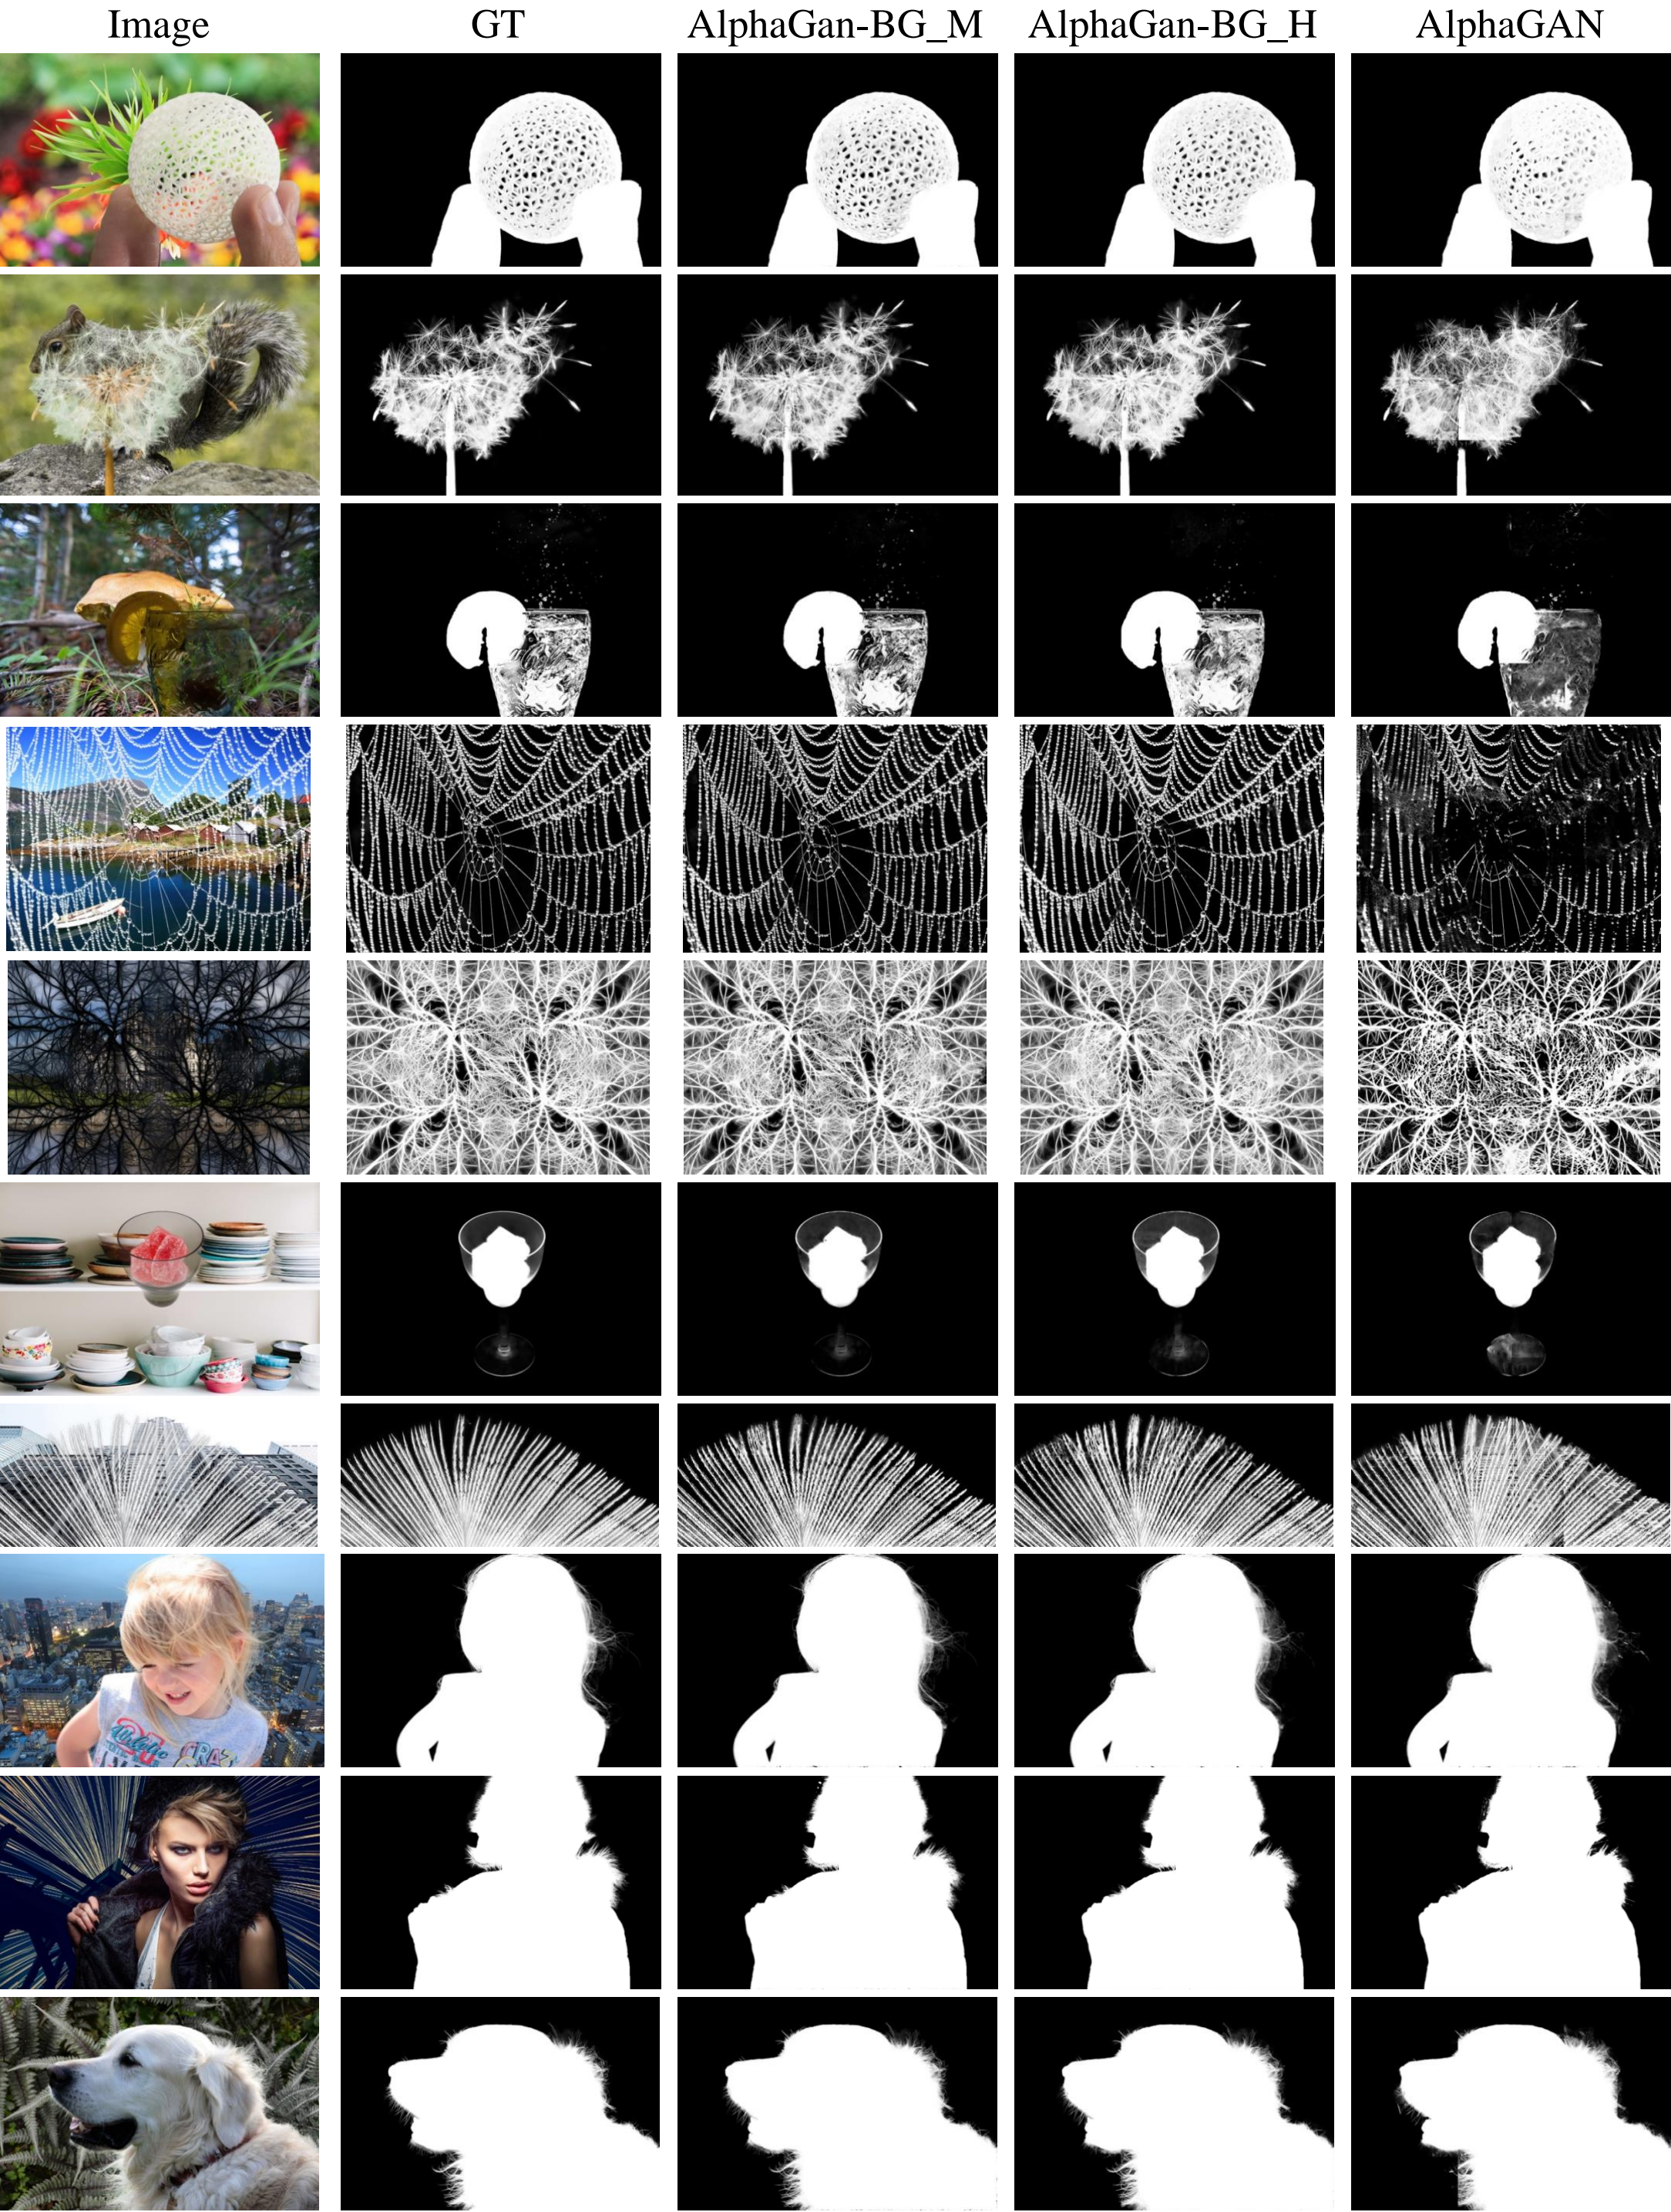 | 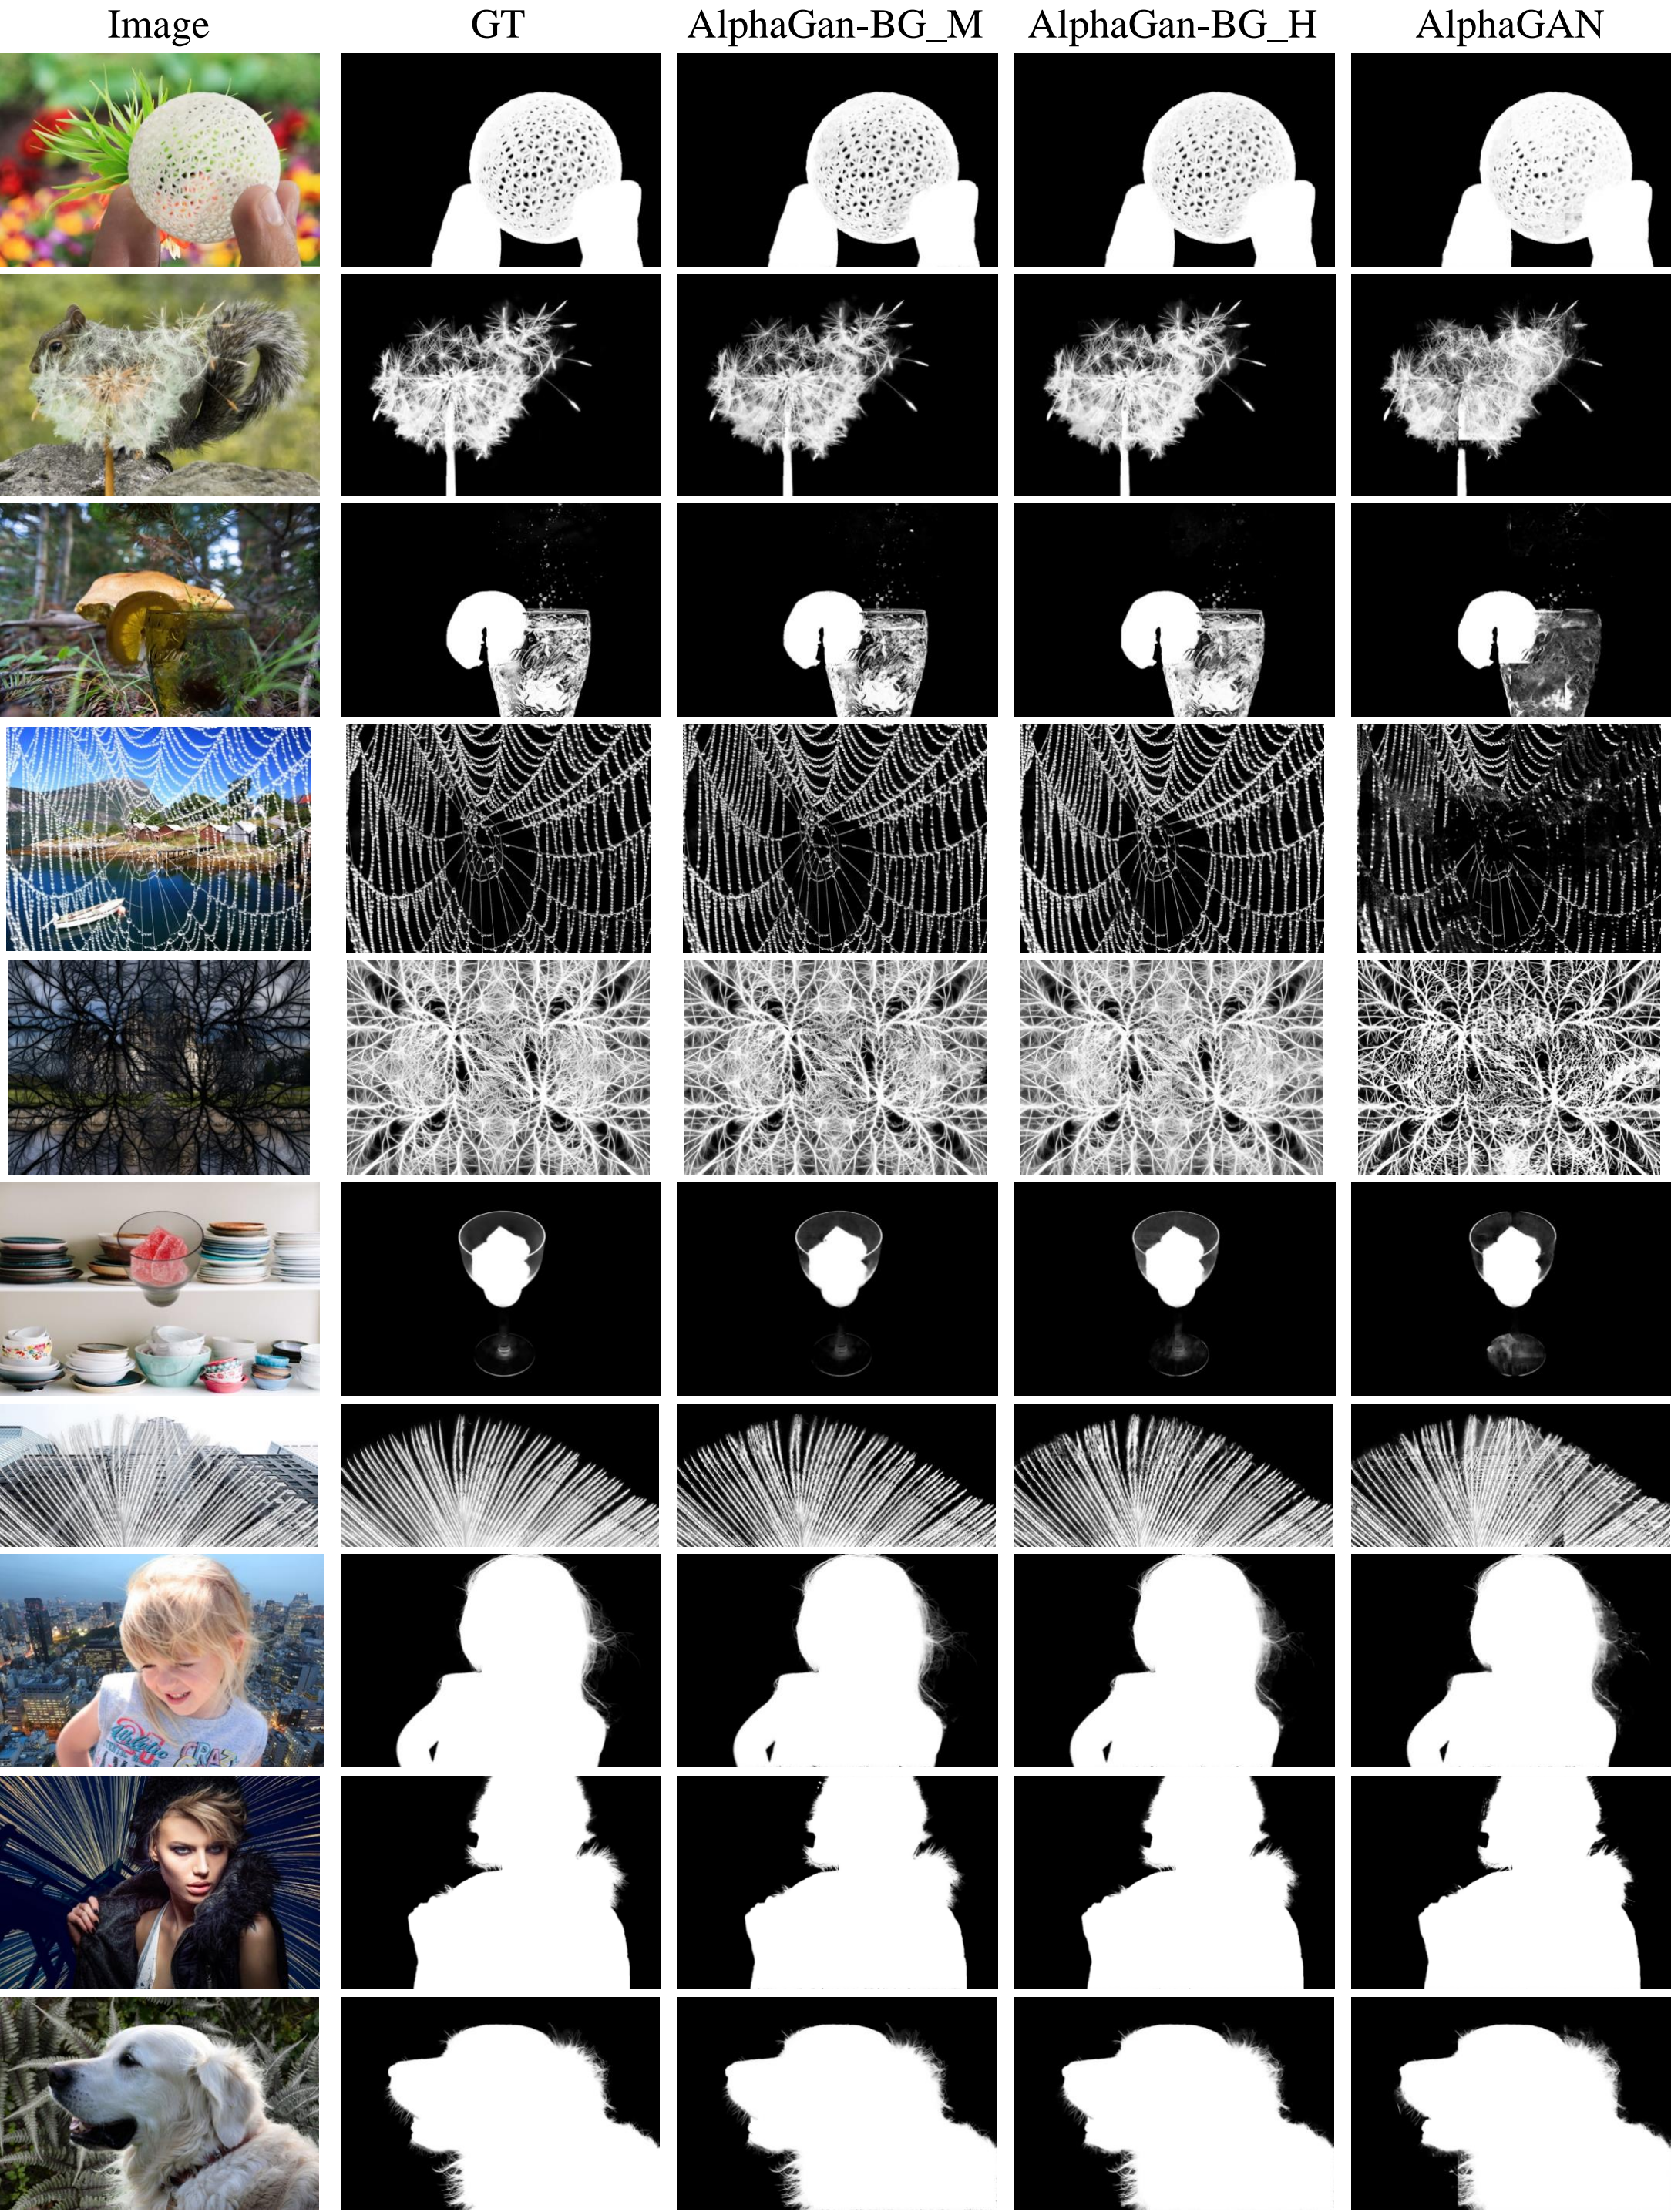 |
| 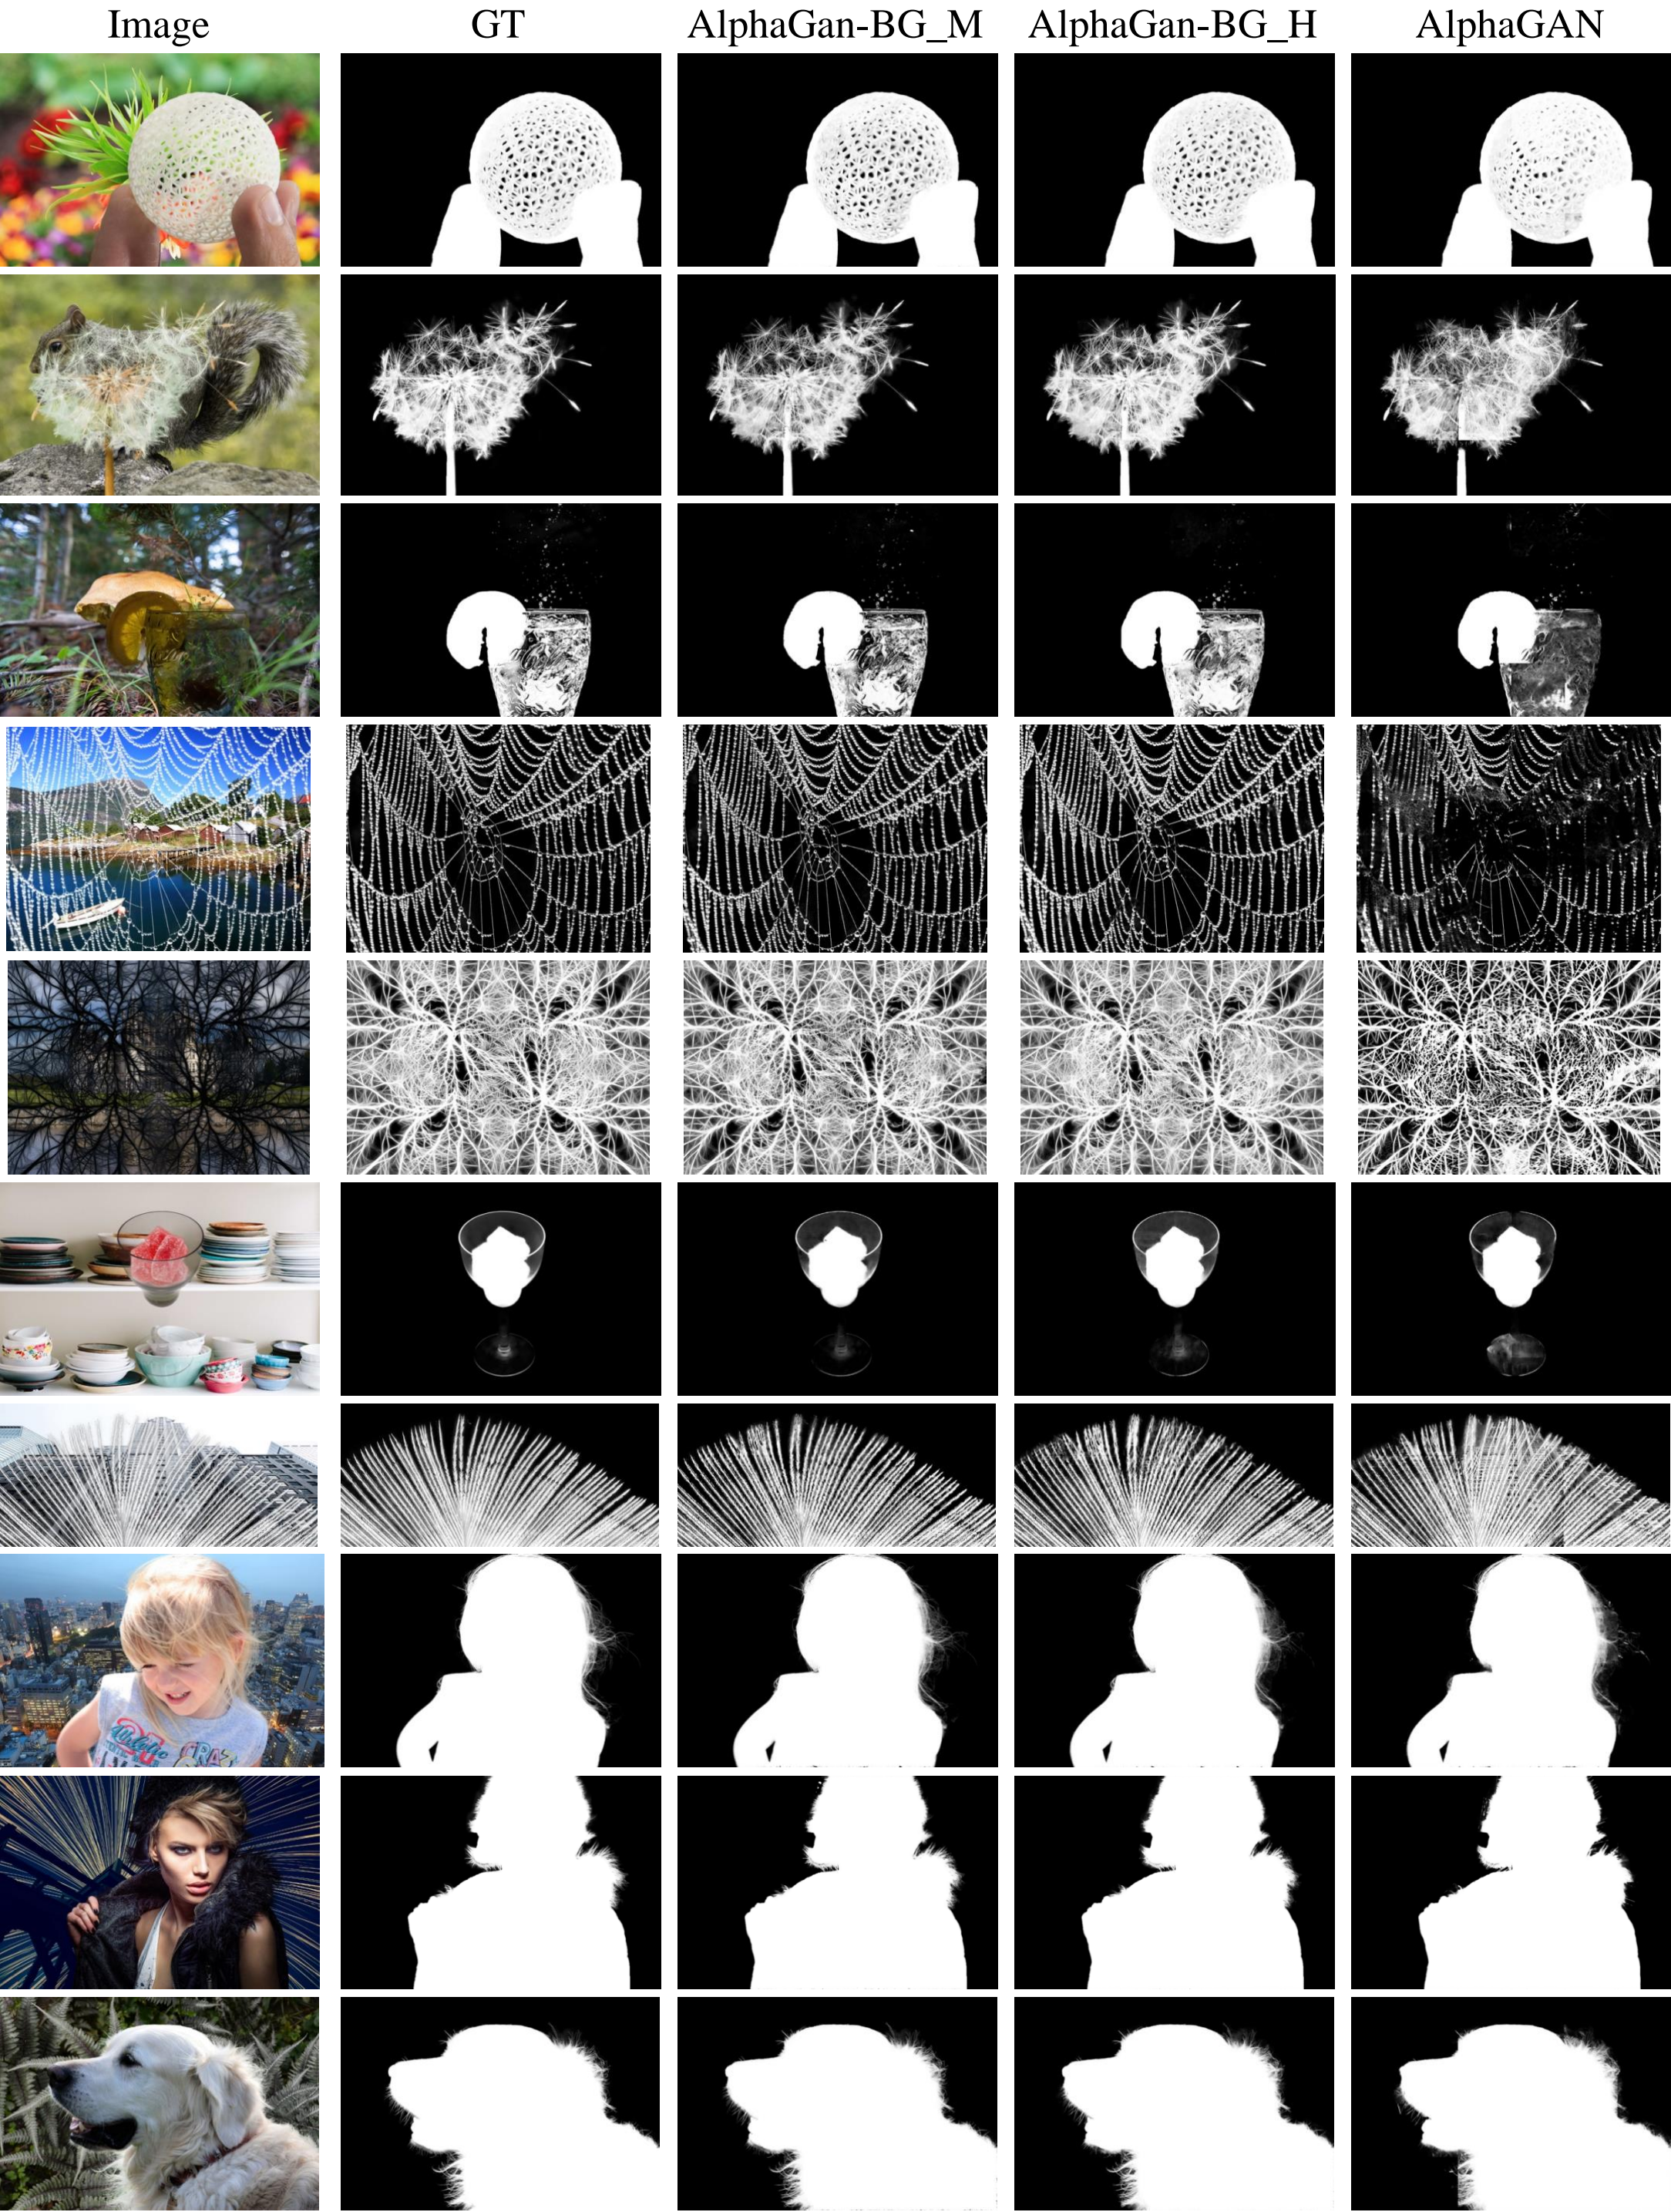 | 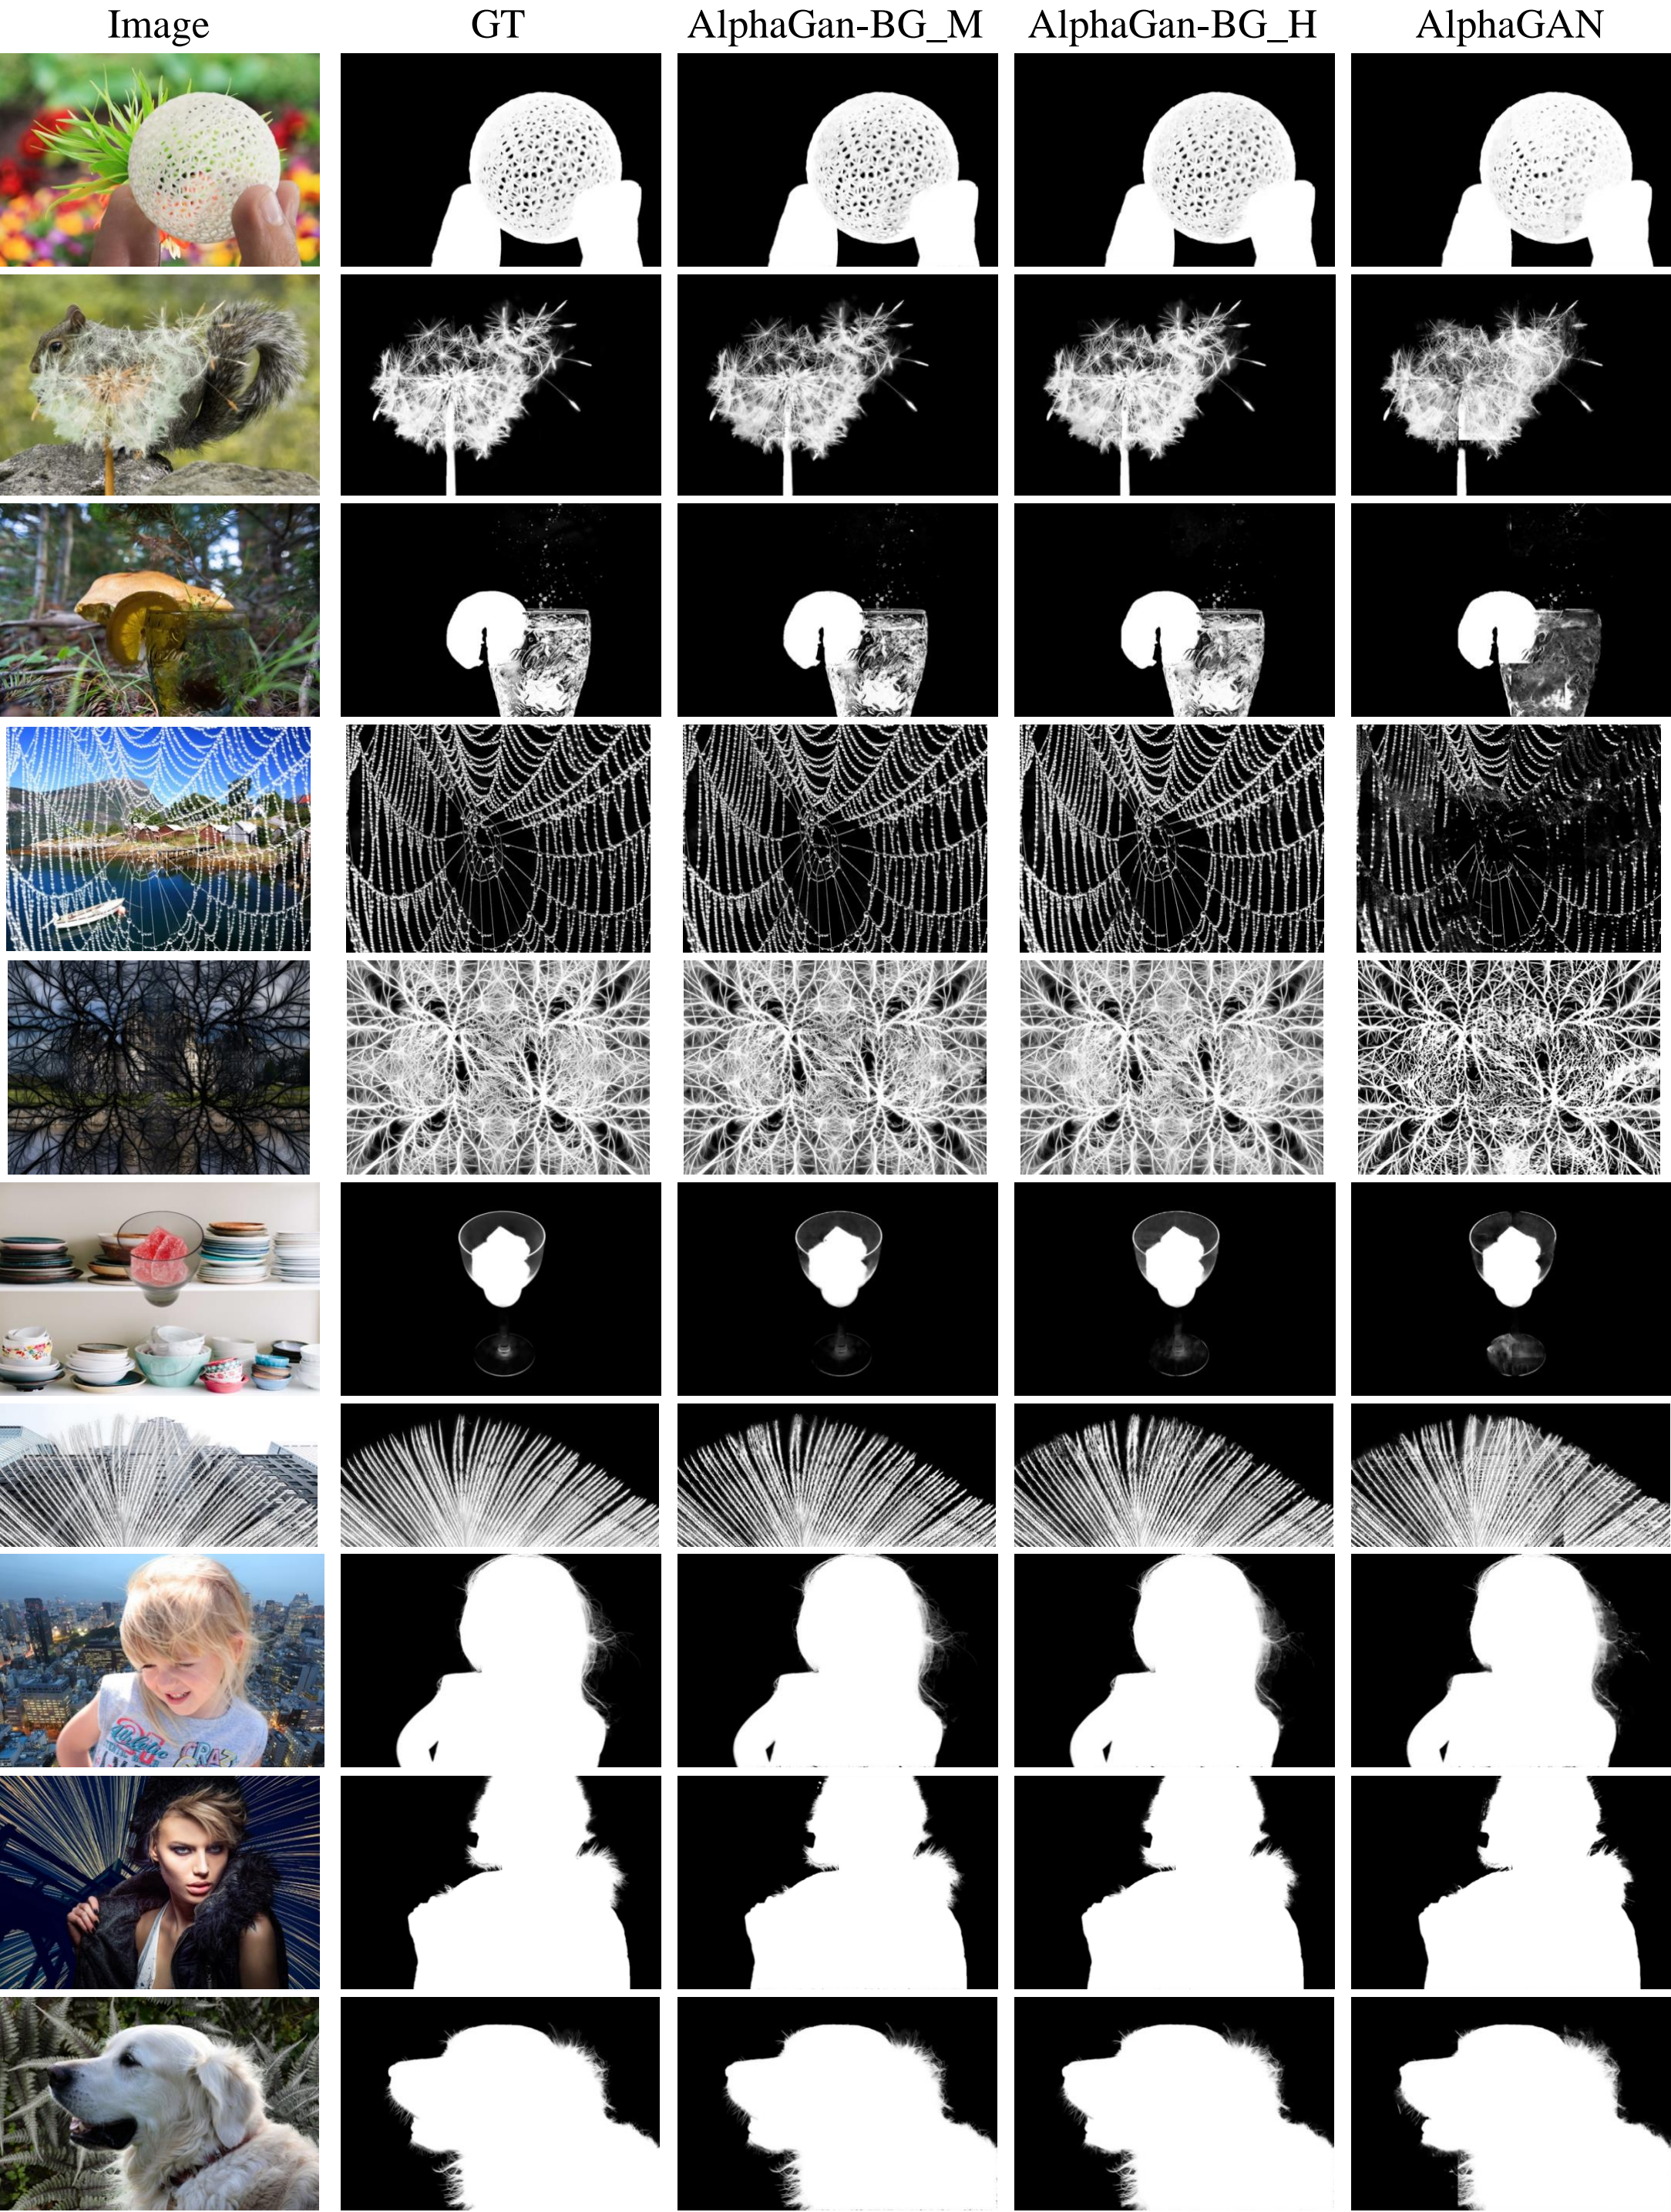 | 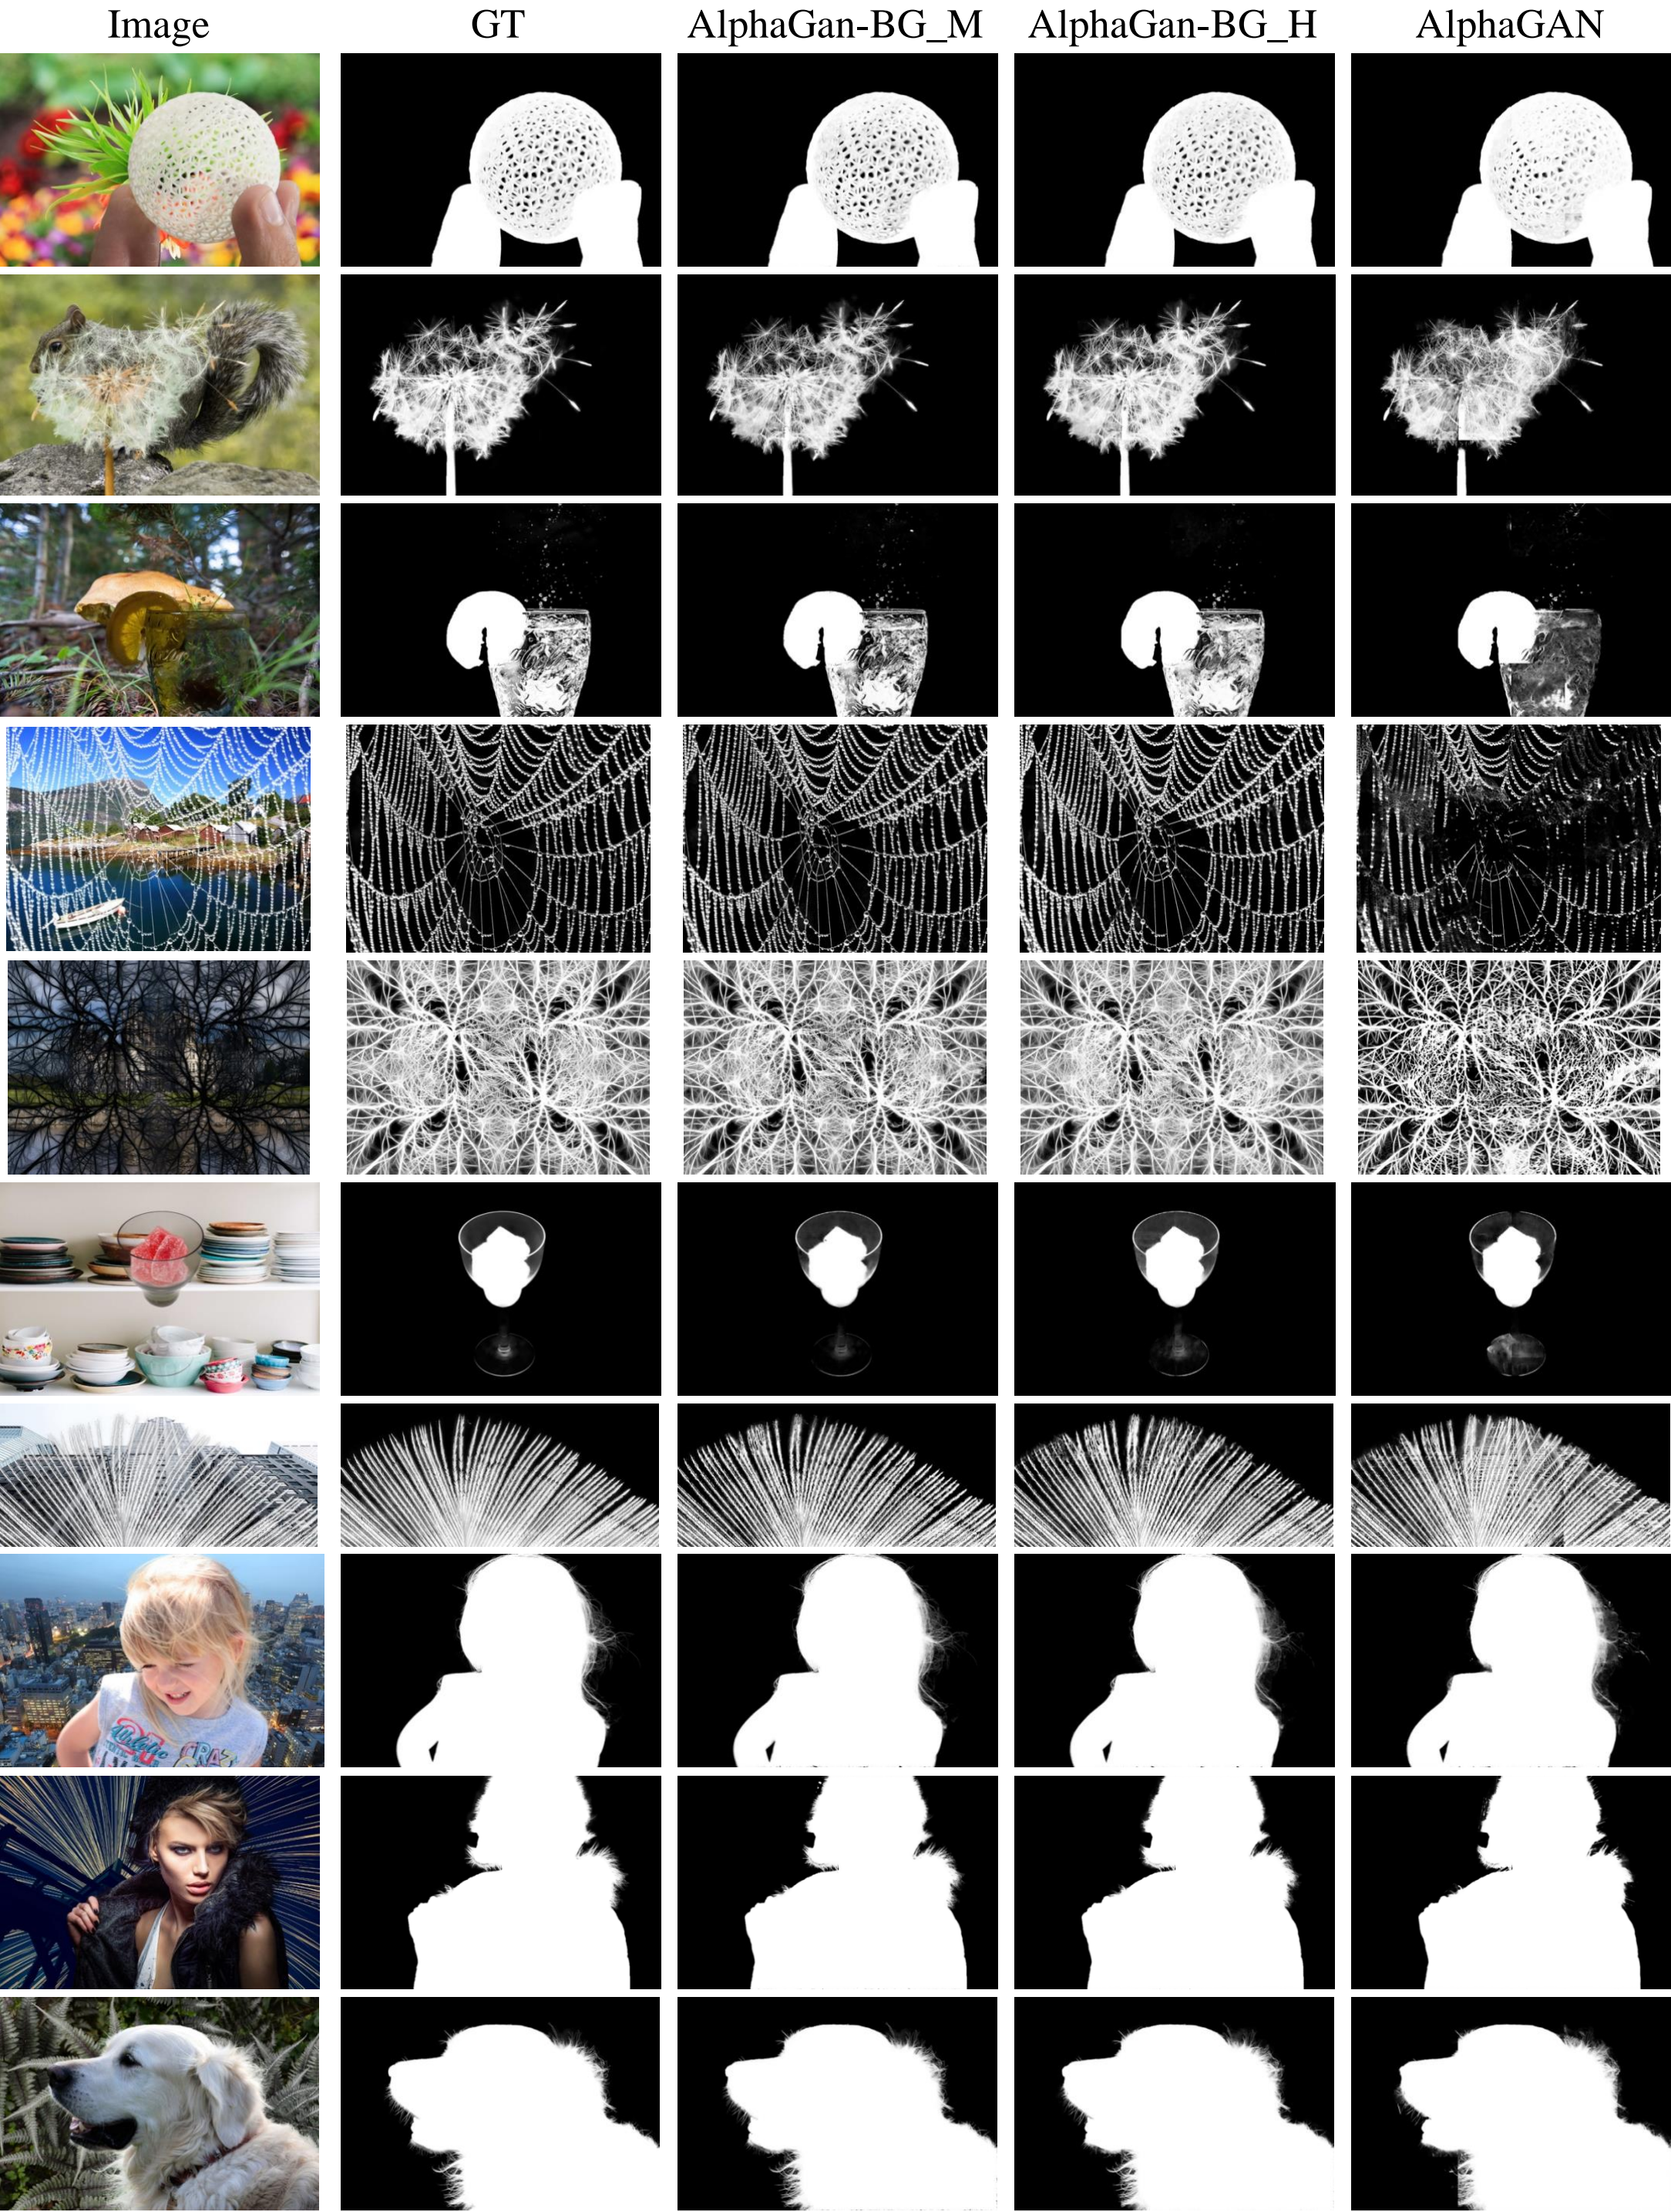 | 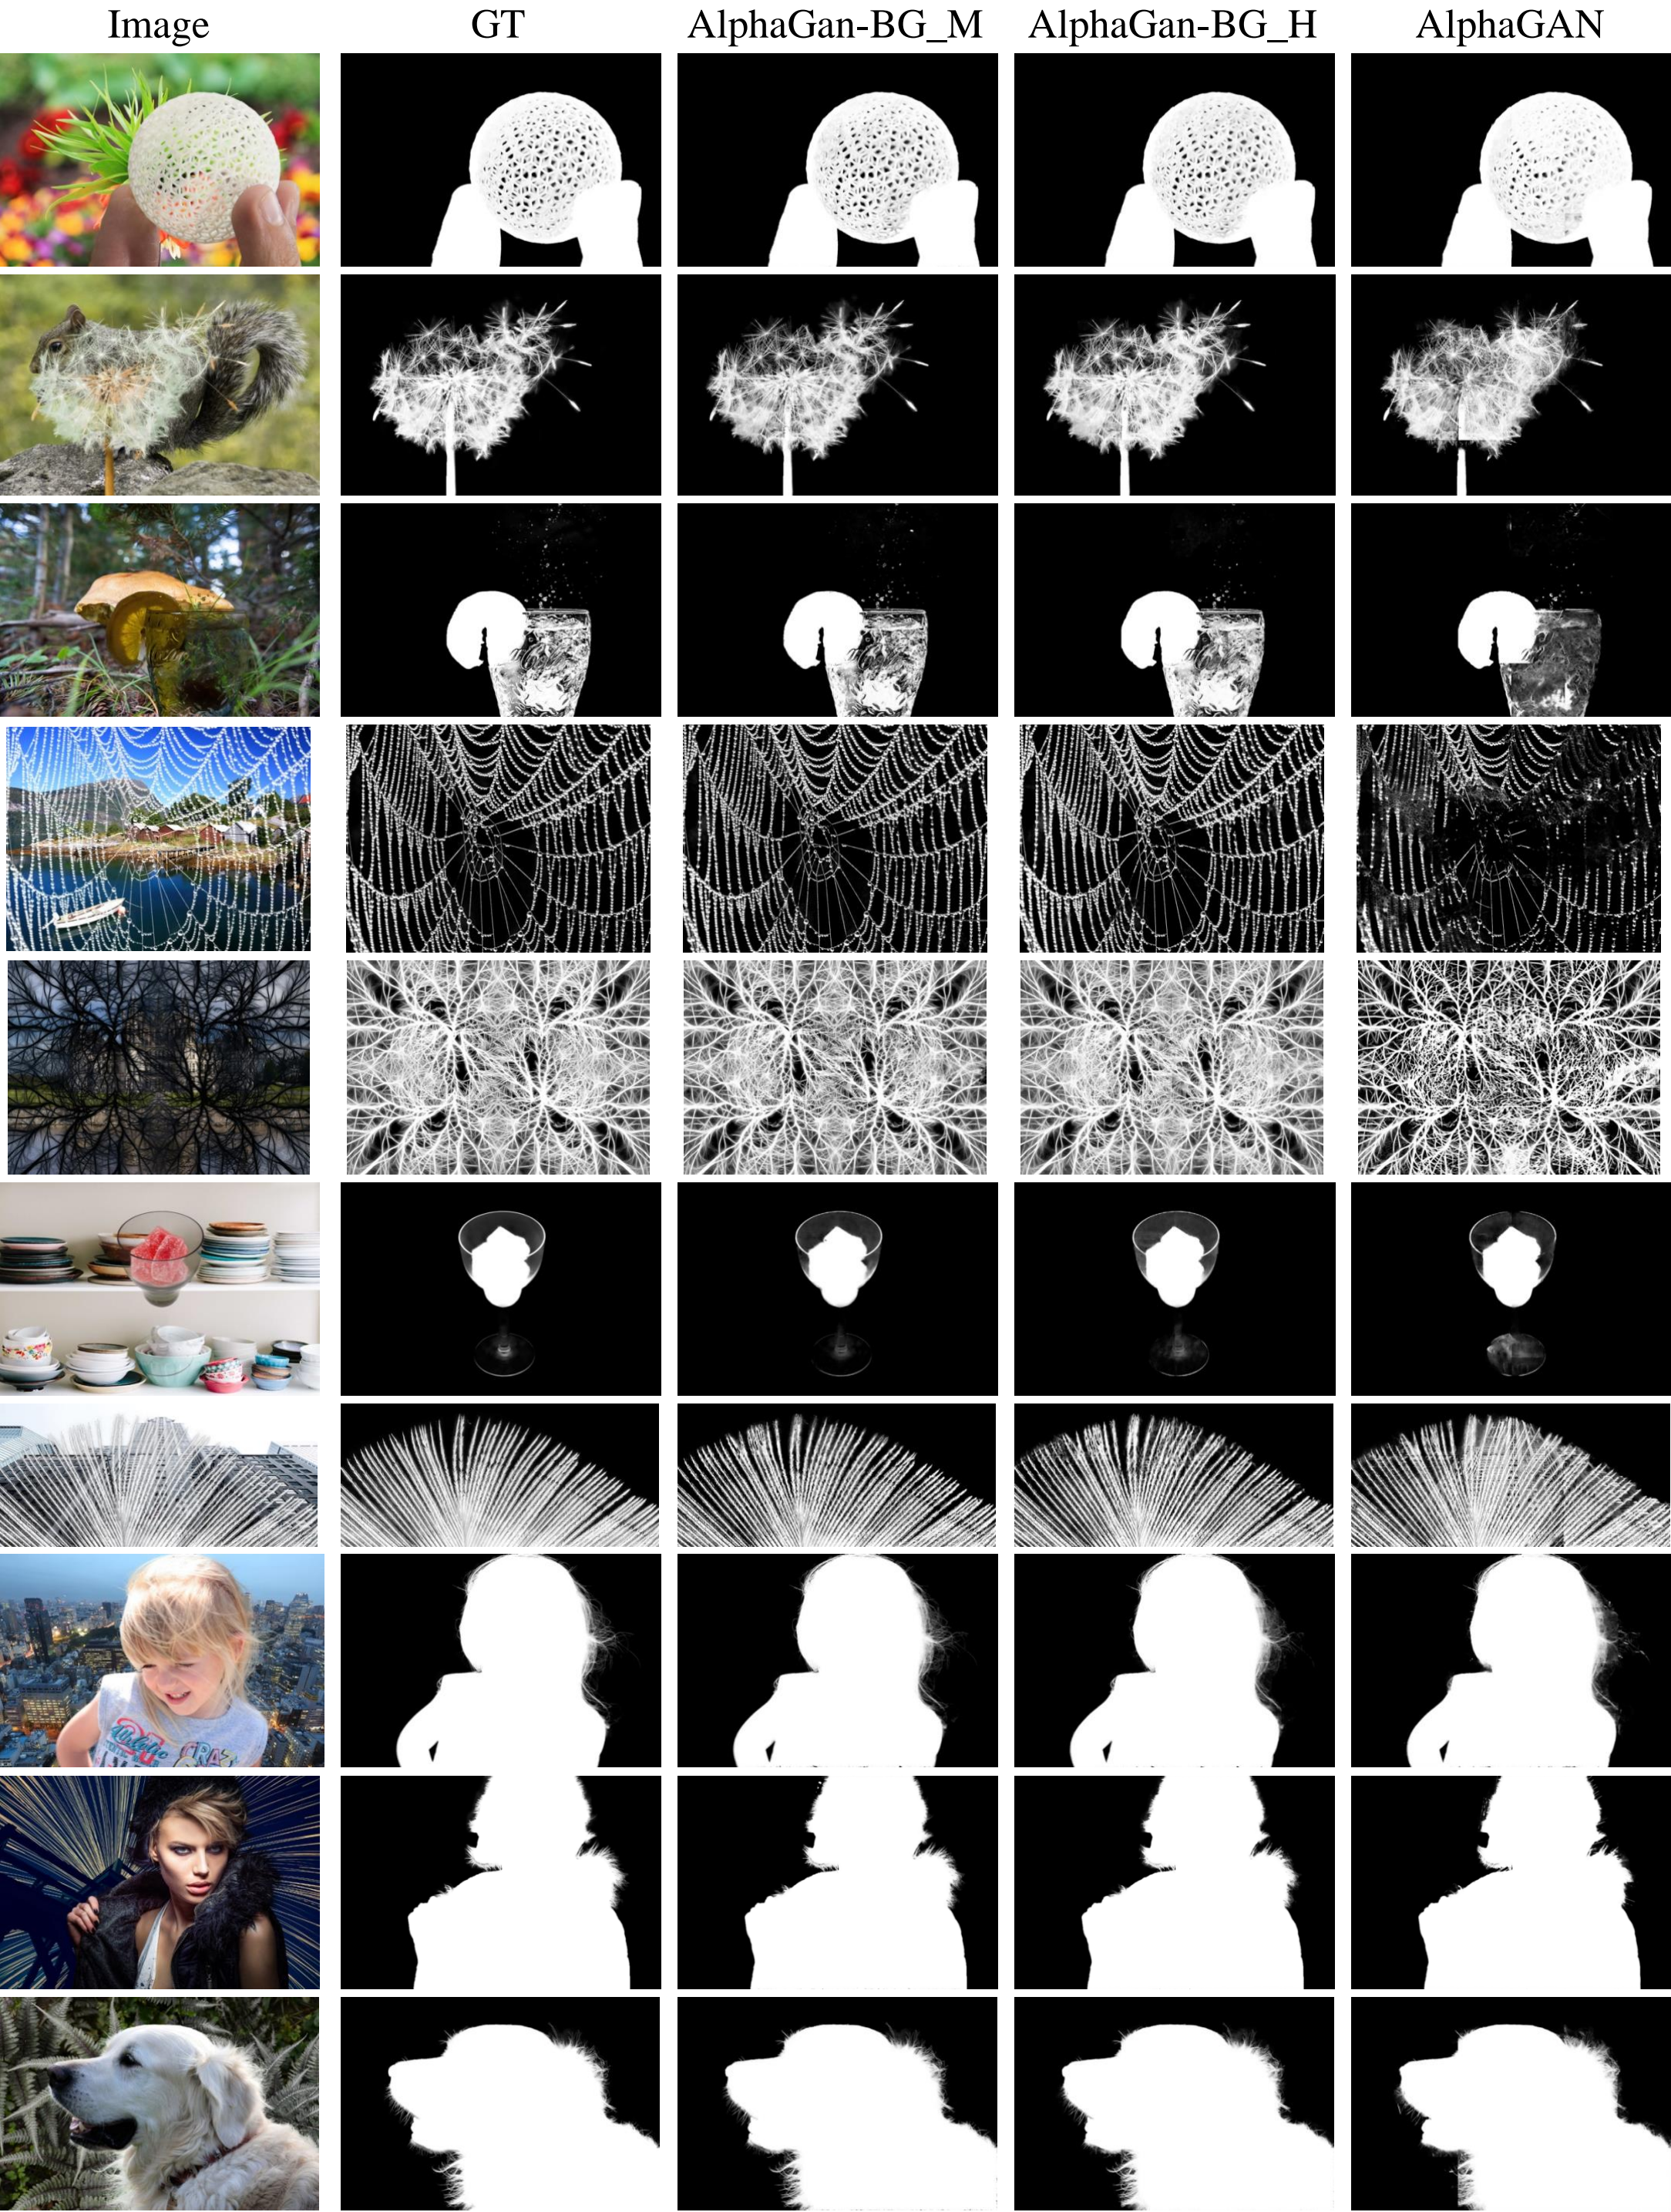 | 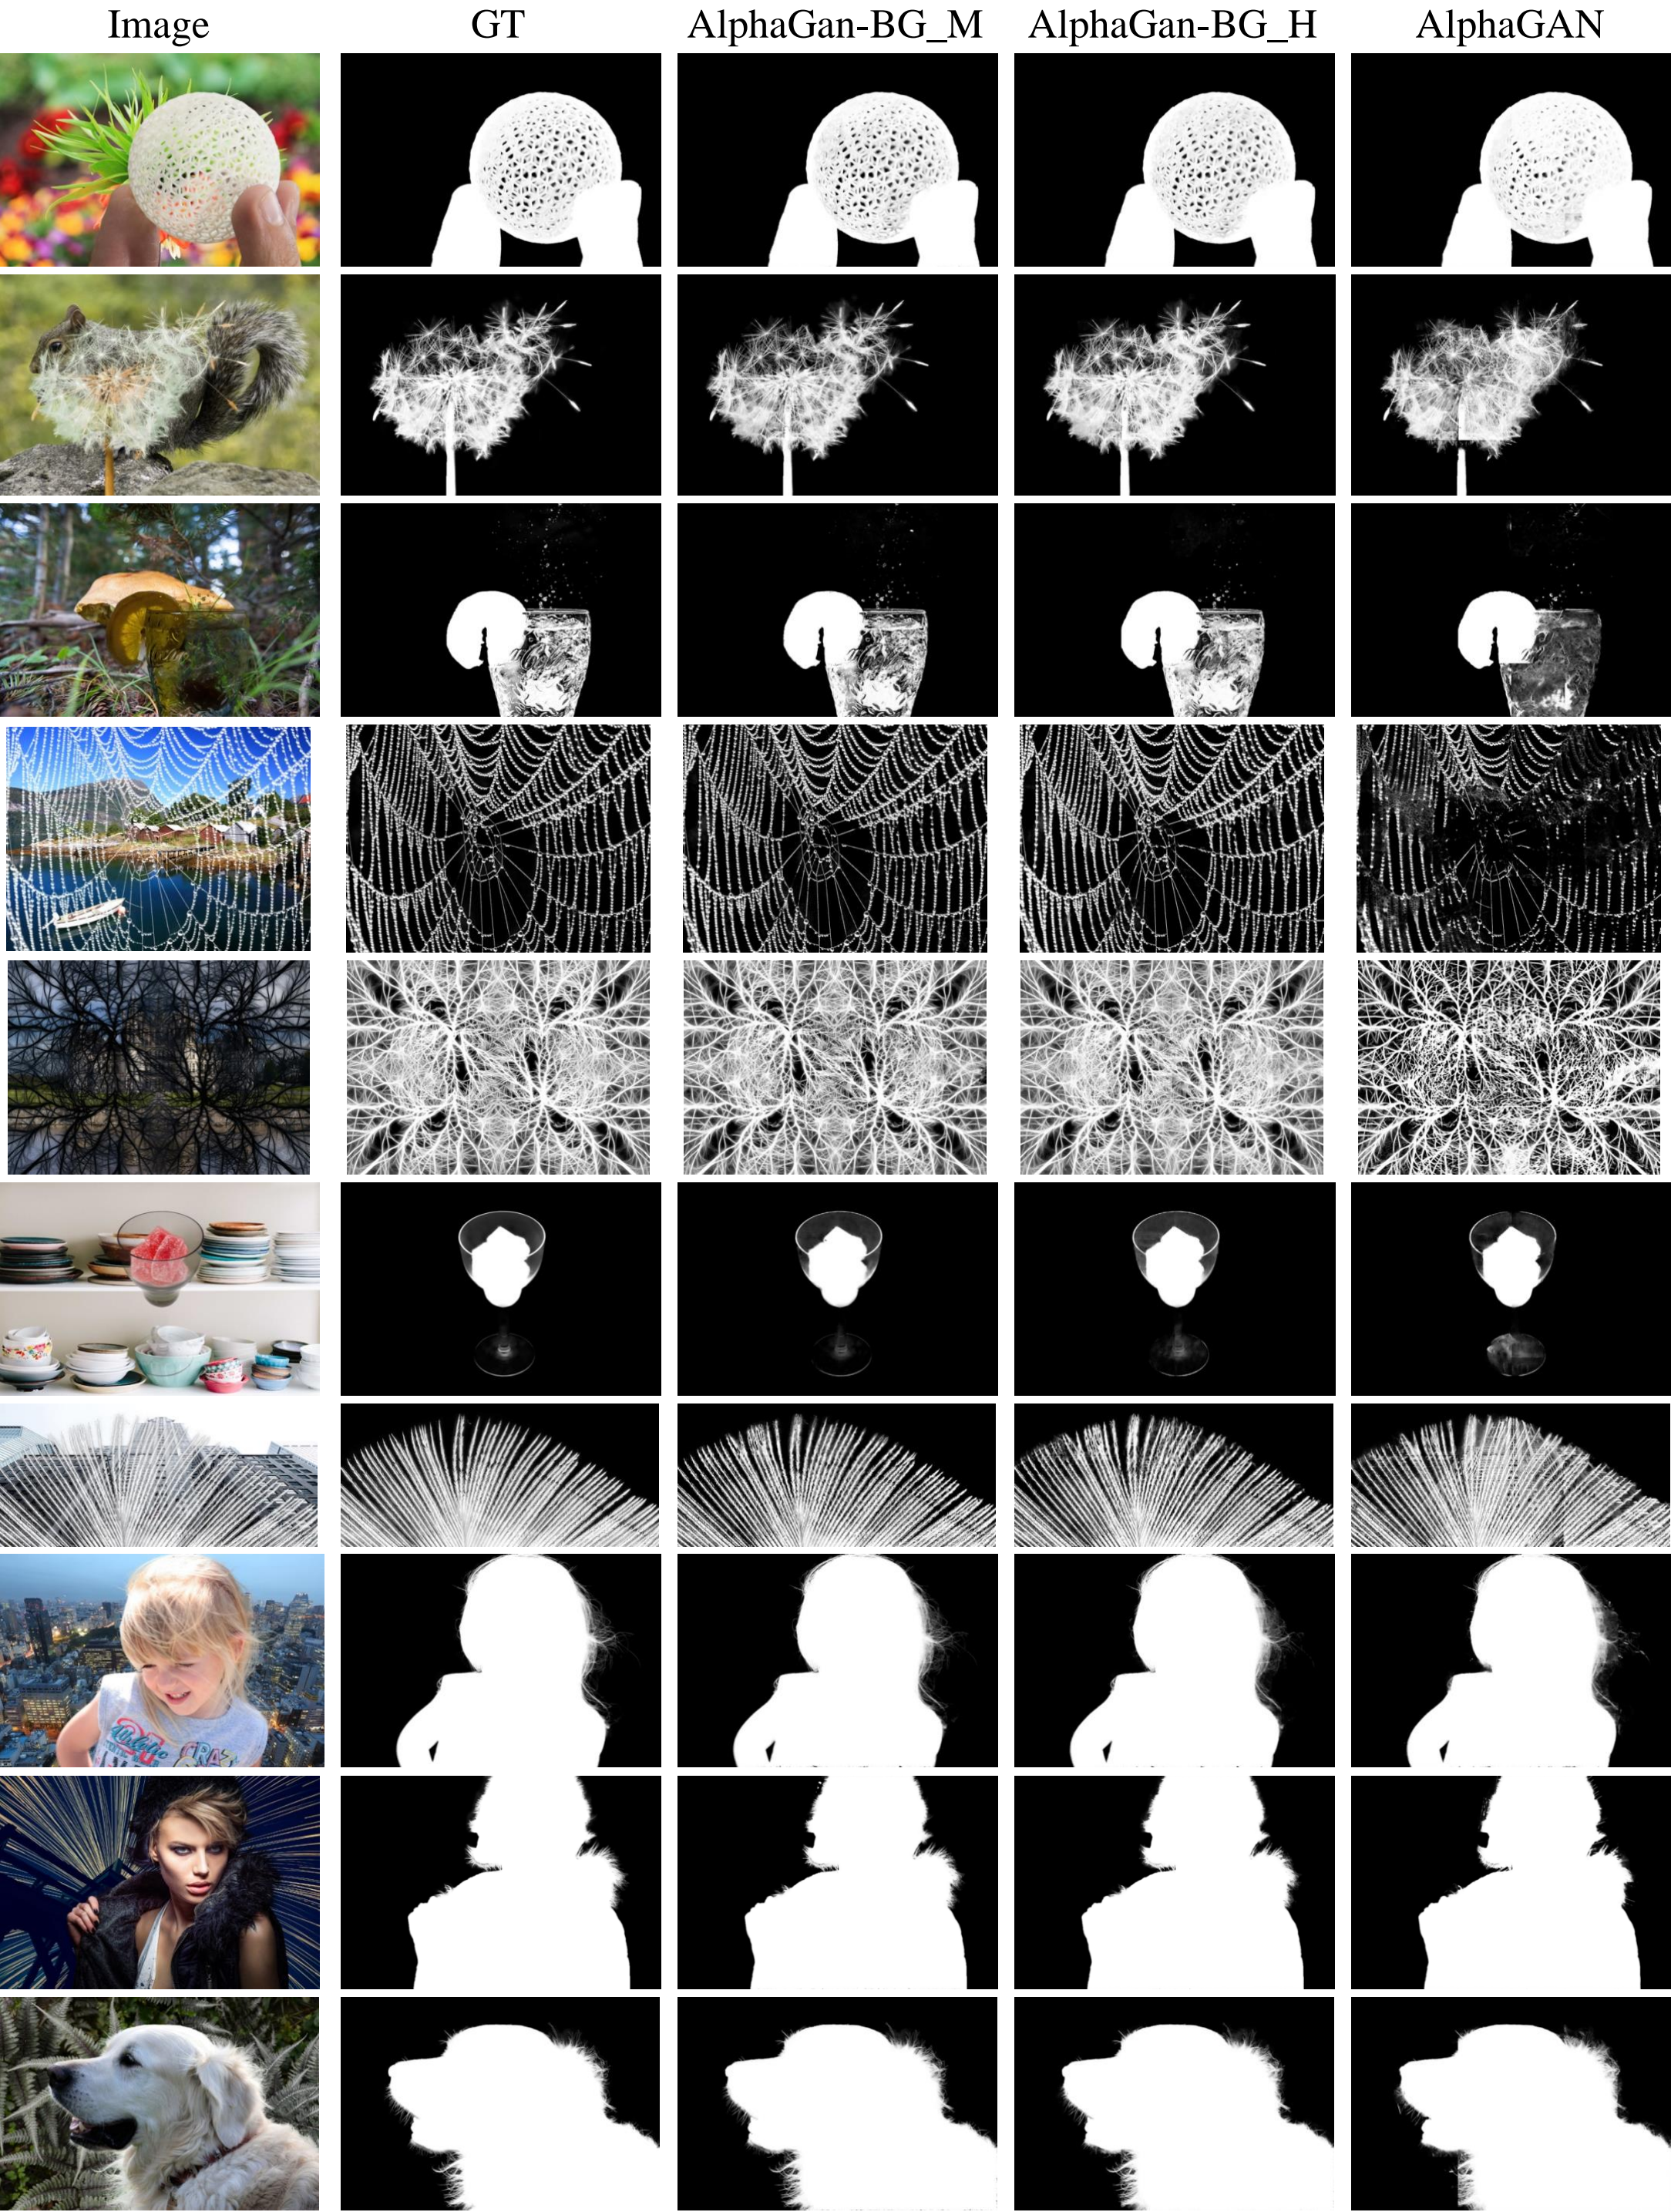 |



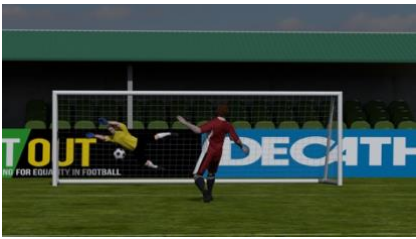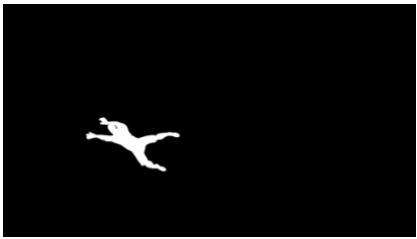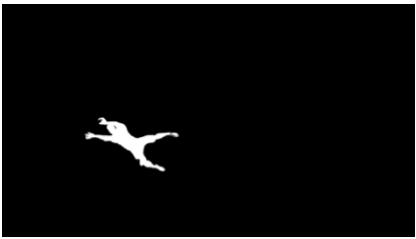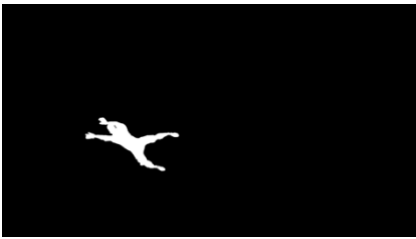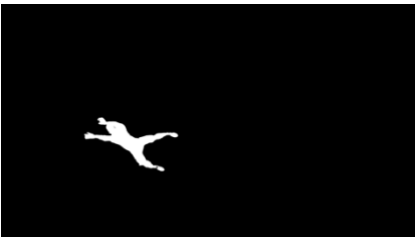

Supplement: Supplementary file 1 [file appendix-lowsize.pdf]
